# Supplementary material for: Cataclysmic variables from Sloan Digital Sky Survey -- V (2020-2023) identified using machine learning
Source: arXiv:2406.19459 ancillary file (2024-11-05)
Supplement: Supplementary file 1 [file Finding_CVs_using_machine_learning___supplementary_data.pdf]

# Cataclysmic variables from Sloan Digital Sky Survey - V (2020-2023) identified using machine learning – Supplementary data.

2 October 2024

## 1 INTRODUCTION

We include here all of the supplementary data supporting the main paper which could not be included because of its size.

In Section 2 we list the set of 504 CVs observed by SDSS-V. For previously known CVs we provide the earliest published reference and, where they exist, references for the best spectrum and orbital period. We also provide our classification of the CV using the definitions from [Inight et al. \(2023a\)](#).

In Section 3 we discuss individual CV classifications and other relevant discoveries. Section 3.1 discusses all the new CVs that we discovered that do not appear in the literature. In Section 3.2 we discuss previously known systems where we are providing the first spectrum, a new period or a new classification.

In Section 4 we present plots of the spectra and light curves for the 504 CVs and in Section 5 we list the fields and catalog IDs of the individual spectra. In Section 6 we list the CV spectra that were omitted from the training/test dataset and the reasons for each one being excluded.

Finally in Section 7 we list those objects, previously classified as CVs, that we now reclassify based on new evidence.

## 2 LIST OF CVS

Table 1: CVs from SDSS V. We provide the geometric distances from [Bailer-Jones et al. \(2021\)](#) and CV sub-types according to the definitions in Sect. 3 in [Inight et al. \(2023a\)](#). The references for the initial discovery (ID), spectrum (Sp) and orbital and superhump periods ( $P$  – where known) are also shown. New discoveries, orbital periods and sub-type identifications are shown in blue. Sub-type identifications in black are from VSX ([Watson et al. 2017](#)). : Tentative values, \* Superhump periods

| SDSS                | Name                          | Gaia EDR3<br>source_id | Period<br>(h) | Gaia EDR3<br>$G$ (mag) | Distance<br>(pc) | Variable<br>Sub-type | References |     |     |
|---------------------|-------------------------------|------------------------|---------------|------------------------|------------------|----------------------|------------|-----|-----|
|                     |                               |                        |               |                        |                  |                      | ID         | Sp  | P   |
| J000155.14–670743.3 | EF Tuc                        | 4707482485122305536    | 3.5:          | 14.85                  | 1329             | NL                   | 239        | 6   | 180 |
| J000600.15+012129.8 |                               | 2738755406045571968    | 1.52(10)      | 19.57                  | 352              | WZ Sge:              | 301        | 301 | 301 |
| J000633.70–690033.8 | HV 8001                       | 4706297108508032128    | 1.90(3)       | 15.1                   | 241              | SU UMa               | 100        | 52  | 52  |
| J000844.33–014014.8 | Gaia15abi                     | 2544817841421994624    |               | 18.15                  | 1236             | NL:/Polar            | 229        | 85  |     |
| J001204.50+020129.6 |                               | 2546760133008036096    | 3.288(1)      | 16.45                  | 1667             | NL                   | 55         | 243 | 1   |
| J002243.55+061002.7 | MGAB-V295                     | 2747622177049417344    | 1.9(1):       | 19.61                  | 2113             | SU UMa               | 336        | 85  | 85  |
| J002257.65+614107.5 | V1033 Cas                     | 430446643235641472     | 4.033         | 16.58                  | 1557             | IP                   | 19         | 344 | 344 |
| J002728.02–010828.7 | EN Cet                        | 2541910801397761152    | 1.424(1)      | 20.76                  | 1218             | WZ Sge               | 215        | 33  | 22  |
| J002848.83+591722.0 | V709 Cas                      | 428101969045877504     | 5.33290(7)    | 14.39                  | 725              | IP                   | 123        | 123 | 298 |
| J003529.47–735826.3 |                               | 4685792041310761984    |               |                        | 957              | CV:                  | 1          | 1   |     |
| J003827.05+250925.0 | 1RXS J003828.7+250920         | 2806802123399581056    | 2.26826(2)    | 18.63                  | 503              | SU UMa               | 350        | 219 | 85  |
| J003941.08+005427.5 | SDSS J003941.06+005427.5      | 2543387617312121216    | 1.52(1)       | 20.76                  | 1078             | WZ Sge:              | 33         | 33  | 252 |
| J004335.16–003729.7 |                               | 2530961280492678528    | 1.3721(14)    | 19.85                  | 447              | WZ Sge:              | 353        | 353 | 228 |
| J005000.03–760827.3 | BMAM-V424                     | 4684361817175293440    | 3.698(4)      | 14.9                   | 1031             | NL                   | 318        | 1   | 60  |
| J005050.87+000912.6 | GS Cet                        | 2537078211571341568    | 1.34          | 20.68                  | 308              | WZ Sge               | 333        | 333 | 333 |
| J010411.62–031342.2 |                               | 2531434796342548224    |               | 19.69                  | 1096             | SU UMa:              | 199        | 316 |     |
| J012132.92–740819.5 |                               | 4686117767317363072    |               | 16.91                  | 2972             | NL:                  | 1          | 1   |     |
| J012754.58–581717.5 | ASASSN -15bg                  | 4909517162610311040    | 1.57(1)*      | 20.43                  | 730              | SU UMa               | 93         | 1   | 34  |
| J012905.53–580841.2 |                               | 4909542996837627648    |               |                        | 357              | AM CVn               | 1          | 1   |     |
| J014227.07+001729.8 |                               | 2510205490257050496    | 1.88(4)       | 19.89                  | 697              | Polar:               | 155        | 155 | 301 |
| J015007.16+302203.9 | ZTF18abtgdw                   | 302565293359409152     |               | 18.83                  | 445              | SU UMa               | 364        | 1   |     |
| J015543.47+002807.4 | FL Cet                        | 2507796391561705728    | 1.452389(1)   | 18.65                  | 317              | Polar                | 160        | 160 | 284 |
| J020712.72–014116.3 |                               | 2494386992562185088    | 1.55(15)      | 20.27                  |                  | Polar:               | 85         | 85  | 301 |
| J020809.57+565239.7 |                               | 505110900157013376     |               | 18.77                  | 2961             | MCV:                 | 269        | 301 |     |
| J021008.36+571121.1 | UV Per                        | 457106501671769472     | 1.557(3)      | 17.75                  | 250              | SU UMa               | 166        | 166 | 253 |
| J021315.48+533822.9 | MASTER OT J021315.37+533822.7 | 455380951309048320     | 2.549(7)*     | 20.05                  | 3224             | SU UMa               | 164        | 301 | 138 |
| J022102.78+732245.1 | ASASSN-14jq                   | 546910213373341184     | 1.32427(31)*  | 19.94                  | 425              | WZ Sge               | 73         | 301 | 34  |
| J022623.33+711831.5 | AM Cas                        | 545338083544363392     | 3.9576(3)     | 14.37                  | 420              | U Gem                | 203        | 203 | 224 |
| J023322.61+005059.2 | HP Cet                        | 2500552912036565120    | 1.601(2)      | 20.12                  | 683              | WZ Sge:              | 160        | 150 | 150 |
| J024131.07+593630.4 | ASASSN-16jv                   | 464373929923792384     |               | 19.84                  | 607              | U Gem                | 73         | 301 |     |
| J024607.56–633546.0 | RU Hor                        | 4721232870163826816    | 1.7*          | 19.84                  | 581              | SU UMa               | 118        | 1   | 234 |
| J024720.92–605050.7 |                               | 4725131257359416960    | 2.4550366(57) | 18.56                  | 525              | Polar                | 1          | 1   | 1   |
| J031538.60+623314.9 | ASASSN-15qx                   | 463818298599820800     |               | 17.98                  | 1177             | ER UMa               | 93         | 1   |     |
| J032815.90+612517.5 | Gaia19bbb                     | 462713869228951424     | 1.5751(2)     | 18.22                  | 244              | SU UMa:              | 5          | 1   | 1   |
| J034515.42–015216.4 | CSS 090219:034515-015216      | 3251069657846812800    | 1.684(1)      | 18.91                  | 399              | SU UMa               | 151        | 1   | 205 |
| J040834.99+511448.2 | FO Per                        | 250700853140894976     | 3.3752(2)     | 16.15                  | 587              | U Gem                | 140        | 144 | 1   |
| J041428.92–631946.0 |                               | 4676110149911252992    |               | 19.03                  | 1026             | DN:                  | 1          | 1   |     |

| SDSS                | Name                          | Gaia EDR3<br>source_id | Period<br>(h) | Gaia EDR3<br>G (mag) | Distance<br>(pc) | Variable<br>Sub-type | References |     |     |
|---------------------|-------------------------------|------------------------|---------------|----------------------|------------------|----------------------|------------|-----|-----|
|                     |                               |                        |               |                      |                  |                      | ID         | Sp  | P   |
| J041844.43+510731.3 | NS Per                        | 271562333932151040     | 6.2994(7)     | 17.43                | 1076             | U Gem                | 186        | 144 | 1   |
| J042609.35+354144.3 | MASTER OT J042609.34+354144.8 | 176429285061830144     | 1.57232(3)    | 16.14                | 184              | SU UMa               | 133        | 226 | 1   |
| J043118.90–005534.9 |                               | 3206246103540947968    |               | 19.58                | 534              | MCV:                 | 1          | 1   |     |
| J043127.01+352713.0 | ASASSN-16og                   | 174868189003974016     | 1.48(1)       | 20.37                | 1677             | SU UMa               | 73         | 301 | 303 |
| J044321.37+472125.8 | V392 Per                      | 254361745823908736     | 77.28(1)      |                      |                  | Nova                 | 225        | 241 | 148 |
| J044652.51+471408.3 |                               | 255613436732021888     | 6.63(2)       | 17.36                | 2403             | CV                   | 1          | 1   | 1   |
| J050153.52–034208.6 | ZTF18abwtmcs                  | 3213078370011948160    | 1.534(1)      | 20.58                | 1905             | WZ Sge:              | 1          | 1   | 1   |
| J050503.07+222529.7 | ASASSN-15su                   | 3418268607216934016    | 1.608(7)*     | 19.12                | 588              | SU UMa               | 73         | 301 | 319 |
| J050906.73–032507.7 | ASASSN-15em                   | 3214449559796032256    | 8.4780(2)     | 17.19                | 1309             | U Gem                | 93         | 1   | 1   |
| J051042.60+513539.9 | MASTER OT J051042.59+513540.0 | 262686320156108288     |               | 20.58                | 3493             | U Gem:               | 356        | 1   |     |
| J051419.88+011120.9 | CSS 091109:051420+011121      | 3233913634323725696    |               | 19.61                | 805              | DN                   | 161        | 1   |     |
| J051814.55–024503.1 | CSS 090219:051815-024503      | 3214173032620838144    |               | 17.86                | 1256             | U Gem                | 98         | 316 |     |
| J051949.58+642921.7 | ZTF18acnavqf                  | 479934630799062656     |               | 16.98                | 2131             | NL:                  | 312        | 312 |     |
| J052316.13–630728.9 | ASASSN-14ky                   | 4757322488219624576    |               | 20.48                | 1151             | DN                   | 93         | 1   |     |
| J052433.47–070527.9 | CSS 101108:052433-070528      | 3207332631484540416    |               | 20.59                | 1538             | SU UMa:              | 98         | 301 |     |
| J052834.08+331821.7 | QZ Aur                        | 3449050362952844288    | 8.579928(1)   | 16.87                | 2528             | Nova                 | 169        | 221 | 66  |
| J052859.54–033352.4 | V1159 Ori                     | 3210749947983249408    | 1.492272(2)   | 14.28                | 351              | ER UMa               | 39         | 39  | 167 |
| J060602.72–603941.4 | ASASSN-14jf                   | 5482325921402847872    | 1.329(1)      | 20.43                | 681              | WZ Sge               | 114        | 1   | 34  |
| J061204.48+252832.5 | HQ Gem                        | 3426743917723751680    |               | 19.31                | 3838             | U Gem                | 134        | 301 |     |
| J061222.10–594449.3 |                               | 5482510257102758272    |               | 20.31                | 1831             | MCV:                 | 1          | 1   |     |
| J061558.69–515423.9 | DDE 100                       | 5549098884600251776    | 5.0407(6)     | 15.19                | 750              | Z Cam                | 174        | 1   | 1   |
| J061643.22+152411.2 | CZ Ori                        | 3345033985983457920    | 5.254(5)      | 15.82                | 499              | U Gem                | 74         | 86  | 86  |
| J062157.14+404236.1 | ASASSN-18bz                   | 956899025419314816     |               | 19.9                 | 3324             | U Gem                | 325        | 301 |     |
| J062406.13+400743.8 |                               | 956670430081266176     |               | 18.54                | 1728             | NL                   | 301        | 301 |     |
| J062429.71+002105.8 | ASASSN-15cu                   | 3120280997380365824    | 2.429755(4)   | 18.86                | 468              | SU UMa               | 113        | 301 | 301 |
| J062516.28+733439.1 | MU Cam                        | 1114243404258933376    | 4.71942(16)   | 14.84                | 930              | IP                   | 345        | 236 | 8   |
| J062601.53–035522.9 | Gaia17cdo                     | 3116642228070616192    |               | 19.19                | 1184             | DN                   | 334        | 301 |     |
| J062724.39+161329.6 | Gaia18atj                     | 3369335048381292032    | 10.428(3)     |                      |                  | U Gem                | 159        | 159 | 152 |
| J062953.89–033508.4 | IRXS J062954.6-033520         | 3105034928633782400    | 9.12(1)       | 13.53                | 652              | Z Cam                | 279        | 301 | 1   |
| J063047.05+023931.2 | ASASSN-16ow                   | 3124075927403447936    | 2.07(6)*      | 20.57                | 3374             | SU UMa               | 280        | 1   | 31  |
| J063301.12+030333.8 |                               | 3130088774241620608    |               | 18.3                 | 242              | WZ Sge:              | 301        | 301 |     |
| J063304.77+032422.7 | Gaia17ber                     | 3130133544980839680    |               | 19.1                 | 2548             | U Gem                | 245        | 301 |     |
| J063516.63+030313.6 |                               | 3130064176963184896    | 1.4717(2)     | 18.95                | 643              | Polar:               | 301        | 301 | 301 |
| J063654.60+000217.2 | CW Mon                        | 3119646304291839872    | 4.643232(1)   | 16.06                | 325              | U Gem                | 254        | 238 | 89  |
| J063844.17+181611.4 | UV Gem                        | 3371136087085232128    | 2.2464        |                      |                  | SU UMa               | 262        | 1   | 358 |
| J063938.60+055352.7 | V959 Mon                      | 3131126129104233344    | 7.098(13)     | 16.98                | 4038             | Nova                 | 107        | 189 | 197 |
| J064949.95+554140.4 | ASASSN-19an                   | 1000154676144230784    | 1.45(2)*      | 19.36                | 539              | SU UMa               | 93         | 1   | 99  |
| J064950.93–073741.0 | RX J0649.8-0737               | 3099139244207211520    | 4.3988(3)     | 17.08                | 581              | Polar                | 177        | 1   | 1   |
| J065733.66–533422.0 | BMAM-V547                     | 5497677749426668800    | 3.7286(2)     | 14.15                | 1033             | NL                   | 339        | 142 | 142 |
| J070533.80–125004.8 |                               | 3044836838812715264    |               | 18.7                 | 246              | DN                   | 301        | 301 |     |
| J070648.97+032448.3 | MG1 400618                    | 3116059834803771904    | 1.7018(3)     | 17.13                | 206              | Polar                | 206        | 206 | 207 |
| J070816.61–124544.8 | ASASSN-16an                   | 3044908474565329280    |               | 19.16                | 2071             | U Gem                | 271        | 301 |     |
| J072142.29–640050.8 |                               | 5282634371914454912    | 3.6492(3)     | 16.02                | 868              | NL                   | 325        | 1   | 1   |

| SDSS                | Name                          | Gaia EDR3<br>source_id | Period<br>(h) | Gaia EDR3<br>G (mag) | Distance<br>(pc) | Variable<br>Sub-type | References |     |     |
|---------------------|-------------------------------|------------------------|---------------|----------------------|------------------|----------------------|------------|-----|-----|
|                     |                               |                        |               |                      |                  |                      | ID         | Sp  | P   |
| J072304.79+020437.2 | LAMOST J072304.77+020437.4    | 3135760162593729792    | 3.1813(5)     | 15.13                | 1363             | NL                   | 312        | 312 | 1   |
| J073143.87+011714.9 | NSV 3626                      | 3134745107203068928    |               |                      |                  | Z Cam                | 202        | 1   |     |
| J073339.29+212200.8 | CSS 091111:073339+212201      | 865345406593708160     |               | 19.37                | 1961             | U Gem                | 292        | 292 |     |
| J073758.55+205544.6 |                               | 673118544624392576     |               | 19.79                | 974              | SU UMa:              | 362        | 301 |     |
| J073817.74+285519.7 |                               | 878597549661945984     | 5.55521(5)    | 18.46                | 1204             | U Gem                | 297        | 297 | 1   |
| J073835.88+095805.6 | ASASSN-14jk                   | 3149415375454827136    |               | 20.27                | 3185             | U Gem                | 93         | 1   |     |
| J074222.55+172806.7 | MLS 110309:074223+172807      | 671077782322909696     | 2.47465(2)    | 20.04                | 1828             | DN                   | 151        | 352 | 1   |
| J074419.74+325448.2 | CSS 091029:074420+325448      | 881969129052843520     | 0.55:         | 19.9                 |                  | AM CVn               | 292        | 292 | 261 |
| J074859.55+312512.5 |                               | 880821067114616832     | 1.39946616(2) | 18.37                | 542              | SU UMa               | 362        | 282 | 368 |
| J074917.11+365427.9 | MGAB-V3545                    | 919046658301858048     | 1.3401(1)     | 19.17                | 820              | Polar:               | 85         | 85  | 85  |
| J075107.51+300628.3 |                               | 878968875354903040     | 1.3918(3)*    | 19.68                | 1366             | SU UMa               | 362        | 301 | 260 |
| J075116.99+100016.3 |                               | 3150339377539742336    | 1.421(1)      | 18.39                | 459              | SU UMa:              | 362        | 40  | 40  |
| J075233.17+294339.5 |                               | 875941782403757056     | 2.4040(1)     | 18.5                 | 702              | DN                   | 216        | 301 | 1   |
| J075240.45+362823.2 | EU Lyn                        | 918840426857988736     | 2.74(5)       | 20.0                 | 631              | Polar                | 297        | 297 | 163 |
| J075331.98+375800.6 | CSS 100407:075332+375801      | 919213474830239616     | 1.5363(1)     | 19.21                | 1699             | MCV:                 | 98         | 85  | 301 |
| J075450.15+091019.6 | MASTER OT J075450.18+091020.2 | 3147178109809800960    | 1.59(1)*      | 21.01                |                  | SU UMa               | 151        | 1   | 138 |
| J075515.20+060439.3 | ASASSN-15tr                   | 3143760548496292480    |               | 20.16                | 1556             | U Gem:               | 93         | 1   |     |
| J075522.38+040719.3 |                               | 3089187354004319104    |               | 19.55                | 1649             | CV:                  | 1          | 1   |     |
| J075540.64+264618.1 | V516 Gem                      | 874545471356863104     | 1.4883(1)     | 18.74                | 359              | Polar:               | 77         | 301 | 301 |
| J075648.85-124653.9 | ATO J119.2035-12.7816         | 3036063148338139776    | 10.79(4)      | 16.86                | 1546             | U Gem                | 111        | 1   | 1   |
| J075653.12+085831.9 |                               | 3146975005100167296    | 3.2859(6)     | 16.88                | 1070             | NL                   | 187        | 187 | 71  |
| J075655.95+062646.7 |                               | 3144149603814424832    |               | 19.68                | 2056             | MCV:                 | 1          | 1   |     |
| J075939.78+191417.3 |                               | 670122409797824000     | 3.142409(1)   | 17.89                | 1754             | NL                   | 146        | 146 | 323 |
| J080033.86+192416.6 | CRTS J080033.8+192416         | 670132550216853632     | 1.92(1)       | 19.73                | 760              | SU UMa               | 362        | 1   | 158 |
| J080407.93-002216.4 | MGAB-V3549                    | 3083251949718928512    | 1.56166(3)    | 18.72                | 994              | Polar                | 15         | 1   | 1   |
| J080448.88+024853.5 | ASASSN-16ac                   | 3094012943037857792    |               | 20.78                |                  | DN                   | 93         | 1   |     |
| J080534.48+072029.1 |                               | 3097732002461148672    | 5.48906(3)    | 17.88                | 1542             | CV                   | 51         | 51  | 85  |
| J080538.98+354054.9 | CSS 170417:080539+354055      | 906152376204919040     | 5.2069(1)     | 20.69                | 1770             | U Gem                | 190        | 301 | 301 |
| J080727.59-763159.8 | Z Cha                         | 5210507882302442368    | 1.787983      | 15.71                | 120              | SU UMa               | 211        | 131 | 171 |
| J080818.98+005859.8 | ASASSN-15cw                   | 3084580919978268672    | 1.899019(5)   | 17.84                | 368              | DN                   | 93         | 63  | 63  |
| J080837.79-694712.8 | ASASSN-14jd                   | 5269753451459457024    |               | 17.57                | 799              | U Gem                | 93         | 1   |     |
| J080853.73+355053.6 | CSS 080416:080854+355053      | 906214223733883264     |               | 19.98                | 1807             | DN                   | 151        | 25  |     |
| J081210.23+040351.3 | CSS 091017:081210+040352      | 3091578315052482304    | 2.6980565(4)  | 18.69                | 1931             | Polar                | 199        | 327 | 327 |
| J081225.44-711437.2 | ASASSN-15qb                   | 5269367797756084096    |               | 17.81                | 385              | DN                   | 93         | 1   |     |
| J081228.29+623621.9 | SU UMa                        | 1091051096255456384    | 1.833010(1)   | 14.68                | 220              | SU UMa               | 315        | 313 | 313 |
| J081318.41-010326.7 | ASASSN -14ag                  | 3071240270519385856    | 1.4474556(2)  | 15.95                | 181              | SU UMa               | 93         | 63  | 179 |
| J081321.93+452809.2 | FH Lyn                        | 928715626116734976     | 6.937(8)      | 17.64                | 1693             | U Gem                | 160        | 160 | 115 |
| J081931.24+213338.0 | MLS 151206:081931+213338      | 676203568093232512     |               | 19.46                | 2768             | U Gem                | 72         | 125 |     |
| J082236.02+510524.4 | BH Lyn                        | 1028258463932870656    | 3.7410138(3)  | 15.17                | 736              | NL                   | 173        | 157 | 136 |
| J082253.13+231300.6 | SDSS J082253.12+231300.6      | 678153002209054336     |               | 19.8                 | 3077             | CV:                  | 80         | 80  |     |
| J082603.71+113820.8 | CSS 110124:082604+113821      | 601203165542995072     | 1.73(1)*      | 20.32                | 1612             | SU UMa               | 151        | 1   | 138 |
| J082827.50-632958.8 | ASASSN-18aau                  | 5276857366024879872    | 10.7(1)       | 17.38                | 2122             | U Gem                | 93         | 1   | 1   |
| J083619.15+212105.2 | CC Cnc                        | 664787098343076992     | 1.764(2)      | 17.45                | 493              | SU UMa               | 287        | 287 | 257 |



| SDSS                                | Name                     | Gaia EDR3<br>source_id | Period<br>(h)              | Gaia EDR3<br>G (mag) | Distance<br>(pc) | Variable<br>Sub-type    | References |     |     |
|-------------------------------------|--------------------------|------------------------|----------------------------|----------------------|------------------|-------------------------|------------|-----|-----|
|                                     |                          |                        |                            |                      |                  |                         | ID         | Sp  | P   |
| J083642.66+532838.0                 | SW UMa                   | 1030279027003254784    | 1.363560(1)                | 16.61                | 160              | SU UMa                  | 153        | 115 | 358 |
| J083821.98+483802.1                 | EI UMa                   | 1014839031890550912    | 6.43(1)                    | 14.79                | 1120             | IP                      | 173        | 172 | 172 |
| J084054.15+045518.4                 |                          | 582480166148927744     | <a href="#">3.080(1)</a>   |                      |                  | Z Cam                   | 146        | 146 | 1   |
| J084400.09+023919.2                 | V495 Hya                 | 3079207606650040320    | 4.9708(6)                  | 18.42                | 1467             | U Gem                   | 297        | 297 | 301 |
| J084413.66–012808.0                 | CSS 090331:084414-012807 | 3072558340145828864    | 0.53:                      | 20.37                | 2153             | AM CVn                  | 292        | 292 | 91  |
| J084555.07+033929.3                 | V498 Hya                 | 581352651334960512     | 1.4536(14)*                | 20.72                | 1635             | WZ Sge:                 | 358        | 292 | 358 |
| <a href="#">J084708.28+011939.1</a> |                          |                        |                            |                      |                  | <a href="#">AM CVn</a>  | 1          | 1   |     |
| <a href="#">J084735.40+014533.9</a> |                          |                        |                            |                      |                  | <a href="#">CV</a>      | 1          | 1   |     |
| J084740.11–474318.5                 | GDS_J0847401-474318      | 5329462159841324800    |                            | 16.23                | 928              | <a href="#">Polar:</a>  | 181        | 1   |     |
| J085107.39+030834.6                 | CT Hya                   | 581110831791334400     | 1.59612(3)*                | 18.54                | 579              | SU UMa                  | 140        | 297 | 317 |
| J085210.44+783246.7                 |                          | 1137977599693611264    | <a href="#">17.109(1)</a>  | 14.51                | 1053             | <a href="#">NL</a>      | 325        | 1   | 1   |
| J085300.55+020424.2                 | CSS 131207:085301+020425 |                        |                            |                      |                  | WZ Sge:                 | 72         | 85  |     |
| <a href="#">J085550.85–015428.6</a> |                          | 5763945754474388480    |                            |                      | 247              | <a href="#">WZ Sge:</a> | 1          | 1   |     |
| J085603.78+322109.1                 | CSS 100508:085604+322109 | 712763536603376512     | 1.441(5)*                  | 19.87                | 1378             | SU UMa                  | 151        | 85  | 138 |
| J085640.28–040439.7                 | ASASSN-15ds              | 5761140728513144192    |                            | 17.69                | 759              | SU UMa                  | 93         | 1   |     |
| J085909.20+053654.4                 | RX J0859.1+0537          | 583340808875713280     | <a href="#">2.3988(1)</a>  | 18.07                | 440              | Polar                   | 109        | 109 | 1   |
| J090246.54–014201.9                 | ASASSN-15gv              | 5764187028557281280    | 2.04(10):                  | 20.58                | 1734             | SU UMa:                 | 73         | 301 | 301 |
| J090344.25–013326.1                 |                          | 5764195103095781120    |                            | 19.53                | 278              | AM CVn                  | 32         | 301 |     |
| J090403.48+035501.1                 |                          | 579909164365936512     | 1.433358(1)                | 19.31                | 295              | WZ Sge:                 | 165        | 353 | 205 |
| J090756.67+715859.2                 |                          | 1120565454382143104    | <a href="#">3.65597(2)</a> | 15.94                | 762              | <a href="#">NL</a>      | 325        | 1   | 1   |
| J090947.82+110636.4                 |                          | 592059145810439808     |                            | 20.55                | 601              | WZ Sge:                 | 85         | 85  |     |
| J091001.64+164820.0                 |                          | 610980332174389632     | 1.762(4)*                  | 18.77                | 554              | SU UMa                  | 80         | 80  | 138 |
| <a href="#">J091248.24–000721.3</a> |                          | 3842489089752592256    |                            |                      | 995              | <a href="#">CV:</a>     | 1          | 1   |     |
| J091410.72+013732.9                 | ASASSN-16as              | 3843535378146405888    | 6.043(7)                   | 17.69                | 1016             | U Gem                   | 92         | 313 | 313 |
| J091453.59+113401.5                 | CSS 081107:091454+113402 | 593451814725151232     |                            | 20.88                |                  | <a href="#">DN</a>      | 151        | 1   |     |
| J091551.64+090049.2                 | GZ Cnc                   | 590619751945633024     | 2.11(1)                    | 16.0                 | 374              | SU UMa                  | 137        | 137 | 242 |
| <a href="#">J091818.55+043610.0</a> |                          |                        |                            |                      |                  | <a href="#">CV</a>      | 1          | 1   |     |
| J092042.64+001903.2                 | CSS_J092042.6+001903     | 3842392440103842560    | 8.2901(2)                  | 15.3                 | 886              | <a href="#">U Gem</a>   | 289        | 1   | 289 |
| J092534.78+434917.3                 | 2MASS J09253483+4349179  | 817673885243718272     | <a href="#">3.56(1)</a>    | 13.3                 | 642              | <a href="#">NL</a>      | 312        | 312 | 1   |
| J092614.29+010557.4                 |                          | 3844016380122912640    | 1.4723(1)                  | 19.47                | 385              | Polar                   | 250        | 250 | 250 |
| J092620.40+034542.0                 | GUVV J092620.4+034541.8  | 3845719592354419712    |                            | 19.7                 | 933              | SU UMa                  | 233        | 301 |     |
| <a href="#">J092902.86+005334.0</a> |                          |                        |                            |                      |                  | <a href="#">CV:</a>     | 1          | 1   |     |
| J093205.23+034332.4                 | ASASSN-17od              | 3850925956004914816    |                            | 17.75                | 633              | SU UMa:                 | 73         | 301 |     |
| J093214.82+495054.6                 | QS UMa                   | 1018018235403653504    | 10.04097(1)                | 16.47                | 2465             | NL                      | 230        | 146 | 115 |
| J093238.20+010902.5                 |                          | 3841337699215167232    |                            | 19.4                 | 3145             | Polar:                  | 297        | 297 |     |
| J093836.99+071454.6                 | HM Leo                   | 3854288674880283264    | <a href="#">4.4736(2)</a>  | 16.66                | 506              | U Gem                   | 363        | 363 | 1   |
| J094431.71+035805.7                 | VZ Sex                   | 3848210123629587072    | 3.574(3)                   | 16.5                 |                  | IP                      | 297        | 297 | 298 |
| <a href="#">J095312.66–042732.0</a> |                          |                        |                            |                      |                  | <a href="#">AM CVn</a>  | 1          | 1   |     |
| J100243.11–024636.0                 |                          |                        |                            |                      |                  | U Gem                   | 362        | 1   |     |
| J100434.76+662914.9                 | LN UMa                   | 1066429869812792576    | <a href="#">3.3209(6)</a>  | 15.2                 | 975              | NL                      | 143        | 222 | 1   |
| J100515.36+191107.7                 |                          | 626719772406892288     | 1.8592(6)*                 | 18.12                | 340              | SU UMa                  | 80         | 80  | 358 |
| J100700.72+673247.0                 | CH UMa                   | 1067083117158668800    | 8.23642(1)                 | 14.73                | 373              | U Gem                   | 154        | 238 | 335 |
| J102026.51+530432.9                 | KS UMa                   | 851753282506891776     | 1.63(1)                    | 16.81                | 350              | SU UMa                  | 281        | 353 | 53  |

| SDSS                                | Name                          | Gaia EDR3<br>source_id | Period<br>(h)             | Gaia EDR3<br>G (mag) | Distance<br>(pc) | Variable<br>Sub-type | References |     |     |
|-------------------------------------|-------------------------------|------------------------|---------------------------|----------------------|------------------|----------------------|------------|-----|-----|
|                                     |                               |                        |                           |                      |                  |                      | ID         | Sp  | P   |
| <a href="#">J102215.84-035927.8</a> |                               | 3780358883122989184    |                           | 20.61                |                  | DN                   | 1          | 1   |     |
| J102320.27+440509.6                 | NSV 4838                      | 806057025204204032     | 1.63(1)                   | 18.41                | 640              | SU UMa               | 33         | 33  | 267 |
| J103317.24+072118.6                 | CSS 080208:103317+072119      | 3862789892627651840    | <a href="#">1.694(2):</a> | 19.58                | 500              | SU UMa               | 151        | 1   | 1   |
| J103352.90+584654.7                 | DW UMa                        | 855119196836523008     | 3.27855678(2)             | 14.25                | 579              | NL                   | 173        | 26  | 366 |
| J104245.16+371819.9                 |                               | 751777469035821312     | 1.82(4)                   | 19.84                | 507              | Polar                | 85         | 85  | 301 |
| J104818.02+521829.3                 | LY UMa                        | 837035254216960128     | 6.51069(1)                | 14.84                | 310              | NL                   | 266        | 266 | 313 |
| J105656.94+494118.4                 | CY UMa                        | 832942871937909632     | 1.670(1)                  | 17.26                | 307              | SU UMa               | 230        | 33  | 130 |
| J105756.29+092315.0                 | IU Leo                        | 3867599701948235648    | 9.03139(7)                | 15.27                | 748              | U Gem                | 54         | 81  | 298 |
| J110425.55+450313.3                 | AN UMa                        | 782275761222286720     | 1.911407(3)               | 16.56                | 333              | Polar                | 204        | 146 | 115 |
| J112238.73-053949.4                 | MASTER OT J112238.72-053950.1 | 3785685299700323712    |                           | 19.84                | 2606             | DN                   | 132        | 1   |     |
| J112332.02+431717.6                 | CSS 090602:112332+431717      | 783809506927814912     |                           | 19.65                | 1261             | SU UMa               | 151        | 292 |     |
| J112555.65-001639.0                 | 2QZ J112555.7-001639          | 3797083726291435648    | 1.471(3)                  | 19.49                | 426              | SU UMa               | 149        | 149 | 149 |
| J113122.38+432238.7                 | MR UMa                        | 772038105376131456     | 1.518(3)                  | 17.92                | 328              | SU UMa               | 62         | 146 | 267 |
| <a href="#">J113542.62-581515.9</a> |                               | 5336482644697237120    |                           | 19.85                | 3644             | MCV:                 | 1          | 1   |     |
| J114338.55+714120.9                 | DO Dra                        | 1074721664954807040    | 3.968982(2)               | 15.24                | 194              | IP                   | 173        | 173 | 48  |
| J114521.19-042606.2                 | TW Vir                        | 3599772726850899712    | 4.3844(1)                 | 16.61                | 401              | U Gem                | 204        | 204 | 198 |
| J115223.94-673828.2                 | ASASSN-19ob                   | 5235694124616931584    |                           | 14.87                | 1012             | NL                   | 93         | 1   |     |
| J115419.06+575750.8                 |                               | 845441772229861760     |                           | 20.42                | 1144             | ER UMa:              | 85         | 85  |     |
| J120619.85-032838.6                 | CSS 120202:120620-032838      | 3598190937639242624    |                           | 20.18                | 799              | SU UMa               | 151        | 1   |     |
| J121005.31-025544.1                 | 2QZ J121005.3-025543          | 3598332710216846208    |                           | 20.81                |                  | U Gem                | 83         | 83  |     |
| J121913.07+204937.2                 |                               | 3952276665815698560    | 1.3018(1)                 | 19.19                | 274              | WZ Sge               | 187        | 187 | 301 |
| <a href="#">J122321.22-614758.1</a> |                               | 6054895841359359872    |                           | 16.93                | 1762             | NL                   | 1          | 1   |     |
| J122508.13-034721.0                 | MLS 180415:122508-034721      | 3693120336335460736    | <a href="#">1.38(7)</a>   | 20.23                |                  | Polar                | 151        | 1   | 1   |
| J122740.88+513924.8                 |                               | 1571768231438756864    | 1.510810(2)               | 18.74                | 390              | SU UMa               | 146        | 146 | 28  |
| J123813.51-033933.9                 | V406 Vir                      | 3681313024562519552    | 1.34(1)                   | 17.66                | 170              | WZ Sge               | 297        | 297 | 208 |
| <a href="#">J124100.45-593033.4</a> |                               | 6059701669245702400    |                           | 16.2                 | 2324             | NL                   | 1          | 1   |     |
| J124426.25+613514.5                 | V351 UMa                      | 1580508421164776064    | 2.382(3)                  | 18.15                | 676              | DN                   | 353        | 353 | 22  |
| J124823.06-040100.9                 | MLS 140522:124823-040100      | 3681836628319835776    |                           | 20.13                | 1145             | U Gem                | 151        | 1   |     |
| J130030.27+115101.2                 | CSS 080702:130030+115101      | 3737180546103830144    | 1.5041(3)                 | 19.86                | 1128             | SU UMa               | 151        | 51  | 205 |
| J130514.73+582856.2                 |                               | 1578672472969644288    |                           | 19.23                | 3911             | DN                   | 353        | 353 |     |
| J131042.66-042600.6                 | CSS 120313:131043-042600      | 3635932911213401600    |                           | 20.61                | 890              | SU UMa:              | 151        | 1   |     |
| J133200.79-045410.5                 | DDE 139                       | 3633639918368838272    | <a href="#">1.93(1):</a>  | 20.53                | 948              | SU UMa               | 102        | 1   | 1   |
| J133309.18+143706.9                 |                               | 3741755132951336192    | 2.1148(1)                 | 19.55                | 2028             | Polar                | 80         | 80  | 301 |
| J133941.06+484727.6                 | V355 UMa                      | 1558322303741820928    | 1.3754(4)                 | 17.37                | 150              | WZ Sge               | 33         | 33  | 13  |
| J134052.05+151340.9                 | CSS 100531:134052+151341      | 3742038776886730368    | 2.451                     |                      |                  | U Gem                | 151        | 331 | 331 |
| J134309.43+782312.7                 | DDE 75                        | 1715087751051729280    | <a href="#">3.77(50)</a>  | 14.52                | 957              | Z Cam                | 102        | 1   | 1   |
| J135218.95+280917.0                 | CSS 090705:135219+280917      | 1451958950484177280    | <a href="#">5.6845(4)</a> | 20.1                 | 2263             | U Gem                | 292        | 292 | 1   |
| J135642.40+613024.4                 | V427 UMa                      | 1661194359687172480    |                           | 20.47                | 2330             | SU UMa:              | 23         | 301 |     |
| <a href="#">J141436.78+162104.2</a> |                               | 1232239792398460672    |                           | 19.93                | 657              | CV                   | 1          | 1   |     |
| J142833.38+003100.4                 | 2QZ J142833.5+003100          | 3654152780958106880    |                           | 19.57                | 352              | WZ Sge:              | 255        | 1   |     |
| J142953.55+073231.2                 |                               | 1172464842754767488    |                           | 20.23                | 1348             | U Gem                | 362        | 301 |     |
| J143317.77+101122.4                 |                               | 1176468611268115200    | 1.30177630(5)             | 18.55                | 232              | WZ Sge               | 51         | 51  | 28  |
| <a href="#">J143427.17-640303.1</a> |                               | 5853133469166421248    |                           | 16.71                | 2091             | NL                   | 1          | 1   |     |

| SDSS                                | Name                     | Gaia EDR3<br>source_id | Period<br>(h)              | Gaia EDR3<br>G (mag) | Distance<br>(pc) | Variable<br>Sub-type | References |     |     |
|-------------------------------------|--------------------------|------------------------|----------------------------|----------------------|------------------|----------------------|------------|-----|-----|
|                                     |                          |                        |                            |                      |                  |                      | ID         | Sp  | P   |
| J143435.34+334050.2                 | OU Vir                   | 1287753107989718784    | 1.7449                     | 20.03                | 363              | WZ Sge:              | 301        | 301 |     |
| J143500.23–004606.5                 |                          | 3650020648757787008    |                            | 18.29                | 485              | SU UMa               | 295        | 255 | 358 |
| <a href="#">J143558.50+033217.6</a> |                          |                        |                            |                      |                  | DN                   | 1          | 1   |     |
| J143947.62–010606.8                 | LBQS 1437-0053           | 3649832043858197376    | 6.66(6):                   |                      |                  | NL:                  | 286        | 286 | 286 |
| J144609.22+013604.5                 | ZTF J144609.22+013604.7  | 3652272306837720448    | <a href="#">2.8646(2)</a>  | 17.54                | 423              | CV                   | 152        | 1   | 1   |
| J144659.96+025330.1                 |                          | 1157501971264781824    | 4.0(4)                     | 17.81                | 1619             | IP                   | 297        | 297 | 218 |
| <a href="#">J145225.24–042931.9</a> |                          | 6337526851463872256    |                            | 19.93                | 380              | WZ Sge:              | 1          | 1   |     |
| <a href="#">J150218.82+023055.2</a> |                          | 1153877014571472384    | <a href="#">1.50227(2)</a> | 20.0                 | 265              | WZ Sge:              | 1          | 1   | 1   |
| J150240.87+333423.4                 | NZ Boo                   | 1289860214647954816    | 1.413831(1)                | 17.26                | 184              | SU UMa               | 146        | 146 | 85  |
| J151400.10–650536.6                 | EK TrA                   | 5825198967486003072    | 1.5092(3)                  | 16.15                | 151              | SU UMa               | 340        | 185 | 358 |
| J151836.03–054803.6                 | CSS 120330:151836-054803 | 6322873110245396992    |                            | 19.33                | 513              | DN                   | 151        | 1   |     |
| <a href="#">J152020.39–000948.3</a> |                          | 4418752449654921088    |                            |                      | 2018             | NL                   | 1          | 1   |     |
| J152506.86–032655.4                 | 1RXS J152506.9-032647    | 4413778946245759360    | 1.545160(1)                | 16.18                | 239              | Polar                | 151        | 68  | 145 |
| J154336.53+751541.4                 | GSC 04560-02157          | 1703849402186302592    | 6.36862(3)                 | 15.34                | 539              | U Gem                | 78         | 78  | 78  |
| J154544.90+442829.9                 | CSS 110428:154545+442830 | 1396642623570704384    | 1.846(5)*                  |                      |                  | SU UMa               | 151        | 292 | 234 |
| J155331.03+551614.4                 | MQ Dra                   | 1597621426298361216    | 4.392(1)                   |                      |                  | Polar                | 341        | 341 | 341 |
| J160450.19+414328.3                 |                          | 1383342720466698240    |                            | 17.9                 | 4506             | NL                   | 33         | 33  |     |
| J160501.32+203056.4                 |                          | 1205022962601053312    | 1.3598(2):*                |                      |                  | WZ Sge               | 80         | 80  | 234 |
| J160525.27–381212.1                 | ASASSN-21hc              | 5997931385192680064    | 0.5969(5)*                 | 19.45                | 457              | AM CVn               | 93         | 1   | 135 |
| J160809.53+542131.4                 | ELAISN1 MOS15-02         | 1429001113336695168    | 1.4646(5)                  | 19.43                | 1168             | ER UMa               | 275        | 301 | 301 |
| J160811.26–135058.2                 | USNO-A2.0 0750-09453854  | 4341529414413909632    |                            | 18.75                | 206              | WZ Sge:              | 329        | 1   | 1   |
| J161030.19+445900.8                 |                          | 1386167468917461376    |                            |                      |                  | CV                   | 151        | 1   |     |
| J161132.67+784319.4                 |                          | 1707864784291009280    | <a href="#">4.2508(2)</a>  |                      | 2297             | NL:                  | 210        | 210 | 1   |
| J161259.87–161715.6                 | ZTF19aaqrldn             | 6249835546407578496    | <a href="#">3.5421(1)</a>  | 17.54                | 1010             | Polar                | 364        | 1   | 1   |
| J161615.09–425825.4                 | ASASSN-17fj              | 5993200495902148352    | 1.583(1)*                  | 20.62                | 3720             | SU UMa               | 93         | 1   | 29  |
| J161618.69+115104.6                 | PNV J16161867+1151058    | 4457044552705226752    |                            | 20.64                |                  | CV                   | 95         | 1   |     |
| J161707.15–562720.0                 | ASASSN-17db              | 5931342384104003200    |                            | 18.41                | 872              | U Gem                | 93         | 1   |     |
| J161817.28+030936.8                 | BMAM-V636                | 4436157508268272000    |                            | 18.65                | 747              | Polar                | 15         | 1   |     |
| J161853.17+070427.2                 | PS15awk                  | 4438295409847666432    | <a href="#">2.6505(1):</a> | 19.15                | 1171             | Polar:               | 351        | 351 | 1   |
| J161935.78+524631.7                 | DDE 32                   | 1425200578380530048    | 1.675066(5)                | 19.28                | 449              | Polar                | 47         | 47  | 47  |
| J161953.25+031908.8                 | WFI J161953.3+031909     | 4436163967899228416    | 2.3860754(1)               | 18.93                | 1992             | Z Cam                | 11         | 11  | 35  |
| <a href="#">J162008.82+024414.6</a> |                          | 4436081229649799808    |                            | 19.87                | 379              | WZ Sge:              | 1          | 1   |     |
| J162032.33–563519.8                 | BESTII F19_123203        | 5931299709303896576    | 4.430(1)                   | 16.44                | 1290             | U Gem                | 217        | 1   | 217 |
| J162109.00–135307.6                 | CSS 140211:162109-135307 | 4329694756584110592    |                            | 20.31                | 1754             | DN                   | 151        | 1   |     |
| J162433.30–293337.1                 | ASASSN-14hd              | 6038087817564263552    | <a href="#">5.5138(4)</a>  | 17.48                | 574              | U Gem                | 93         | 1   | 1   |
| J162501.76+390926.3                 | V844 Her                 | 1332378466733219456    | 1.3117(1)                  | 17.44                | 304              | SU UMa               | 20         | 33  | 176 |
| J162528.90–552003.6                 | IK Nor                   | 5931832796260621440    |                            | 17.07                | 588              | DN                   | 118        | 1   |     |
| J162806.14+065315.3                 | CSS 110611:162806+065316 | 4439576375257512960    | 1.652(1)*                  | 20.41                | 1838             | SU UMa               | 151        | 1   | 244 |
| J162830.61–571407.3                 | Gaia17cus                | 5928197196659159808    |                            | 19.59                | 4266             | U Gem                | 251        | 1   |     |
| J163120.88+103133.8                 | CSS 080505:163121+103134 | 4458774810347862528    | 1.504(2)                   | 18.39                | 481              | SU UMa               | 151        | 63  | 63  |
| J163353.63–562759.2                 | LR Nor                   | 5928526152484537856    |                            | 18.02                | 1381             | U Gem                | 230        | 1   |     |
| J163447.70–345423.6                 |                          | 6020695124183575552    |                            | 17.36                | 3164             | NL:                  | 30         | 30  |     |
| J163722.20–001957.1                 | V2690 Oph                | 4383291477376259968    | 1.61736(3)                 | 19.99                | 1254             | SU UMa               | 160        | 160 | 228 |

| SDSS                | Name                          | Gaia EDR3<br>source_id | Period<br>(h) | Gaia EDR3<br>G (mag) | Distance<br>(pc) | Variable<br>Sub-type | References |     |     |
|---------------------|-------------------------------|------------------------|---------------|----------------------|------------------|----------------------|------------|-----|-----|
|                     |                               |                        |               |                      |                  |                      | ID         | Sp  | P   |
| J163805.39+083758.3 | V544 Her                      | 4445459754597440000    | 5.320(1):     | 19.0                 | 1668             | U Gem                | 332        | 292 | 1   |
| J164017.89+080823.0 | CSS 090711:164018+080823      | 4445183742818068864    |               | 20.29                | 4583             | U Gem                | 151        | 1   |     |
| J164204.25+151218.1 | CSS 170628:164204+151218      | 4462565475465425664    |               | 20.75                |                  | SU UMa               | 151        | 1   |     |
| J164205.37-655335.8 | ASASSN-20gs                   | 5815733821613451776    |               | 20.07                | 2012             | DN                   | 93         | 1   |     |
| J164248.50+134751.6 |                               | 4461280391188698368    | 1.89(1)       | 17.86                | 531              | SU UMa               | 51         | 51  | 228 |
| J164449.42+195940.1 | V611 Her                      | 4563219790691190912    | 1.53(1)*      | 19.9                 | 1073             | SU UMa               | 97         | 1   | 244 |
| J164653.53+090726.1 | CSS 160705:164654+090726      | 4445723435524824448    |               | 19.29                | 793              | CV:                  | 151        | 1   |     |
| J164654.82+135359.4 | DDE 152                       | 4461484144442112896    |               | 16.41                | 3299             | NL                   | 102        | 1   |     |
| J164925.44+140243.3 | ASASSN-15jd                   | 4461525307402835328    | 1.5595(2)*    | 20.83                | 3009             | WZ Sge               | 93         | 1   | 367 |
| J164950.38+035834.5 | CSS 100707:164950+035835      | 4386357538567811456    | 1.82(3)*      | 18.66                | 414              | SU UMa               | 151        | 1   | 96  |
| J165127.25-131809.2 | SSS 130510:165127-131809      | 4332792802397772672    |               | 19.91                |                  | U Gem                | 72         | 301 |     |
| J165141.45-490712.2 |                               | 5939153486460025472    |               | 16.61                | 1333             | NL:                  | 1          | 1   |     |
| J165242.98+703014.8 | PTFS1116cc                    | 1650169457811634176    | 6.47486(2)    | 17.09                | 1151             | U Gem                | 339        | 1   | 293 |
| J165244.82+333925.5 |                               | 1314596271336013824    | 1.67:         | 20.74                | 3281             | SU UMa               | 33         | 33  | 301 |
| J165859.91-512331.3 |                               | 5936536373909968512    |               | 16.53                | 1670             | NL:                  | 1          | 1   |     |
| J165930.37-125327.2 | V841 Oph                      | 4333061392472253440    | 14.4313(2)    | 13.65                | 815              | Nova                 | 258        | 27  | 27  |
| J170044.63-500505.3 | USNO-B1.0 0399-0591734        | 5938122346376835840    |               | 19.94                | 5460             | CV:                  | 67         | 1   |     |
| J170515.33+724403.3 | MASTER OT J170515.37+724402.5 | 1655084339211334016    |               | 19.41                | 2686             | SU UMa               | 354        | 301 |     |
| J170609.67+143451.6 | CSS 090205:170610+143452      | 4545086473126911360    | 1.397(3)      | 18.11                | 506              | SU UMa               | 151        | 247 | 247 |
| J170655.18-150852.5 | ASASSN-15fe                   | 4139463473867514112    |               | 18.36                | 632              | DN                   | 93         | 1   |     |
| J171226.57-641656.8 |                               | 5817042446598231040    |               | 18.66                | 159              | WZ Sge:              | 1          | 1   |     |
| J171233.50-643342.6 | MASTER OT J171233.67-643342.6 | 5816657136492166784    | 3.84(2):      | 17.82                | 2905             | U Gem:               | 361        | 1   | 1   |
| J171247.71+604602.9 |                               | 1437612007369245696    | 3.9167(1)     | 18.8                 | 687              | CV                   | 160        | 160 | 152 |
| J171658.14-313958.4 | ASASSN-21jw                   | 5980383415813258496    |               | 16.62                | 809              | U Gem                | 93         | 1   | 1   |
| J171752.03-070654.2 | MASTER OT J171752.02-070654.6 | 4360435241974939392    |               | 20.52                | 3089             | U Gem                | 65         | 301 |     |
| J171935.88-410053.6 | IGR J17195-4100               | 5959894875620104064    | 4.005(6)      | 15.24                | 621              | IP                   | 278        | 278 | 69  |
| J171937.17+043123.3 | ASASSN-15kw                   | 4390013139853618560    | 1.422(3)      | 16.93                | 325              | DN                   | 93         | 313 | 82  |
| J172021.48-150928.9 | ASASSN-18jc                   | 4137716620471790208    | 1.598(1)*     | 19.25                | 501              | SU UMa               | 93         | 1   | 259 |
| J172148.84-051713.3 | CSS 120611:172149-051713      | 4362925292215906176    |               | 20.12                | 3942             | U Gem                | 98         | 301 |     |
| J172256.18-261906.8 |                               | 4109836269759904768    | 6.63601(2)    | 17.49                | 944              | CV                   | 1          | 1   | 1   |
| J172515.56+073249.2 | CSS 100706:172516+073249      | 4490114392134401536    |               | 20.77                | 1865             | DN:                  | 151        | 1   |     |
| J172527.50-680822.4 | ASASSN-14is                   | 5811466410809732352    |               | 20.25                | 1255             | U Gem                | 93         | 1   |     |
| J172733.67+130512.4 | CSS 090929:172734+130513      | 4542096415677872640    |               | 19.39                | 3110             | U Gem                | 151        | 247 |     |
| J172805.33+775117.3 |                               | 1705302990918074880    |               | 20.62                | 974              | WZ Sge:              | 301        | 301 |     |
| J172904.97-483742.0 |                               | 5949941928900837760    |               | 19.53                | 831              | CV                   | 1          | 1   |     |
| J172925.15-404335.8 | ASASSN-18hl                   | 5960096262343370240    |               | 19.28                | 7634             | U Gem:               | 93         | 1   |     |
| J172959.01+522947.8 | MGAB-V705                     | 1415247906500831744    | 2.1528(1)     | 18.35                | 542              | Polar                | 336        | 1   | 1   |
| J173008.35+624754.4 |                               | 1440078211950524544    | 1.838(4)      | 16.3                 | 530              | SU UMa               | 160        | 160 | 267 |
| J173021.89-055931.2 | V2731 Oph                     | 4361932643672982272    | 15.421(3)     |                      | 1938             | IP                   | 248        | 248 | 248 |
| J173045.23-421143.3 | MM Sco                        | 5959120892518988160    | 1.445(2)      | 18.59                | 388              | SU UMa               | 124        | 232 | 201 |
| J173408.80-430550.9 | ASASSN-18cs                   | 5958472730368477184    |               | 18.8                 | 333              | SU UMa               | 162        | 1   |     |
| J173634.28-711258.6 | ASASSN-14dk                   | 5803994640884298496    |               | 20.12                | 2464             | DN                   | 93         | 1   |     |
| J173905.58-452714.5 | V728 Sco                      | 5949184223617563136    | 3.32016(4)    | 18.12                | 1077             | CV                   | 322        | 87  | 263 |

| SDSS                                | Name                          | Gaia EDR3<br>source_id | Period<br>(h)               | Gaia EDR3<br>G (mag) | Distance<br>(pc) | Variable<br>Sub-type | References |     |     |
|-------------------------------------|-------------------------------|------------------------|-----------------------------|----------------------|------------------|----------------------|------------|-----|-----|
|                                     |                               |                        |                             |                      |                  |                      | ID         | Sp  | P   |
| J173924.38+050049.7                 | ASASSN-15mk                   | 4473606466292898688    |                             | 20.54                |                  | DN                   | 73         | 301 |     |
| J174045.86+060350.1                 | 4PBC J1740.7+0603             | 4485786821746343680    | 1.6826(50)                  | 15.84                | 232              | Polar:               | 207        | 207 | 207 |
| J174056.31+025831.5                 | MG1 995493                    | 4376325246582929920    | 4.143(3):                   | 17.81                | 928              | U Gem                | 306        | 301 | 301 |
| J174155.61–620817.9                 | MASTER OT J174155.54-620817.1 | 5909844973188085632    |                             | 20.61                |                  | DN                   | 104        | 1   |     |
| J174342.09–553005.7                 | MASTER OT J174342.12-553006.3 | 5921119983898941056    |                             | 20.38                | 6322             | U Gem                | 304        | 1   |     |
| <a href="#">J174345.53–725309.1</a> |                               | 5803741718847252352    |                             | 19.18                | 915              | CV                   | 1          | 1   |     |
| J174714.34+150047.5                 | CSS 080409:174714+150048      | 4500863084668459136    |                             | 19.6                 | 2249             | U Gem                | 127        | 1   |     |
| J174759.87+032859.6                 | ASASSN-15fm                   | 4472400370757130496    | 6.94(3):                    | 20.07                | 957              | IP:                  | 82         | 301 | 82  |
| <a href="#">J174907.74–621227.0</a> |                               | 5911295572625135360    | <a href="#">2.569307(6)</a> |                      | 120              | CV:                  | 1          | 1   | 1   |
| J175505.10+132519.4                 | ZTF18abdjpb0                  | 4499667881166202624    | 1.370570(3)                 | 19.16                | 1114             | Polar                | 364        | 1   | 16  |
| J175545.04–704634.3                 | ASASSN-14fh                   | 5809846898900205440    |                             | 17.81                | 855              | U Gem                | 93         | 1   |     |
| J175622.38+025804.1                 | DDE 155                       | 4469167909646470528    |                             | 19.35                | 3227             | U Gem                | 102        | 1   |     |
| J175951.66–592000.2                 | V437 Pav                      | 5917882261448293120    |                             | 18.65                | 3038             | DN                   | 249        | 1   |     |
| J175957.70+022144.5                 | Gaia17bdz                     | 4468133711592496000    |                             | 20.05                | 938              | SU UMa:              | 17         | 1   |     |
| J180005.86+525632.7                 | ASASSN-13ax                   | 2125514104303018112    | 1.3477(2)*                  | 20.85                | 1853             | WZ Sge               | 277        | 1   | 158 |
| J180035.52+081014.8                 | V2301 Oph                     | 4476137370261520000    | 1.88283                     | 16.61                | 122              | Polar                | 121        | 182 | 182 |
| J180048.99+523234.5                 | CSS 121025:180049+523235      | 2125131710479521408    |                             | 20.0                 | 1161             | SU UMa               | 151        | 1   |     |
| J180245.76+100146.4                 | ASASSN-17lh                   | 4482623075816487168    |                             | 19.34                | 813              | DN                   | 93         | 1   |     |
| J180312.65+114154.5                 | MASTER OT J180312.78+114154.7 | 4495450498157403392    |                             | 20.38                | 1933             | DN                   | 227        | 1   |     |
| J180324.99+114757.1                 | V2104 Oph                     | 4495453590539471488    |                             | 20.48                | 3963             | Nova                 | 43         | 43  |     |
| J180414.38+675412.5                 | EX Dra                        | 2258357545848389888    | 5.038488(2)                 | 14.41                | 239              | U Gem                | 2          | 2   | 231 |
| J180835.15+084829.1                 | MGAB-V361                     | 4481498344142355328    | <a href="#">4.9647(3)</a>   | 18.01                | 1962             | U Gem                | 15         | 1   | 1   |
| J180835.86+101029.6                 | V2779 Oph                     | 4482863941883637632    | 1.68088(3)                  | 16.98                | 291              | Polar                | 61         | 349 | 61  |
| J180845.59+152101.1                 | ASASSN-19wr                   | 4498827815625756416    |                             | 19.58                | 604              | SU UMa               | 93         | 1   |     |
| J181033.82–534946.0                 | ASASSN-15ia                   | 6653381770072822144    | 1.687(1)*                   | 20.46                | 6161             | SU UMa               | 93         | 1   | 326 |
| J181111.75+124301.7                 |                               | 4496951052360182656    |                             | 19.79                | 689              | SU UMa:              | 301        | 301 |     |
| J181244.08–592315.5                 | AS Pav                        | 6635454580877907328    | <a href="#">2.149544(3)</a> | 17.25                | 871              | SU UMa               | 249        | 1   | 1   |
| J181258.29+160247.1                 | MASTER OT J181258.26+160246.8 | 4498803076615421312    |                             | 20.62                | 738              | DN                   | 42         | 1   |     |
| J181407.30+113642.1                 | V849 Oph                      | 4484747641520751872    | 4.146147(4)                 | 18.35                | 4939             | NL                   | 112        | 112 | 191 |
| J181429.83+612334.0                 | HS 1813+6122                  | 2158980729992107776    | 3.54048(2)                  | 15.25                | 812              | NL                   | 240        | 240 | 366 |
| J181647.37+080014.9                 | MGAB-V467                     | 4478239529117464576    |                             | 19.01                | 1358             | U Gem                | 15         | 1   |     |
| <a href="#">J181738.37+042644.3</a> |                               | 4470501789052997504    |                             | 18.24                | 1203             | U Gem                | 1          | 1   |     |
| J181809.14–653136.0                 | Gaia23apm                     | 6437300247422664960    |                             | 19.65                | 972              | CV                   | 291        | 1   |     |
| <a href="#">J181810.72+050958.5</a> |                               | 4470844316992639488    |                             | 19.21                | 159              | SU UMa:              | 1          | 1   |     |
| J181821.01+125350.2                 | MGAB-V242                     | 4484951497852219264    |                             | 19.44                | 8807             | U Gem                | 336        | 1   |     |
| J181904.82–744123.8                 | Gaia16aoh                     | 6414762702890492544    |                             | 19.94                | 1252             | DN                   | 7          | 1   |     |
| J182122.52+614855.2                 | ASASSN-13at                   | 2159834324676298880    | 1.901(5)                    | 19.46                | 764              | SU UMa               | 122        | 40  | 40  |
| J182134.65+020307.1                 | ASASSN-15kd                   | 4276717778105656320    | <a href="#">4.2704(1)</a>   | 16.36                | 577              | U Gem                | 93         | 1   | 1   |
| J182138.61+615904.0                 | ASASSN-14gg                   | 2159842815827966720    | 1.44(3)*                    | 19.78                | 722              | SU UMa               | 209        | 301 | 120 |
| J182205.84+270849.8                 | MASTER OT J182205.85+270849.7 | 4585224931075337216    |                             | 20.66                | 1772             | SU UMa               | 141        | 301 |     |
| J182313.80–604106.1                 | Gaia19azx                     | 6634683406609133568    |                             | 19.48                | 1647             | U Gem                | 103        | 1   |     |
| J182319.26+051857.1                 | Gaia17cbl                     | 4476631738187393536    |                             | 19.67                | 3236             | U Gem                | 36         | 1   |     |
| J182643.55+613816.5                 | MASTER OT J182643.42+613816.2 | 2159773512236202624    | <a href="#">2.06541(5)</a>  | 20.62                | 2118             | SU UMa               | 12         | 1   | 1   |

| SDSS                                | Name                          | Gaia EDR3<br>source_id | Period<br>(h)               | Gaia EDR3<br>G (mag) | Distance<br>(pc) | Variable<br>Sub-type | References |     |     |
|-------------------------------------|-------------------------------|------------------------|-----------------------------|----------------------|------------------|----------------------|------------|-----|-----|
|                                     |                               |                        |                             |                      |                  |                      | ID         | Sp  | P   |
| <a href="#">J182707.63–520430.0</a> |                               | 6653973655219987328    |                             | 20.48                | 2730             | CV:                  | 1          | 1   |     |
| J183014.15–671032.9                 | ASASSN-17lw                   | 6436264958441648256    |                             | 20.15                | 515              | DN                   | 93         | 1   |     |
| J183052.72+265514.8                 | MGAB-V733                     | 4585376839774011520    |                             | 18.79                | 1175             | SU UMa               | 336        | 301 |     |
| J183144.55+651130.2                 | RX J1831.7+6511               | 2256734632327338496    | <a href="#">3.999660(1)</a> | 16.37                | 853              | Z Cam                | 14         | 14  | 1   |
| J183211.36+615505.9                 | ASASSN-13ah                   | 2159698023890909184    | 1.5874(3)*                  | 20.47                | 960              | SU UMa               | 288        | 288 | 319 |
| J183228.19+101654.1                 | MGAB-V1268                    | 4480616299611285888    | 3.928318(3)                 | 15.92                | 1042             | NL                   | 336        | 1   | 336 |
| J183442.34–514858.7                 | ASASSN-21ij                   | 6655259839011716352    |                             | 19.0                 | 2281             | DN                   | 93         | 1   |     |
| J183722.86–571407.2                 | ASASSN-14jj                   | 6637569010457325952    |                             | 19.33                | 1091             | DN                   | 151        | 1   |     |
| J183840.12+092222.5                 | V651 Oph                      | 4479524171021295744    |                             | 18.29                | 2216             | U Gem                | 309        | 1   |     |
| J184127.11+053821.9                 | 2MASS J18412712+0538217       | 4285476071111900928    | <a href="#">7.6184(2)</a>   | 17.8                 | 1516             | IP                   | 84         | 1   | 1   |
| J184658.80+553829.0                 | MT Dra                        | 2147082017019347968    | 2.145286(3)                 | 17.53                | 499              | Polar                | 264        | 264 | 355 |
| J185306.11–515722.1                 | ASASSN-14fm                   | 6651781950586156288    |                             | 18.87                | 1221             | U Gem                | 93         | 1   |     |
| J185333.52+223559.1                 | Gaia17aqz                     | 4531464383068467456    | <a href="#">8.617(1)</a>    | 18.38                | 2859             | U Gem                | 346        | 1   | 1   |
| J185720.40+713118.7                 | V416 Dra                      | 2262915708740112000    | 4.53862(4)                  | 16.23                | 595              | U Gem                | 76         | 76  | 76  |
| J185721.58+131429.1                 | V446 Her                      | 4506083222318688000    | 4.97                        | 16.62                | 1253             | U Gem                | 56         | 337 | 337 |
| J190005.28–493034.6                 | ASASSN-14fz                   | 6661251730703015168    | 1.873(1)*                   | 19.83                | 1629             | SU UMa               | 93         | 1   | 319 |
| J190121.32–622804.4                 | ASASSN-15kt                   | 6439687458962887040    |                             | 19.75                | 1341             | SU UMa               | 93         | 1   |     |
| J190243.24–483406.0                 | ASASSN-18ik                   | 6661371817991995904    |                             | 19.67                | 320              | SU UMa               | 93         | 1   |     |
| J190342.14+534745.8                 | ASASSN-15fv                   | 2134633793047290368    | 1.6(1)*                     | 18.44                | 877              | SU UMa               | 93         | 1   | 29  |
| <a href="#">J190508.92–130608.6</a> |                               | 4197744908775449856    |                             | 18.47                | 966              | DN                   | 1          | 1   |     |
| J190531.87–534944.4                 | ASASSN-22fs                   | 6644349801742495488    | <a href="#">3.2394(1):</a>  | 18.52                | 1252             | U Gem                | 93         | 1   | 1   |
| <a href="#">J190625.62–111156.8</a> |                               | 4199144823283065728    | <a href="#">3.8250(2)</a>   | 16.56                | 1927             | NL                   | 1          | 1   | 1   |
| <a href="#">J190645.39–131314.2</a> |                               | 4197686978265668224    |                             | 17.11                | 727              | CV:                  | 1          | 1   |     |
| J190651.05–114103.3                 | Gaia21ban                     | 4199068102300166528    | <a href="#">3.96(1):</a>    | 17.59                | 3284             | NL                   | 128        | 1   | 1   |
| J190706.25+690844.6                 | EP Dra                        | 2262055164796424576    | 1.743750(4)                 | 18.05                | 379              | Polar                | 116        | 116 | 116 |
| J190708.20–123552.9                 | ZTF18abdlifh                  | 4197860387542088192    |                             | 16.27                | 1233             | NL                   | 364        | 1   |     |
| J190732.76+525828.5                 | CG Dra                        | 2134394786705862272    | 4.527(1)                    | 16.68                |                  | U Gem                | 212        | 213 | 3   |
| <a href="#">J190739.31–124117.5</a> | ZTFJ190739.31-124117.3        | 4197811119993908864    | <a href="#">3.4437(1)</a>   |                      |                  | NL                   | 1          | 1   | 1   |
| J190811.74–634331.2                 | ASASSN-15mo                   | 6438589085504526208    |                             | 20.15                | 1920             | DN                   | 93         | 1   |     |
| J191306.79+013423.2                 | V1419 Aql                     | 4267751638733390592    |                             | 20.32                | 4329             | Nova                 | 308        | 18  |     |
| J191339.74–614257.0                 | MASTER OT J191339.65-614257.6 | 6439792977720310656    |                             | 19.08                |                  | DN                   | 170        | 1   |     |
| J191343.58–141831.6                 | MGAB-V390                     | 4185395159812049536    | <a href="#">3.72827(2)</a>  | 17.13                | 530              | U Gem                | 336        | 1   | 1   |
| J191421.38–135026.9                 | ZTF18abssftk                  | 4185448206933655424    | <a href="#">5.14102(6)</a>  | 19.11                | 2540             | IP                   | 364        | 1   | 1   |
| J191534.92–620318.5                 | MASTER OT J191535.00-620318.7 | 6439019990983066112    |                             | 20.24                | 846              | DN                   | 270        | 1   |     |
| J191609.69–623551.7                 | V344 Pav                      | 6438943162609124224    | 1.9170(8)                   |                      |                  | SU UMa               | 79         | 232 | 138 |
| <a href="#">J191630.00–065204.4</a> |                               | 4204933683282572288    |                             | 16.9                 | 2092             | NL                   | 1          | 1   |     |
| <a href="#">J191705.21–095144.8</a> |                               | 4200886076037166720    |                             | 18.77                | 236              | AM CVn               | 1          | 1   |     |
| J191713.68+014321.7                 | V356 Aql                      | 4264846415484216576    | 10.2361(1)                  | 18.2                 | 3542             | Nova                 | 24         | 220 | 168 |
| J192002.30–105446.5                 | Gaia19fhp                     | 4199824733785703040    |                             | 17.66                | 2052             | NL                   | 88         | 1   |     |
| J192241.96+524359.0                 | V1113 Cyg                     | 2139385126386829824    | 1.897(1)*                   | 19.07                | 891              | SU UMa               | 212        | 1   | 158 |
| J192305.36+045719.7                 | V1494 Aql                     | 4292840226362457088    | 3.230731(5)                 | 17.43                | 2102             | Nova                 | 299        | 195 | 294 |
| J192321.24+022926.2                 | V1370 Aql                     | 4288898099224201856    |                             | 18.2                 | 2698             | Nova                 | 117        | 220 |     |
| J192336.67–514444.0                 | ASASSN-14ga                   | 6644989197816347776    | 3.8842(1):                  | 18.82                | 613              | U gem:               | 174        | 1   |     |



| SDSS                | Name                          | Gaia EDR3<br>source_id | Period<br>(h) | Gaia EDR3<br>G (mag) | Distance<br>(pc) | Variable<br>Sub-type | References |     |     |
|---------------------|-------------------------------|------------------------|---------------|----------------------|------------------|----------------------|------------|-----|-----|
|                     |                               |                        |               |                      |                  |                      | ID         | Sp  | P   |
| J192444.60+041446.6 | V1229 Aql                     | 4292552738416030208    |               | 19.99                | 5719             | Nova                 | 41         | 156 |     |
| J192513.82–521137.3 | MASTER OT J192513.88-521137.6 | 6646275149680411136    |               | 18.74                | 1132             | DN                   | 194        | 1   |     |
| J192554.81–461903.5 | Gaia16akr                     | 6663284766361627648    |               | 18.45                | 2840             | Z Cam                | 7          | 1   |     |
| J192609.70+611312.7 | ZTF J192609.69+611312.7       | 2240062496996573952    | 9.45158(2)    | 17.24                | 1148             | U Gem                | 152        | 1   | 152 |
| J192610.82–101530.6 | DH Aql                        | 4200218019655998720    | 1.86(1)*      | 17.96                | 296              | SU UMa               | 175        | 1   | 358 |
| J192632.51–011612.0 | Gaia19eop                     | 4215167834436009984    |               | 18.39                | 790              | DN                   | 46         | 1   |     |
| J192634.45+073613.8 | V368 Aql                      | 4295580518601261696    | 16.572223(2)  | 15.73                | 2479             | Nova                 | 305        | 1   | 338 |
| J192710.18–484752.7 | ASASSN-14gq                   | 6659092053645754496    | 1.73(5)*      | 19.34                | 525              | SU UMa               | 174        | 1   | 34  |
| J192711.75+541750.4 | V2176 Cyg                     | 2139968318524093056    | 1.34973(3)*   | 20.29                | 595              | WZ Sge               | 302        | 302 | 358 |
| J192725.39+022303.3 | V1233 Aql                     | 4288751962934103808    |               | 18.43                | 1356             | U Gem                | 281        | 232 |     |
| J192739.29+020013.8 | MASTER OT J192739.31+020014.3 | 4288703653143472896    |               | 19.15                | 1525             | U Gem                | 273        | 1   |     |
| J192830.04–741053.1 | Gaia19efo                     | 6415545035475037312    | 5.991(3)      | 17.84                | 894              | U Gem                | 178        | 1   | 1   |
| J192832.32–500134.9 | V379 Tel                      | 6658737220627065984    | 1.68373(1)    | 16.19                | 129              | Polar                | 265        | 1   | 1   |
| J192914.76+202759.5 | NQ Vul                        | 2017742684676480896    | 3.516(2)      | 17.29                | 1170             | Nova                 | 274        | 274 | 148 |
| J192927.83+202035.0 | 1RXS J192926.6+202038         | 2017736641707652608    | 3.89(3)       | 17.58                | 567              | U Gem                | 330        | 313 | 313 |
| J192933.11–560343.0 |                               | 6640165468504197120    | 1.542(2)      | 17.33                | 376              | Polar                | 1          | 1   | 1   |
| J193025.79–483052.4 |                               | 6659112459034776192    | 2.29126(5):   | 19.32                | 780              | Polar                | 1          | 1   | 1   |
| J193149.51+094939.4 | Gaia16asd                     | 4302469646138706048    |               | 19.82                | 4686             | U Gem                | 7          | 1   |     |
| J193244.66+003559.9 |                               | 4287473746301764224    | 3.6327(1)     | 18.07                | 2593             | NL                   | 1          | 1   | 1   |
| J193423.17+020252.7 |                               | 4288094214457507968    | 3.6370(1):    | 17.54                | 1731             | NL                   | 1          | 1   | 1   |
| J193430.49+020110.3 | ASASSN-19sg                   | 4288093870860070272    | 1.932954(1)   | 18.69                | 395              | SU UMa               | 93         | 1   | 49  |
| J193436.19+510742.1 | V2289 Cyg                     | 2136026049644724864    | 3.41(5)       | 17.94                | 1662             | ER UMa               | 188        | 1   | 1   |
| J193436.97+100213.3 | Gaia17cuh                     | 4302558775291059840    |               | 18.72                | 1717             | U Gem                | 276        | 268 |     |
| J193504.85–574934.9 |                               | 6446867338612443264    |               | 19.6                 | 1621             | U Gem                | 1          | 1   |     |
| J193511.46–531745.8 | CRTS J193511.4-531746         | 6645220099552944000    | 7.96(5):      | 18.98                | 4534             | U Gem                | 98         | 1   | 1   |
| J193628.84–551642.2 |                               | 6641724713432985216    |               | 18.9                 | 310              | DN                   | 1          | 1   |     |
| J193709.85+023600.9 | V1141 Aql                     | 4288234509582097664    | 1.5110(5)*    | 19.18                | 455              | SU UMa               | 118        | 232 | 358 |
| J193835.89–461257.8 | QS Tel                        | 6684490840966796928    | 2.3325(8)     | 16.81                | 186              | Polar                | 75         | 75  | 75  |
| J194124.99+152254.2 | 2MASS J19412506+1522553       | 4318508939464901760    | 1.55650(1)    | 16.96                | 215              | Polar                | 193        | 1   | 152 |
| J194139.92+214557.8 | FY Vul                        | 1826189758928713216    | 4.5758(3)     | 14.38                | 572              | Z Cam                | 118        | 365 | 1   |
| J194255.82–672725.6 | ASASSN-16ku                   | 6427054486972835584    |               | 19.02                | 531              | DN                   | 93         | 1   |     |
| J194309.99+093227.9 | ASASSN-15qv                   | 4301862848814908160    |               | 19.35                | 2710             | U Gem                | 93         | 1   |     |
| J194829.02–562939.5 | ASASSN-15in                   | 6448558353136107776    |               | 18.25                | 839              | DN                   | 93         | 1   |     |
| J194906.45+774423.1 | AB Dra                        | 2291308397504739968    | 3.647(4)      | 14.47                | 396              | Z Cam                | 4          | 45  | 45  |
| J194910.48+583159.4 | V542 Cyg                      | 2235768113813831936    | 4.3518(2)     | 17.27                | 1482             | U Gem                | 37         | 298 | 1   |
| J194947.62+031304.8 | MGAB-V300                     | 4242116898789536640    | 1.563:        | 19.01                | 497              | SU UMa               | 336        | 1   | 1   |
| J195039.55+055619.9 | ASASSN-15qr                   | 4296770769961336448    |               | 18.86                | 1132             | SU UMa:              | 93         | 1   |     |
| J195227.99+082846.9 | V500 Aql                      | 4298546829138834304    | 3.48622(2)    | 19.0                 | 1904             | Nova                 | 223        | 220 | 168 |
| J195306.68+125900.8 | PQ Aql                        | 4304999622372178048    | 5.9220(2)     | 17.25                | 1388             | U Gem                | 342        | 298 | 298 |
| J195436.76+322155.1 | EY Cyg                        | 2034238902485581824    | 11.023800(3)  | 14.34                | 628              | U Gem                | 105        | 324 | 324 |
| J195512.47+004536.3 | 2MASS J19551247+0045365       | 4240284979281473920    | 1.35549(3)    | 15.9                 | 165              | Polar                | 129        | 129 | 1   |
| J195814.47+323241.9 | V2306 Cyg                     | 2034071055160353792    | 4.37149(2)    | 15.69                | 1252             | IP                   | 59         | 313 | 313 |
| J195837.08+164128.4 | AW Sge                        | 1820137772050526464    | 1.788(5)*     | 19.29                | 604              | SU UMa               | 118        | 301 | 272 |



| SDSS                                | Name                          | Gaia EDR3<br>source_id | Period<br>(h)               | Gaia EDR3<br>G (mag) | Distance<br>(pc) | Variable<br>Sub-type | References |     |     |
|-------------------------------------|-------------------------------|------------------------|-----------------------------|----------------------|------------------|----------------------|------------|-----|-----|
|                                     |                               |                        |                             |                      |                  |                      | ID         | Sp  | P   |
| <a href="#">J195938.44-551902.4</a> |                               | 6449054649493107456    |                             | 17.76                | 1758             | NL:                  | 1          | 1   |     |
| <a href="#">J195939.71+655440.9</a> |                               | 2248147377795686528    | <a href="#">7.8307(8)</a>   | 17.18                | 3509             | NL                   | 1          | 1   | 1   |
| J200318.50+170251.5                 | RZ Sge                        | 1820209309009288960    | 1.6387(5)                   | 18.29                |                  | SU UMa               | 118        | 118 | 53  |
| J200504.93+322122.5                 | V550 Cyg                      | 2031052139815189120    | 1.660(6)*                   |                      |                  | SU UMa               | 196        | 1   | 358 |
| <a href="#">J200512.34-561255.4</a> |                               | 6448008532897572736    |                             | 19.22                | 1294             | CV:                  | 1          | 1   |     |
| J200611.52+334237.5                 | V1363 Cyg                     | 2058291887543939968    | <a href="#">9.586(1)</a>    | 16.28                | 1641             | U Gem                | 256        | 126 | 1   |
| J200622.88+031935.3                 | MASTER OT J200622.89+031935.3 | 4247062678194630528    |                             | 20.22                | 1148             | SU UMa:              | 237        | 1   |     |
| J200703.00+051927.3                 | MNIC V88                      | 4247969152508516352    |                             | 17.61                | 1228             | U Gem                | 38         | 1   |     |
| <a href="#">J200729.55+625047.6</a> | ZTF J200729.55+625047.6       | 2244014927765357440    | <a href="#">5.610679(1)</a> | 17.42                | 754              | MCV:                 | 1          | 1   | 1   |
| J200754.82+032738.0                 | MGAB-V903                     | 4247077242421541760    |                             | 18.77                | 645              | U Gem                | 336        | 1   |     |
| J200934.41+550525.7                 |                               | 2185841249306525696    |                             | 16.52                | 1707             | NL                   | 307        | 301 |     |
| J200946.47+042232.6                 | USNO-B1.0 0943-0510775        | 4247567006133149824    |                             | 19.71                | 1985             | SU UMa:              | 364        | 1   |     |
| J201116.80+600428.1                 | Romanov V48                   | 2236896418906579072    | 2.45548(8)                  | 17.3                 | 1423             | IP                   | 359        | 1   | 359 |
| J201135.94+025435.1                 | MG1 1818424                   | 4243983805113737472    |                             | 17.19                | 2493             | IP:                  | 306        | 1   |     |
| <a href="#">J201234.82-550304.4</a> |                               | 6472180471400079360    | <a href="#">4.43(1):</a>    | 19.95                | 3042             | U Gem:               | 1          | 1   | 1   |
| J201403.80-540624.9                 | SSS 110626:201404-540625      | 6473004898964045312    |                             | 19.92                | 1237             | DN                   | 151        | 1   |     |
| J201439.78-093715.2                 | ASASSN-14hy                   | 4191349732517052032    |                             | 20.65                | 6068             | DN                   | 151        | 1   |     |
| J202206.39-565101.7                 | ASASSN-14kx                   | 6468755698837823488    | <a href="#">5.4895(6)</a>   | 18.73                | 863              | U Gem                | 93         | 1   | 1   |
| J202300.38+063142.3                 | LAMOST J202300.37+063142.4    | 4249755657041989376    |                             |                      | 1924             | NL                   | 312        | 312 |     |
| <a href="#">J202310.39+643244.0</a> |                               | 2244642542744444928    | <a href="#">3.680630(1)</a> | 17.28                | 2101             | NL                   | 1          | 1   | 1   |
| J202422.01-083744.3                 | ASASSN-16fk                   | 6906004530876435712    |                             | 19.79                | 2060             | DN                   | 93         | 1   |     |
| J202543.97-582334.2                 | Gaia19cho                     | 6467622480308296448    | <a href="#">5.312(3)</a>    | 16.34                | 849              | U Gem                | 357        | 1   | 1   |
| J202640.97+045901.2                 | ZTF18abtvjuf                  | 4246335587467254912    | <a href="#">3.9992(4)</a>   | 18.79                | 947              | Polar                | 364        | 1   | 1   |
| J202642.06-572154.5                 | ASASSN-15en                   | 6468483805933681920    |                             | 20.33                | 1110             | SU UMa:              | 93         | 1   |     |
| J202812.47+414836.3                 | V2467 Cyg                     | 2068080976989664768    | 3.83(1)                     | 18.04                | 1847             | IP:                  | 300        | 321 | 70  |
| J202857.08-061803.5                 | CSS 110621:202857-061803      | 4217782168142736384    |                             | 19.88                | 2141             | SU UMa               | 151        | 1   |     |
| J203134.50+030422.0                 | MASTER OT J203134.48+030423.4 | 4232789947811070080    |                             | 19.24                | 1602             | SU UMa               | 348        | 1   |     |
| J203137.56-000512.2                 | V1901 Aql                     | 4229582917206160896    | 2.03544(5)                  |                      |                  | Polar                | 90         | 90  | 285 |
| <a href="#">J203256.81-565951.8</a> |                               | 6468131618614808832    |                             | 19.45                | 288              | WZ Sge:              | 1          | 1   |     |
| J203337.17-563345.4                 | TT Ind                        | 6468246487517124736    | <a href="#">4.876360(1)</a> | 16.63                | 642              | U Gem                | 314        | 131 | 1   |
| J203501.48-001946.3                 | ZTF18abssrbs                  | 4229597343999338880    |                             | 18.4                 | 966              | DN                   | 139        | 1   |     |
| J203529.78+063652.7                 | MASTER OT J203529.80+063652.8 | 1747913601981951872    |                             | 20.08                | 3115             | U Gem                | 194        | 1   |     |
| J204247.17-604524.2                 | SSS 110526:204247-604523      | 6454201807020662016    |                             | 19.1                 | 2722             | NL:                  | 151        | 44  |     |
| J204448.92-045928.9                 | V485 Aqr                      | 6914363228723335296    | 40.3(4)                     | 16.4                 | 1948             | U Gem:               | 297        | 343 | 343 |
| J204522.73-011004.5                 | CSS 110930:204523-011004      | 4226992708327722752    |                             | 20.57                | 2348             | DN                   | 151        | 1   |     |
| J204638.68+603802.9                 | V713 Cep                      | 2194206707428148480    | 2.0500424(1)                | 18.35                | 319              | SU UMa               | 57         | 301 | 110 |
| J204643.26-000630.2                 |                               | 4227947904759422976    |                             | 17.73                | 4366             | NL                   | 151        | 32  |     |
| J204720.74+000007.8                 |                               | 4227956460334694272    |                             | 19.89                | 824              | DN                   | 353        | 353 |     |
| J204817.87-061045.3                 |                               | 6913162042334862720    | 1.4543(1)                   | 19.68                | 565              | WZ Sge:              | 297        | 297 | 101 |
| J204827.92+005008.9                 |                               | 4228442478834563712    | 4.2(1)                      | 18.26                | 612              | PREP                 | 146        | 146 | 58  |
| J205110.37+044842.1                 | MASTER OT J205110.36+044842.2 | 1734813603834406144    | 1.9370(1)*                  | 19.34                | 790              | SU UMa               | 328        | 1   | 29  |
| J205212.78+441926.1                 | V751 Cyg                      | 2162954949132840192    | 3.468(3)                    | 14.27                | 748              | NL                   | 106        | 296 | 296 |
| J205227.38+034355.2                 | MASTER OT J205227.38+034355.1 | 1734093874691078144    |                             | 20.61                | 2789             | DN                   | 21         | 1   |     |

| SDSS                | Name                      | Gaia EDR3<br>source_id | Period<br>(h) | Gaia EDR3<br>G (mag) | Distance<br>(pc) | Variable<br>Sub-type | References |     |     |
|---------------------|---------------------------|------------------------|---------------|----------------------|------------------|----------------------|------------|-----|-----|
|                     |                           |                        |               |                      |                  |                      | ID         | Sp  | P   |
| J205305.37+591732.2 | ASASSN-15rz               | 2193827788233092096    | 4.99(4)       | 18.11                | 891              | U Gem                | 93         | 1   | 313 |
| J205423.75+601706.8 | V962 Cep                  | 2194035978188297728    |               | 19.28                | 3095             | Nova                 | 183        | 301 |     |
| J205705.32–072426.1 | Gaia17avi                 | 6909816159737233024    |               | 20.12                | 889              | DN                   | 283        | 1   |     |
| J205914.87–061220.6 | QT Aqr                    | 6910341691929801856    | 1.791(1)      | 18.95                | 1123             | SU UMa               | 297        | 297 | 333 |
| J205931.86–070516.9 |                           | 6909840044045178624    |               | 20.6                 |                  | SU UMa:              | 362        | 1   |     |
| J210306.63+661032.5 | FX Cep                    | 2221753321994545920    |               |                      |                  | U Gem                | 9          | 10  |     |
| J210404.68+463113.4 | V3101 Cyg                 | 2163612727665972096    | 1.284(7)      | 17.7                 | 108              | WZ Sge               | 119        | 108 | 108 |
| J210720.93–022145.9 |                           | 6916066196140198784    |               | 18.61                | 220              | WZ Sge:              | 347        | 1   |     |
| J211312.23–590715.2 |                           | 6453406580942148608    |               | 20.1                 | 660              | SU UMa:              | 151        | 1   |     |
| J211508.00+015715.1 | ASASSN-14dg               | 2692129481599420160    |               | 19.49                | 946              | SU UMa:              | 93         | 1   |     |
| J211541.12–584054.6 | CD Ind                    | 6453536224527716224    | 1.847(2)      | 17.29                | 235              | Polar                | 310        | 310 | 310 |
| J211936.94+033211.6 | CSS 150520:211937+033212  | 2692906015980924544    | 2.37223(1)    | 19.24                | 796              | CV                   | 72         | 85  | 85  |
| J212114.67–622749.7 |                           | 6451474227909044224    |               | 17.03                | 4072             | NL                   | 1          | 1   |     |
| J212521.76–102628.3 | CSS 080927:212522-102627  | 6892469405297825280    | 1.898(3)*     | 20.29                | 1863             | SU UMa               | 151        | 1   | 319 |
| J212654.54–012054.3 | CRTS J212654.5-012054     | 2686013551247649152    |               | 19.06                | 1676             | Polar                | 98         | 98  |     |
| J213024.64–025917.7 | VZ Aqr                    | 2684755714241156736    | 3.85          | 17.49                | 598              | U Gem                | 94         | 298 | 298 |
| J213343.63+510724.6 | 1RXS J213344.1+510725     | 2171623670612602496    | 7.13837(7)    | 15.03                | 1371             | IP                   | 311        | 137 | 298 |
| J213432.34–012040.5 | CSS 081120:213432-012040  | 2686614060690086016    |               | 18.83                |                  | U Gem                | 98         | 301 |     |
| J213559.33+052700.6 | HS 2133+0513              | 2699396467479492480    | 3.29(2)       | 16.18                | 1256             | Z Cam                | 32         | 32  | 184 |
| J214804.43+080950.3 | CSS 080505:214804+080951  | 2701764742511777280    |               | 20.64                |                  | DN                   | 151        | 1   |     |
| J215637.24–632655.5 | SSS 101124:215637-632655  | 6402626839000977408    | 1.573377(1)   | 18.63                | 630              | DN                   | 151        | 1   | 1   |
| J220542.33+033917.1 | ASASSN-17jb               | 2683923998122264832    |               | 20.31                | 2064             | SU UMa:              | 93         | 1   |     |
| J220630.83–524419.8 | DDE 99                    | 6509768960023763584    | 3.9091(2)     |                      |                  | U Gem                | 102        | 1   | 1   |
| J220807.49+021618.8 | HS 2205+0201              | 2682826238837632384    | 5.398(1)      | 16.22                | 3017             | U Gem                | 151        | 1   | 1   |
| J221541.08+553701.3 | CP Lac                    | 2006109065688505472    | 3.48343(2)    | 15.66                | 1127             | Nova                 | 192        | 27  | 27  |
| J221552.06–613545.1 |                           | 6406243514998464640    |               | 20.24                | 3132             | MCV:                 | 1          | 1   |     |
| J221832.75+192520.2 | Swift J2218.5+1925        | 1777232423131443840    | 2.159(24)     | 17.31                | 240              | Polar                | 147        | 50  | 50  |
| J221900.24+201831.2 |                           | 177846868222798080     | 3.36(1)       | 18.23                | 821              | DN                   | 85         | 85  | 85  |
| J222117.33+194817.6 |                           | 1777640754262037248    |               | 18.77                | 708              | DN                   | 73         | 301 |     |
| J224813.46+640023.1 |                           | 2208306092930237440    |               |                      | 184              | Polar                | 1          | 1   |     |
| J225040.37+632837.3 | GD 552                    | 2208124536065383424    | 1.7122(1)     | 16.42                | 80               | WZ Sge               | 64         | 290 | 290 |
| J225608.49+595430.2 | 2MASS J22560844+5954299   | 2014349389931360768    | 5.486535(1)   | 14.5                 | 478              | NL                   | 360        | 214 | 214 |
| J230346.67+531714.9 | V425 Cas                  | 1996248233085177472    | 3.590(3)      | 14.48                | 908              | NL                   | 246        | 238 | 235 |
| J230538.41+652158.8 | IPHAS J230538.39+652158.7 | 2208852614629148800    | 1.685(7)      | 18.9                 | 593              | SU UMa               | 320        | 40  | 40  |
| J233737.44–604358.2 | Gaia21ebk                 | 6488727296765507712    |               | 20.57                | 1359             | DN                   | 200        | 1   |     |
| J234440.54–001206.1 | MLS 100904:234441-001206  | 2642699218384434432    | 1.8411(7)*    | 20.07                | 668              | SU UMa               | 72         | 292 | 317 |
| J234955.19–605417.1 | ASASSN-14hl               | 6488289892999985280    |               | 19.85                | 806              | SU UMa               | 93         | 1   |     |

References: 1 This work, 2 Barwig et al. (1994), 3 Shears et al. (2008b), 4 Howarth (1978a), 5 Delgado et al. (2019d), 6 Stobie et al. (1995), 7 Delgado et al. (2016), 8 Kozhevnikov (2016), 9 Downes et al. (1997), 10 Liu et al. (1999), 11 Rau et al. (2007), 12 Malkova et al. (2016), 13 Gänsicke et al. (2006), 14 Pretorius et al. (2007), 15 Masci et al. (2019), 16 vsnet-chat 9272, 17 Delgado et al. (2017f), 18 Kamath et al. (1997), 19 Halpern & Mirabal (2006), 20 Antipin (1996), 21 Shumkov et al. (2014), 22 Dillon et al. (2008), 23 Stanek et al. (2013a), 24 Parenago (1949), 25 Wright et al. (2012), 26 Araujo-Betancor et al. (2003b), 27 Peters & Thorstensen (2006), 28 Littlefair et al. (2008), 29 Kato et al. (2020), 30 Pretorius & Knigge (2008a), 31 vsnet-alert 20483, 32 Carter et al. (2013), 33 Szkody et al. (2005), 34 Kato et al. (2015), 35 Kato (2022), 36 Delgado et al. (2017h), 37 Goetz & Wenzel (1956), 38 Hodgkin et al.

(2020a), 39 Jablonski & Cieslinski (1992), 40 Thorstensen (2020), 41 Geisel et al. (1970), 42 Balanutsa et al. (2016c), 43 Osawa & Kuwano (1976), 44 Oliveira et al. (2017), 45 Thorstensen & Freed (1985), 46 Hodgkin et al. (2019b), 47 Denisenko & Martinelli (2016), 48 Joshi (2013), 49 vsnet-alert 25875, 50 Thorstensen & Halpern (2013), 51 Szkody et al. (2007), 52 Augustejn et al. (2010), 53 Patterson et al. (2003), 54 Greaves (2006), 55 vsnet-chat 7946, 56 Cragg (1960), 57 Antipin & Kroll (2003), 58 Schmidt et al. (2005b), 59 Israel et al. (1998), 60 Stefanov & Stefanov (2023), 61 Denisenko et al. (2008), 62 Wei et al. (1997), 63 Thorstensen et al. (2016), 64 Richter (1990), 65 Vladimirov et al. (2017), 66 Schaefer et al. (2019), 67 Delgado et al. (2018a), 68 Gabdeev et al. (2019), 69 Pretorius (2009), 70 Swierczynski et al. (2010), 71 Southworth et al. (2015), 72 CRTS candidate CV, 73 ASAS-SN CV candidate, 74 Hoffmeister (1928), 75 Buckley et al. (1993), 76 Aungwerojwit et al. (2006), 77 Morokuma et al. (2014), 78 Khruslov et al. (2015), 79 Maza et al. (1990), 80 Szkody et al. (2009), 81 Thorstensen et al. (2009), 82 Paterson et al. (2019), 83 Croom et al. (2001), 84 Witham et al. (2007), 85 Inight et al. (2023a), 86 Ringwald et al. (1994), 87 Tappert et al. (2012), 88 Hodgkin et al. (2019c), 89 Kato & Hamsch (2023), 90 Kryachko et al. (2010), 91 Schwöpe et al. (2024), 92 VSNET 19440, 93 Shappee et al. (2014), 94 Bateson (1982), 95 CBAT, 96 vsnet-alert 18545, 97 Hoffmeister (1968), 98 Drake et al. (2014b), 99 vsnet-alert 22930, 100 Luyten (1933), 101 Woudt & Warner (2010), 102 Denis Denisenko, 103 Delgado et al. (2019c), 104 Balanutsa et al. (2017a), 105 Kraft (1962), 106 Herbig (1958), 107 Cheung et al. (2012), 108 Teyssier (2019), 109 Beuermann et al. (1999), 110 Boyd et al. (2011), 111 Pretorius & Knigge (2008b), 112 Adams & Burwell (1920), 113 Delgado et al. (2017i), 114 Simonian et al. (2014), 115 Gänsicke et al. (2009), 116 Remillard et al. (1991), 117 Rosino et al. (1983), 118 Vogt & Bateson (1982), 119 vsnet-alert 23388, 120 vsnet 20079, 121 Barwig et al. (1993), 122 Garnavich & Deal (2013), 123 Motch et al. (1996), 124 Bateson et al. (1997), 125 Szkody et al. (2020), 126 Bruch & Schimpke (1992), 127 Drake et al. (2008), 128 Hodgkin et al. (2021b), 129 Masetti et al. (2010), 130 Thorstensen et al. (1996), 131 Jones et al. (2009), 132 Balanutsa et al. (2016b), 133 Denisenko et al. (2012), 134 Bruch et al. (1987), 135 vsnet-alert 25868, 136 Stanishev et al. (2006), 137 Jiang et al. (2000), 138 Kato et al. (2017), 139 Ivezić et al. (2007), 140 Petit (1960), 141 Denisenko et al. (2014), 142 Thorstensen et al. (2023), 143 Green et al. (1986), 144 Bruch (1989), 145 Hardy et al. (2017), 146 Szkody et al. (2006), 147 Thorstensen & Halpern (2009), 148 Schaefer (2021), 149 Marsh et al. (2002), 150 Southworth et al. (2006), 151 Drake et al. (2009a), 152 Chen et al. (2020), 153 Dunér et al. (1911), 154 Goranskij (1972), 155 Carbon et al. (2017), 156 Ciatti & Rosino (1974), 157 Hoard & Szkody (1997), 158 Kato et al. (2014), 159 Fremling et al. (2018), 160 Szkody et al. (2002), 161 vsnet-alert 16767, 162 Stanek et al. (2018), 163 Homer et al. (2005), 164 Yecheistov et al. (2013b), 165 Downes et al. (2005), 166 Szkody (1985), 167 Thorstensen et al. (1997), 168 Schaefer (2022), 169 Sanduleak (1975), 170 Gress et al. (2017), 171 Kreiner (2004), 172 Thorstensen (1986), 173 Green et al. (1982), 174 Pojmanski (2002), 175 Guthnick & Prager (1926), 176 Thorstensen et al. (2002), 177 Motch et al. (1998), 178 Hodgkin et al. (2019a), 179 vsnet 17036, 180 CBA512, 181 Hackstein et al. (2015), 182 Silber et al. (1994), 183 Ashok et al. (2014), 184 Watson et al. (2006), 185 Munari & Zwitter (1998), 186 Hoffmeister (1966a), 187 Szkody et al. (2011), 188 vsnet-alert 5142, 189 Shore et al. (2013), 190 Hodgkin et al. (2020b), 191 Fuentes-Morales et al. (2021), 192 Howarth (1978b), 193 vsnet-chat 8009, 194 Gress et al. (2015), 195 Kamath et al. (2005), 196 Skiff (1999), 197 Hamsch (2014), 198 Dai et al. (2017), 199 Drake et al. (2009b), 200 Stanek (2017), 201 Uemura et al. (2010), 202 Morgenroth (1934), 203 Richter et al. (1988), 204 Williams (1983), 205 Woudt et al. (2012), 206 Parisi et al. (2014), 207 Halpern & Thorstensen (2015), 208 Zharikov et al. (2006), 209 Delgado et al. (2018b), 210 Prins et al. (2019), 211 Bateson (1972), 212 Hoffmeister (1966b), 213 Bruch et al. (1997), 214 Kjurkchieva et al. (2015), 215 Bao Supernova Survey et al. (1997), 216 VSNET 7967, 217 Fruth et al. (2013), 218 Homer et al. (2006), 219 Szkody et al. (2018), 220 Tappert et al. (2014), 221 Campbell & Shafter (1995), 222 Rodríguez-Gil et al. (2007a), 223 Duerbeck (1987), 224 Taylor & Thorstensen (1996), 225 Richter (1970), 226 Hou et al. (2020), 227 Yecheistov et al. (2013a), 228 Southworth et al. (2008), 229 Hodgkin et al. (2021a), 230 Downes & Shara (1993), 231 Fiedler et al. (1997), 232 Mason & Howell (2003), 233 Welsh et al. (2005), 234 Kato et al. (2012), 235 Shafter (1983), 236 Araujo-Betancor et al. (2003a), 237 Balanutsa et al. (2016a), 238 Szkody (1987), 239 Chen et al. (2001), 240 Rodríguez-Gil et al. (2007b), 241 Wagner et al. (2018), 242 Sheets et al. (2007), 243 Luo et al. (2018), 244 Kato et al. (2013), 245 Delgado et al. (2017g), 246 Hoffmeister (1967a), 247 Thorstensen & Skinner (2012), 248 Gänsicke et al. (2005), 249 Shapley et al. (1940), 250 Rodriguez et al. (2023), 251 Delgado et al. (2017b), 252 Southworth et al. (2010), 253 Thorstensen & Taylor (1997), 254 Szkody & Mateo (1986), 255 Croom et al. (2004), 256 Miller (1971), 257 Thorstensen (1997), 258 Humason (1938), 259 vsnet-alert 22124, 260 vsnet 15408, 261 Ramsay et al. (2018), 262 Hartwig et al. (1919), 263 Tappert et al. (2013), 264 Schwarz et al. (2002), 265 Tappert et al. (2004), 266 Szkody & Howell (1992), 267 Thorstensen et al. (2015), 268 Inight & Copperwheat (2018), 269 Mowlavi et al. (2021), 270 Balanutsa et al. (2015a), 271 Delgado et al. (2019b), 272 Shears et al. (2008a), 273 Balanutsa et al. (2012), 274 Cordoni et al. (1977), 275 Gezari et al. (2013), 276 Delgado et al. (2017a), 277 Stanek et al. (2013b), 278 Masetti et al. (2006), 279 Ritter & Kolb (2003), 280 Siviero & Munari (2016), 281 Downes et al. (2001), 282 Lamost 8/1/2016, 283 Delgado et al. (2017e), 284 Schmidt et al. (2005a), 285 Gabdeev et al. (2015), 286 Shimansky et al. (2011), 287 Munari et al. (1990), 288 Shappee et al. (2013), 289 Drake et al. (2014a), 290 Unda-Sanzana et al. (2008), 291 Hodgkin et al. (2023), 292 Breedt et al. (2014), 293 vsnet-chat 8507, 294 Kato et al. (2004), 295 Berg et al. (1992), 296 Patterson et al. (2001), 297 Szkody et al. (2003a), 298 Thorstensen et al. (2010), 299 di Ciccio et al. (1999), 300 Nakano et al. (2007), 301 Inight et al. (2023b), 302 Hu et al. (1997), 303 vsnet-alert 21863, 304 Balanutsa et al. (2017b), 305 Wyse (1936), 306 Kraus et al. (2007), 307 Heinze et al. (2018), 308 Hirayama et al. (1993), 309 Ahnert & Hoffmeister (1941), 310 Schwöpe et al. (1997), 311 Hagen et al. (1995), 312 Sun et al. (2021), 313 Thorstensen et al. (2017), 314 Gessner & Meinunger (1974), 315 Ceraski (1908), 316 Szkody et al. (2014), 317 Kato et al. (2010), 318 AAVSO, 319 Kato et al. (2016), 320 Witham et al. (2008), 321 Poggiani (2009), 322 Tebbutt (1878), 323 Joshi et al. (2022), 324 Echevarría et al. (2007), 325 Jayasinghe et al. (2018), 326 vsnet-alert 18588, 327 Thorstensen et al. (2020), 328 Shumkov et al. (2017), 329 vsnet-chat 7968, 330 Denisenko & Sokolovsky (2011), 331 Thorstensen (2013), 332 Hoffmeister (1967b), 333 Southworth et al. (2007), 334 Delgado et al. (2017j), 335 Thorstensen et al. (2004), 336 MGAB Variable Star Catalog, 337 Thorstensen & Taylor (2000), 338 Marin & Shafter (2009), 339 Kochanek et al. (2017), 340 Vogt (1980), 341 Szkody et al. (2003b), 342 Hoffleit (1932), 343 Peters & Thorstensen (2005), 344 Bonnet-Bidaud et al. (2007), 345 Wei et al. (1999), 346 Delgado et al. (2017d), 347 vsnet-chat 7978, 348 Popova et al. (2015), 349 Yakin et al. (2011), 350 VSNET 12318, 351 Huber et al. (2015), 352 Oliveira et al. (2020), 353 Szkody et al. (2004), 354 Balanutsa et al. (2013), 355 Zubareva et al. (2011), 356 Vladimirov et al. (2014), 357 Delgado et al. (2019a), 358 Kato et al. (2009), 359 Kato & Romanov (2022), 360 Groebel (2009), 361 Malkova et al. (2017), 362 Wils et al. (2010), 363 Thorstensen & Taylor (2001), 364 Förster et al. (2021), 365 Downes et al. (1995), 366 Bruch (2023), 367 Kimura et al. (2016), 368 vsnet 19297

### 3 RESULTS

Specific Details are presented below. For simplicity the system names are abbreviated by omitting arc seconds – thus for example SDSS J000600.15+012129.8 becomes J0006+0121.

#### 3.1 New systems

##### 3.1.1 SDSS J003529.47–735826.3

The SDSS spectrum shows single-peaked Balmer and He I emission lines above a blue continuum. The object is above the white dwarf cooling sequence in the HR diagram. The ATLAS light curve shows frequent low-amplitude transients ( $\approx 0.3$  mag). The spectrum resembles an Ae/Be star, but the absolute magnitude is a bit too low. There is no infrared excess in the SED to indicate a Young Stellar Object (YSO). This is probably a CV and, from its spectrum and position in the HR diagram, probably a novalike.

##### 3.1.2 SDSS J012132.92–740819.5

The spectrum shows Balmer emission lines consistent with a novalike. The position in the HR diagram is also consistent with a novalike.

##### 3.1.3 SDSS J012905.53–580841.2

The SDSS spectrum shows double-peaked He I emission lines. The object is on the white dwarf cooling sequence in the HR diagram. This is an AM CVn.

##### 3.1.4 SDSS J024720.92–605050.7

There is a *ROSAT* detection in the range 0.1 – 20 keV, which is most likely the X-ray counterpart to this object. The CRTS light curve does not show any outbursts whilst Gaia shows variability around an overall brightening. The spectrum shows strong single-peaked Balmer, He I and He II emission lines. The donor signature is clearly visible in the spectrum. This is midway between the main sequence and the white dwarf cooling sequence in the HR diagram. The ATLAS light curve shows a double-humped modulation, and apparent cyclotron beaming, with a period of 2.455 h. This is a polar CV.

##### 3.1.5 SDSS J041428.92–631946.0

The spectrum shows single-peaked Balmer and He I emission lines. The CRTS light curve shows one outburst. The Gaia light curve shows gradual dimming. There is a *GALEX* ultraviolet detection. The *Gaia* variability table classifies this as a CV.

##### 3.1.6 SDSS J043118.90–005534.9

The SDSS spectrum shows double-peaked Balmer, He I and Ca lines. The ZTF and CRTS light curves show no outbursts but significant variability. This object may be weakly magnetic with a field strong enough to prevent a disk forming.

##### 3.1.7 SDSS J044652.51+471408.3

This object is referred to as ZTF J044652.50+471408.4 in [Chen et al. \(2020\)](#) of the BY Dra type and reporting periods of 18.17 d (*g*-band) and 1.05 d (*r* band). The folded TESS light curve shows a double eclipse with a period of 6.63 h. The spectrum shows double-peaked Balmer and He II emission. Although this is above the main sequence in the HR diagram it would be placed below the sequence when reddening of  $E(B - V) = 0.64$  is taken into account. This is a CV with starspots the likely reason for the differing magnitude of the two peaks in the folded light curve.

##### 3.1.8 SDSS J050153.52–034208.6

The spectrum shows double-peaked asymmetric Balmer lines. It is at the top of the white dwarf cooling sequence in the HR diagram. We obtained a period of 1.534(1) h from ZTF photometry. Based on the period and lack of outbursts it is an SU UMa and probably a WZ Sge.

##### 3.1.9 SDSS J061222.10–594449.3

The spectrum shows asymmetric single-peaked Balmer emission lines and He II emission. The object is located closer to the main sequence than the white dwarf cooling sequence in the HR diagram. The sparse CRTS light curve does not show any outbursts. There is an *XMM* X-ray detection in the range 0.1 – 12 keV. This is probably a magnetic CV.

##### 3.1.10 SDSS J075522.38+040719.3

The sparse ZTF and CRTS light curves do not show any outbursts. The spectrum shows asymmetric single-peaked Balmer and He I emission lines. The object is located half way between the main sequence and the white dwarf cooling sequence in the HR diagram.

##### 3.1.11 SDSS J075655.95+062646.7

The spectrum shows single-peaked Balmer and He II emission lines. The object is located half way between the main sequence and the white dwarf cooling sequence in the HR diagram. The ZTF light curve shows a dimming period but no outbursts.

##### 3.1.12 SDSS J084708.28+011939.1

The spectrum shows double-peaked helium emission lines but no hydrogen lines. The sparse ZTF and CRTS light curves do not show any outbursts. This is an AM CVn.

##### 3.1.13 SDSS J084735.40+014533.9

The SDSS spectrum shows double-peaked Balmer and He I emission lines. Neither the ZTF nor the CRTS light curves exhibit any outbursts. This is a CV - most probably a short-period CV such as a WZ Sge.

*3.1.14 SDSS J085550.85–015428.6*

The SDSS spectrum shows double-peaked Balmer and He I emission lines. There are also indistinct Balmer absorption lines from the white dwarf signature. Neither the ZTF nor the CRTS light curves exhibit any outbursts. It is on the white dwarf sequence in the HR diagram. This is likely to be a WZ Sge: although its white dwarf is cooler than that of most WZ Sge's (which would be consistent with the indistinct signature).

*3.1.15 SDSS J091248.24–000721.3*

The SDSS spectrum shows double-peaked Balmer and He I emission lines. The object is midway between the main sequence and the white dwarf cooling sequence in the HR diagram. The ZTF light curve shows variability but no outbursts.

*3.1.16 SDSS J091818.55+043610.0*

The SDSS spectrum shows double-peaked Balmer and He I emission lines. Neither the ZTF nor the ATLAS light curves exhibit any outbursts. This is a CV - most probably a short-period CV such as a WZ Sge.

*3.1.17 SDSS J092902.86+005334.0*

The SDSS spectrum shows double-peaked Balmer and He I emission lines. There is no *Gaia* counterpart. There is an *XMM* X-ray detection in the range 0.1 – 12 keV.

*3.1.18 SDSS J095312.66–042732.0*

The spectrum shows asymmetric double-peaked He I lines. There is no *Gaia* counterpart. There is a *GALEX* ultraviolet detection. The ZTF and ATLAS light curves do not show any dwarf novae outbursts. The ZTF light curve shows an outburst lasting  $\approx 200$  d around MJD = 58870.

*3.1.19 SDSS J102215.84–035927.8*

The spectrum shows asymmetric double-peaked Balmer and He I emission lines. There is no *Gaia* parallax. The ZTF light curve shows four outbursts.

*3.1.20 SDSS J113542.62–581515.9*

Our noisy ( $S/N = 1.8$ ) spectrum exhibits double-peaked Balmer and He II emission lines. There is no light curve data available and so we tentatively classify this as a magnetic CV.

*3.1.21 SDSS J122321.22–614758.1*

The spectrum shows single-peaked Balmer, He I and He II emission lines above a red continuum. There are *XMM* X-ray detections in the range 0.1 – 12 keV. The object is located next to the main sequence in the novalike area. We therefore classify this as a novalike.

*3.1.22 SDSS J124100.45–593033.4*

The spectrum shows single-peaked Balmer emission lines above a blue continuum. The object is located near to the main sequence in the novalike area. There are no outbursts in the *Gaia* light curve. We classify this as a novalike.

*3.1.23 SDSS J141436.78+162104.2*

The spectrum shows double-peaked Balmer and He I emission lines. The white dwarf signature is prominent in the spectrum. It is located close to the white dwarf cooling sequence in the HR diagram. The ZTF and CRTS light curves do not show any outbursts although the ZTF light curve does show variability with  $\Delta m \approx 1.5$  over a duration of months. Without further data we can only classify this as a CV.

*3.1.24 SDSS J143427.17–640303.1*

The spectrum shows single-peaked Balmer emission lines above a red continuum. There are *XMM* X-ray detections in the range 0.1 – 12 keV. The object is located next to the main sequence in the novalike area. We therefore classify this as a novalike.

*3.1.25 SDSS J143558.50+033217.6*

The spectrum shows double-peaked Balmer, He I and He II emissions lines. There is no *Gaia* counterpart. The ZTF light curve shows at least one outburst.

*3.1.26 SDSS J145225.24–042931.9*

The SDSS spectrum shows double-peaked Balmer and double-peaked He I emission lines. The white dwarf is visible and there is no sign of the donor signature. The ZTF light curve shows no outbursts. It lies close to the white dwarf cooling sequence. We therefore tentatively classify this as a WZ Sge.

*3.1.27 SDSS J150218.82+023055.2*

The SDSS spectrum shows double-peaked Balmer emission lines. The white dwarf is visible and there is no sign of the donor signature. The ZTF and CRTS light curves show no outbursts. We found a period of 1.50227(2) h from the ZTF light curve. The object lies on the white dwarf cooling sequence. We therefore tentatively classify this as a WZ Sge.

*3.1.28 SDSS J152020.39–000948.3*

The SDSS spectrum shows single-peaked Balmer emission lines above a blue continuum. The object is in the novalike area of the HR diagram. The ZTF light curve shows a deep dimming consistent with a VY Scl type novalike.

*3.1.29 SDSS J162008.82+024414.6*

The SDSS spectrum shows double-peaked Balmer and double-peaked He I emission lines. The Balmer lines sit in the absorption lines from the white dwarf whilst there is no sign of the donor signature. The sparse ZTF light curve shows no outbursts. It lies close to the white dwarf cooling sequence. We therefore tentatively classify this as a WZ Sge.



## 3.1.30 SDSS J165141.45–490712.2

The spectrum shows double-peaked Balmer and Paschen emission lines above a red continuum. It is next to the main sequence in the HR diagram. The ATLAS light curve shows no outbursts. This is probably a novalike.

## 3.1.31 SDSS J165859.91–512331.3

The spectrum shows double-peaked Balmer emission lines above a blue continuum. It is close to the main sequence in the HR diagram. The ATLAS light curve shows variability but no outbursts.

## 3.1.32 SDSS J171226.57–641656.8

The SDSS spectrum shows double-peaked Balmer emission lines. The Balmer lines sit in the absorption lines from the white dwarf whilst there is no sign of the donor signature. The ATLAS light curve shows no outbursts. It lies in the white dwarf cooling sequence. We therefore tentatively classify this as a WZ Sge.

## 3.1.33 SDSS J172256.18–261906.8

The spectrum shows double-peaked Balmer emission lines above a red continuum. It is next to the main sequence in the HR diagram when reddening is accounted for. The ZTF light curve shows no outbursts. We found a period of 6.63601(2) h from the ZTF light curve.

## 3.1.34 SDSS J172904.97–483742.0

The SDSS spectrum shows double-peaked Balmer emission lines. The object is closer to the white dwarf cooling sequence than the main sequence in the HR diagram. There is no light curve data and hence we can only classify this as a CV.

## 3.1.35 SDSS J174345.53–725309.1

The SDSS spectrum shows double-peaked Balmer, He I and He II emission lines. The object is midway between the white dwarf cooling sequence and the main sequence in the HR diagram. There is no light curve data available other than some isolated ATLAS datapoints.

## 3.1.36 SDSS J174907.74–621227.0

The SDSS spectrum shows single-peaked Balmer and He I emission lines with the cool donor signature clearly visible. The object is close to the main sequence in the HR diagram. The *Gaia* light curve shows variability but no outbursts. We obtained a period of 2.569307(6) h from the *Gaia*, ATLAS and CRTS photometry. There is an *XMM* X-ray detection in the range 0.1 – 12 keV. This is probably a CV.

## 3.1.37 SDSS J181738.37+042644.3

The SDSS spectrum shows double-peaked Balmer and He I lines. The object is close to the main sequence in the HR diagram. The ATLAS light curve shows frequent outbursts and a period of smaller outbursts.

## 3.1.38 SDSS J181810.72+050958.5

The SDSS spectrum shows double-peaked Balmer emission lines and a hint of the white dwarf signature above a blue continuum. The object is next to the white dwarf cooling sequence in the HR diagram. There are no outbursts in the ZTF light curve. There is no He II emission, Zeeman splitting or cyclotron humps to indicate a magnetic CV and so this is likely to be a short-period SU UMa or WZ Sge.

## 3.1.39 SDSS J182707.63–520430.0

The spectrum shows double-peaked Balmer and He I emission lines. The object is nearer the white dwarf cooling sequence than the main sequence in the HR diagram.

## 3.1.40 SDSS J190508.92–130608.6

The SDSS spectrum shows double-peaked Balmer and He I emission lines. The object is midway between the main sequence and the white dwarf cooling sequence in the HR diagram. The ZTF light curve shows multiple outbursts.

## 3.1.41 SDSS J190625.62–111156.8

The SDSS spectrum shows weak Balmer emission lines above a blue continuum. The object is near the main sequence in the novalike area. The spectrum is consistent with the SED and the *Gaia* G-band magnitude and so is not in outburst. We obtained a period of 3.8250(2) h from the ZTF light curve.

## 3.1.42 SDSS J190645.39–131314.2

The SDSS spectrum shows single-peaked Balmer, He I and He II emission lines. There is no sign of the donor or the white dwarf in the spectrum. The object is located near to the main sequence in the HR diagram. The ZTF light curve shows unusual deep dropouts but no outbursts.

## 3.1.43 SDSS J190739.31–124117.5

The SDSS spectrum shows Balmer and He II emission lines above a blue continuum. The object is located in the novalike area of the HR diagram. The ZTF light curve shows variability but no outbursts. We obtained a period of 3.4437(1) h from the ZTF light curve.

## 3.1.44 SDSS J191630.00–065204.4

The SDSS spectrum shows single-peaked Balmer, He I and He II emission lines above a blue continuum. The ZTF light curve shows variability ( $\Delta m \approx 0.4$ ) but no outbursts. This object is in the novalike area of the HR diagram.

## 3.1.45 SDSS J191705.21–095144.8

See main paper.

*3.1.46 SDSS J192933.11–560343.0*

The spectrum shows single-peaked Balmer, He I and strong He II emission lines. It is located closer to the main sequence than the white dwarf cooling sequence. The CRTS light curve shows variability and phase changes but no outbursts. The *TESS* light curve shows a period of 1.542 h.

*3.1.47 SDSS J193025.79–483052.4*

The SDSS spectrum shows single-peaked Balmer, He I and He II emission lines. The equivalent width of the He II line is almost as large as that of the H $\beta$  line. The object is located midway between the main sequence and the white dwarf cooling sequence. The CRTS light curve does not show any outbursts. We obtained a tentative period of 2.29126(5) h from the CRTS light curve. Based on the shape of the emission lines together with apparent cyclotron humps in the spectrum we classify this as a polar.

*3.1.48 SDSS J193244.66+003559.9*

The SDSS spectrum shows single-peaked Balmer and He II emission lines. The equivalent width of the He II line is greater than that of the H $\beta$  line. The object is located near the main sequence in the HR diagram when reddening of  $E(B - V) = 0.35$  is accounted for. The ZTF light curve does not show any outbursts but shows evidence of eclipsing. We obtained a period of 3.6327(1) h from the ZTF light curve. We classify this as a novalike.

*3.1.49 SDSS J193423.17+020252.7*

The SDSS spectrum shows single-peaked Balmer, He I and He II emission lines. The equivalent width of the He II line is similar to that of the H $\beta$  line. The object is located near the main sequence in the HR diagram when reddening of  $E(B - V) = 0.36$  is accounted for. The ZTF light curve does not show any outbursts. We obtained a tentative period of 3.6370(1) h from the ZTF light curve. We classify this as a novalike.

*3.1.50 SDSS J193504.85–574934.9*

The SDSS spectrum shows Balmer, He I and He II emission lines. The object is located midway between the main sequence and the white dwarf cooling sequence. The *Gaia* light curve shows an outburst of  $\Delta m \approx 2$ .

*3.1.51 SDSS J193628.84–551642.2*

The SDSS spectrum shows double-peaked Balmer emission lines with the white dwarf signature visible. The object is closer to the white dwarf cooling sequence than the main sequence in the HR diagram. There is one outburst in the CRTS light curve.

*3.1.52 SDSS J195938.44–551902.4*

We have two spectra observed on consecutive days. They both show double-peaked Balmer emission lines above a blue continuum although the equivalent width of the lines has doubled in the second spectrum. The object is located in the novalike area of the HR diagram. The CRTS and ATLAS light curves do not show any outbursts. The double-peaked lines are unusual in a novalike and this,

together with the doubling of equivalent width, is reminiscent of stunted outbursts (Schlegel & Honeycutt 2019).

*3.1.53 SDSS J195939.71+655440.9*

Our three spectra all show single-peaked Balmer emission lines above the red continuum from the donor. The object is located next to the main sequence in the HR diagram. The ZTF and ATLAS light curves do not show any outbursts. We obtained a period of 7.8307(8) h from the *TESS* light curve.

*3.1.54 SDSS J200512.34–561255.4*

Our two spectra show dual-peaked Balmer and He I emission lines. The object is located midway between the main sequence and the white dwarf cooling sequence. We have no light curve data and so can only classify this as a candidate CV.

*3.1.55 SDSS J200729.55+625047.6*

See main paper.

*3.1.56 SDSS J201234.82–550304.4*

The spectrum shows single-peaked Balmer, He I and He II emission lines. It is located closer to the main sequence than the white dwarf cooling sequence. There is one apparent outburst in the ATLAS light curve. We found a tentative period of 4.43 h from the ATLAS photometry.

*3.1.57 SDSS J202310.39+643244.0*

The SDSS spectrum shows Balmer emission lines above a blue continuum. The object is located in the novalike area of the HR diagram. There are no outbursts in the ZTF light curve. We obtained a period of 3.680630(1) h from the *TESS* light curve.

*3.1.58 SDSS J203256.81–565951.8*

Our two spectra show double-peaked Balmer emission lines. The H $\beta$  and higher lines are set in the absorption lines from the white dwarf. The object is on the white dwarf cooling sequence in the HR diagram. The CRTS light curve does not show any outbursts.

*3.1.59 SDSS J212114.67–622749.7*

Our two spectra show single-peaked Balmer emission lines above a blue continuum. The object lies in the novalike area of the HR diagram. The ASAS-SN light curve does not show any outbursts.

*3.1.60 SDSS J221552.06–613545.1*

The spectrum shows single-peaked Balmer, He I and He II emission lines. It is located closer to the main sequence than the white dwarf cooling sequence. There is an *eROSITA* X-ray detection (Merloni et al. 2024) in the range 0.3 – 10 keV. This is probably a magnetic CV but more data is needed to confirm the classification.



### 3.1.61 SDSS J224813.46+640023.1

The SDSS spectrum is dominated by cyclotron humps - consistent with a magnetic field of  $B \simeq 47$  MG. This object is midway between the main sequence and the white dwarf cooling sequence in the HR diagram. The ZTF light curve shows a clear state change but no outbursts.

## 3.2 Previously known systems

### 3.2.1 SDSS J000155.14-670743.3

We concur with vsnet-chat 8105 that this is a novalike based on its spectrum and position in the HR diagram. The period is quoted on VSX and originates from J Patterson and the Center of Backyard Astrophysics message number 512.

### 3.2.2 SDSS J001204.50+020129.6

The spectrum shows broad double-peaked Balmer emission lines on a blue continuum. Taken with its position on the HR diagram this a novalike and not a subdwarf as previously reported. The ZTF light curve shows no outbursts and a narrow eclipse. We obtained a period of 3.288(1) h from the *TESS* photometry.

### 3.2.3 SDSS J005000.03-760827.3

The SDSS spectrum shows weak Balmer emission lines above a blue continuum consistent with a novalike. The position in the HR diagram is also consistent with a novalike. The ATLAS light curve does not show any outbursts.

### 3.2.4 SDSS J005050.87+000912.6

The outburst in 2016 (vsnet-alert 20328) confirmed that this is a WZ Sge.

### 3.2.5 SDSS J012754.58-581717.5

The SDSS spectrum shows double-peaked Balmer emission lines. It is close to the white dwarf cooling sequence in the HR diagram which is consistent with the previous classification of SU UMa.

### 3.2.6 SDSS J015007.16+302203.9

The spectrum shows both Balmer and He I emission lines typical of a CV. The ZTF light curve shows multiple outbursts and one superoutburst. These, together with the position in the HR diagram, indicate that this is an SU UMa.

### 3.2.7 SDSS J015543.47+002807.4

See main paper.

### 3.2.8 SDSS J020809.57+565239.7

The SDSS spectrum shows narrow single-peaked Balmer emission lines and also strong He II emission. The spectrum also shows strong Mg I absorption which is indicative of a K-type star. There is a hint of cyclotron humps in the continuum. It is located at the edge of the main sequence in the HR diagram when reddening of

$E(B - V) = 0.43$  is accounted for. There is a *Swift* (0.1 – 10 keV) detection. This is probably a magnetic CV.

### 3.2.9 SDSS J024607.56-633546.0

The SDSS spectrum shows double-peaked Balmer and He II emission lines. It is close to the white dwarf cooling sequence in the HR diagram which is consistent with the previous classification of SU UMa.

### 3.2.10 SDSS J031538.60+623314.9

The ZTF light curve shows frequent, almost continuous, superoutbursts every  $\sim 20$  h.

### 3.2.11 SDSS J032815.90+612517.5

This was identified as a CV by *Gaia* alerts. The ZTF light curve shows outbursts and we obtained a reliable orbital period from *TESS*. However a more accurate period was obtained from unpublished MDM observations.

### 3.2.12 SDSS J034515.42-015216.4

The SDSS spectrum shows double-peaked Balmer, Paschen and He II emission lines and also the signature of a white dwarf. It is located nearer to the white dwarf cooling sequence than the main sequence in the HR diagram. The ZTF light curve shows multiple outbursts and superoutbursts confirming the previous classification of SU UMa.

### 3.2.13 SDSS J040834.99+511448.2

Sheets et al. (2007) found two possible orbital periods, 3.52 h or 4.13 h. We have obtained a photometric period from *TESS* of 3.3752(2) h.

### 3.2.14 SDSS J041844.43+510731.3

We have obtained a photometric period from *TESS* of 6.2994(7) h.

### 3.2.15 SDSS J042609.35+354144.3

We have obtained a photometric period from *TESS* of 1.57232(2) h.

### 3.2.16 SDSS J050906.73-032507.7

The spectrum shows Balmer and He emission lines together with both a K-type donor and a white dwarf. The ZTF and CRTS light curves both show  $\sim 3.5$  mag outbursts whilst the *TESS* photometry reveals a period of 8.48 h. The folded *TESS* light curve shows a double eclipse. Unpublished MDM data provides a more accurate period of 8.4780(2) h. This is a U Gem.

### 3.2.17 SDSS J051042.60+513539.9

The spectrum shows double-peaked Balmer and He I emission lines. The ZTF light curve reveals outbursts and two apparent superoutbursts. The superoutbursts suggest that this is an SU UMa but that would not be consistent with the position on the HR diagram nearer the main sequence than the white dwarf cooling sequence.

3.2.18 *SDSS J051419.88+011120.9*

The CRTS light curve shows a single outburst of  $\sim 5$  mag whilst the ZTF light curve shows two outbursts of  $\sim 3$  mag. The spectrum shows single-peaked Balmer and He I emission lines.

3.2.19 *SDSS J051949.58+642921.7*

The spectrum shows double-peaked Balmer and He I emission lines. The He I lines are much stronger (relative to the Balmer lines) in our spectrum (MJD = 59893) than that of LAMOST (MJD = 58045). The ZTF light curve shows significant variability ( $\Delta m \simeq 0.5$ ) but no significant outbursts. The long term ZTF light curve shows a gradual drop in magnitude of  $\sim 1$  mag over five years. This is in the novalike area of the HR diagram and therefore this is the most likely subtype. The deep dimming in the ZTF light curve around MJD = 58750 is suggestive of the VY Scl subtype.

3.2.20 *SDSS J052316.13+630728.9*

[Brimacombe et al. \(2014\)](#) identified a transient. The SDSS spectrum shows Balmer and double-peaked He I lines. The position in the HR diagram is consistent with, and confirms, our classification of a dwarf nova. The system is too faint to obtain survey photometry and hence the orbital period for this system.

3.2.21 *SDSS J060602.72+603941.4*

There are nine spectra all showing double-peaked Balmer emission lines. The *Gaia* light curve shows the  $\Delta m \simeq 6$  outburst reported by [Simonian et al. \(2014\)](#). It is located close to the white dwarf cooling sequence and the period of 1.329 h leads to the classification of WZ Sge.

3.2.22 *SDSS J061558.69+515423.9*

The ASAS-SN light curve shows frequent outbursts with  $\Delta m \simeq 2$  and a standstill between MJD  $\simeq 57920$  and MJD  $\simeq 58130$  confirming the classification of Z Cam by Denis Denisenko. The spectrum shows Balmer emission lines above a blue continuum. The synthetic magnitude is  $M_G = 14.7$  indicating that it was in outburst at the time of the observation. We obtained a period of 5.0407(6) h from *TESS* photometry.

3.2.23 *SDSS J062953.89+033508.4*

[Arjyotha et al. \(2009\)](#) obtained a period of 9.24(1) h. We obtained an improved period of 9.120(1) h from *TESS* photometry.

3.2.24 *SDSS J063047.05+023931.2*

The SDSS spectrum shows single-peaked Balmer emission lines. It appears close to the main sequence in the HR diagram before reddening and parallax uncertainty are taken into account. The observed superhumps confirm that this is an SU UMa.

3.2.25 *SDSS J063844.17+181611.4*

The SDSS spectrum shows Balmer absorption lines above a blue continuum. The synthetic magnitude is  $M_G = 15.9$  indicating that it was in outburst at the time of the observation.

3.2.26 *SDSS J064949.95+554140.4*

The SDSS spectrum shows Balmer and double-peaked He I emission lines consistent with the photometric classification of SU UMa.

3.2.27 *SDSS J064950.93+073741.0*

See main paper.

3.2.28 *SDSS J070533.80+125004.8*

There are multiple outbursts in the ATLAS photometry showing that this object is a dwarf nova.

3.2.29 *SDSS J072142.29+640050.8*

The SDSS spectrum shows double-peaked Balmer and He I emission lines above a blue continuum. It is closer to the main sequence than the white dwarf cooling sequence in the HR diagram. There is a 1.3 mag outburst in the ASAS-SN light curve. We found a period of 3.6492 h from the *TESS* light curve. This is a novalike.

3.2.30 *SDSS J072304.79+020437.2*

We obtained a period of 3.181 h from the *TESS* light curve. There are no outbursts in the *TESS*, ZTF and CRTS light curves. The object is in the top of the HR diagram just below the main sequence. This is all consistent with the existing classification of novalike.

3.2.31 *SDSS J073143.87+011714.9*

The SDSS spectrum shows weak single-peaked Balmer emission lines above a blue continuum. It is in the novalike area of the HR diagram consistent with the previous classification of Z Cam.

3.2.32 *SDSS J073817.74+285519.7*

Our new period is based upon MDM spectroscopy together with ZTF and *TESS* photometry.

3.2.33 *SDSS J073835.88+095805.6*

The SDSS spectrum shows double-peaked Balmer and He I emission lines. It is closer to the main sequence than the white dwarf cooling sequence in the HR diagram. Together with the outbursts in the ASAS-SN light curve we classify this as a U Gem.

3.2.34 *SDSS J074222.55+172806.7*

See main paper.

3.2.35 *SDSS J075233.17+294339.5*

[Inight et al. \(2023b\)](#) noted He II emission and this, combined with variability in the ZTF light curve that is reminiscent of cyclotron beaming, suggests that this may be a polar. [Inight et al. \(2023b\)](#) obtained a period of 1.4455 h from ZTF photometry. We obtained *TESS* photometry which shows that 1.4455 h was an alias and that the true period is either 1.2020(1) h or 2.4040(1) h. The ZTF light curve folded on 2.4040(1) h shows that this is the photometric period. However if this is a magnetic CV with the signal arising

from the magnetic poles the orbital period could still be half - i.e. 1.2020(1) h.

### 3.2.36 SDSS J075450.15+091019.6

The SDSS spectrum shows double-peaked Balmer and He II emission lines and also the signature of a white dwarf. There is no *Gaia* parallax and so it cannot be positioned on the HR diagram. The observed superhumps confirm that this is an SU UMa.

### 3.2.37 SDSS J075515.20+060439.3

Our three spectra show double-peaked Balmer emission lines thereby, together with the transient identified by ASAS-SN, confirming this as a dwarf nova. It is closer to the main sequence than the white dwarf cooling sequence in the HR diagram and is therefore likely to be a U Gem.

### 3.2.38 SDSS J075648.85-124653.9

See main paper.

### 3.2.39 SDSS J080033.86+192416.6

The SDSS spectrum shows double-peaked Balmer and He I emission lines. The object is between the main sequence and the white dwarf cooling sequence in the HR diagram. The ZTF light curve exhibits outbursts and Kato et al. (2014) reports superhumps. It is therefore classified as an SU UMa.

### 3.2.40 SDSS J080407.93-002216.4

See main paper.

### 3.2.41 SDSS J080448.88+024853.5

The SDSS spectrum shows double-peaked Balmer and He I emission lines. The ZTF and ASAS-SN light curves show outbursts leading to the classification of dwarf nova.

### 3.2.42 SDSS J080837.79-694712.8

The spectrum exhibits dual-peaked Balmer emission lines. The object is located next to the main sequence in the HR diagram. The *TESS* light curve shows five outbursts. There is an *XMM* X-ray detection in the range 0.1 – 12 keV.

### 3.2.43 SDSS J080853.73+355053.6

The SDSS spectrum shows double-peaked Balmer, He I and He II emission lines. The CRTS light curve shows frequent outbursts.

### 3.2.44 SDSS J081225.44-711437.2

The SDSS spectrum shows single-peaked Balmer, He I and He II emission lines. There are *Swift* (0.1 – 10 keV), *ROSAT* (0.1 – 20 keV) and *XMM* (0.1 – 12 keV) X-ray detections. The *TESS* and *Gaia* light curves both show outbursts. This may be magnetic but in the absence of more data we can only classify this as a dwarf nova.

### 3.2.45 SDSS J082603.71+113820.8

The SDSS spectrum shows single-peaked Balmer and He II emission lines and the signature of a white dwarf. It is midway between the white dwarf cooling sequence and the main sequence. The observed superhumps confirm that this is an SU UMa.

### 3.2.46 SDSS J082827.50-632958.8

The SDSS spectrum shows double-peaked Balmer emission lines above the donor signature. It is located on the main sequence in the HR diagram. The ATLAS light curve shows multiple outbursts confirming the classification of U Gem.

### 3.2.47 SDSS J084054.15+045518.4

Vsnet-chat 8566 classifies this as a Z Cam. We obtained a period of 3.08h from the *TESS* light curve

### 3.2.48 SDSS J084740.11-474318.5

The spectrum shows asymmetric single-peaked Balmer lines. There are broad wiggles in the continuum which may be cyclotron humps. The object is located just below the main sequence in the HR diagram. The *TESS*, ATLAS, ASAS-SN light curves do not show any outbursts but ASAS-SN shows variability with an amplitude of  $\Delta m = 1$ . This is likely to be a polar.

### 3.2.49 SDSS J085210.44+783246.7

See main paper.

### 3.2.50 SDSS J085640.28-040439.7

We have two SDSS spectra. Both spectra show Balmer emission lines but only one shows significant He I emission. Comparison with the ZTF light curve, which shows frequent outbursts, confirms that the spectra occurred during quiescence. There is at least one superoutburst exhibiting superhumps in the ZTF light curve. The object is positioned half way between the main sequence and the white dwarf cooling sequence in the HR diagram. We were unable to obtain a period from the *TESS* light curve due to flickering.

### 3.2.51 SDSS J085909.20+053654.4

We find a period of 2.3988(1) h from the *TESS* light curve which we believe is more precise than the period in Gänsicke et al. (2009).

### 3.2.52 SDSS J090756.67+715859.2

See main paper.

### 3.2.53 SDSS J091453.59+113401.5

The SDSS spectrum shows double-peaked Balmer and possibly He I lines. There are no outbursts in the ZTF light curve whilst the original CRTS discovery was based on a  $\Delta m \approx 4$  outburst.

3.2.54 *SDSS J092042.64+001903.2*

The SDSS spectrum shows broad Balmer emission lines, possibly double-peaked, indicating the presence of an accretion disk. The spectrum and SED are dominated by the K-type donor. The ZTF light curve shows frequent small ( $\sim 1$  mag) outbursts. The system may actually be eclipsing, as the primary minimum is sharp and flat-bottomed. We therefore classify this as a U Gem.

3.2.55 *SDSS J092534.78+434917.3*

See main paper.

3.2.56 *SDSS J093836.99+071454.6*

We obtained a period of 4.4736 h from the *TESS* photometry which is more precise than the period from [Thorstensen & Taylor \(2001\)](#).

3.2.57 *SDSS J100243.11-024636.0*

The spectrum shows asymmetric double-peaked Balmer lines. There is no *Gaia* counterpart. [Wils et al. \(2010\)](#) report multiple outbursts. ZTF photometry also shows multiple outbursts.

3.2.58 *SDSS J100434.76+662914.9*

We obtained a period of 3.3209(6) h from the *TESS* light curve which we consider to be more accurate than previous estimates.

3.2.59 *SDSS J103317.24+072118.6*

We obtained a tentative period of 1.694(2) h from *TESS* photometry.

3.2.60 *SDSS J112238.73-053949.4*

The SDSS spectrum shows double-peaked Balmer and He I lines. There are five outbursts ( $\Delta m \simeq 3$ ) recorded in *Gaia* alert Gaia19afc and at least seven outbursts in the ZTF light curve. It is near the main sequence in the HR diagram suggesting that it is a U Gem. However without an orbital period we can only classify this as a dwarf nova.

3.2.61 *SDSS J115223.94-673828.2*

The spectrum shows single-peaked Balmer and He II emission lines above a blue continuum. There are *ROSAT* (0.1 – 20 keV) and *XMM* (0.1 – 12 keV) X-ray detections. The object is located next to the main sequence in the novalike area. The ASAS-SN report shows a transient of  $\Delta m \simeq 1.5$ . We therefore classify this as a novalike.

3.2.62 *SDSS J120619.85-032838.6*

The SDSS spectrum shows double-peaked Balmer and He I emission lines. The ZTF light curve shows at least one superoutburst and superhumps.

3.2.63 *SDSS J122508.13-034721.0*

The SDSS spectrum shows double-peaked Balmer, He I and He II emission lines. The equivalent width of the He II emission line is comparable to that of H $\beta$  indicative of a polar CV. The continuum is flat and, especially as the CV is in a high state, the strong emission lines are not consistent with a novalike classification. There are *GALEX* FUV and NUV detections and also an *XMM* X-ray observation in the range 0.1 – 12 keV. The ZTF light curve shows a prolonged low state ( $m \simeq 22$  between MJD = 58250 and MJD = 59250 before reverting to the present regime of varying between  $m = 18$  and  $m = 19$ ). The light curves of both ZTF and CRTS show a period of 1.38 h with a possible alias of 1.31 h. We consider that this is a polar and that the VSX classification of novalike is incorrect.

3.2.64 *SDSS J124823.06-040100.9*

Our five spectra show double-peaked Balmer and He I emission lines. It is located closer to the white dwarf cooling sequence than the main sequence in the HR diagram.

3.2.65 *SDSS J131042.66-042600.6*

The SDSS spectrum shows double peaked Balmer and He I emission lines. The donor is not visible. The CRTS light curve shows an outburst and the ZTF light curve shows four including one probable superoutburst. It is located nearer the white dwarf cooling sequence than the main sequence in the HR diagram. This is probably an SU UMa.

3.2.66 *SDSS J133200.79-045410.5*

The SDSS spectrum shows double peaked Balmer and He I emission lines whilst the donor is not visible. vsnet-alert 27472 reports the presence of a superoutburst with superhumps confirming the classification as SU UMa. We obtained a tentative period of 1.93(1)h from the *TESS* light curve.

3.2.67 *SDSS J134309.43+782312.7*

The SDSS spectrum shows Balmer and He I emission lines above a blue continuum whilst the donor is not visible. The ASAS-SN light curve shows multiple outbursts together with a period of “stand-still” thereby confirming the classification of Z Cam. We obtained a clear period of 3.630 h from the *TESS* light curve. This is however inconsistent with our MDM spectroscopic period which has a daily cycle-count ambiguity and is either 3.77 h or 3.24 h. The *TESS* period, which is constant over more than three years, is most likely a negative superhump period with the orbital period being 3.77 h.

3.2.68 *SDSS J135218.95+280917.0*

We obtained a tentative period of 5.6845(4) h from ZTF photometry.

3.2.69 *SDSS J142833.38+003100.4*

The SDSS spectrum shows double peaked Balmer and He I emission lines. The H $\beta$  and higher emission lines are sitting in the absorption troughs from the white dwarf. The donor is not visible. It is located on the white dwarf cooling sequence in the HR diagram. Neither the ZTF nor the CRTS nor the ASAS-SN light curves show any outbursts. We tentatively classify this as a WZ Sge.

## 3.2.70 SDSS J144609.22+013604.5

The spectrum shows double-peaked Balmer emission lines above a stellar signature. It is located closer to the main sequence than the white dwarf cooling sequence. The ZTF, CRTS and *Gaia* light curves do not show any outbursts whilst the ATLAS light curve shows four. [Chen et al. \(2020\)](#) found a period of 1.4323 h from the ZTF light curve. The folded light curve from the ATLAS data clearly shows that the orbital period is twice this value.

## 3.2.71 SDSS J151836.03–054803.6

The SDSS spectrum shows double-peaked Balmer and He I emission lines. There is no sign of the white dwarf or donor signatures. The ZTF light curve shows two outbursts and the CRTS light curves shows one more. The object lies between the main sequence and the white dwarf cooling sequence. It is likely to be a short-period system but from the available data we can only classify this as a dwarf nova.

## 3.2.72 SDSS J152506.86–032655.4

The SDSS spectrum shows single-peaked Balmer, He I and He II emission lines above a blue continuum. The He II emission line is stronger than the H $\beta$  line in contrast to the much weaker He II in the spectra in [Gabdeev et al. \(2019\)](#). The object is located closer to the main sequence than the white dwarf cooling sequence in the HR diagram. The ZTF and CRTS light curves show variability but no outbursts. We obtained a period of 1.5453(1) h from *TESS* photometry which confirms the period found by [Hardy et al. \(2017\)](#) and is not consistent with the period found by [Gabdeev et al. \(2019\)](#).

## 3.2.73 SDSS J154336.53+751541.4

The photometry and spectroscopy of [Khruslov et al. \(2015\)](#) clearly identified this object as a CV with a period of 6.36862(3) h. From the ZTF light curve we observe frequent outbursts. This object lies next to the main sequence in the HR diagram and we therefore classify this as a U Gem.

## 3.2.74 SDSS J160450.19+414328.3

See main paper.

## 3.2.75 SDSS J160525.27–381212.1

The SDSS spectrum shows double-peaked He I and He II emission lines and no Balmer lines confirming that this is an AM CVn.

## 3.2.76 SDSS J160811.26–135058.2

See main paper.

## 3.2.77 SDSS J161030.19+445900.8

The SDSS spectrum shows double-peaked Balmer and He II emission lines. It is located next to the white dwarf cooling sequence in the HR diagram. In the absence of light curve data we can only classify this as a CV.

## 3.2.78 SDSS J161132.67+784319.4

The SDSS spectrum shows single-peaked Balmer emission lines above a blue continuum. The object is in the novalike area of the HR diagram. The ZTF light curve shows variability but no outbursts. The ATLAS light curve shows long-term variability. We found a period of 4.2508(2) h from the *TESS* photometry.

## 3.2.79 SDSS J161259.87–161715.6

The spectrum shows double-peaked Balmer, He I and He II emission lines. The He II line is approximately half the strength of the H $\beta$  line. It is located close to the main sequence. The ZTF light curve shows that it is eclipsing with a period of 3.5421(1) h. The ZTF and CRTS light curves do not show any outbursts. Based on the strength of the He II line and lack of outbursts this is a polar.

## 3.2.80 SDSS J161615.09–425825.4

The SDSS spectrum shows double-peaked Balmer and He I emission lines. The donor and white dwarf signatures are not visible. The object is closer to the main sequence than the white dwarf cooling sequence but this is unreliable due to the uncertainty in the *Gaia* parallax. We have no light curve data available.

## 3.2.81 SDSS J161618.69+115104.6

Our noisy (S/N = 1.7) spectrum exhibits double-peaked Balmer emission lines. There is no light curve data available and there is no *Gaia* parallax.

## 3.2.82 SDSS J161707.15–562720.0

The SDSS spectrum shows double-peaked Balmer emission lines above the absorption lines due to the white dwarf. TiO lines from the donor signature are visible. The object sits close to the main sequence in the HR diagram. The ASAS-SN light curve shows some variability and outbursts.

## 3.2.83 SDSS J161817.28+030936.8

See main paper.

## 3.2.84 SDSS J161853.17+070427.2

Our noisy (S/N = 1.8) spectrum exhibits single-peaked Balmer emission lines. The ZTF light curve shows variability ( $\Delta m \approx 1$ ) and a change to a low state but no outbursts. We obtained a period of 2.65 h from the ZTF photometry although it is possible that the period is half that as the folded light curve is ambiguous.

## 3.2.85 SDSS J162032.33–563519.8

The SDSS spectrum shows single-peaked Balmer emission lines above a stellar signature. The object is located on the left side of the main sequence when reddening is accounted for.



3.2.86 *SDSS J162109.00–135307.6*

Our noisy ( $S/N = 1.1$ ) spectrum exhibits double-peaked Balmer and He I emission lines. The ZTF light curve shows four outbursts. It is midway between the main sequence and the white dwarf cooling sequence in the HR diagram.

3.2.87 *SDSS J162433.30–293337.1*

The SDSS spectrum shows single-peaked Balmer emission lines. There is no sign of the white dwarf signature whilst the donor signature is visible. The CRTS light curve shows one outburst ( $\Delta m \approx 4.5$ ) and the ASAS-SN light curve shows two more. It lies close to the main sequence. We obtained a period of 5.5138(4) h from the TESS light curve. We therefore classify this as a U Gem.

3.2.88 *SDSS J162528.90–552003.6*

Our two spectra show single-peaked Balmer emission lines including unusually weak higher Balmer lines. There is no sign of the white dwarf signature whilst the donor signature is visible. It lies close to the main sequence. In conjunction with the outbursts noted in [Bateson & McIntosh \(1997\)](#) this is suggestive of a U Gem. However without further data we can only classify this as a dwarf nova.

3.2.89 *SDSS J162806.14+065315.3*

Our noisy ( $S/N = 1.8$ ) spectrum exhibits double-peaked Balmer and He I emission lines. It is midway between the main sequence and the white dwarf cooling sequence in the HR diagram. This is consistent with the classification of SU UMa noted by [Kato et al. \(2020\)](#).

3.2.90 *SDSS J162830.61–571407.3*

Our noisy ( $S/N = 0.6$ ) spectrum exhibits double-peaked Balmer and He I emission lines. It is near the main sequence in the HR diagram. This is consistent with the existing classification of U Gem.

3.2.91 *SDSS J163353.63–562759.2*

The SDSS spectrum exhibits double-peaked Balmer and He I emission lines. It is near the main sequence in the HR diagram.

3.2.92 *SDSS J163447.70–345423.6*

Our two spectra both show single-peaked Balmer lines above a blue continuum. The lines are narrow implying that the disc is almost face-on. The object is located next to the main sequence in the novalike region.

3.2.93 *SDSS J163805.39+083758.3*

See main paper.

3.2.94 *SDSS J164017.89+080823.0*

Our noisy ( $S/N = 2$ ) spectrum exhibits double-peaked Balmer and He I emission lines. It is nearer the main sequence than the white dwarf cooling sequence in the HR diagram. The ZTF light curve shows frequent outbursts with the quiescent level varying over time.

3.2.95 *SDSS J164204.25+151218.1*

The SDSS spectrum exhibits double-peaked Balmer and He I emission lines. There is no *Gaia* parallax. The ZTF light curve shows outbursts including two superoutbursts with superhumps.

3.2.96 *SDSS J164205.37–655335.8*

The spectrum shows double-peaked Balmer, He I and He II emission lines. It is located midway between the main sequence and the white dwarf cooling sequence. The ATLAS light curve does not show any outbursts. The ASAS-SN report shows an outburst of  $\Delta m > 4.8$ .

3.2.97 *SDSS J164449.42+195940.1*

The SDSS spectrum exhibits double-peaked Balmer and He I emission lines. There is no sign of the donor signature. The object is midway between the main sequence and the white dwarf cooling sequence in the HR diagram. This is all consistent with the existing classification of SU UMa.

3.2.98 *SDSS J164653.53+090726.1*

The SDSS spectrum exhibits single-peaked asymmetric Balmer and He I emission lines. There is no sign of the donor signature. The object is closer to the white dwarf cooling sequence than the main sequence in the HR diagram. The ZTF light curve shows variability  $\Delta m \approx 1$  but no outbursts although there is a state change of  $\Delta m \approx 2$ . The data is ambiguous as the spectrum shows no signs of being a magnetic CV (in particular weak He II emission) whilst the light curve is consistent with a magnetic CV (state change and no outbursts). We can therefore only classify this as a candidate CV.

3.2.99 *SDSS J164654.82+135359.4*

The SDSS spectrum shows Balmer emission lines above a blue continuum. The ZTF light curve shows variability but no outbursts. It is located on the blue horizontal branch of the HR diagram. This is consistent with being a novalike.

3.2.100 *SDSS J164925.44+140243.3*

Our noisy ( $S/N = 1.4$ ) spectrum exhibits double-peaked Balmer and He I emission lines. It is nearer the main sequence than the white dwarf cooling sequence in the HR diagram although this may be erroneous as the *Gaia* parallax is negative. The ZTF light curve shows no outbursts whilst the CRTS light curve shows a single  $\Delta m \approx 6$  superoutburst. This is all consistent with the classification of WZ Sge noted by [Kimura et al. \(2016\)](#).

3.2.101 *SDSS J164950.38+035834.5*

The spectrum shows double-peaked Balmer and He I emission lines. The signature of the white dwarf is clearly visible in the spectrum. The object is nearer the white dwarf cooling sequence than the main sequence in the HR diagram. The ZTF and CRTS light curves show multiple outbursts and at least two superoutbursts confirming the existing classification of SU UMa.

## 3.2.102 SDSS J165242.98+703014.8

The SDSS spectrum shows double-peaked Balmer lines above the red continuum from the donor. The object is next to the main sequence in the HR diagram. This is all consistent with the existing classification of U Gem.

## 3.2.103 SDSS J170044.63–500505.3

The SDSS spectrum shows narrow single-peaked Balmer emission lines. The H $\beta$  and higher Balmer lines are set in broad absorption lines. The synthetic magnitude of the spectrum is  $G = 18.5$  whilst *Gaia* reports  $G = 19.94$ . The light curve from *Gaia* alerts shows a gradual brightening since 2014 together with outbursts  $\Delta m \simeq 2$  in subsequent years. The emission lines are very narrow which might be due to the spectrum being taken during the rise or decline from an outburst. The object may also be a novalike or not a CV at all. We therefore classify this as a candidate CV.

## 3.2.104 SDSS J170655.18–150852.5

The SDSS spectrum exhibits double-peaked Balmer and He I emission lines. The object is midway between the main sequence and the white dwarf cooling sequence in the HR diagram. Outbursts are visible in the CRTS and *Gaia* light curves.

## 3.2.105 SDSS J171233.50–643342.6

The SDSS spectrum shows double-peaked Balmer emission lines. It is very close to the main sequence in the HR diagram. From the *Gaia* alerts light curve it has frequent outbursts of  $\Delta m \simeq 3.5$ . We obtained a period of 3.84(2) h from *TESS* photometry although it is possible that the orbital period is twice this. This therefore is probably a U Gem.

## 3.2.106 SDSS J171247.71+604602.9

See main paper.

## 3.2.107 SDSS J171658.14–313958.4

The spectrum shows single-peaked Balmer emission lines. It is close to the main sequence in the HR diagram. The ATLAS light curve shows regular outbursts with  $\Delta m \simeq 2$ . The ASAS-SN report shows an outburst of  $\Delta m \simeq 1.5$ . We obtained a period of 5.9446(4) h from ATLAS photometry.

## 3.2.108 SDSS J171937.17+043123.3

The SDSS spectrum exhibits double-peaked Balmer and He I emission lines. The object is midway between the main sequence and the white dwarf cooling sequence in the HR diagram. There are 4 low amplitude ( $\Delta m \sim 1.25$  mag) outbursts in the ASASSN light curve.

## 3.2.109 SDSS J172021.48–150928.9

The SDSS spectrum exhibits double-peaked Balmer and He I emission lines. The object is midway between the main sequence and the white dwarf cooling sequence in the HR diagram. Outbursts are visible in the ASAS-SN and *Gaia* alerts light curves.

## 3.2.110 SDSS J172515.56+073249.2

The ZTF light curve shows an isolated outburst with  $\Delta m \simeq 5$ . Taken with the position on the HR diagram this is likely to be an SU UMa but without additional data we can only classify this as a probable dwarf nova.

## 3.2.111 SDSS J172527.50–680822.4

The noisy (S/N = 1.3) SDSS spectrum shows weak Balmer emission lines.

## 3.2.112 SDSS J172925.15–404335.8

The SDSS spectrum shows double-peaked Balmer and He I emission lines. The object is positioned above the main sequence in the HR diagram although this is misleading as the *Gaia* parallax has a large uncertainty. The ATLAS photometry shows eight outbursts. Given that it is close to the main sequence it most probably has a long period and hence likely to be a U Gem.

## 3.2.113 SDSS J172959.01+522947.8

The SDSS spectrum has single-peaked asymmetric Balmer, He I and He II emission lines. The donor and the white dwarf are not visible. It is midway between the main sequence and the white dwarf cooling sequence in the HR diagram. The ZTF light curve shows  $\Delta m \simeq 2$  mag variability and also a state change but no outbursts. We obtained a period of 2.1528 h from the ZTF light curve. Together these are indicative of a polar classification.

## 3.2.114 SDSS J173408.80–430550.9

The SDSS spectrum shows double-peaked Balmer and He I emission lines. The object is closer to the white dwarf cooling sequence than the main sequence in the HR diagram. The ASAS-SN light curve shows a single outburst followed by sparse observations that appear to be superhumps. There is no other light curve data available.

## 3.2.115 SDSS J173634.28–711258.6

The SDSS spectrum shows double-peaked Balmer, He I and He II emission lines. The object is close to the main sequence in the HR diagram. The ASAS-SN light curve shows multiple outbursts. There is no other light curve data available.

## 3.2.116 SDSS J173905.58–452714.5

See main paper.

## 3.2.117 SDSS J174155.61–620817.9

The SDSS spectrum shows double-peaked Balmer and He I emission lines. The object is close to the main sequence in the HR diagram. There is no *Gaia* parallax. The only photometry available consists of three outbursts  $\sim 17$  mag observed by ATLAS. We can therefore only classify it as a dwarf nova based upon these outbursts and the original MASTER transient detection.



3.2.118 *SDSS J174342.09+553005.7*

The SDSS spectrum shows double-peaked Balmer, He I and He II emission lines. The object is close to the main sequence in the HR diagram. The *Gaia* light curve shows multiple transients.

3.2.119 *SDSS J174714.34+150047.5*

The SDSS spectrum shows double-peaked Balmer emission lines. The object is midway between the white dwarf cooling sequence and the main sequence in the HR diagram. The ZTF light curve shows frequent outbursts.

3.2.120 *SDSS J175505.10+132519.4*

The SDSS spectrum shows Balmer, He I and He II emission lines. The object is nearer the main sequence than the white dwarf cooling sequence in the HR diagram. The ZTF light curve shows considerable variability ( $\Delta m \simeq 2$ ) but no outbursts.

3.2.121 *SDSS J175545.04+704634.3*

The spectrum shows single-peaked Balmer, He I and He II emission lines. It is located closer to the main sequence than the white dwarf cooling sequence. The ASAS-SN and *TESS* light curves show frequent outbursts.

3.2.122 *SDSS J175622.38+025804.1*

The SDSS spectrum shows single-peaked Balmer lines above a blue continuum. The synthetic magnitude is  $G = 18.3$ . The ZTF light curve shows frequent outbursts whose magnitude confirms that our spectrum was observed during an outburst.

3.2.123 *SDSS J175951.66+592000.2*

The SDSS spectrum shows double-peaked Balmer lines above a blue continuum. The object is close to the main sequence in the HR diagram. The *Gaia* light curve shows outbursts.

3.2.124 *SDSS J175957.70+022144.5*

The SDSS spectrum shows Balmer, He I and He II emission lines. The object is nearer the white dwarf cooling sequence than the main sequence in the HR diagram. The ZTF light curve shows frequent outbursts including ones followed by apparent superhumps. We tentatively classify this as an SU UMa.

3.2.125 *SDSS J180005.86+525632.7*

Our noisy spectrum ( $S/N = 1.2$ ) shows double-peaked Balmer emission lines.  $H\beta$  and higher appear to sit in broad absorption lines. The object is closer to the white dwarf cooling sequence than the main sequence in the HR diagram.

3.2.126 *SDSS J180048.99+523234.5*

The SDSS spectrum shows Balmer, He I and He II emission lines. The object is midway between the main sequence and the white dwarf cooling sequence in the HR diagram. The ZTF light curve shows frequent outbursts and a probable superhump. We classify this as an SU UMa.

3.2.127 *SDSS J180245.76+100146.4*

The SDSS spectrum shows single-peaked Balmer and He I. The object is midway between the main sequence and the white dwarf cooling sequence in the HR diagram. The ZTF light curve shows three outbursts ( $\Delta m \simeq 4$ ) and considerable ( $\Delta m \simeq 1$ ) variability. The ASAS-SN light curve shows two more outbursts.

3.2.128 *SDSS J180312.65+114154.5*

The SDSS spectrum shows double-peaked Balmer and He I emission lines. The object is midway between the main sequence and the white dwarf cooling sequence in the HR diagram. The sparse ZTF light curve shows an outburst ( $\Delta m \simeq 2.5$ ) and the ASAS-SN light curve also shows an outburst.

3.2.129 *SDSS J180835.15+084829.1*

The SDSS spectrum shows double-peaked Balmer and He I lines. The object is close to the main sequence in the HR diagram. The ZTF light curve shows frequent outbursts and the object appears to be eclipsing. We obtained a period of 4.9647(3) h from ZTF photometry which is consistent with our MDM photometry.

3.2.130 *SDSS J180845.59+152101.1*

The SDSS spectrum shows Balmer, He I and He II emission lines. The object is nearer the white dwarf cooling sequence than the main sequence in the HR diagram. The ZTF and ATLAS light curves show frequent outbursts including ones followed by apparent superhumps. We classify this as an SU UMa.

3.2.131 *SDSS J181033.82+534946.0*

Our noisy ( $S/N = 1.4$ ) spectrum exhibits double-peaked Balmer and He I emission lines. It is nearer the main sequence than the white dwarf cooling sequence in the HR diagram although this may be erroneous as there is a large uncertainty in the *Gaia* parallax.

3.2.132 *SDSS J181244.08+592315.5*

The spectrum shows single-peaked Balmer, He I and He II emission lines. It is located closer to the main sequence than the white dwarf cooling sequence. The ZTF light curve shows outbursts and vsnet-alert 27854 reports superhumps from a superoutburst confirming the existing classification of an SU UMa. We obtained a period of 2.149544(3) h from the *TESS* light curve.

## 3.2.133 SDSS J181258.29+160247.1

The SDSS spectrum shows Balmer, He I and He II emission lines. The object is nearer the white dwarf cooling sequence than the main sequence in the HR diagram. The SED shows the contribution of the donor. The ZTF light curve shows one outburst and the ATLAS light curve shows multiple outbursts including one followed by apparent superhumps.

## 3.2.134 SDSS J181647.37+080014.9

The SDSS spectrum shows double-peaked Balmer lines in emission. The synthetic magnitude of  $G = 17.8$  indicates that the spectrum was observed during an outburst. The ZTF light curve shows frequent outbursts and also that the object is apparently eclipsing.

## 3.2.135 SDSS J181809.14+653136.0

The SDSS spectrum shows single-peaked asymmetric Balmer and He I lines. The object is midway between the main sequence and the white dwarf cooling sequence in the HR diagram. There are two outbursts in the *Gaia* alerts light curve.

## 3.2.136 SDSS J181821.01+125350.2

The SDSS spectrum shows double-peaked Balmer emission lines above a blue continuum. The object is located close to the main sequence in the HR diagram although this may be misleading due to the large uncertainties in the *Gaia* parallax. The ZTF light curve shows frequent outbursts; the object also appears to be eclipsing.

## 3.2.137 SDSS J181904.82+744123.8

The spectrum shows double-peaked Balmer and He I emission lines. The object is nearer the white dwarf cooling sequence than the main sequence in the HR diagram. The *Gaia* light curve shows multiple outbursts.

## 3.2.138 SDSS J182134.65+020307.1

The SDSS spectrum shows double-peaked Balmer and He I emission lines above the red continuum from the donor. The object is located next to the main sequence in the HR diagram. The ZTF light curve shows frequent outbursts and the object appears to be eclipsing. We obtained a period of 4.2704 h from the ZTF light curve. MDM observations confirmed the period and revealed a radial velocity of  $227 \text{ km s}^{-1}$ .

## 3.2.139 SDSS J182313.80+604106.1

The SDSS spectrum shows single-peaked Balmer lines in emission. The synthetic magnitude of  $G = 17.0$  indicates that the spectrum was observed during an outburst. The object is located close to the main sequence in the HR diagram. The *Gaia* and ATLAS light curves show outbursts.

## 3.2.140 SDSS J182319.26+051857.1

See main paper.

## 3.2.141 SDSS J182643.55+613816.5

Our spectra show double-peaked Balmer emission lines. The ZTF light curve shows multiple outbursts and at least two superoutbursts with superhumps. We obtained a period of 2.06541 h from the ZTF light curve.

## 3.2.142 SDSS J183014.15+671032.9

The SDSS spectrum shows double-peaked Balmer and He I emission lines. There is no sign of the donor or white dwarf signatures in the spectrum. The CRTS light curve shows two outbursts in addition to the one identified by ASAS-SN. The object is located next to the white dwarf cooling sequence in the HR diagram. This is likely to be a short-period system such as an SU UMa but we can only classify this as a dwarf nova with the available data.

## 3.2.143 SDSS J183144.55+651130.2

Pretorius et al. (2007) reported a spectroscopic period of 4.01(3) h. We obtained a period of 3.999660(1) h from *TESS* photometry.

## 3.2.144 SDSS J183228.19+101654.1

The SDSS spectrum shows Balmer, He I and He II emission lines. The object is close to the main sequence in the HR diagram in the novalike area. The ZTF light curve shows that the object is eclipsing but there are no outbursts visible. We obtained a period of 3.928318(3) h from the ZTF photometry.

## 3.2.145 SDSS J183442.34+514858.7

The spectrum shows double-peaked Balmer and He I emission lines. The object is next to the main sequence in the HR diagram. The ASAS-SN report shows an outburst  $\Delta m = 1.8$ . CRTS shows two outbursts with  $\Delta m = 4$ .

## 3.2.146 SDSS J183722.86+571407.2

The SDSS spectrum shows Balmer and He I emission lines. The object is midway between the main sequence and the white dwarf cooling sequence in the HR diagram. The CRTS light curve exhibits one outburst.

## 3.2.147 SDSS J183840.12+092222.5

The SDSS spectrum shows Balmer and He I emission lines. The object is close to the main sequence in the HR diagram. The ZTF and ATLAS light curves show frequent outbursts.

## 3.2.148 SDSS J184127.11+053821.9

The SDSS spectrum shows Balmer, He I and He II emission lines together with double-peaked Paschen emission lines. The He II line is over half the strength of the H $\beta$  line. The object is close to the main sequence in the HR diagram when reddening of  $E(B - V) = 0.58$  is accounted for. The ZTF light curve shows variability of  $\Delta m \approx 1.5$ , eclipses and frequent outbursts. We obtained a period of 7.6184 h from the ZTF light curve. Although we could not detect a spin period this is an intermediate polar.

*3.2.149 SDSS J185306.11–515722.1*

The SDSS spectrum shows Balmer emission lines. Both the donor and white dwarf signatures are visible in the spectrum. The object is close to the main sequence in the HR diagram. The *Gaia* light curve shows four outbursts and the ATLAS light curve shows frequent outbursts.

*3.2.150 SDSS J185333.52+223559.1*

The SDSS spectrum shows Balmer and He I emission lines. The object is on the main sequence in the HR diagram when reddening of  $E(B - V) = 0.23$  is accounted for. The ZTF light curve shows four outbursts. We obtained a period of 8.617 h from the ZTF light curve.

*3.2.151 SDSS J185721.58+131429.1*

This is V0466 Her, an old nova which erupted in 1960. It now shows the characteristics of a U Gem and we classify it accordingly.

*3.2.152 SDSS J190005.28–493034.6*

The SDSS spectrum shows double-peaked Balmer and He I lines. The signature of the white dwarf is visible in the spectrum whilst that of the donor is not. The object is midway between the main sequence and the white dwarf cooling sequence in the HR diagram.

*3.2.153 SDSS J190121.32–622804.4*

The SDSS spectrum shows double-peaked Balmer and He I emission lines. The object is midway between the main sequence and the white dwarf cooling sequence in the HR diagram. The CRTS light curve exhibits three outbursts whilst the ATLAS light curve shows two superoutbursts followed by the characteristic superhumps.

*3.2.154 SDSS J190243.24–483406.0*

The SDSS spectrum shows double-peaked Balmer and He I emission lines. Neither the white dwarf nor the donor are visible in the spectrum. The object is on the white dwarf cooling sequence in the HR diagram. The CRTS light curve exhibits an outburst ( $\Delta m \approx 4.5$  on MJD = 55676) whilst the ASAS-SN light curve shows five outbursts including one superoutburst. This superoutburst combined with the object's position in the HR diagram indicates that this is an SU UMa. The very deep central absorption in the Balmer lines is suggestive of a high inclination.

*3.2.155 SDSS J190342.14+534745.8*

The SDSS spectrum shows double-peaked Balmer and He I emission lines. The object is midway between the main sequence and the white dwarf cooling sequence in the HR diagram. The ZTF light curve exhibits multiple outbursts and superoutbursts.

*3.2.156 SDSS J190531.87–534944.4*

The SDSS spectrum shows double-peaked Balmer and He I emission lines. The object is midway between the main sequence and the white dwarf cooling sequence in the HR diagram. The CRTS light curve shows one outburst with  $\Delta m \approx 5$ . We obtained a tentative period of 3.2394(1) h from the CRTS light curve.

*3.2.157 SDSS J190651.05–114103.3*

The SDSS spectrum shows single-peaked Balmer emission lines above a blue continuum. The object is on the edge of the main sequence in the novalike area. The spectrum is consistent with the SED and the *Gaia* G – band magnitude and so is not in outburst or a high state. The *Gaia* light curve shows a temporary low level indicative of the VY Scl type of novalike. We obtained a tentative period of 3.96 h from the *Gaia* light curve.

*3.2.158 SDSS J190708.20–123552.9*

The SDSS spectrum shows weak Balmer emission lines above a blue continuum. The object is near the main sequence in the novalike area. The spectrum is not consistent with the SED and the *Gaia* G-band magnitude implying a possible low state. The ZTF light curve shows variability of  $\Delta m \approx 1$  with drop-outs of  $\Delta m \approx 2$ .

*3.2.159 SDSS J190811.74–634331.2*

The SDSS spectrum shows double-peaked Balmer and He I emission lines. The object is midway between the main sequence and the white dwarf cooling sequence in the HR diagram. The outburst noted by ASAS-SN confirms that this is a dwarf nova but the absence of light curve data precludes any further classification.

*3.2.160 SDSS J191339.74–614257.0*

Our noisy spectrum shows double-peaked Balmer and He I emission lines. The *Gaia* light curve shows two outbursts  $\Delta m \approx 4$ . There is no *Gaia* parallax available and we can therefore only classify this object as a dwarf nova.

*3.2.161 SDSS J191343.58–141831.6*

The spectrum shows asymmetric Balmer and He I emission lines. It is located closer to the main sequence than the white dwarf cooling sequence. The ZTF light curve shows frequent outbursts and also that it is eclipsing. We obtained a period of 3.728 h from the ZTF light curve which we refined to 3.72827(2) h using MDM photometry.

*3.2.162 SDSS J191421.38–135026.9*

The spectrum shows sharp, single-peaked Balmer, He I and He II emission lines. The spectrum is dominated by the donor, an M-dwarf. The object is next to the main sequence in the HR diagram. The ZTF light curve yields two periods, 5.14102(6) h and 0.447 h, but no outbursts. The folded ZTF light curve shows that this is deeply eclipsing with asymmetric eclipses, presumably due to the hot spot or accretion stream. This would appear to be an IP in a low state.

*3.2.163 SDSS J191534.92–620318.5*

Our noisy spectrum shows double-peaked Balmer and He I emission lines.

## 3.2.164 SDSS J192002.30–105446.5

The SDSS spectrum shows Balmer, and He I emission lines. Comparison with the SED shows that the spectrum was observed when the object was in a low state. The object is near the main sequence in the novalike area in the HR diagram. The ZTF light curve shows variability ( $\Delta m \simeq 0.5$ ) but no outbursts. The ZTF light curve shows two level changes ,

## 3.2.165 SDSS J192241.96+524359.0

The SDSS spectrum has a better S/N than that of Liu et al. (1999) and shows double-peaked Balmer, and He I emission lines.

## 3.2.166 SDSS J192336.67–514444.0

The SDSS spectrum shows double-peaked Balmer and He I emission lines. The object is midway between the main sequence and the white dwarf cooling sequence in the HR diagram. The CRTS light curve shows four outbursts ( $\Delta m \simeq 4.5$ ). We obtained a tentative period of 3.8842(1) h from the CRTS photometry.

## 3.2.167 SDSS J192513.82–521137.3

The SDSS spectrum shows double-peaked Balmer and He I emission lines. From the SED the spectrum was observed during quiescence. The object is midway between the main sequence and the white dwarf cooling sequence in the HR diagram. The CRTS light curve shows frequent outbursts ( $\Delta m \simeq 2$ ).

## 3.2.168 SDSS J192554.81–461903.5

The spectrum shows single-peaked Balmer and He I emission lines above a blue continuum. The object is next to the main sequence in the HR diagram. The synthetic *G*-band magnitude is 16.2 whilst the *Gaia* is 18.45 indicating that our spectrum probably occurred during an outburst. The CRTS and *Gaia* alerts light curves show frequent outbursts with an apparent standstill in the CRTS light curve.

## 3.2.169 SDSS J192609.70+611312.7

The SDSS spectrum shows double-peaked Balmer and He I emission lines. From the SED the spectrum was observed during quiescence. The object is next to the main sequence in the HR diagram. The ZTF light curve shows at least five outbursts ( $\Delta m = 1 - 2$ ). Chen et al. (2020) classify this as a “EW-type eclipsing binary” but we believe that this is a U Gem.

## 3.2.170 SDSS J192610.82–101530.6

The SDSS spectrum shows single-peaked Balmer and He I emission lines. The H $\beta$  and higher Balmer lines are sitting in the absorption lines from the white dwarf. The object is midway between the main sequence and the white dwarf cooling sequence in the HR diagram.

## 3.2.171 SDSS J192632.51–011612.0

The SDSS spectrum shows Balmer emission lines with no sign of the white dwarf or donor. The object is located midway between the main sequence and the white dwarf cooling sequence when reddening of  $E(B - V) = 0.23$  is accounted for. The ZTF light curve shows seven outbursts.

## 3.2.172 SDSS J192634.45+073613.8

The SDSS spectrum shows single-peaked Balmer lines above the spectrum of the donor. The object is located on the left of the main sequence in the HR diagram when reddening of  $E(B - V) = 0.38$  is accounted for.

## 3.2.173 SDSS J192710.18–484752.7

The SDSS spectrum shows double-peaked Balmer emission lines. The CRTS light curve shows seven outbursts.

## 3.2.174 SDSS J192739.29+020013.8

The SDSS spectrum shows double-peaked Balmer and He I emission lines. The object is closer to the main sequence than the white dwarf cooling sequence in the HR diagram. The ZTF light curve shows at least twelve outbursts ( $\Delta m = 4 - 5$ ).

## 3.2.175 SDSS J192830.04–741053.1

The spectrum shows single-peaked Balmer emission lines. The object is on the main sequence in the HR diagram and the donor signature is visible in the spectrum. The *TESS* light curve yields a period of 5.991(3) h. Vsnnet-alert 23569 reported a period of 2.99638 h, however this is half the orbital period as our folded light curve clearly shows ellipsoidal modulation.

## 3.2.176 SDSS J192832.32–500134.9

The SDSS spectrum shows Balmer, He I and He II emission lines. The object is located midway between the main sequence and the white dwarf cooling sequence. There is an *XMM* X-ray detection in the range 0.1 – 12 keV. We obtained a period of 1.68373(1) h from the *TESS* photometry.

## 3.2.177 SDSS J193149.51+094939.4

The SDSS spectrum shows single-peaked Balmer emission lines above a red continuum dominated by the donor. The object is located next to the main sequence in the HR diagram when reddening of  $E(B - V) = 0.42$  is accounted for. The ZTF and *Gaia* light curves show outbursts.

## 3.2.178 SDSS J193430.49+020110.3

The SDSS spectrum shows double-peaked Balmer and He I emission lines. The object is located midway between the main sequence and the white dwarf cooling sequence. The ZTF light curve shows at least seven outbursts.

3.2.179 *SDSS J193436.19+510742.1*

See main paper.

3.2.180 *SDSS J193436.97+100213.3*

The SDSS spectrum shows single-peaked Balmer and He I emission lines. The object is located near the main sequence in the HR diagram when reddening of  $E(B - V) = 0.29$  is accounted for. The ZTF and *Gaia* light curves show frequent outbursts of  $\Delta m \simeq 4$ .

3.2.181 *SDSS J193511.46-531745.8*

See main paper.

3.2.182 *SDSS J194124.99+152254.2*

Cyclotron humps yield an estimate of  $B \simeq 32$  MG. We confirm the classification as a polar.

3.2.183 *SDSS J194139.92+214557.8*

We obtained a period of 4.5758 h from the *TESS* light curve.

3.2.184 *SDSS J194255.82-672725.6*

The SDSS spectrum shows Balmer and He I emission lines. The object is located midway between the main sequence and the white dwarf cooling sequence. The CRTS light curve shows variability  $\Delta m \simeq 2$ . ASAS-SN reported an outburst of  $\Delta m = 16.1$ .

3.2.185 *SDSS J194309.99+093227.9*

The SDSS spectrum shows Balmer and He I emission lines. The object is located next to the main sequence when reddening of  $E(B - V) = 0.3$  is accounted for. The ZTF light curve shows three outbursts.

3.2.186 *SDSS J194829.02-562939.5*

The SDSS spectrum shows Balmer, He I and He II emission lines. The object is located midway between the main sequence and the white dwarf cooling sequence. The CRTS light curve shows five outbursts.

3.2.187 *SDSS J194910.48+583159.4*

[Thorstensen et al. \(2010\)](#) found a spectroscopic period of 4.36 h. We found a more precise period of 4.3518(23) h from *TESS* photometry.

3.2.188 *SDSS J194947.62+031304.8*

The SDSS spectrum shows double-peaked Balmer emission lines and also absorption lines from the white dwarf. These Balmer lines rule out previous suggestions that this might be an AM CVn. The ZTF light curve shows frequent outbursts ( $\Delta m \simeq 5$ ) consistent with the classification of SU UMa. We find a tentative period of 1.563 h from the ZTF light curve.

3.2.189 *SDSS J195039.55+055619.9*

The SDSS spectrum shows Balmer and He I emission lines. The object is located midway between the main sequence and the white dwarf cooling sequence. The ZTF light curve shows multiple outbursts and two probable superoutbursts.

3.2.190 *SDSS J195512.47+004536.3*

We obtained a period of 1.35549(3) h from the *TESS* light curve which is more precise than the photometric period in [Tovmassian et al. \(2017\)](#).

3.2.191 *SDSS J200504.93+322122.5*

See main paper.

3.2.192 *SDSS J200611.52+334237.5*

Vsnet 13294 reported a tentative period of 2.42 h. We obtained a period of 9.586(2) h from the *TESS* photometry.

3.2.193 *SDSS J200622.88+031935.3*

The SDSS spectrum shows dual-peaked Balmer emission lines and also the white dwarf signature. The object is located midway between the main sequence and the white dwarf cooling sequence. The ZTF light curve shows four outbursts including a probable superoutburst.

3.2.194 *SDSS J200703.00+051927.3*

The SDSS spectrum shows dual-peaked Balmer and He I emission lines. The object is located near the main sequence. The ZTF and ATLAS light curves show frequent outbursts.

3.2.195 *SDSS J200754.82+032738.0*

The SDSS spectrum shows Balmer and He I emission lines. The object is located midway between the main sequence and the white dwarf cooling sequence. The ZTF light curve shows four outbursts.

3.2.196 *SDSS J200946.47+042232.6*

The SDSS spectrum shows Balmer and He I emission lines. The object is located midway between the main sequence and the white dwarf cooling sequence. The ZTF light curve shows many outbursts including two probable superoutbursts.

3.2.197 *SDSS J201116.80+600428.1*

The SDSS spectrum shows Balmer, He I and He II emission lines. The object is closer to the main sequence than the white dwarf cooling sequence in the HR diagram when reddening of  $E(B - V) = 0.16$  is accounted for. The spectrum is consistent with the existing classification of IP.



## 3.2.198 SDSS J201135.94+025435.1

The SDSS spectrum shows Balmer, He I and He II emission lines. The signature of the white dwarf is visible. The object is close to the main sequence in the HR diagram when reddening of  $E(B-V) = 0.1$  is accounted for. This is likely to be the optical counterpart to an *XMM* X-ray detection in the range 0.1 – 12 keV. The ZTF light curve shows variability. We obtained a period of 0.5307 h from the ZTF light curve indicative of an intermediate polar.

## 3.2.199 SDSS J201403.80–540624.9

Our two spectra show Balmer and He I emission lines. The object is located midway between the main sequence and the white dwarf cooling sequence. The CRTS light curve shows three outbursts.

## 3.2.200 SDSS J201439.78–093715.2

The SDSS spectrum shows Balmer and He I emission lines. The object is located midway between the main sequence and the white dwarf cooling sequence. The ASAS-SN light curve shows two outbursts.

## 3.2.201 SDSS J202206.39–565101.7

Our two spectra show Balmer and He I emission lines. The object is located midway between the main sequence and the white dwarf cooling sequence. The ATLAS light curve shows multiple outbursts. We obtained a period of 5.4895(6) h from the ATLAS photometry.

## 3.2.202 SDSS J202422.01–083744.3

The SDSS spectrum shows Balmer and He I emission lines. The object is located midway between the main sequence and the white dwarf cooling sequence. The ZTF light curve shows two outbursts.

## 3.2.203 SDSS J202543.97–582334.2

The spectrum shows double-peaked Balmer and He I emission lines. The object is next to the main sequence in the HR diagram. The *Gaia* alerts light curve shows outbursts. We obtained a period of 5.312 h from the *TESS* light curve.

## 3.2.204 SDSS J202640.97+045901.2

The SDSS spectrum shows single-peaked Balmer, He I and He II emission lines. The object is located midway between the main sequence and the white dwarf cooling sequence in the HR diagram. The ZTF light curve shows variability ( $\Delta m \approx 2$ ) but no outbursts. We obtained a period of 3.9992(4) h from the ZTF light curve. We classify this object as a polar based on the strength of the He II emission line.

## 3.2.205 SDSS J202642.06–572154.5

The SDSS spectrum shows Balmer and He I emission lines. The signature of the white dwarf is visible. The object is located closer to the white dwarf cooling sequence than the main sequence. The CRTS light curve shows five outbursts ( $\Delta m \approx 5$ ). This is a dwarf nova and probably an SU UMa.

## 3.2.206 SDSS J202857.08–061803.5

The SDSS spectrum shows double-peaked Balmer and He I emission lines. The object is closer to the main sequence than the white dwarf cooling sequence in the HR diagram. The ZTF light curve shows at least eight outbursts including several superoutbursts with superhumps.

## 3.2.207 SDSS J203134.50+030422.0

The SDSS spectrum shows double-peaked Balmer and He I emission lines. The object is located midway between the main sequence and the white dwarf cooling sequence in the HR diagram. The ZTF light curve shows at least eight outbursts including several superoutbursts with superhumps.

## 3.2.208 SDSS J203337.17–563345.4

Our two spectra show double-peaked Balmer and He I emission lines. The object is next to the main sequence in the HR diagram. The CRTS light curve shows three outbursts ( $\Delta m \approx 3$ ). We obtained a period of 4.876360(1) h from the *TESS* light curve.

## 3.2.209 SDSS J203501.48–001946.3

The SDSS spectrum shows double-peaked Balmer and He I emission lines. The object is located midway between the main sequence and the white dwarf cooling sequence in the HR diagram. The ZTF light curve shows multiple outbursts ( $\Delta m \approx 3$ ).

## 3.2.210 SDSS J203529.78+063652.7

The SDSS spectrum shows double-peaked Balmer and He I emission lines. The object is located closer to the main sequence than the white dwarf cooling sequence in the HR diagram. The ZTF light curve shows multiple outbursts.

## 3.2.211 SDSS J204247.17–604524.2

The *Gaia* light curve is consistent with the classification of novalike proposed by Oliveira et al. (2017).

## 3.2.212 SDSS J204522.73–011004.5

The SDSS spectrum shows double-peaked Balmer and He I emission lines. The object is located midway between the main sequence and the white dwarf cooling sequence in the HR diagram. The ZTF light curve shows one outburst.

## 3.2.213 SDSS J204643.26–000630.2

The spectrum shows single-peaked Balmer emission lines above a blue continuum. The object is located in the novalike area of the HR diagram. The ZTF light curve shows variability but no outbursts. The ZTF light curve also shows a deep low state indicative of the VY Scl subtype of a novalike. We therefore classify this as a novalike.

3.2.214 *SDSS J205110.37+044842.1*

The SDSS spectrum shows double-peaked Balmer and He I emission lines. The object is located midway between the main sequence and the white dwarf cooling sequence in the HR diagram. This is consistent with the previous classification of SU UMa.

3.2.215 *SDSS J205227.38+034355.2*

Our noisy ( $S/N = 2.0$ ) spectrum shows a double-peaked H $\alpha$  emission line. The object is located closer to the main sequence than the white dwarf sequence in the HR diagram although the *Gaia* parallax is negative and hence the position is not reliable. The ZTF light curve shows one outburst ( $\Delta m \simeq 5$ )

3.2.216 *SDSS J205305.37+591732.2*

Our two spectra show double-peaked Balmer and He I emission lines. The object is next to the main sequence in the HR diagram and the donor signature is visible in the spectrum. The ZTF light curve shows one outburst. The level of the light curve varies between  $m = 17.5$  and  $m = 19$ . The *Gaia* light curve shows a more constant level ( $m \simeq 18$ ) and one outburst ( $m = 15.0$ ).

3.2.217 *SDSS J205705.32-072426.1*

The SDSS spectrum shows double-peaked Balmer, He I and He II emission lines. The object is located nearer the white dwarf cooling sequence than the main sequence in the HR diagram. The ZTF light curve shows level changes ( $\Delta m \simeq 21$ ) and two outbursts.

3.2.218 *SDSS J205931.86-070516.9*

Our noisy ( $S/N = 2.1$ ) spectrum shows double-peaked Balmer and He I emission lines. There is no *Gaia* parallax but from its colours ( $G_{BP} - G_{RP} = -0.2$ ) this object must lie close to the white dwarf cooling sequence. The ZTF light curve shows six outbursts and one probable superoutburst. We tentatively classify this as an SU UMa.

3.2.219 *SDSS J210720.93-022145.9*

The SDSS spectrum shows double-peaked Balmer and He I emission lines. The signature of the white dwarf is visible and there is no sign of the donor. The object is close to the white dwarf cooling sequence. The ZTF and CRTS light curves do not show any outbursts. We tentatively classify this as a WZ Sge.

3.2.220 *SDSS J211312.23-590715.2*

The SDSS spectrum shows double-peaked Balmer and He I emission lines. The signature of the white dwarf is visible and there is no sign of the donor. The object is on the white dwarf cooling sequence. The ASAS-SN light curve shows three outbursts. We tentatively classify this as an SU UMa.

3.2.221 *SDSS J211508.00+015715.1*

The SDSS spectrum shows double-peaked Balmer and He I emission lines. The object is located midway between the main sequence and the white dwarf cooling sequence in the HR diagram. The ZTF light curve shows four outbursts one of which appears to have superhumps. We tentatively classify this as an SU UMa.

3.2.222 *SDSS J212521.76-102628.3*

The SDSS spectrum shows double-peaked Balmer and He I emission lines. The object is located midway between the main sequence and the white dwarf cooling sequence in the HR diagram. The ZTF light curve shows seven outbursts several of which appear to be superoutbursts. This is all consistent with the existing classification of SU UMa.

3.2.223 *SDSS J214804.43+080950.3*

The SDSS spectrum shows double-peaked Balmer and He I emission lines. The signature of the white dwarf is visible and there is no sign of the donor. There is no *Gaia* parallax but from the *Gaia* colours the object must lie close to the white dwarf cooling sequence in the HR diagram. The ZTF light curve shows two outbursts leading to the dwarf nova classification.

3.2.224 *SDSS J215637.24-632655.5*

The SDSS spectrum shows double-peaked Balmer and He I emission lines. The signature of the white dwarf is visible and there is no sign of the donor. The object is midway between the main sequence and the white dwarf cooling sequence in the HR diagram. The CRTS and *Gaia* light curves each show an outburst. We obtained a period of 1.573377(1) h from the *TESS* photometry.

3.2.225 *SDSS J220542.33+033917.1*

The SDSS spectrum shows double-peaked Balmer and He I emission lines. The signature of the white dwarf is visible and there is no sign of the donor. The object is midway between the main sequence and the white dwarf cooling sequence in the HR diagram. The ZTS light curve shows multiple outbursts including one probable superoutburst. We therefore tentatively classify this as an SU UMa.

3.2.226 *SDSS J220630.83-524419.8*

The spectrum shows H $\alpha$  and H $\beta$  emission lines above a blue continuum. The synthetic magnitude shows that the object was in outburst when the spectrum was taken. It is located closer to the main sequence than the white dwarf cooling sequence. The CRTS light curve shows multiple outbursts. We obtained a period of 3.9091(2) h from the *TESS* photometry.

3.2.227 *SDSS J220807.49+021618.8*

The SDSS spectrum shows single-peaked Balmer and He I emission lines. The object is on the main sequence in the HR diagram. The CRTS and ZTF light curves show multiple outbursts. We obtained a tentative period of 5.398(1) h from the CRTS photometry.

3.2.228 *SDSS J233737.44-604358.2*

The spectrum shows double-peaked Balmer and He I emission lines. It is located midway between the main sequence and the white dwarf cooling sequence. The *Gaia* alerts light curve shows at least two outbursts.



### 3.2.229 SDSS J234955.19–605417.1

The spectrum shows double-peaked Balmer emission lines. The object is nearer the white dwarf cooling sequence than the main sequence in the HR diagram. The CRTS light curve shows three outbursts. The ASAS-SN light curve shows five outbursts and two superoutbursts.

## 4 SPECTRA AND LIGHT CURVES

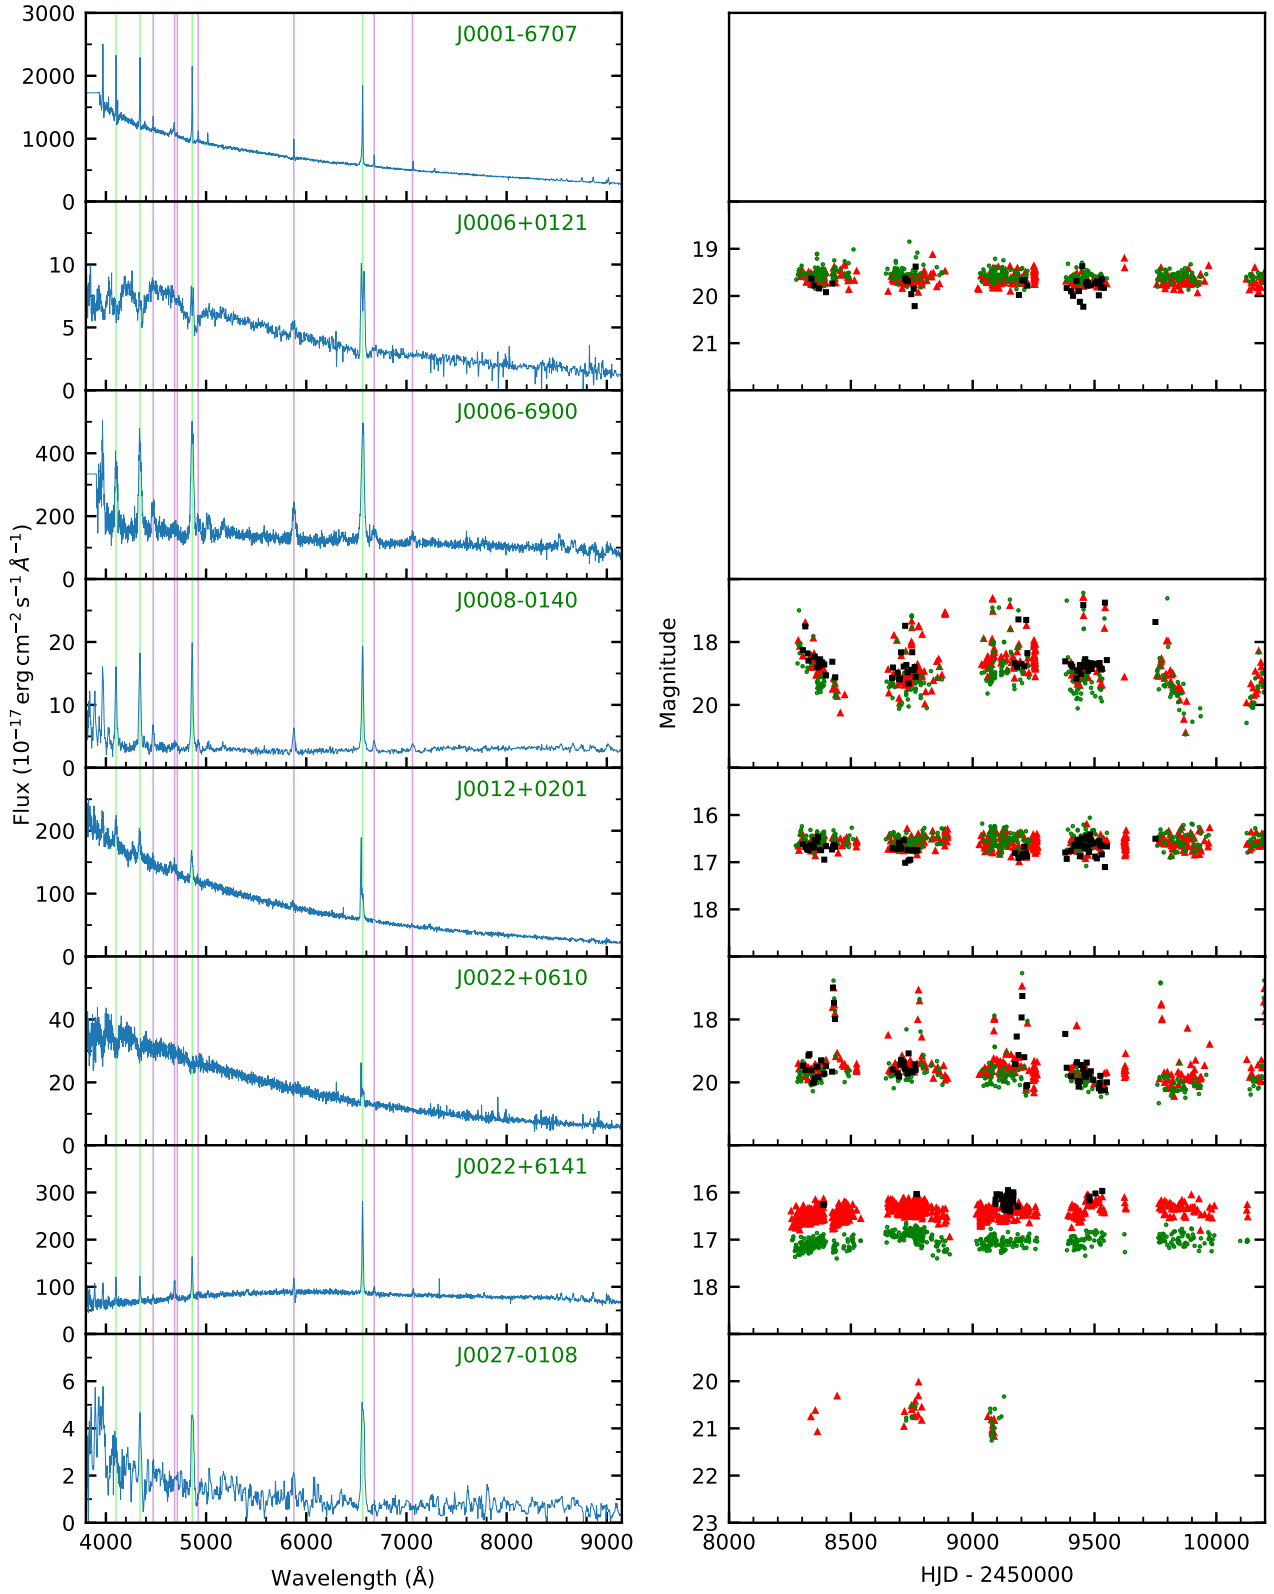

Figure 1: Left panels: Spectra with H lines shown in green and He in pink. Right panels: Light curves with ZTF *r*-band shown in red triangles, *g*-band in green dots and *i*-band in black squares.

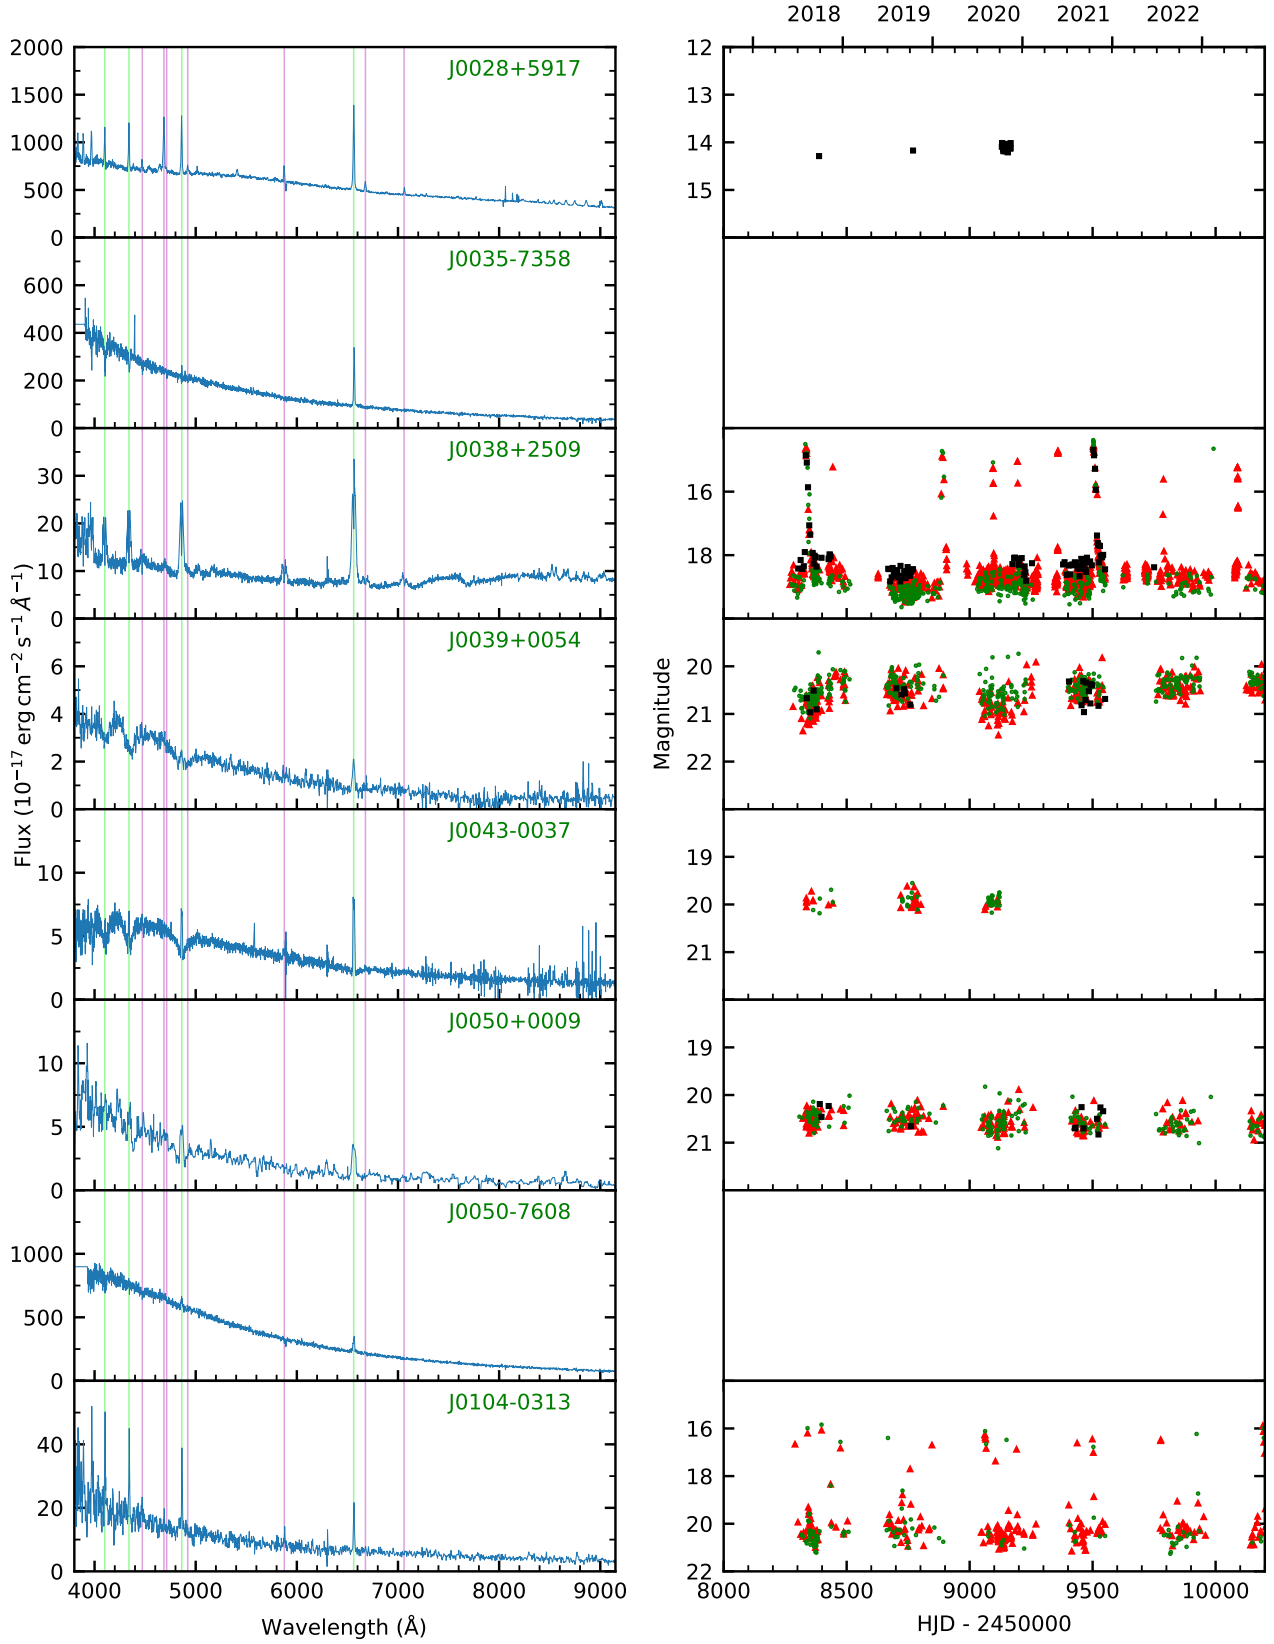

Figure 2: Left panels: Spectra with H lines shown in green and He in pink. Right panels: Light curves with ZTF  $r$ -band shown in red triangles,  $g$ -band in green dots and  $i$ -band in black squares.

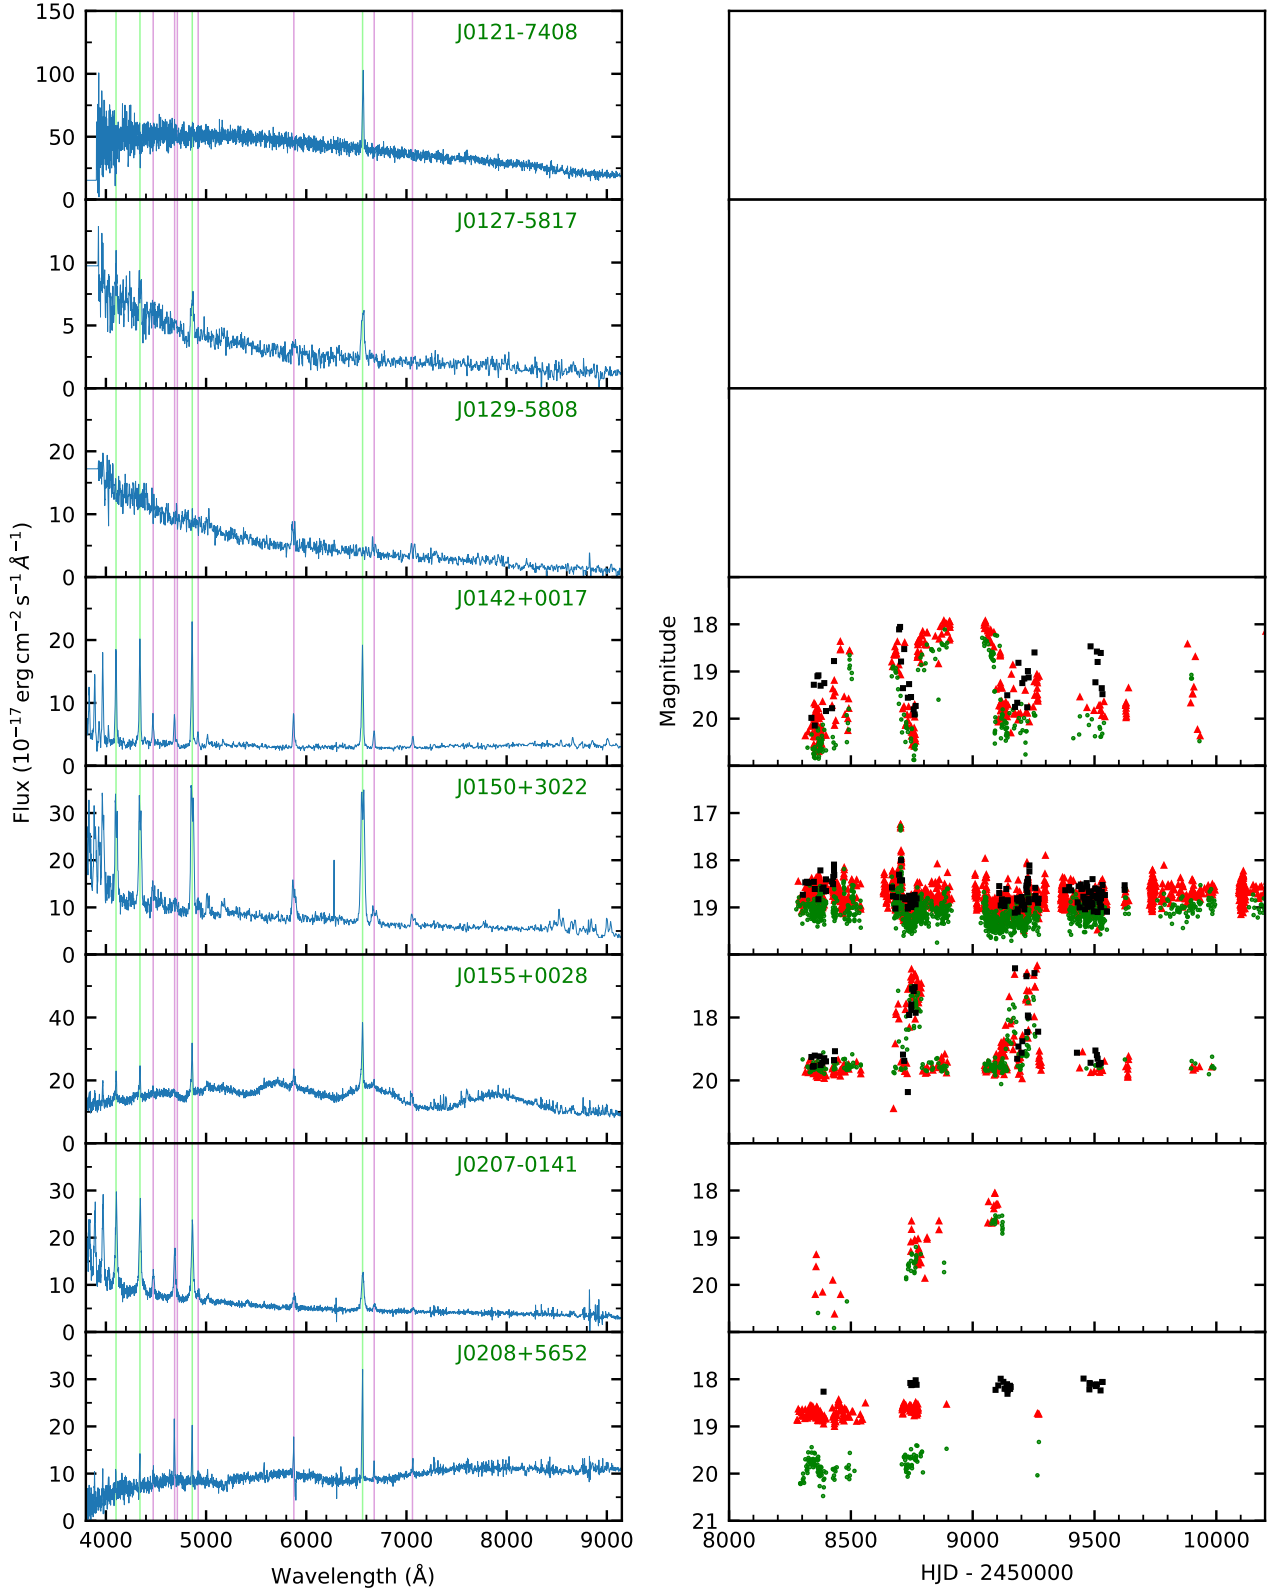

Figure 3: Left panels: Spectra with H lines shown in green and He in pink. Right panels: Light curves with ZTF *r*-band shown in red triangles, *g*-band in green dots and *i*-band in black squares.

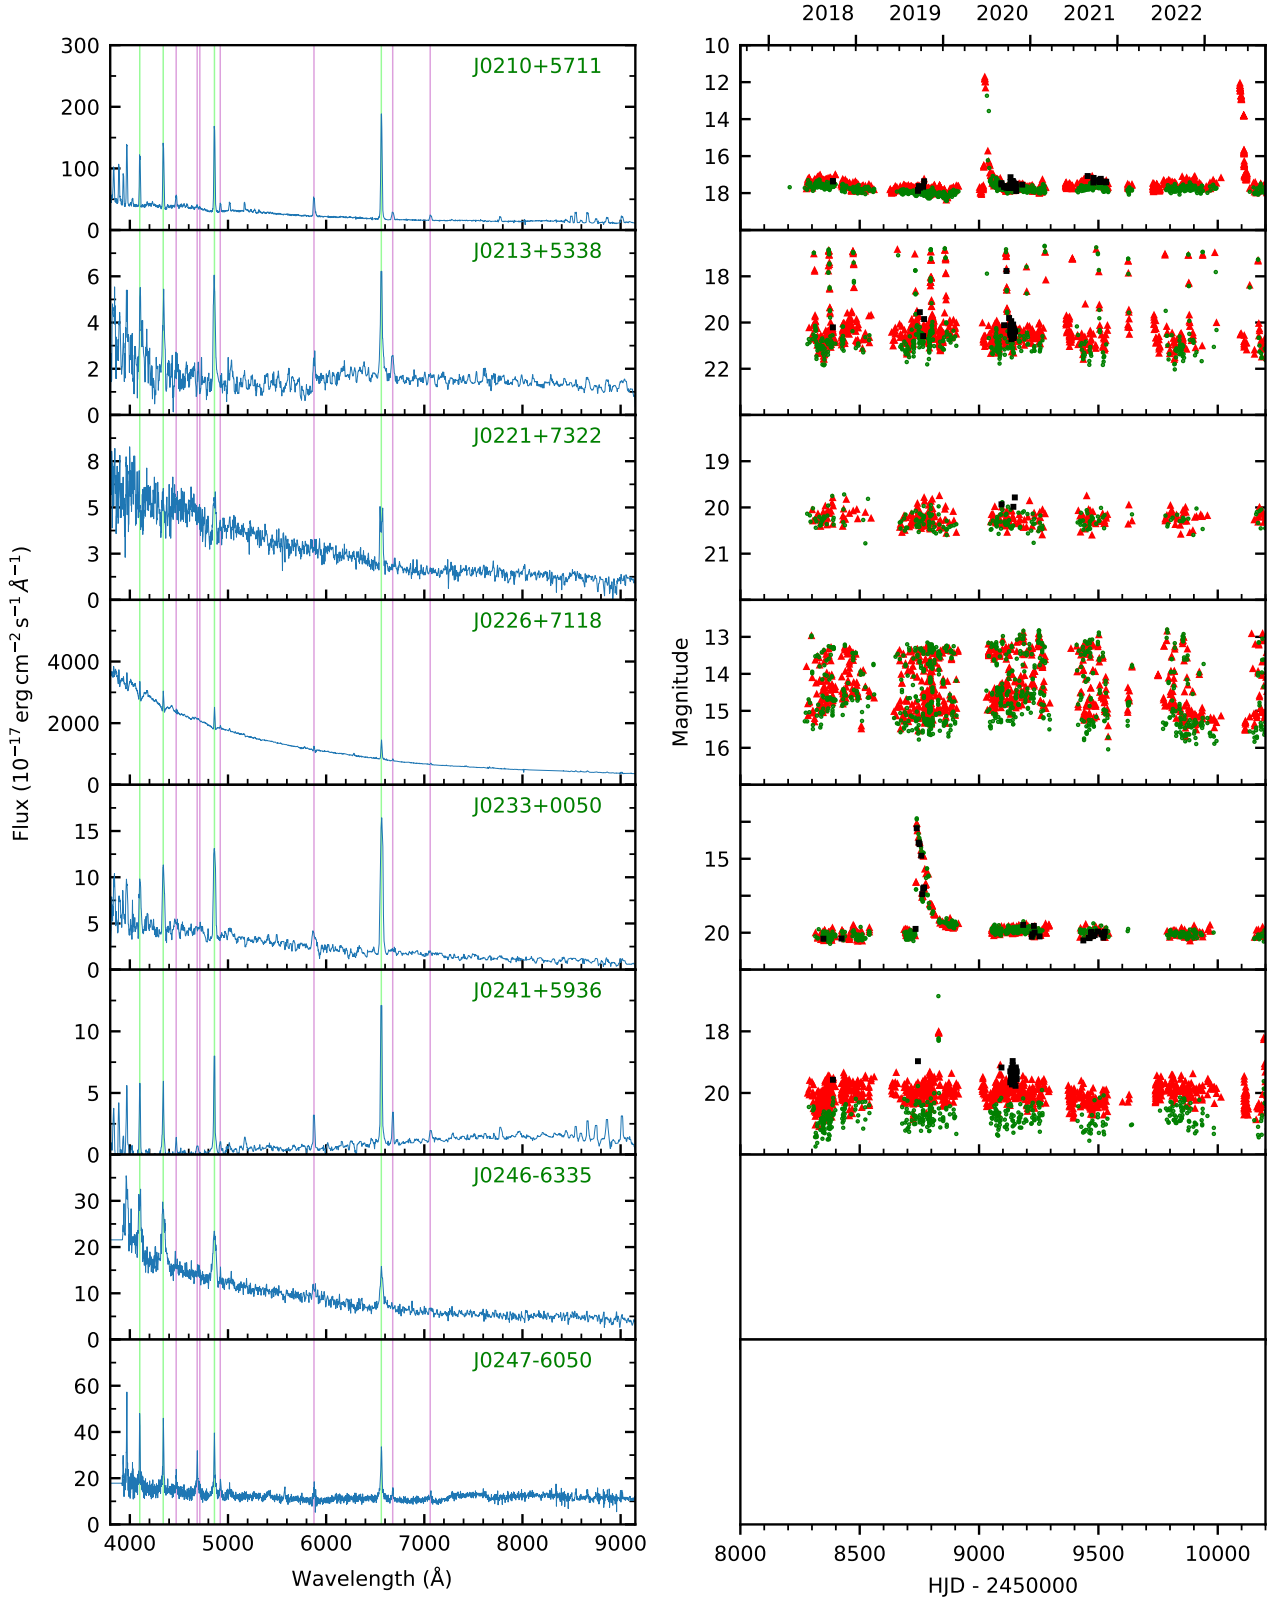

Figure 4: Left panels: Spectra with H lines shown in green and He in pink. Right panels: Light curves with ZTF *r*-band shown in red triangles, *g*-band in green dots and *i*-band in black squares.



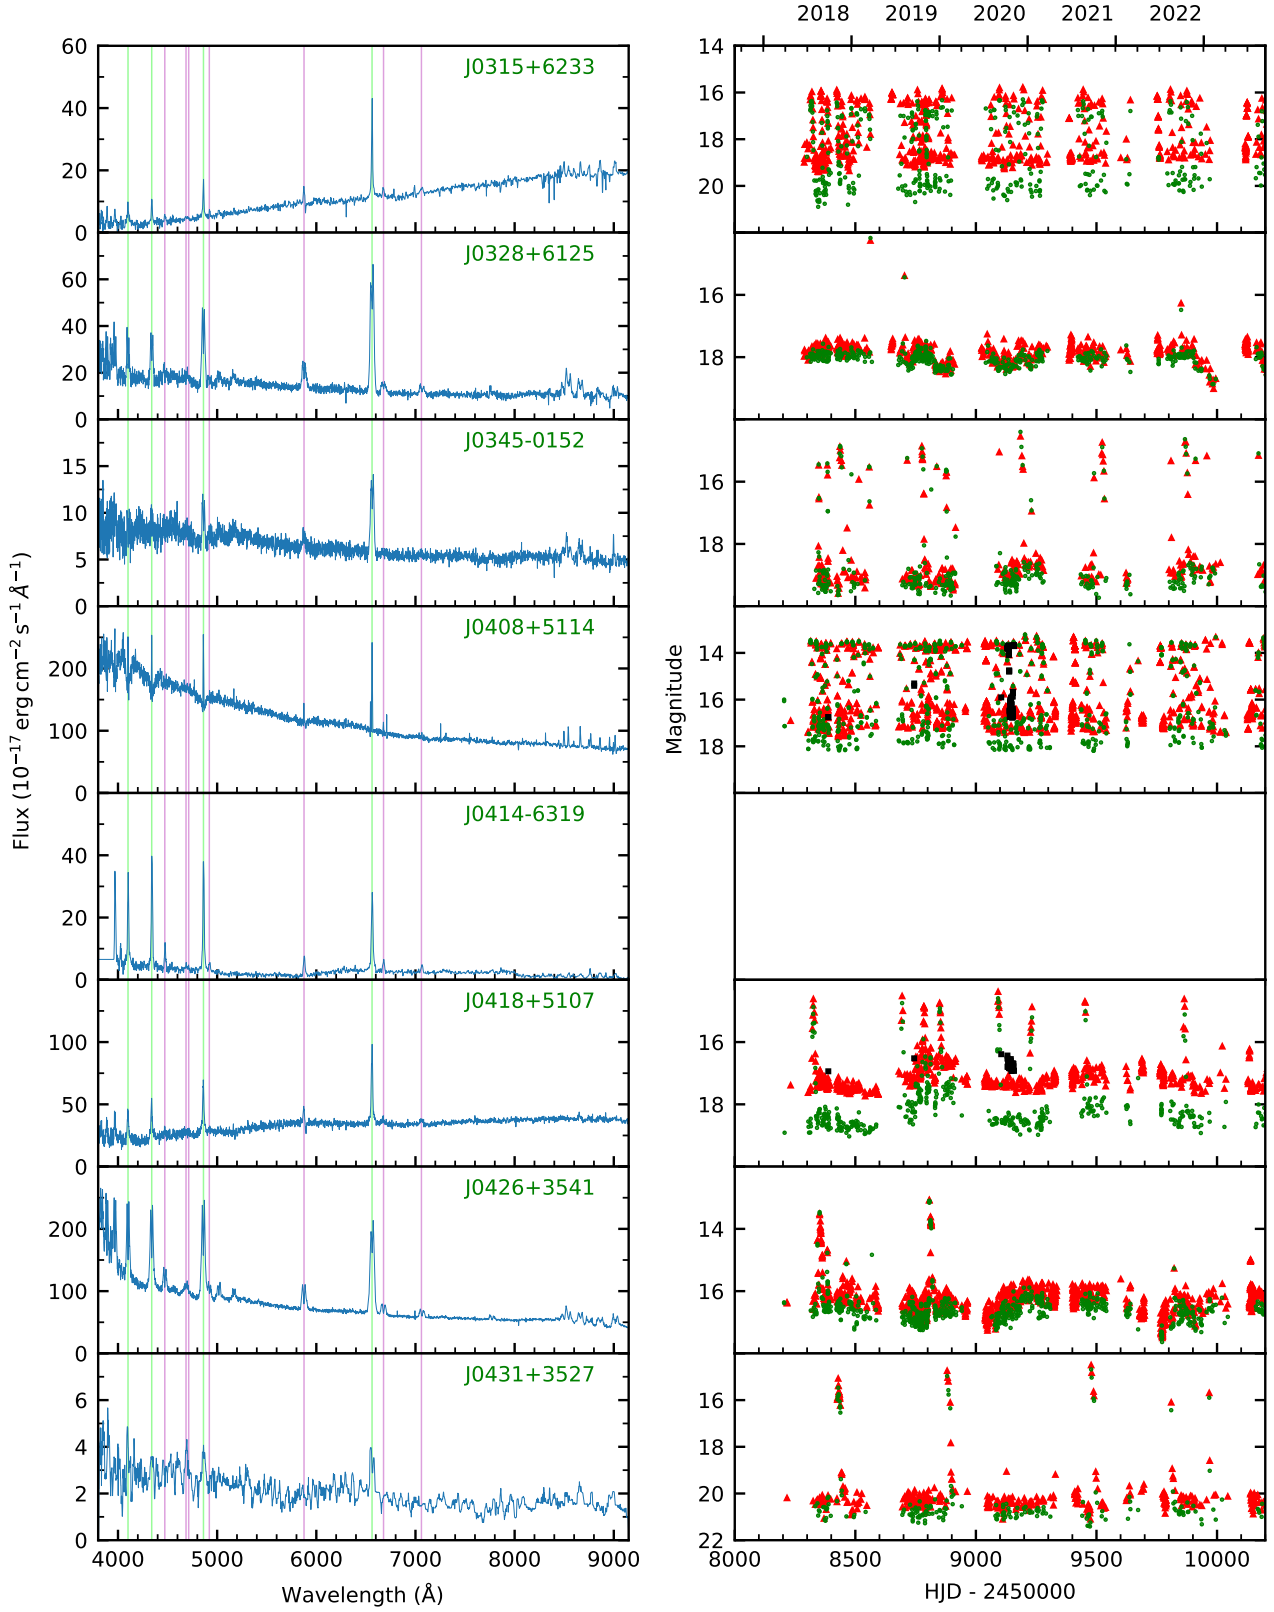

Figure 5: Left panels: Spectra with H lines shown in green and He in pink. Right panels: Light curves with ZTF *r*-band shown in red triangles, *g*-band in green dots and *i*-band in black squares.

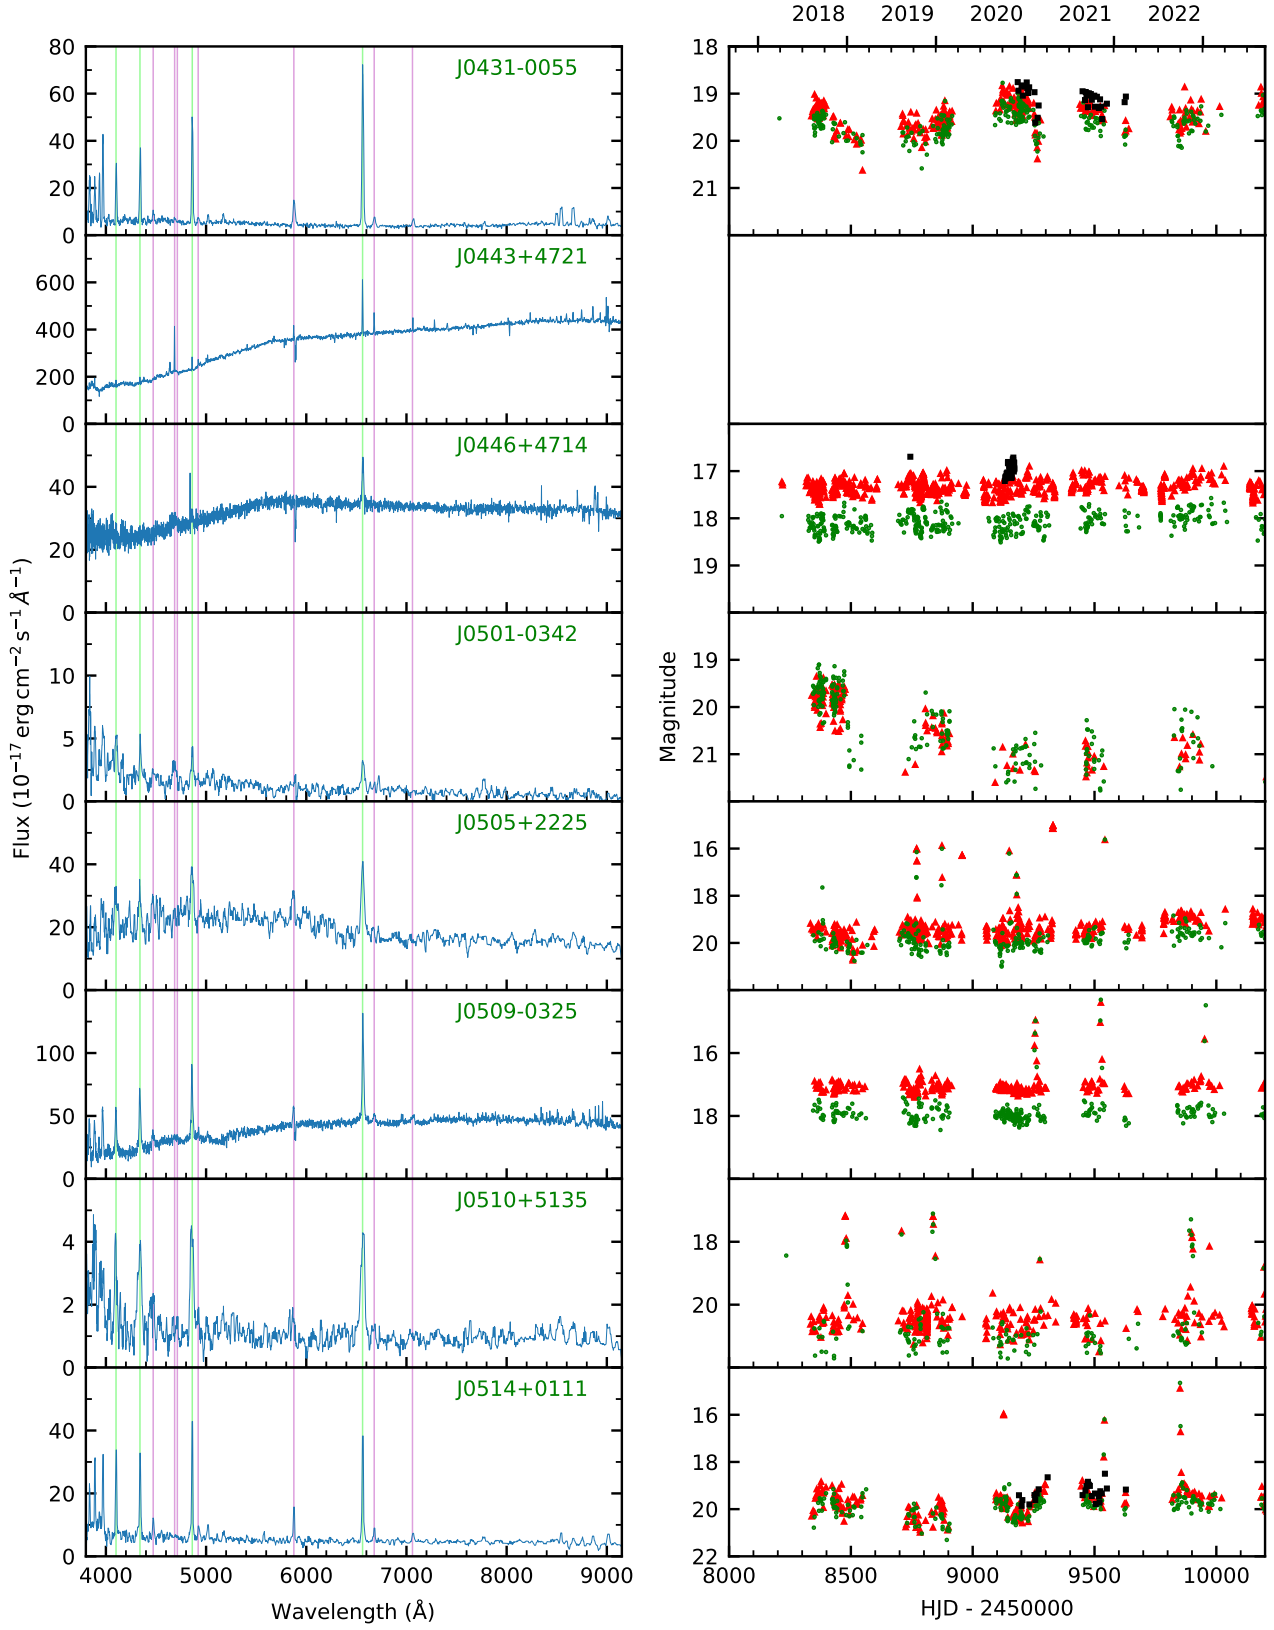

Figure 6: Left panels: Spectra with H lines shown in green and He in pink. Right panels: Light curves with ZTF  $r$ -band shown in red triangles,  $g$ -band in green dots and  $i$ -band in black squares.

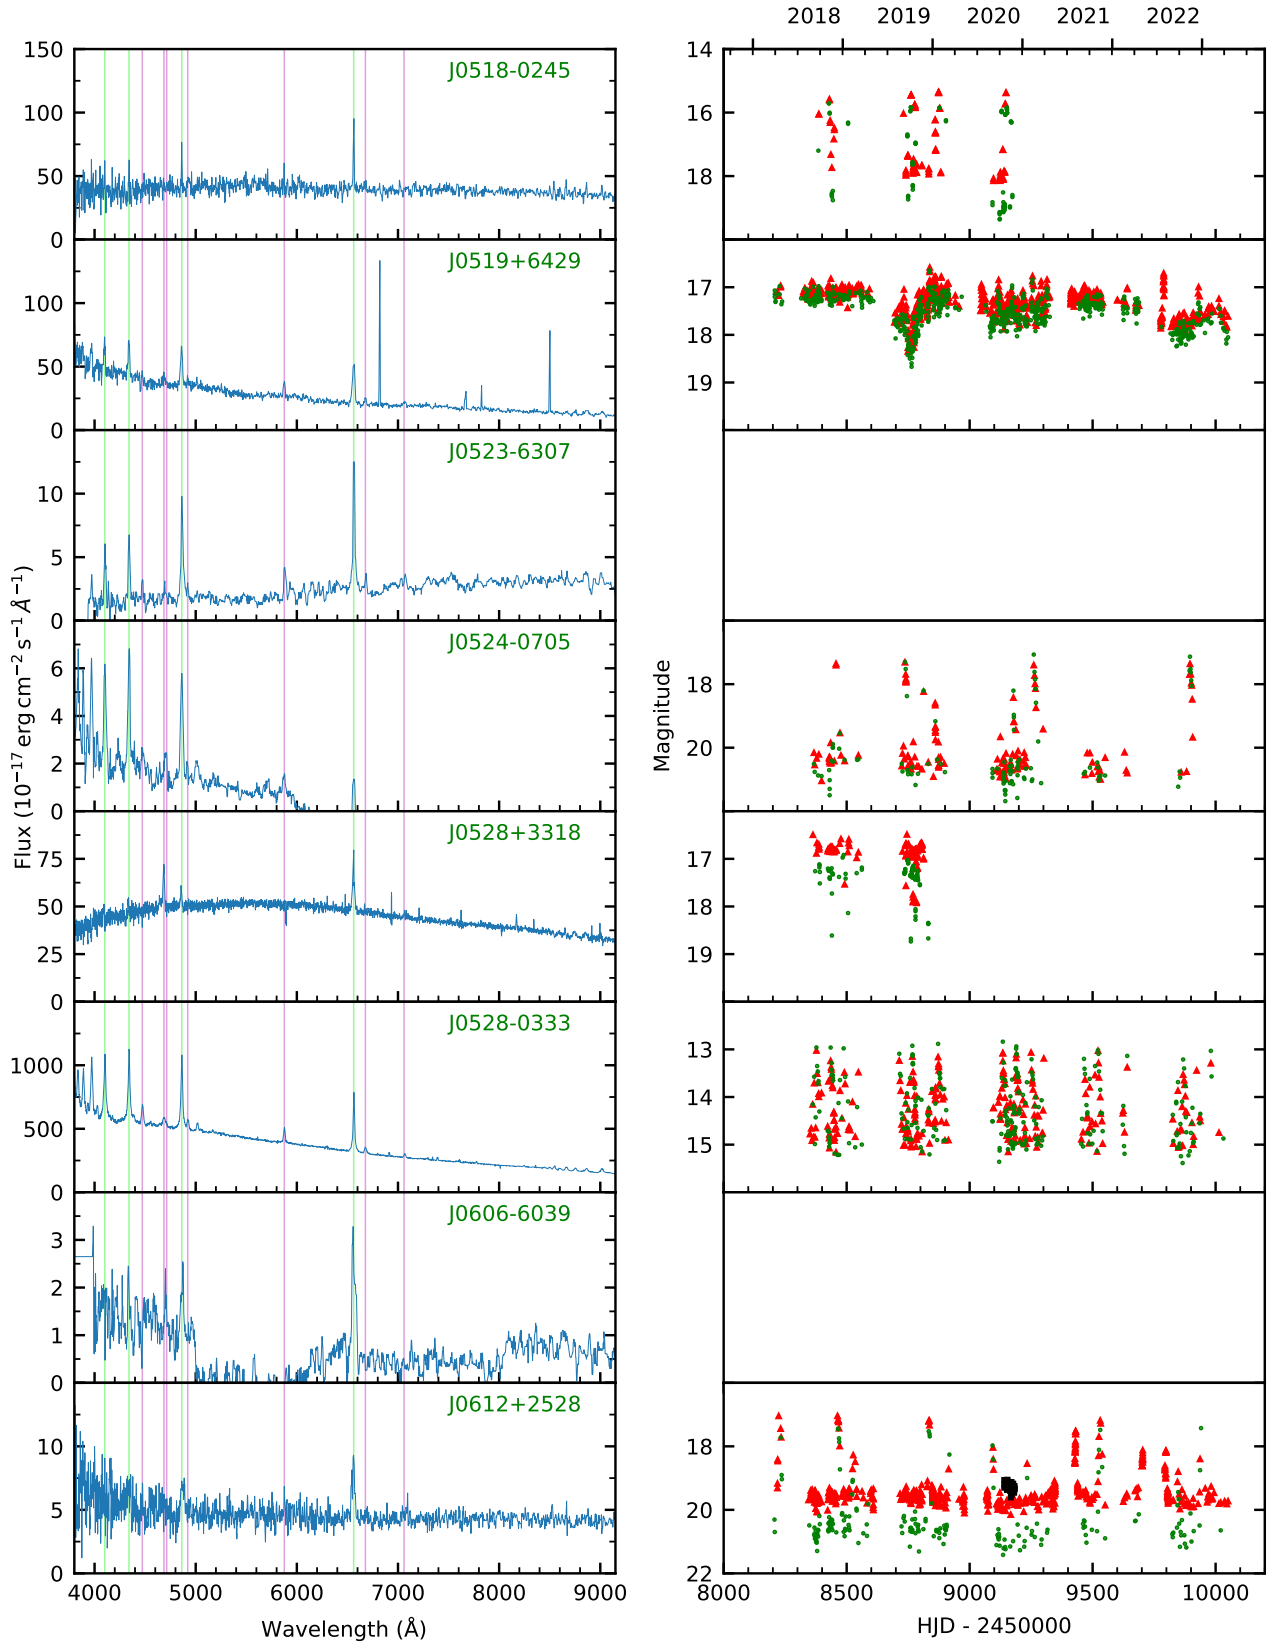

Figure 7: Left panels: Spectra with H lines shown in green and He in pink. Right panels: Light curves with ZTF *r*-band shown in red triangles, *g*-band in green dots and *i*-band in black squares.

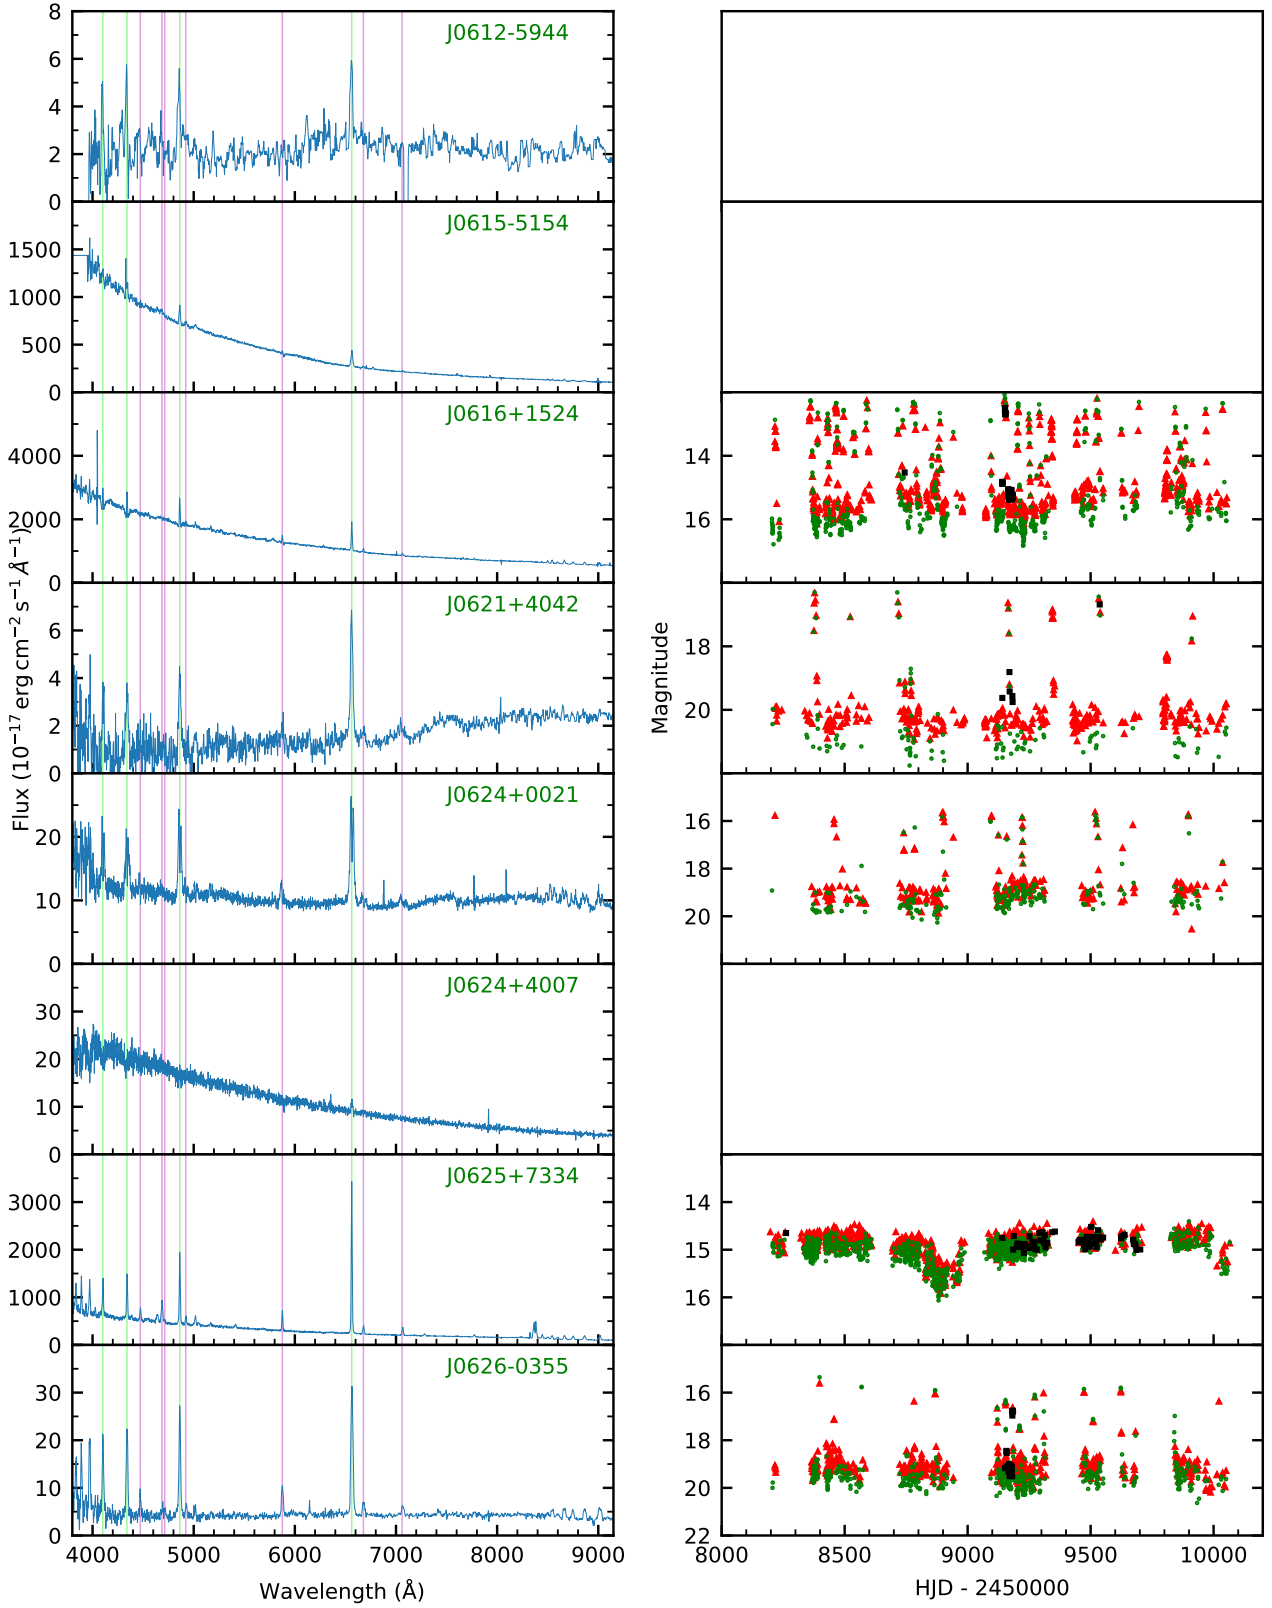

Figure 8: Left panels: Spectra with H lines shown in green and He in pink. Right panels: Light curves with ZTF *r*-band shown in red triangles, *g*-band in green dots and *i*-band in black squares.

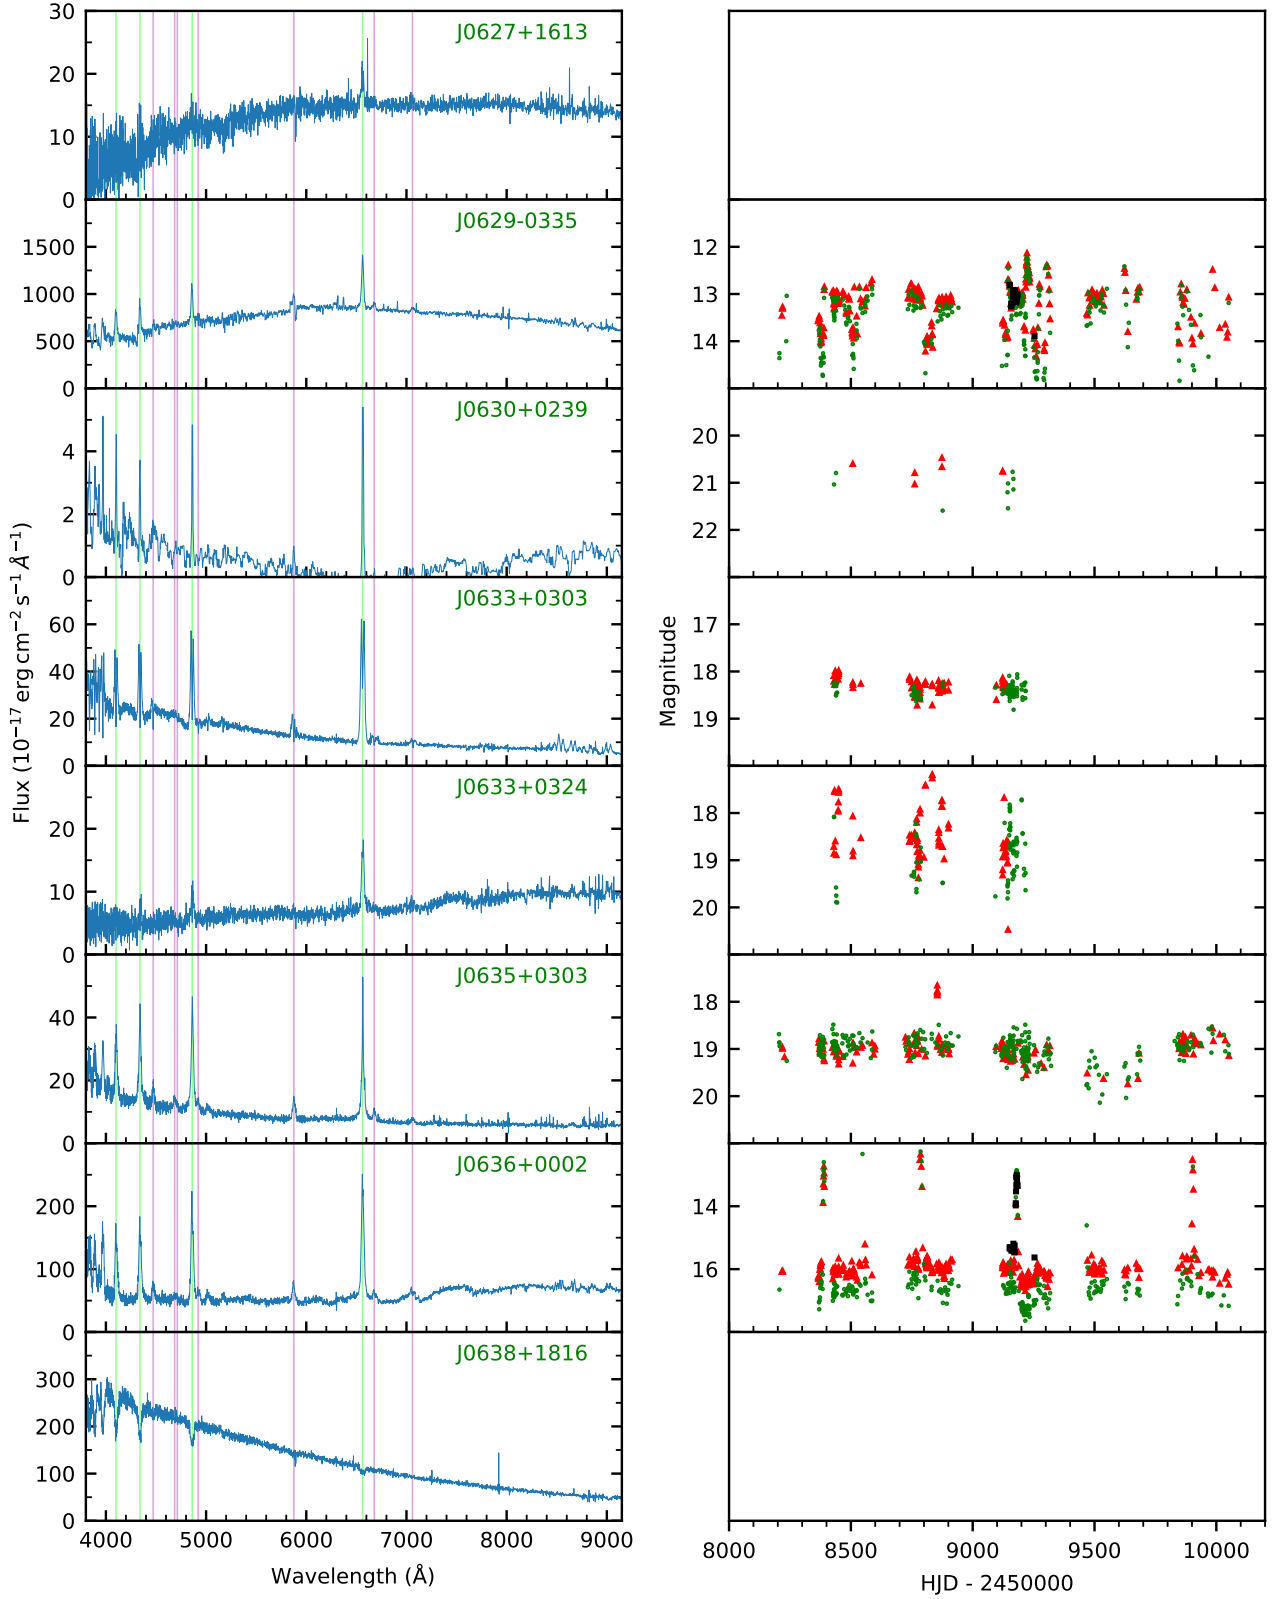

Figure 9: Left panels: Spectra with H lines shown in green and He in pink. Right panels: Light curves with ZTF *r*-band shown in red triangles, *g*-band in green dots and *i*-band in black squares.



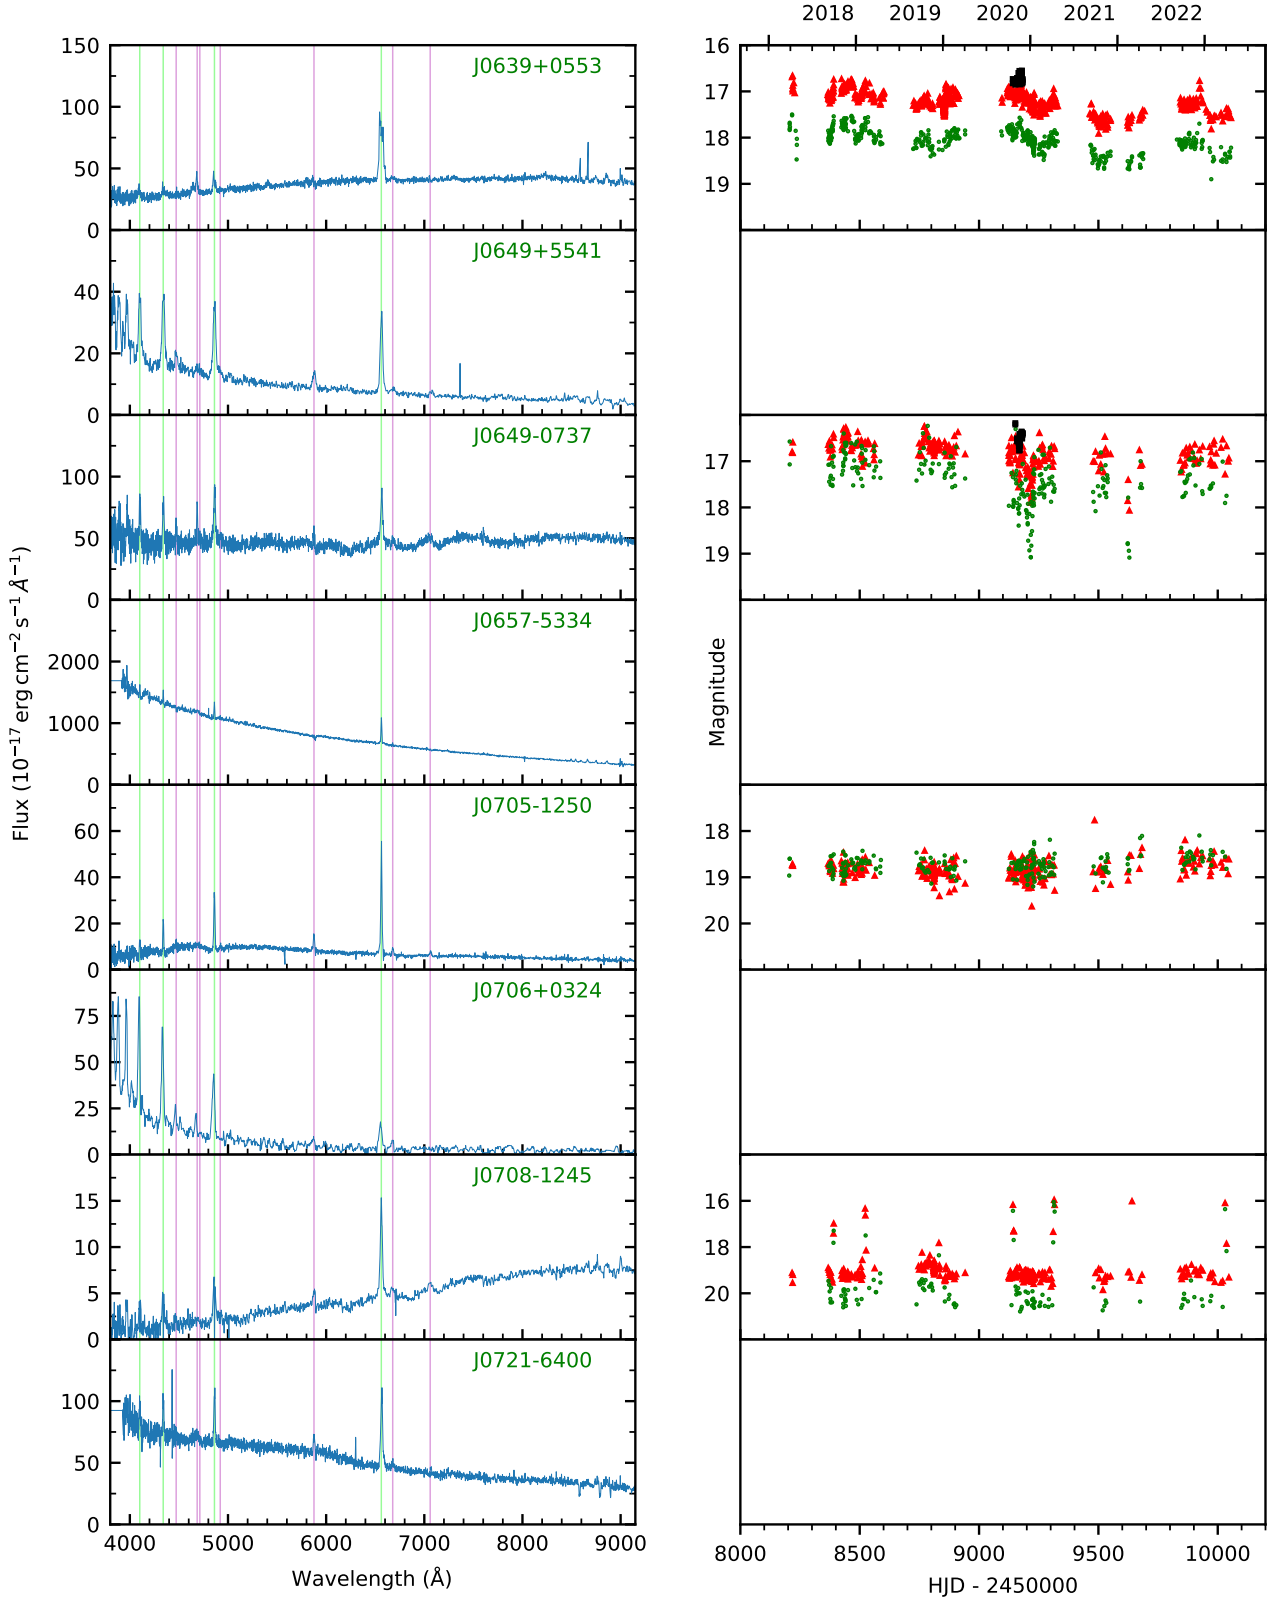

Figure 10: Left panels: Spectra with H lines shown in green and He in pink. Right panels: Light curves with ZTF  $r$ -band shown in red triangles,  $g$ -band in green dots and  $i$ -band in black squares.

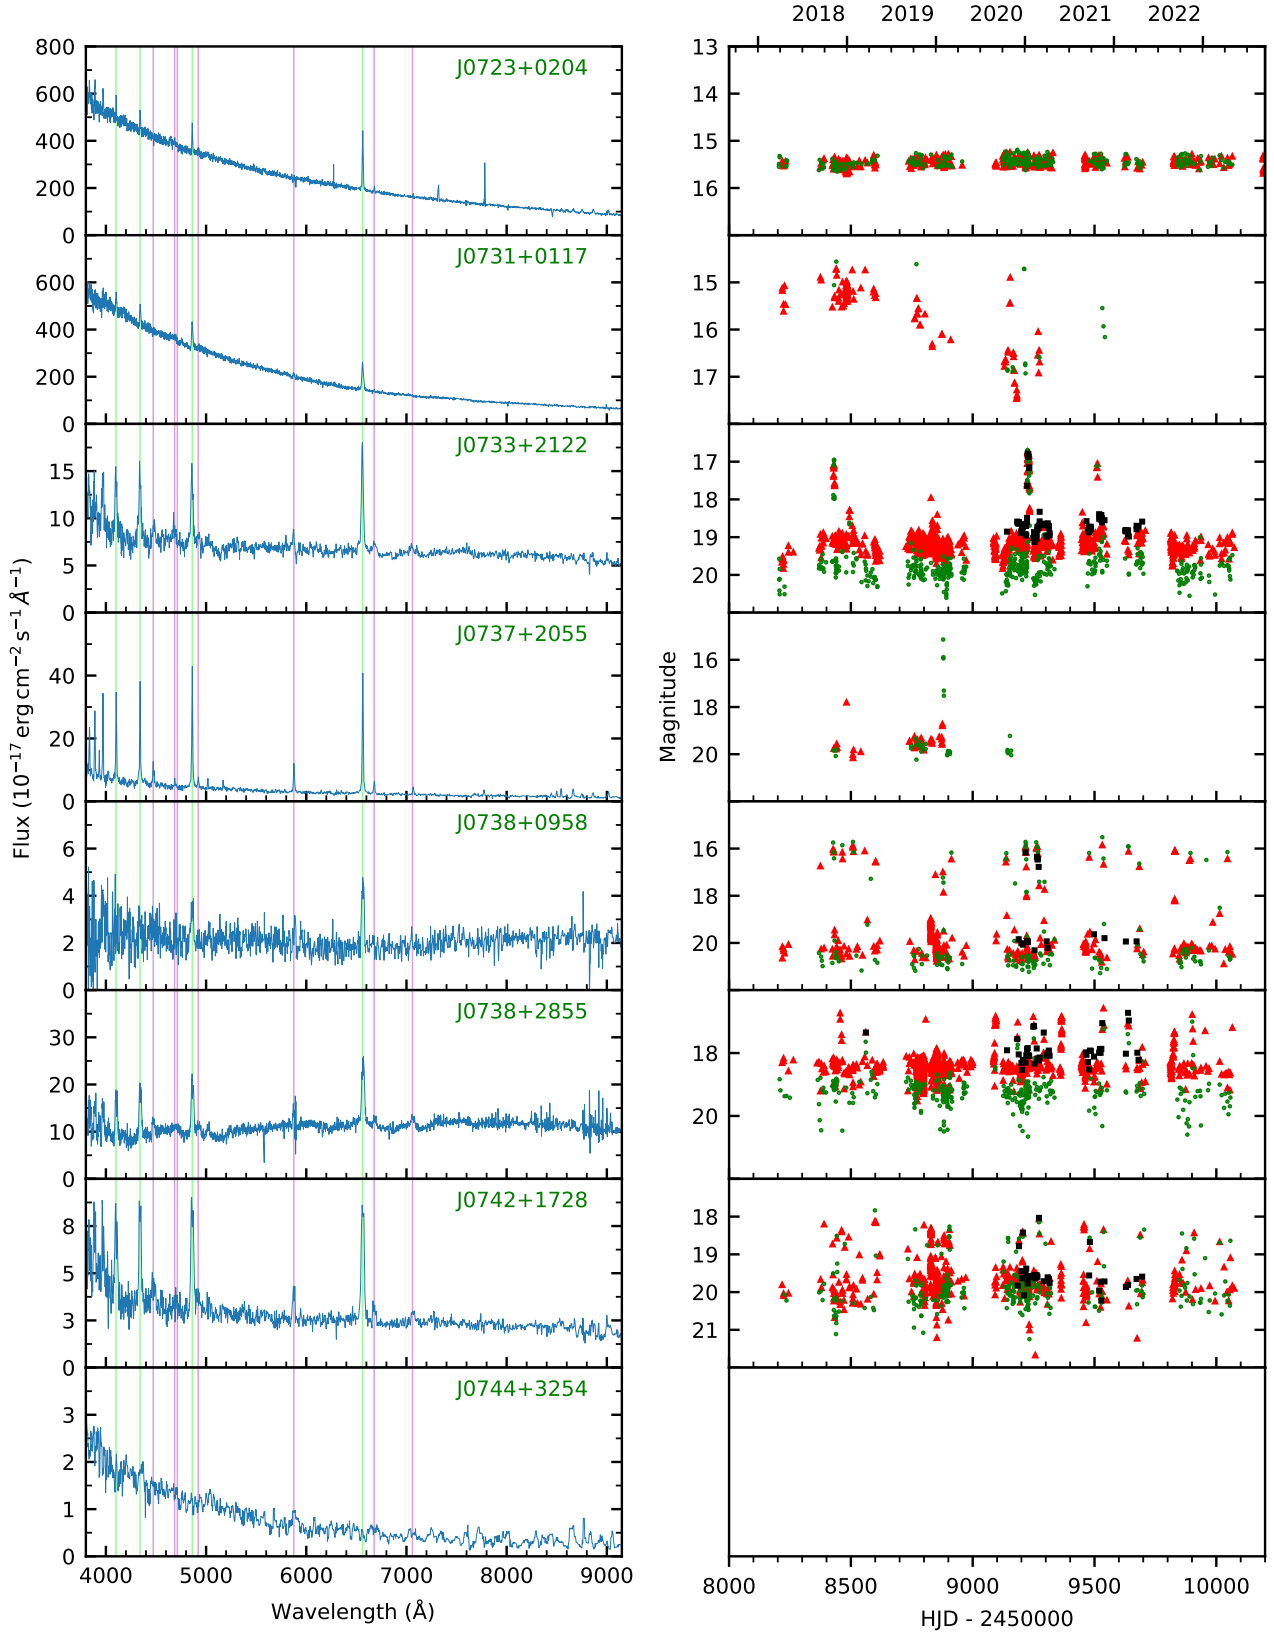

Figure 11: Left panels: Spectra with H lines shown in green and He in pink. Right panels: Light curves with ZTF  $r$ -band shown in red triangles,  $g$ -band in green dots and  $i$ -band in black squares.

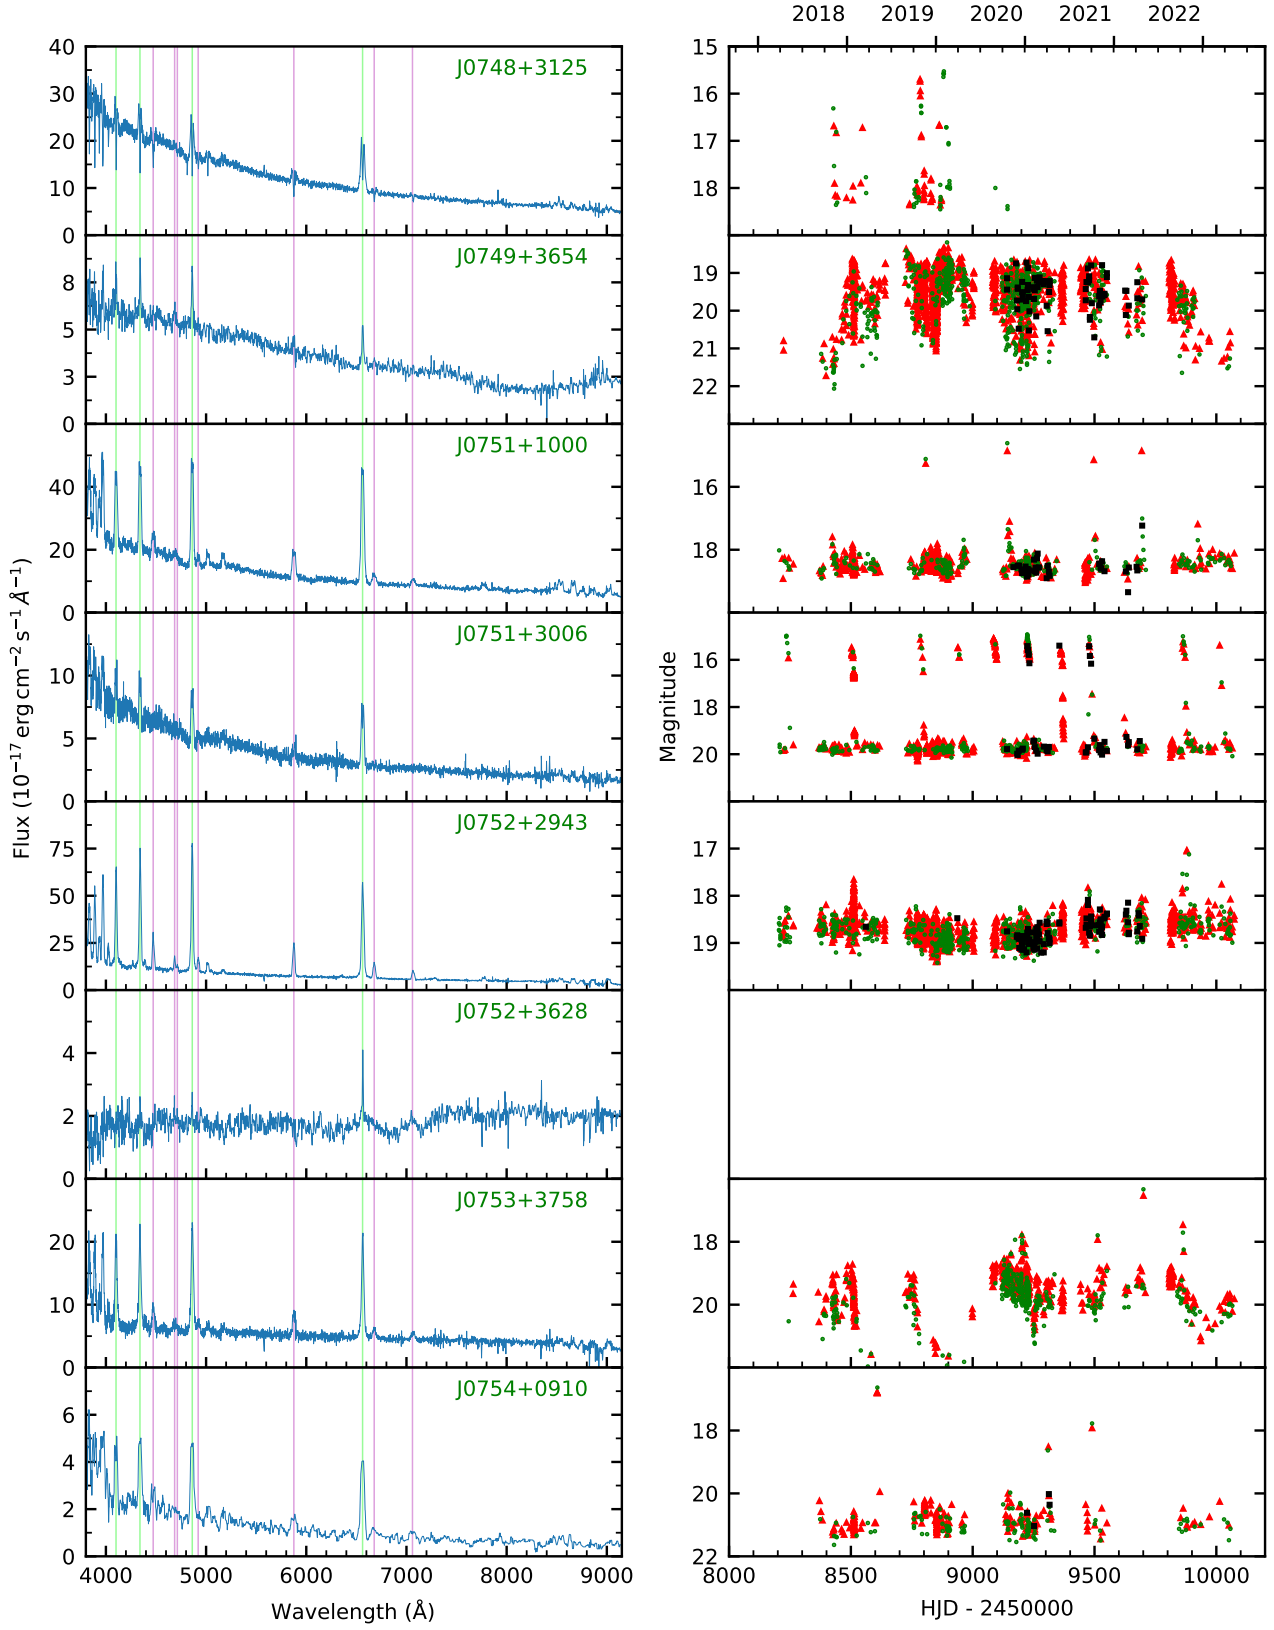

Figure 12: Left panels: Spectra with H lines shown in green and He in pink. Right panels: Light curves with ZTF  $r$ -band shown in red triangles,  $g$ -band in green dots and  $i$ -band in black squares.

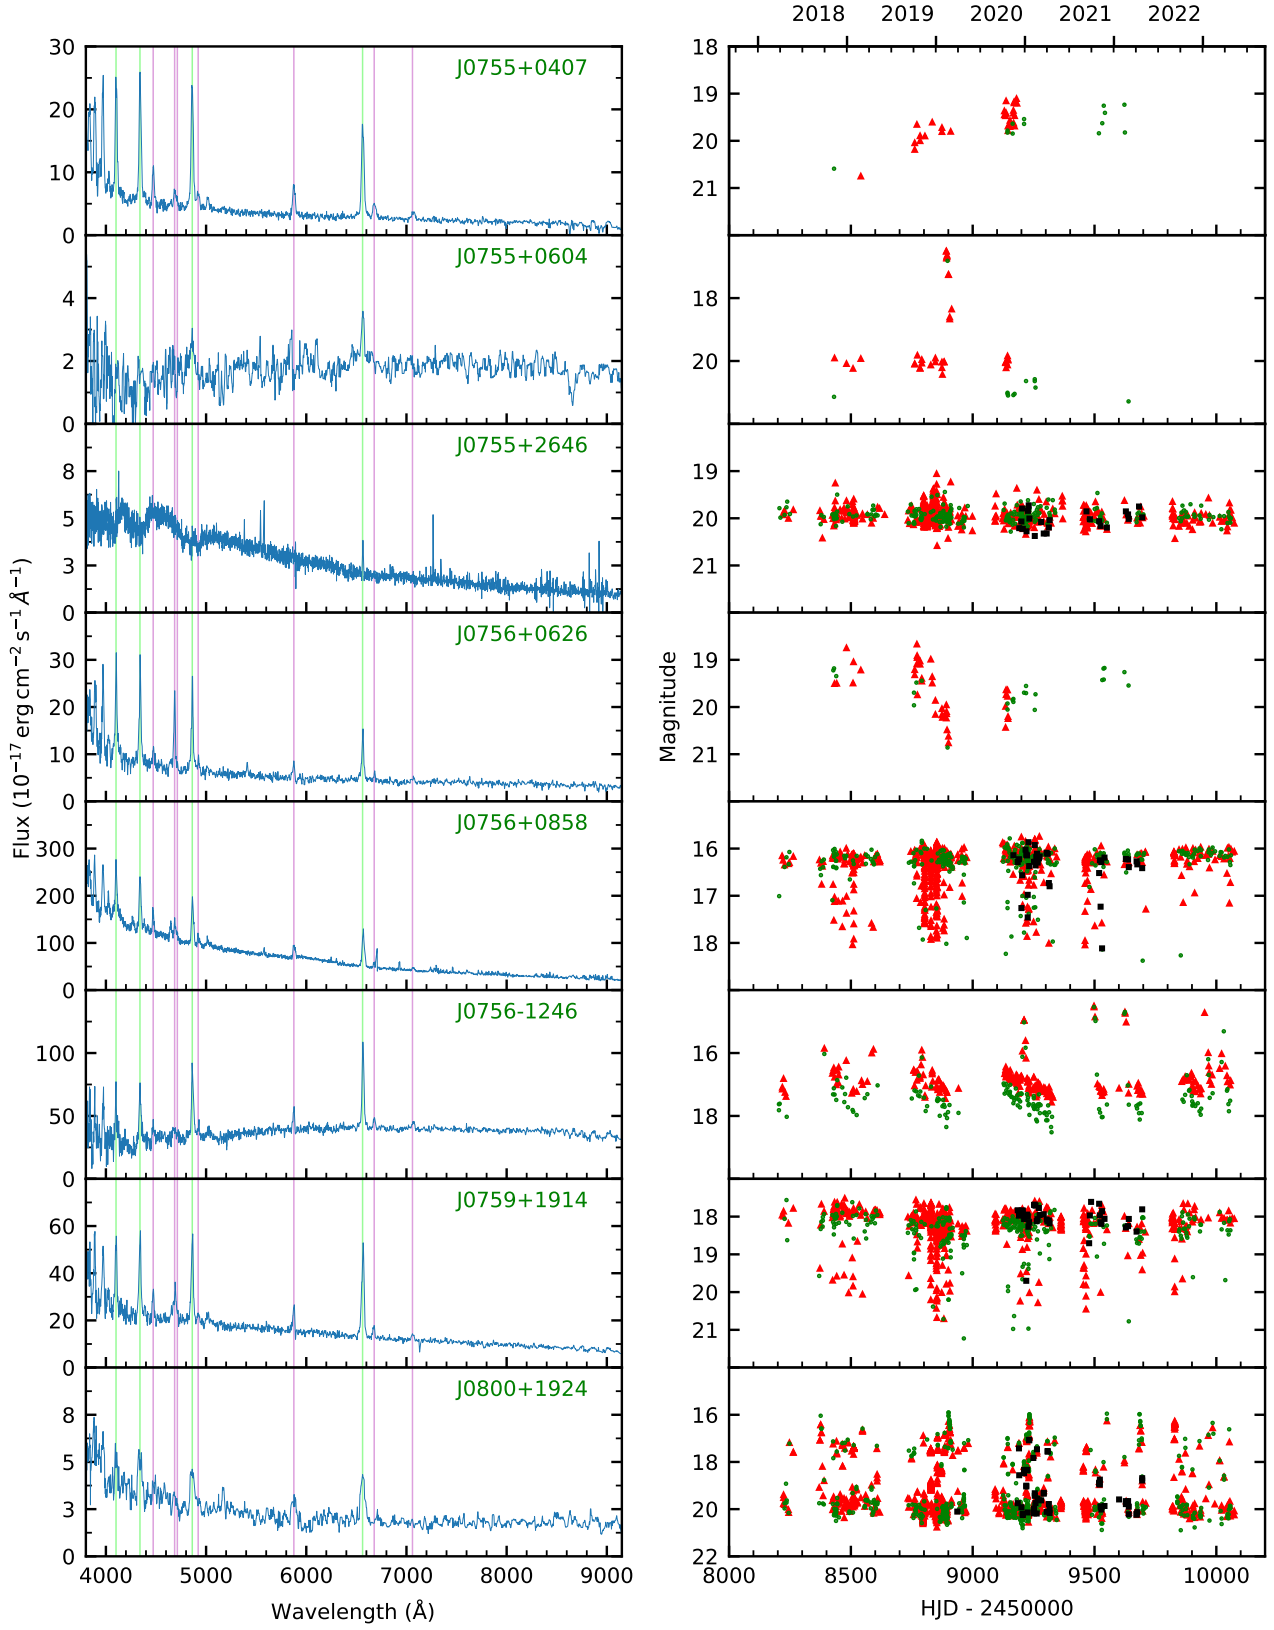

Figure 13: Left panels: Spectra with H lines shown in green and He in pink. Right panels: Light curves with ZTF  $r$ -band shown in red triangles,  $g$ -band in green dots and  $i$ -band in black squares.

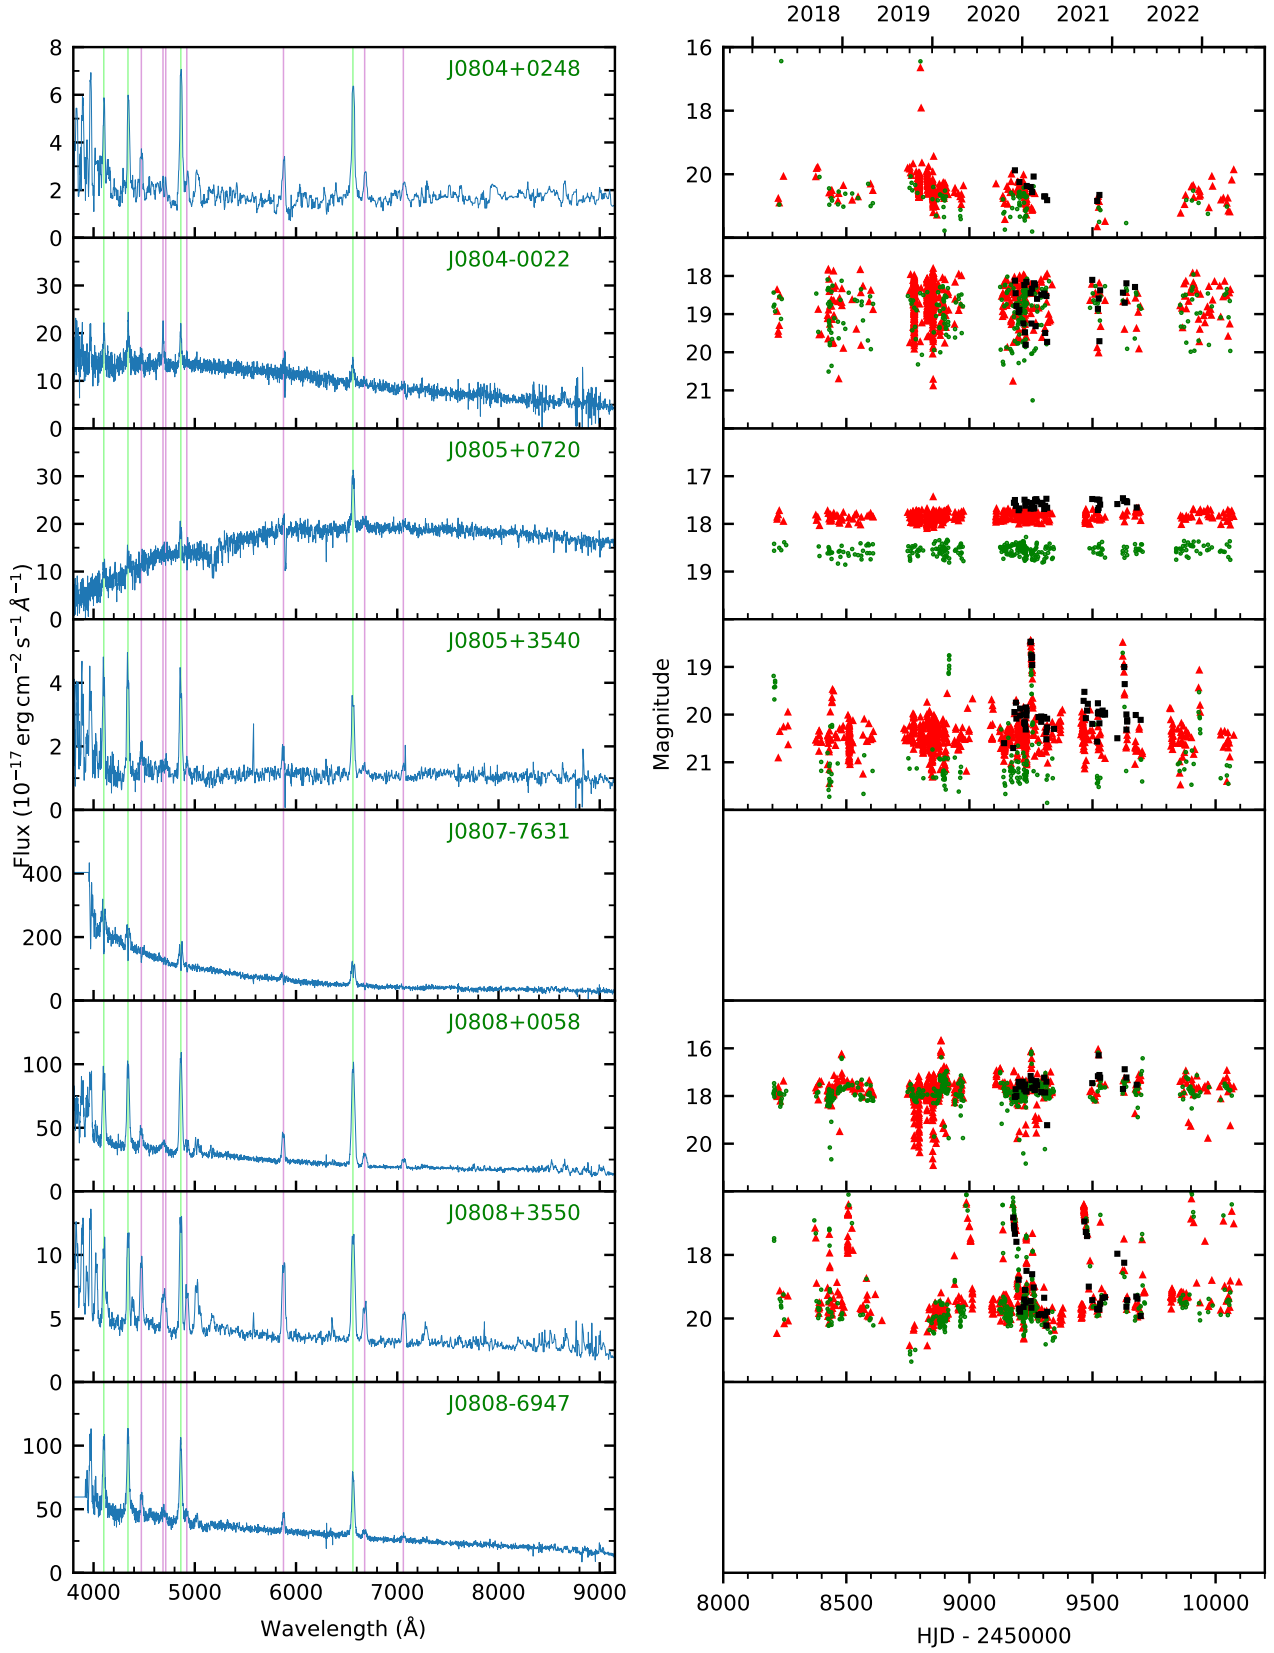

Figure 14: Left panels: Spectra with H lines shown in green and He in pink. Right panels: Light curves with ZTF *r*-band shown in red triangles, *g*-band in green dots and *i*-band in black squares.



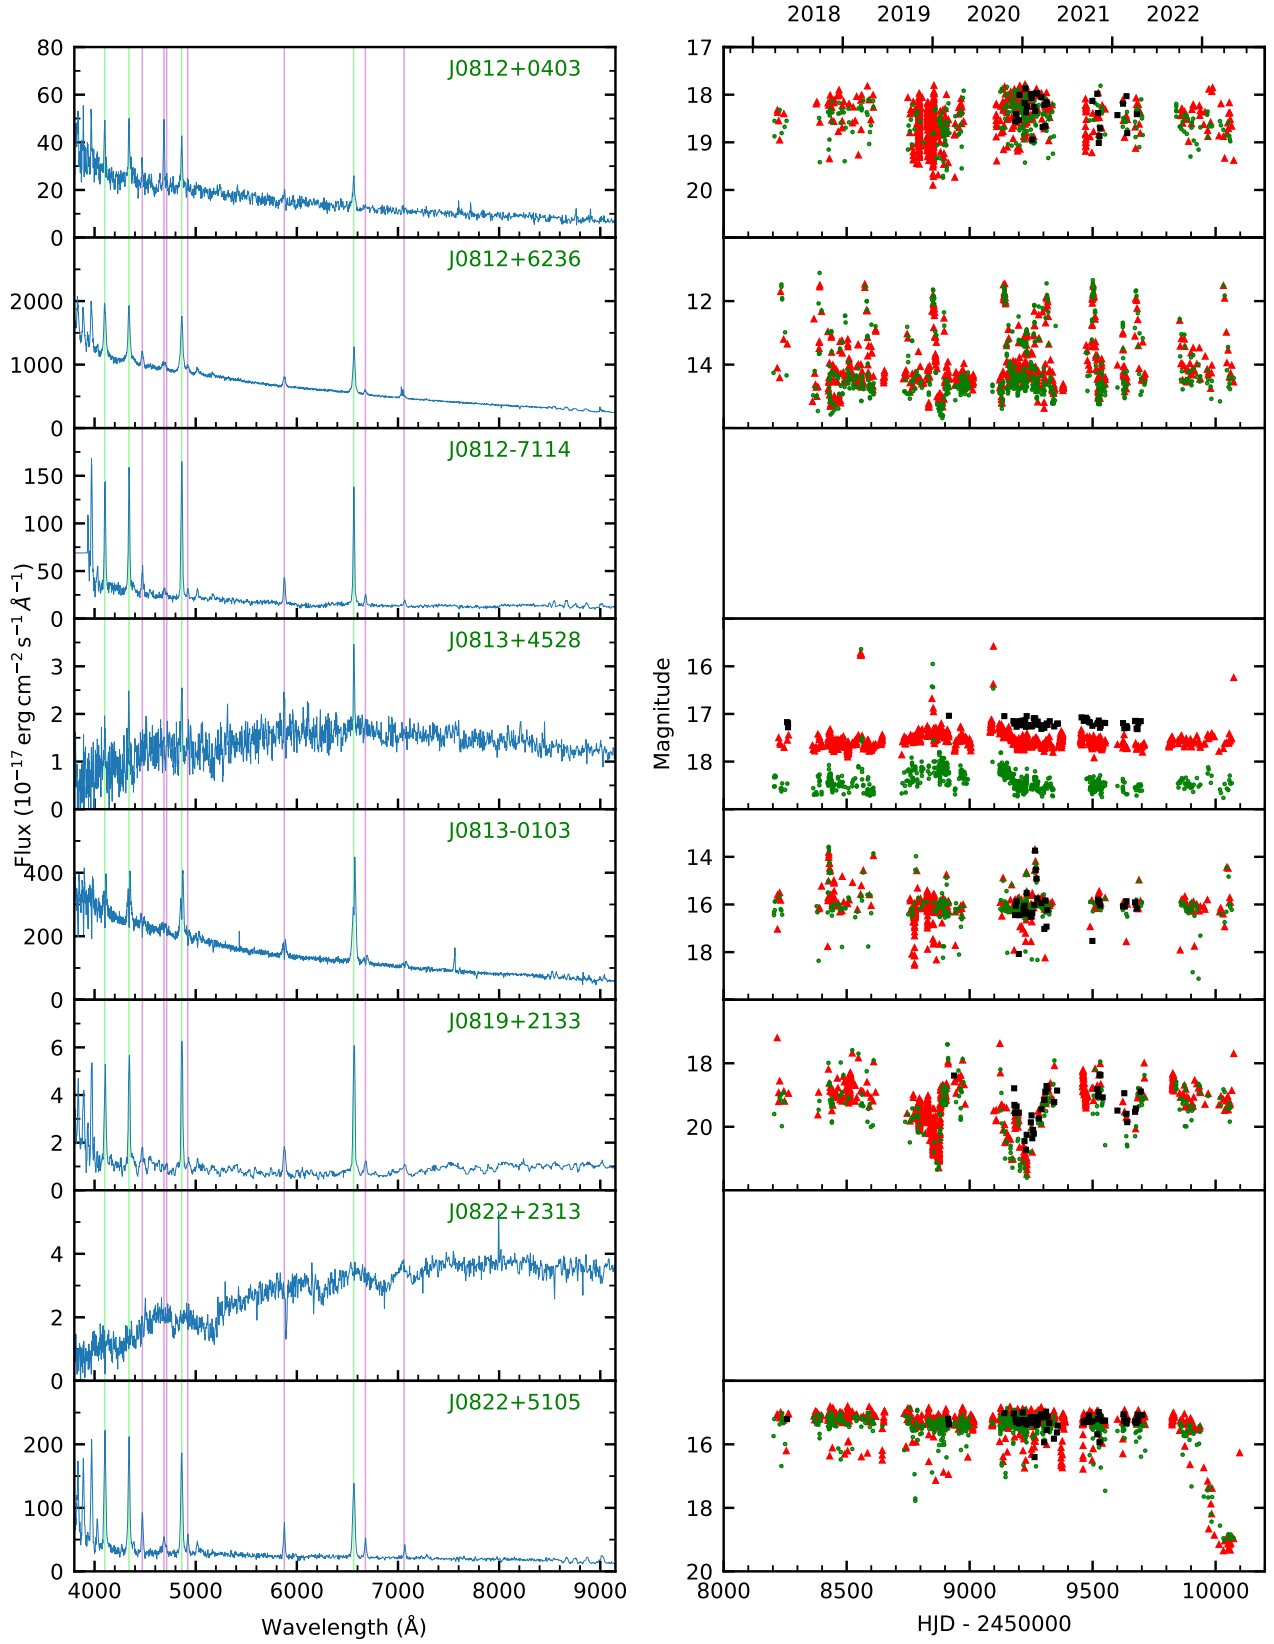

Figure 15: Left panels: Spectra with H lines shown in green and He in pink. Right panels: Light curves with ZTF *r*-band shown in red triangles, *g*-band in green dots and *i*-band in black squares.

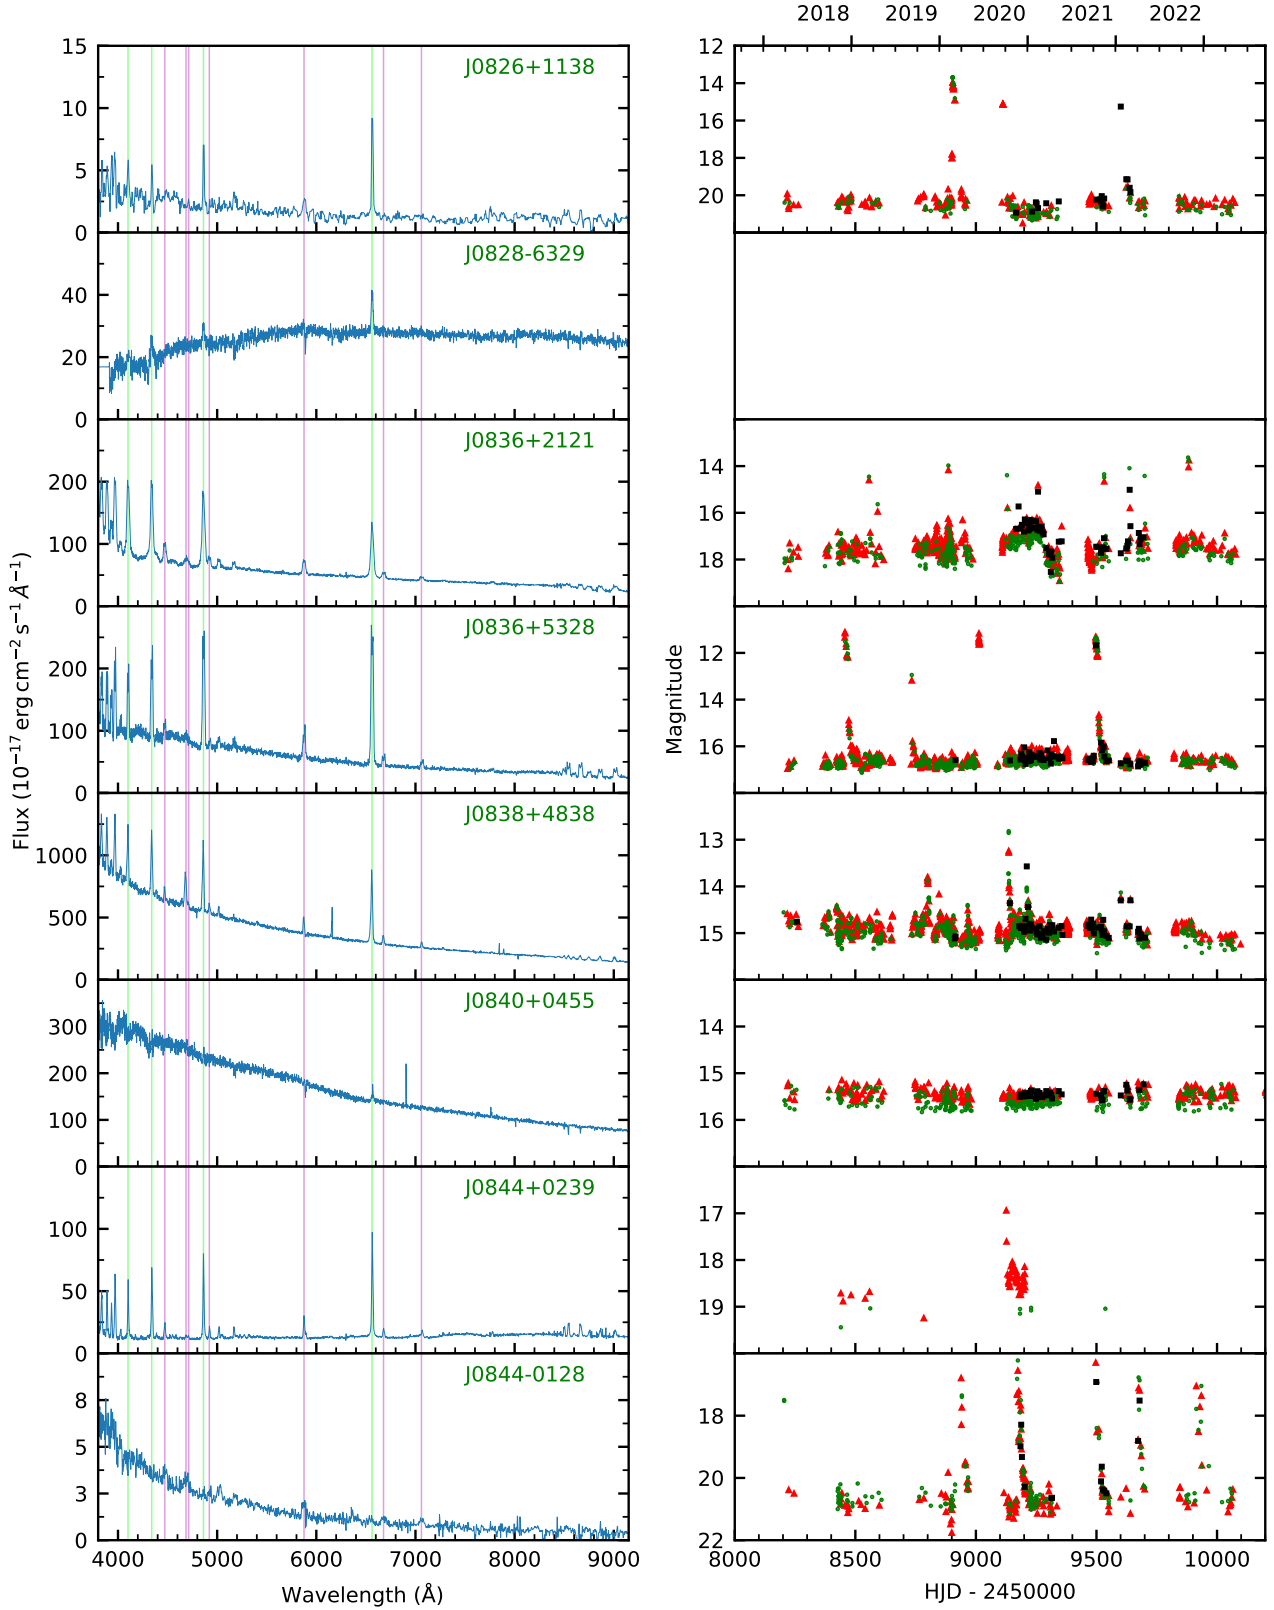

Figure 16: Left panels: Spectra with H lines shown in green and He in pink. Right panels: Light curves with ZTF  $r$ -band shown in red triangles,  $g$ -band in green dots and  $i$ -band in black squares.

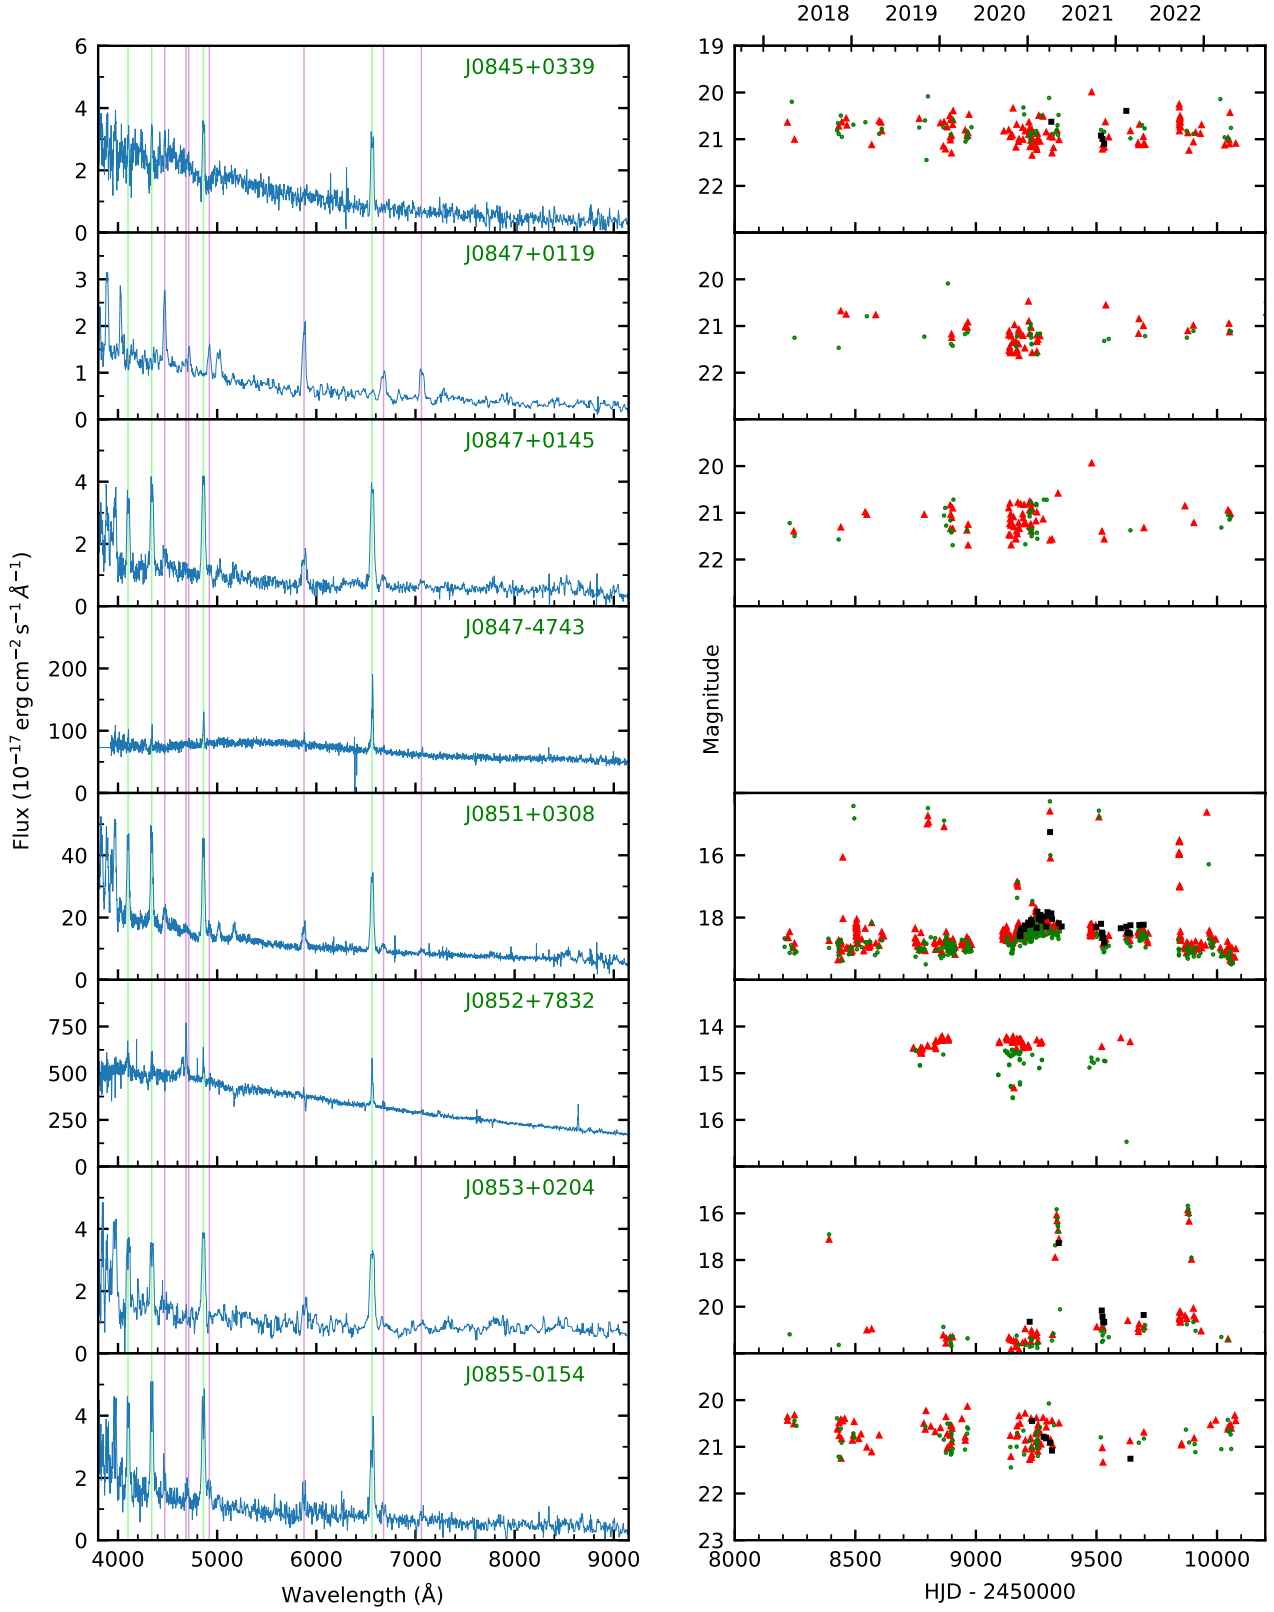

Figure 17: Left panels: Spectra with H lines shown in green and He in pink. Right panels: Light curves with ZTF *r*-band shown in red triangles, *g*-band in green dots and *i*-band in black squares.

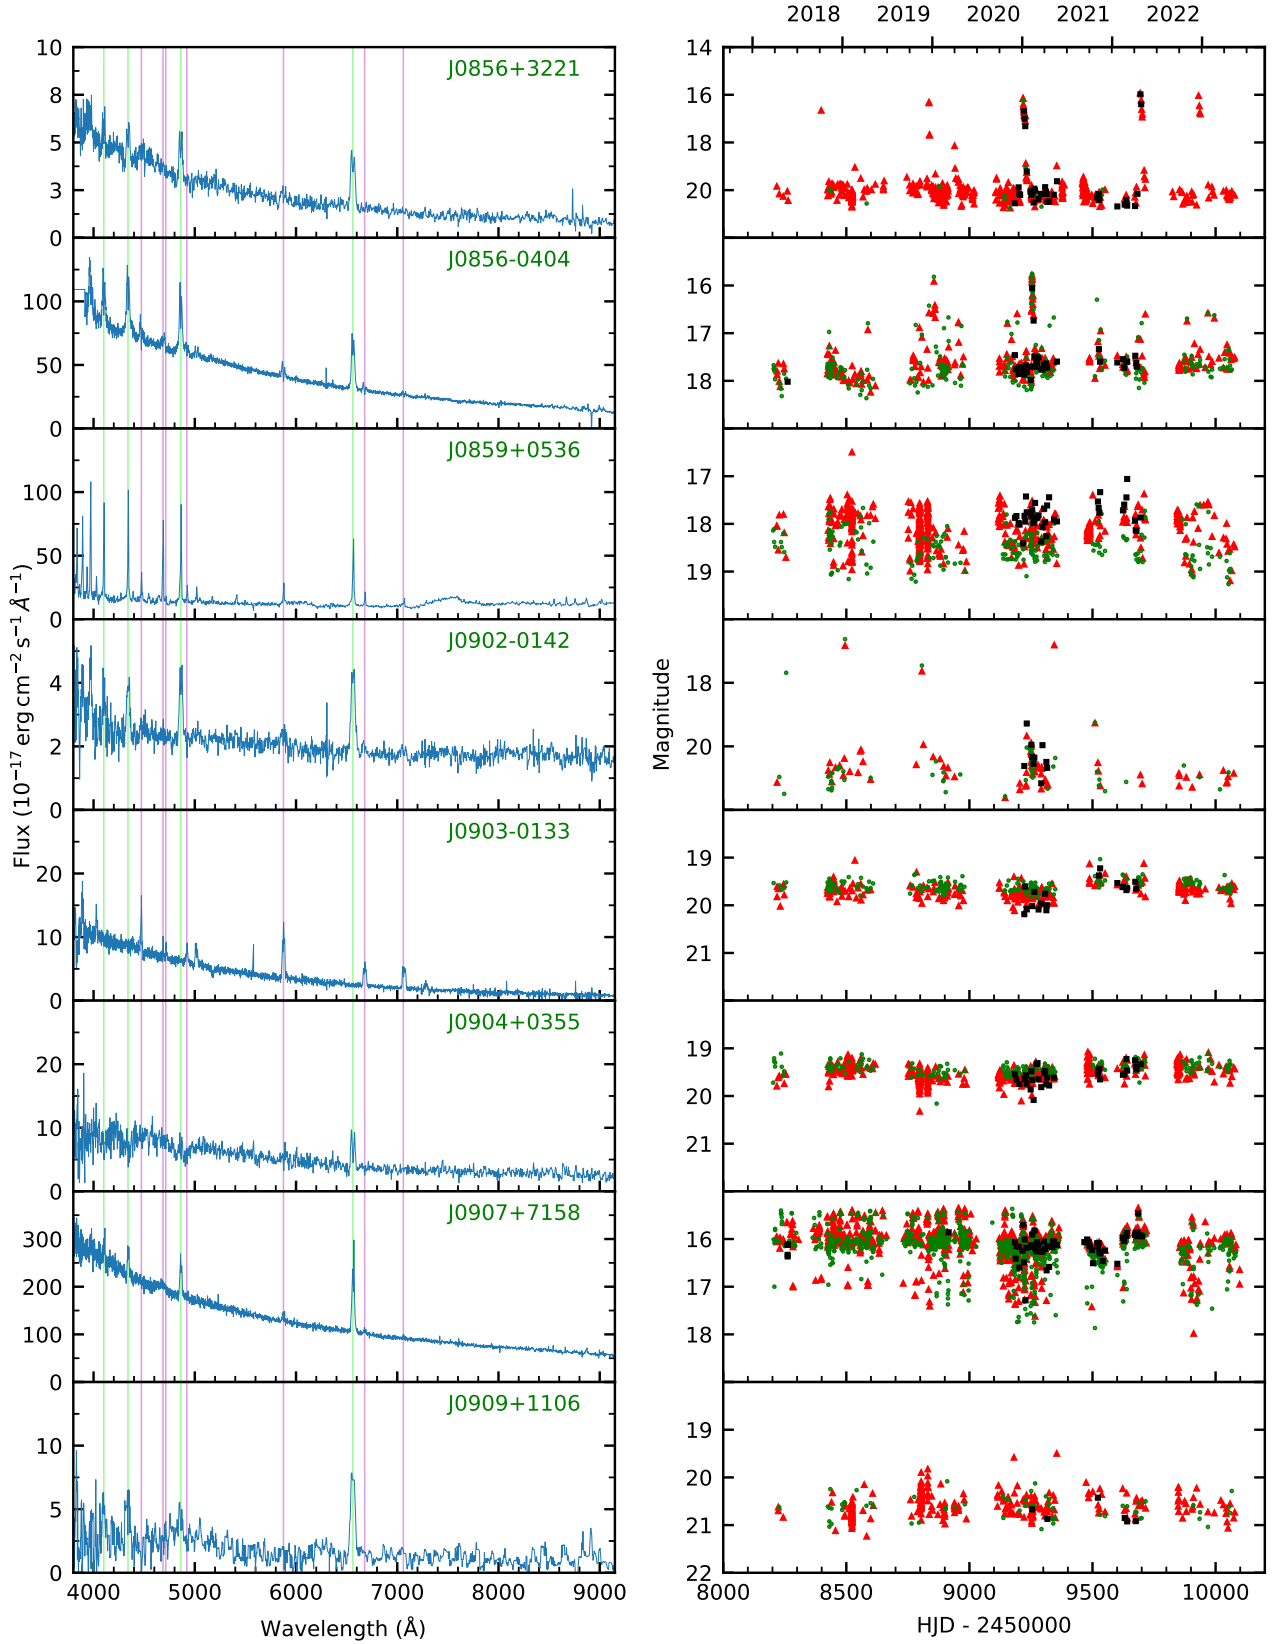

Figure 18: Left panels: Spectra with H lines shown in green and He in pink. Right panels: Light curves with ZTF  $r$ -band shown in red triangles,  $g$ -band in green dots and  $i$ -band in black squares.

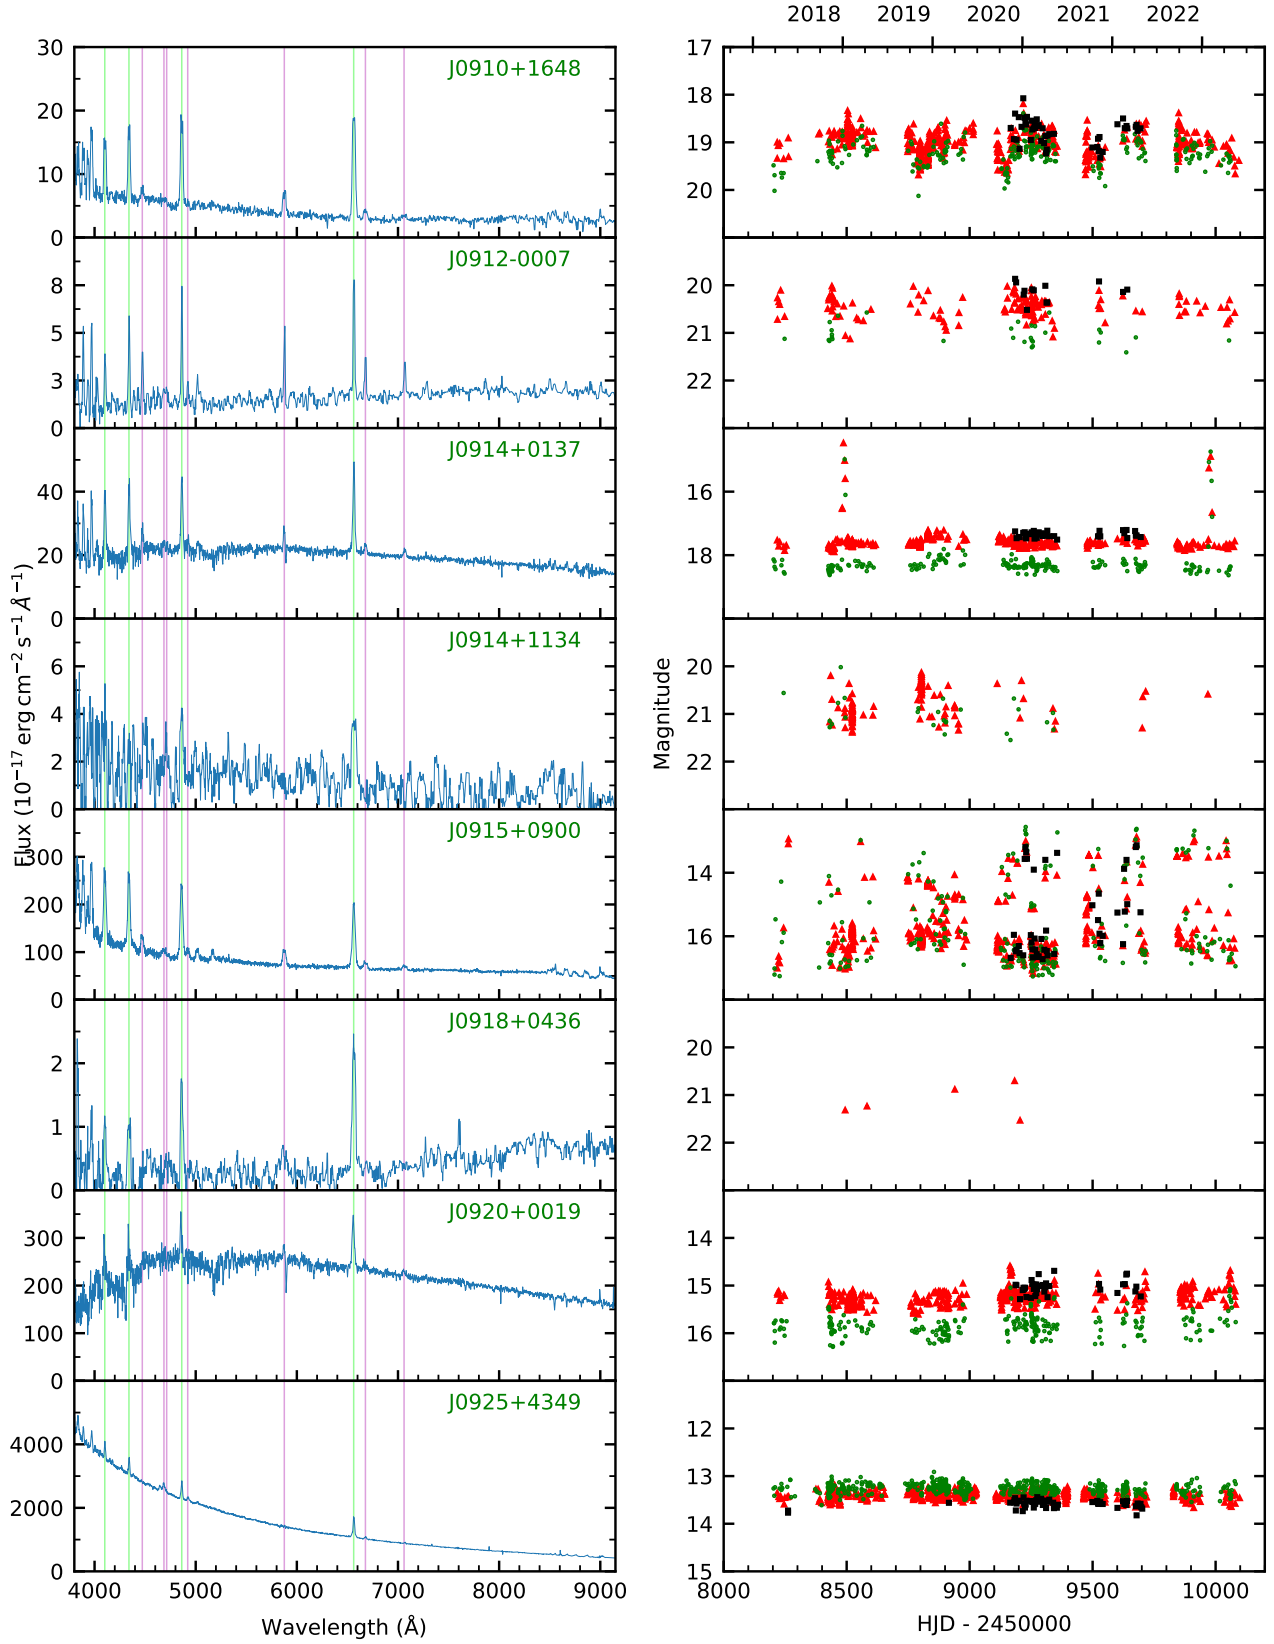

Figure 19: Left panels: Spectra with H lines shown in green and He in pink. Right panels: Light curves with ZTF  $r$ -band shown in red triangles,  $g$ -band in green dots and  $i$ -band in black squares.



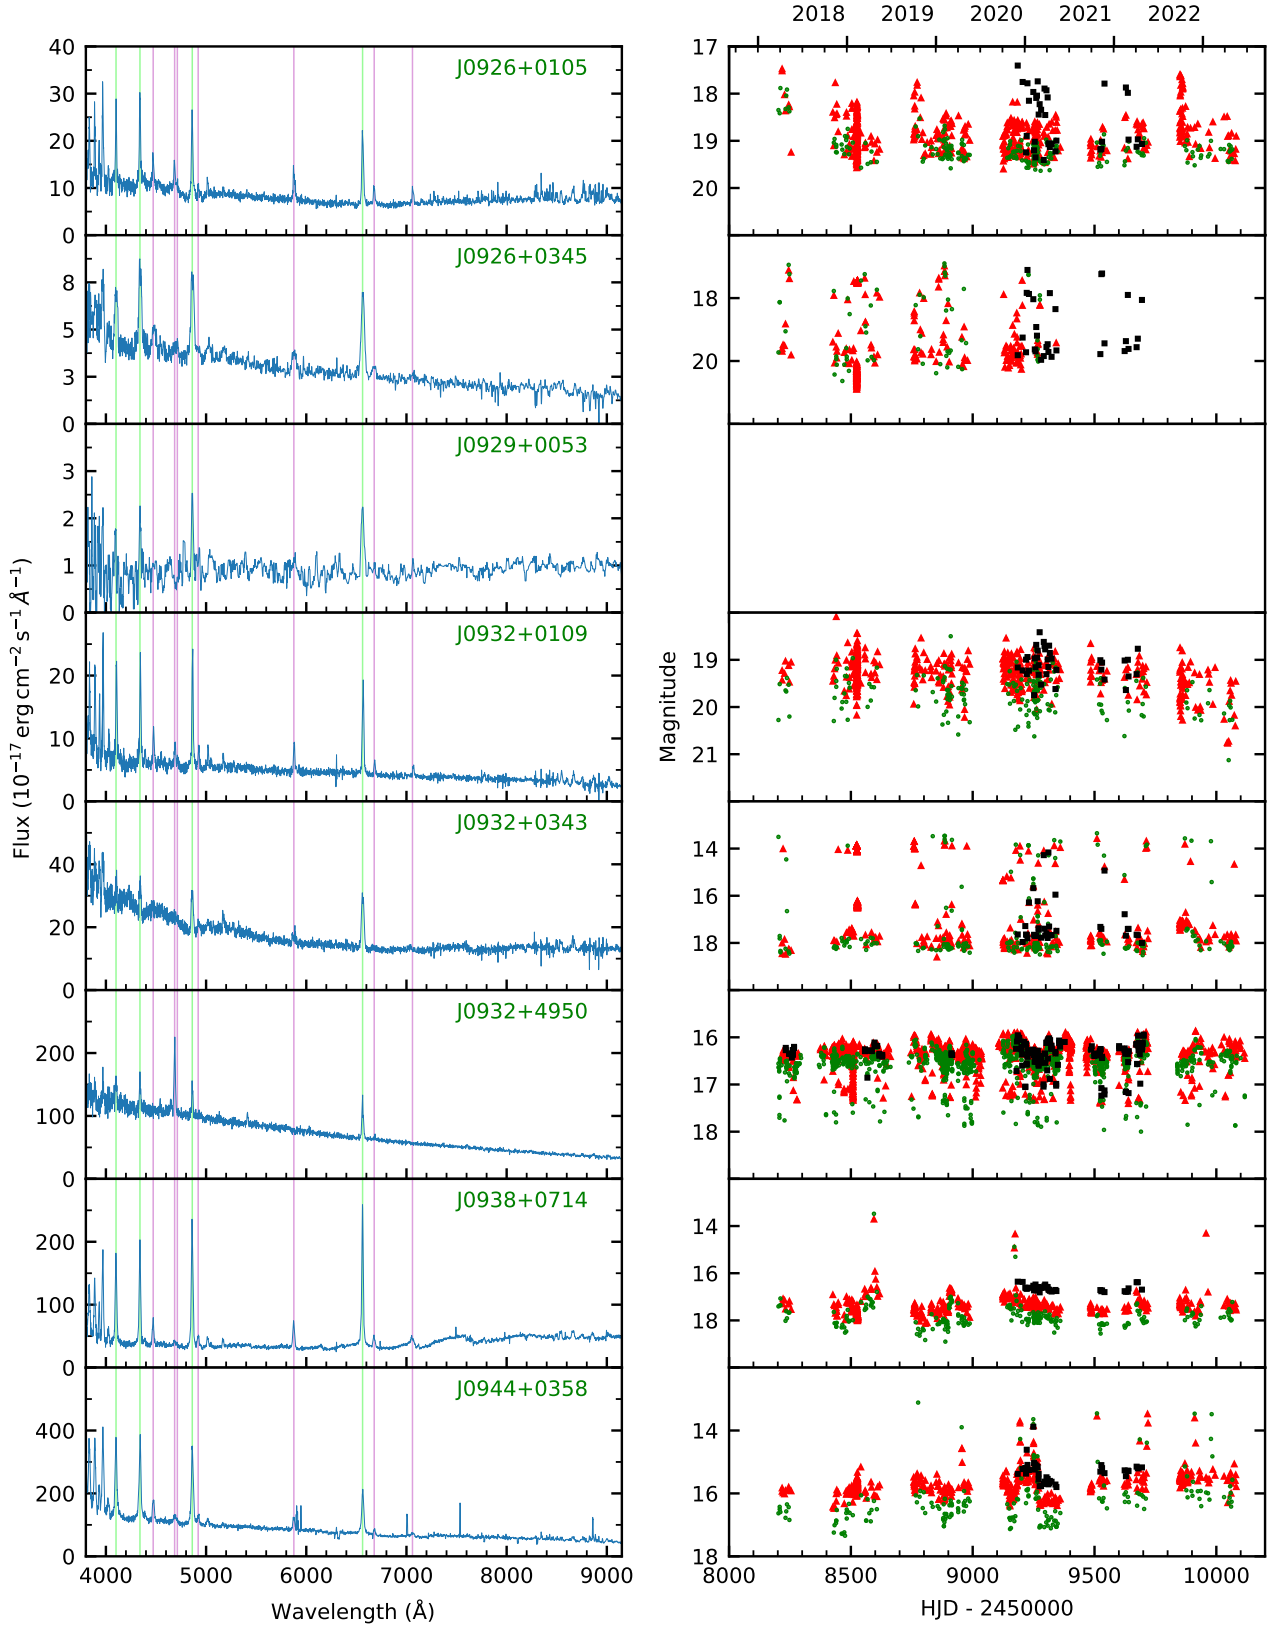

Figure 20: Left panels: Spectra with H lines shown in green and He in pink. Right panels: Light curves with ZTF  $r$ -band shown in red triangles,  $g$ -band in green dots and  $i$ -band in black squares.

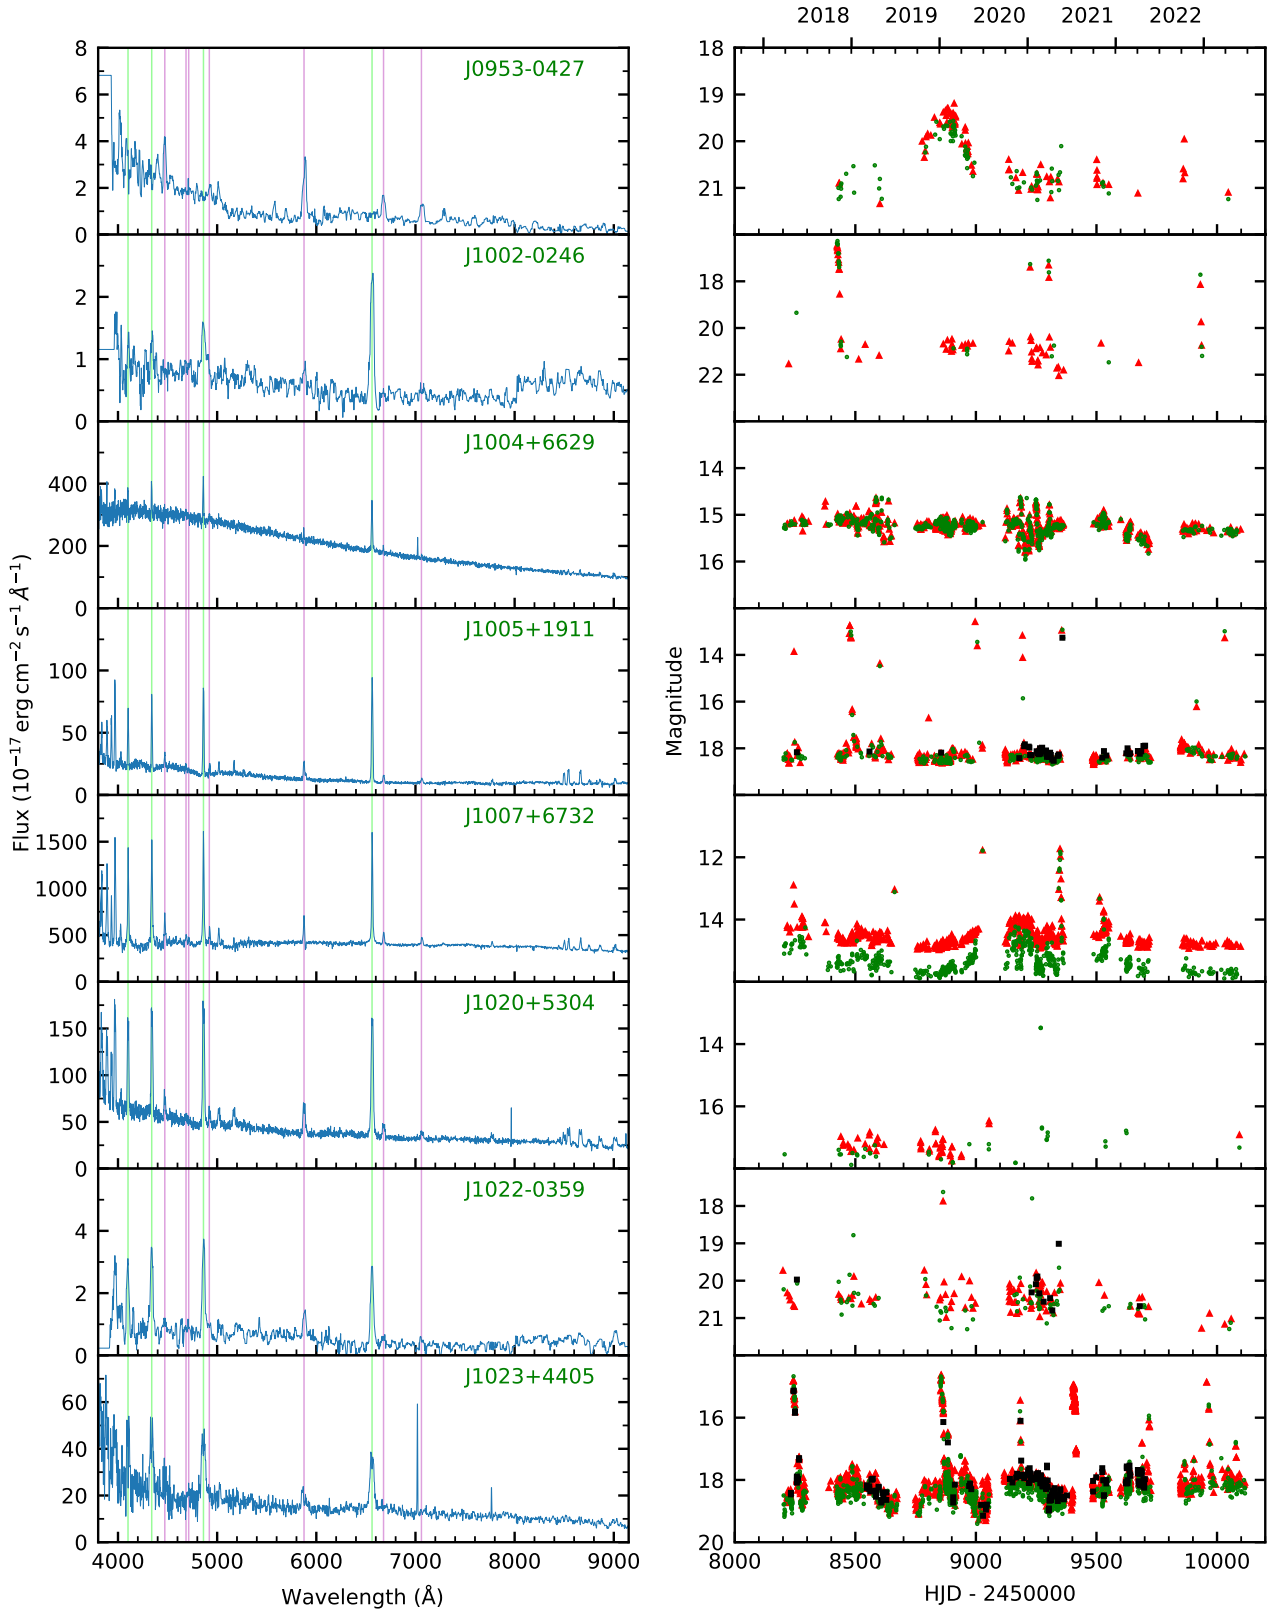

Figure 21: Left panels: Spectra with H lines shown in green and He in pink. Right panels: Light curves with ZTF *r*-band shown in red triangles, *g*-band in green dots and *i*-band in black squares.

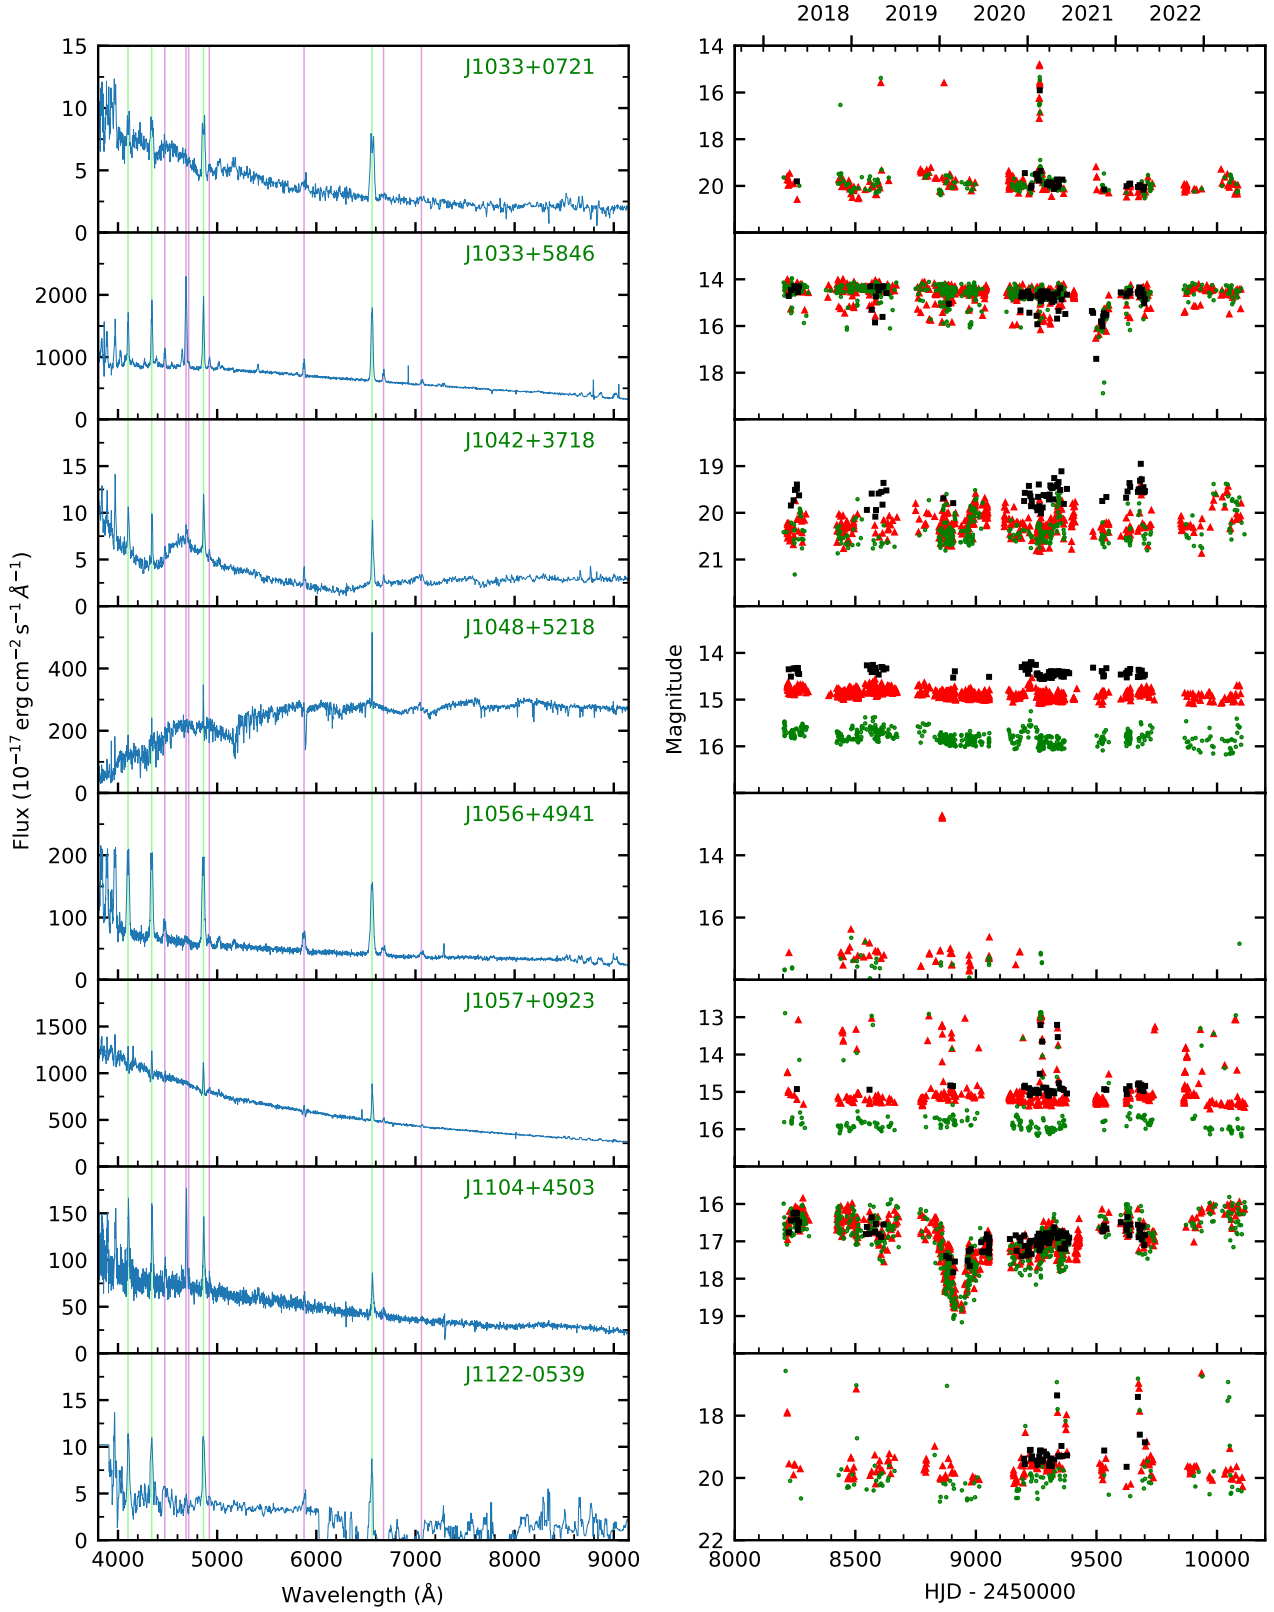

Figure 22: Left panels: Spectra with H lines shown in green and He in pink. Right panels: Light curves with ZTF  $r$ -band shown in red triangles,  $g$ -band in green dots and  $i$ -band in black squares.

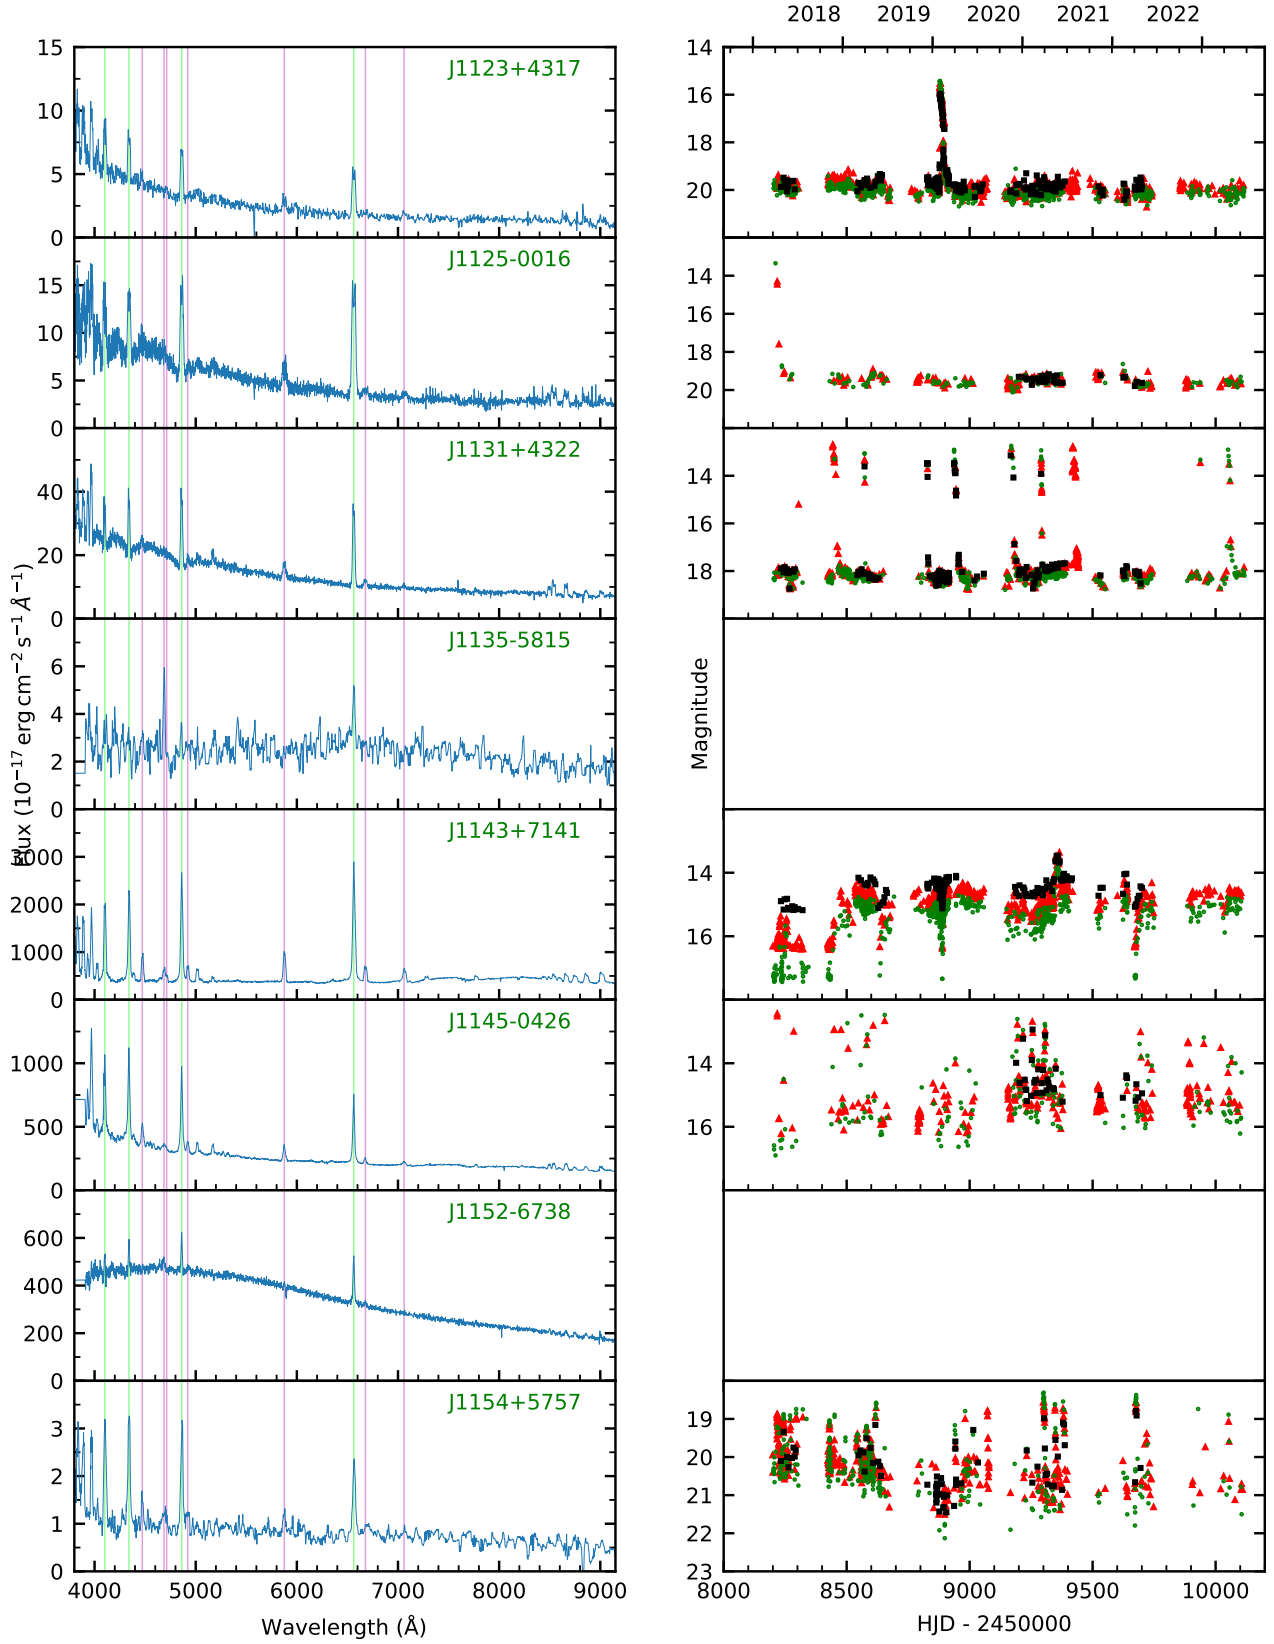

Figure 23: Left panels: Spectra with H lines shown in green and He in pink. Right panels: Light curves with ZTF *r*-band shown in red triangles, *g*-band in green dots and *i*-band in black squares.

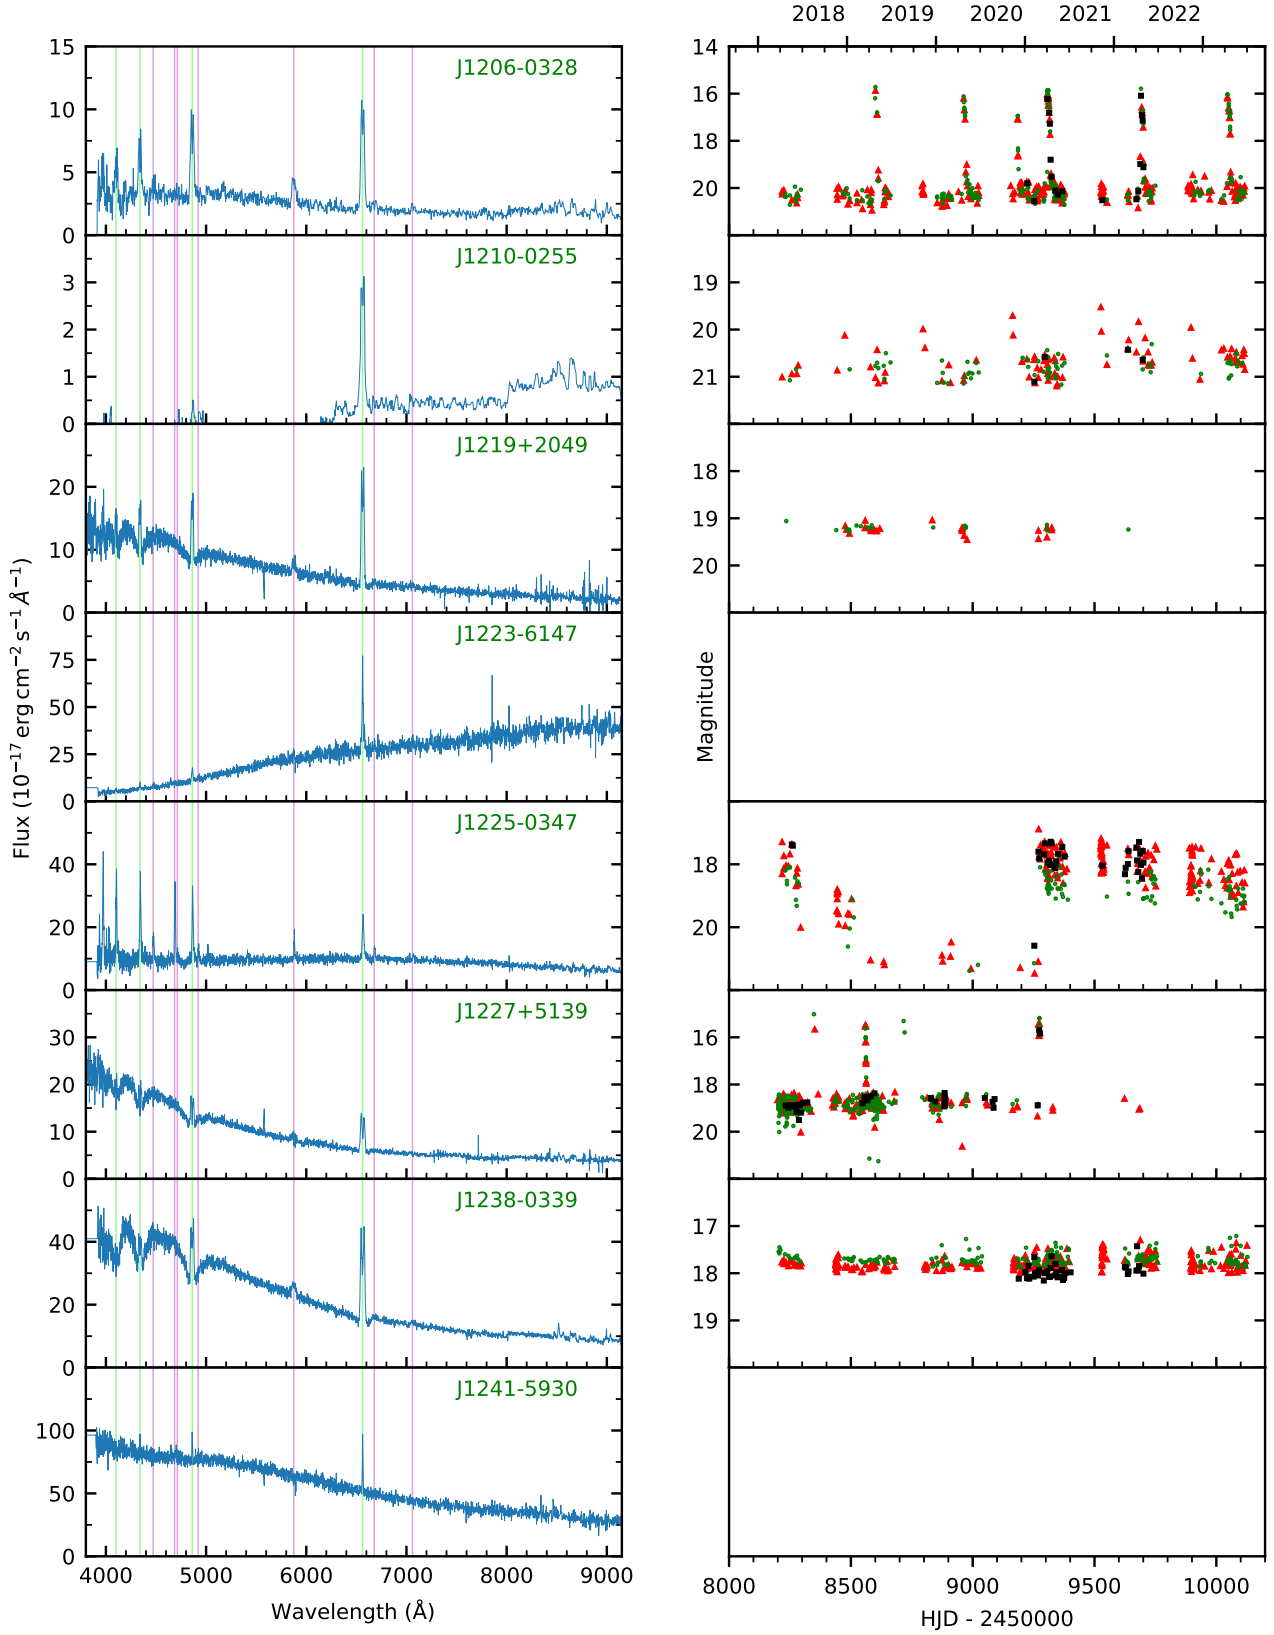

Figure 24: Left panels: Spectra with H lines shown in green and He in pink. Right panels: Light curves with ZTF  $r$ -band shown in red triangles,  $g$ -band in green dots and  $i$ -band in black squares.

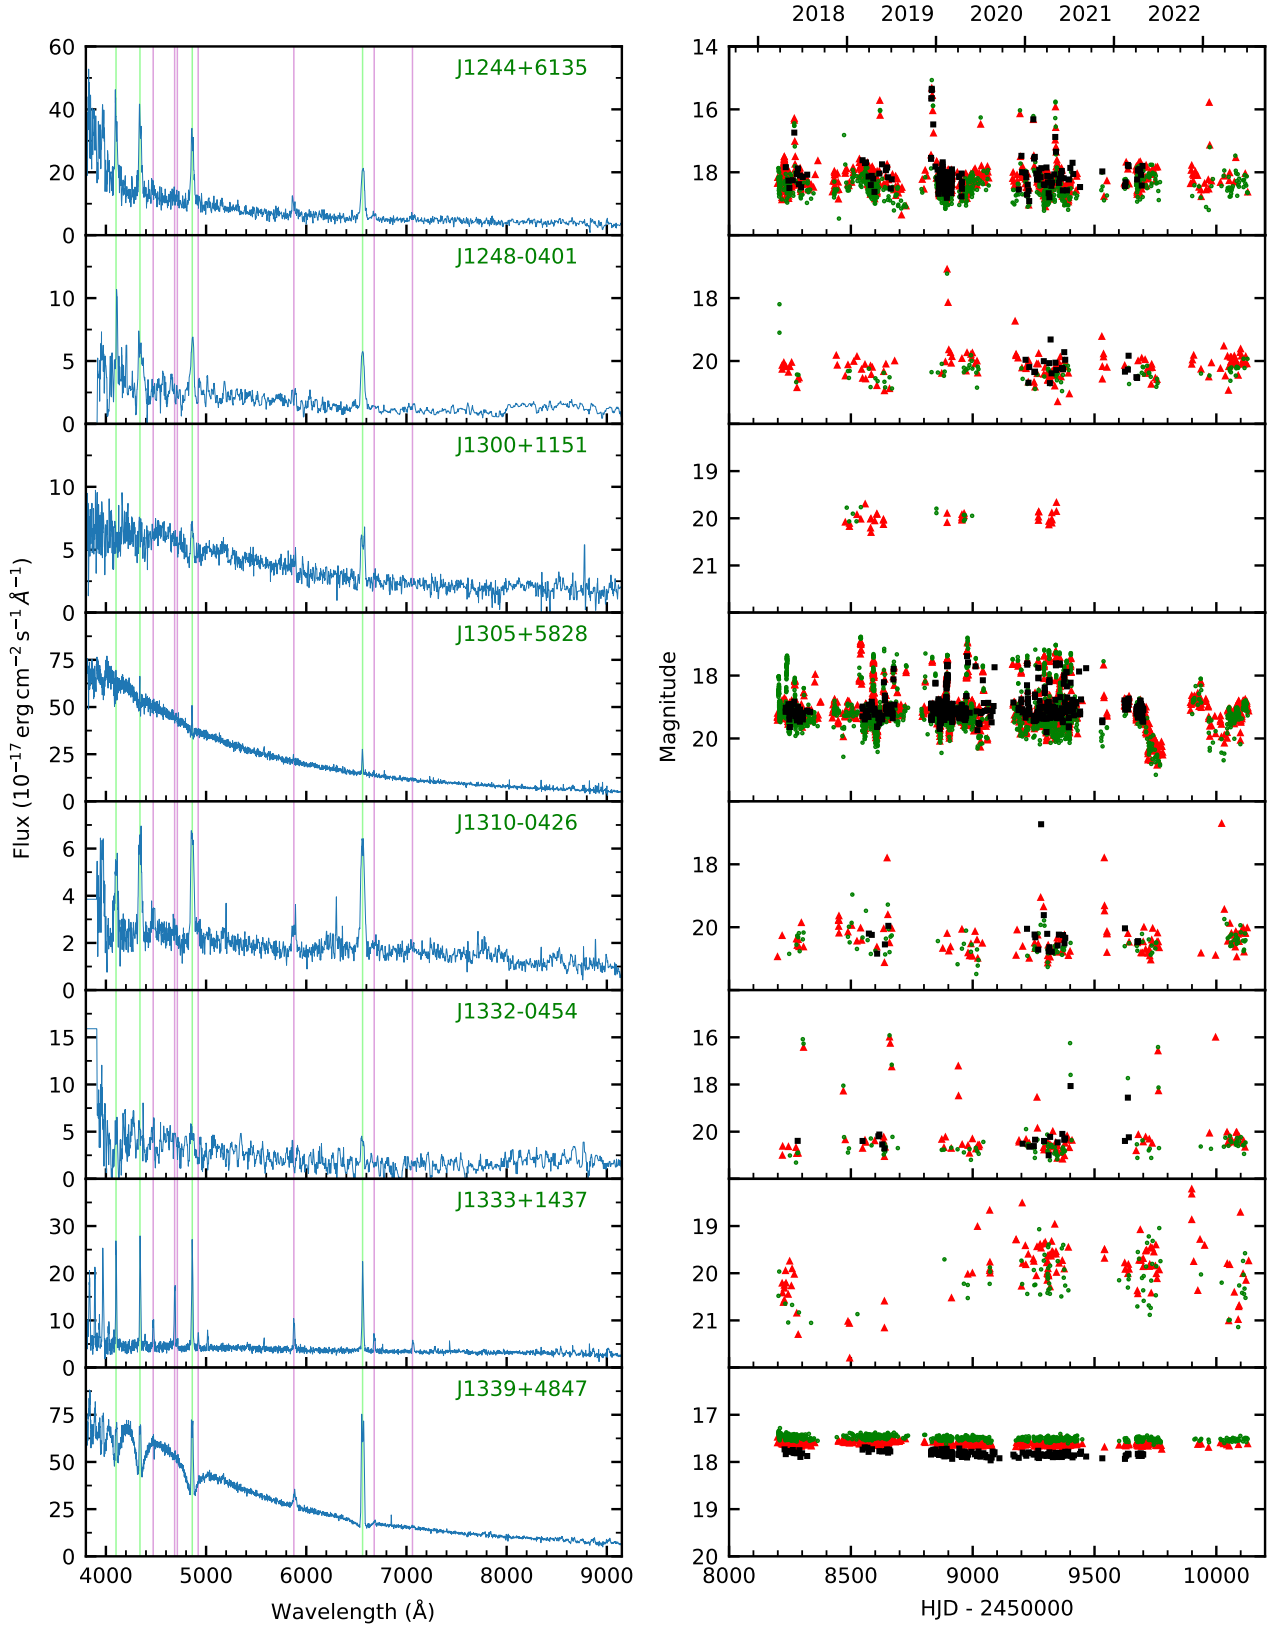

Figure 25: Left panels: Spectra with H lines shown in green and He in pink. Right panels: Light curves with ZTF  $r$ -band shown in red triangles,  $g$ -band in green dots and  $i$ -band in black squares.



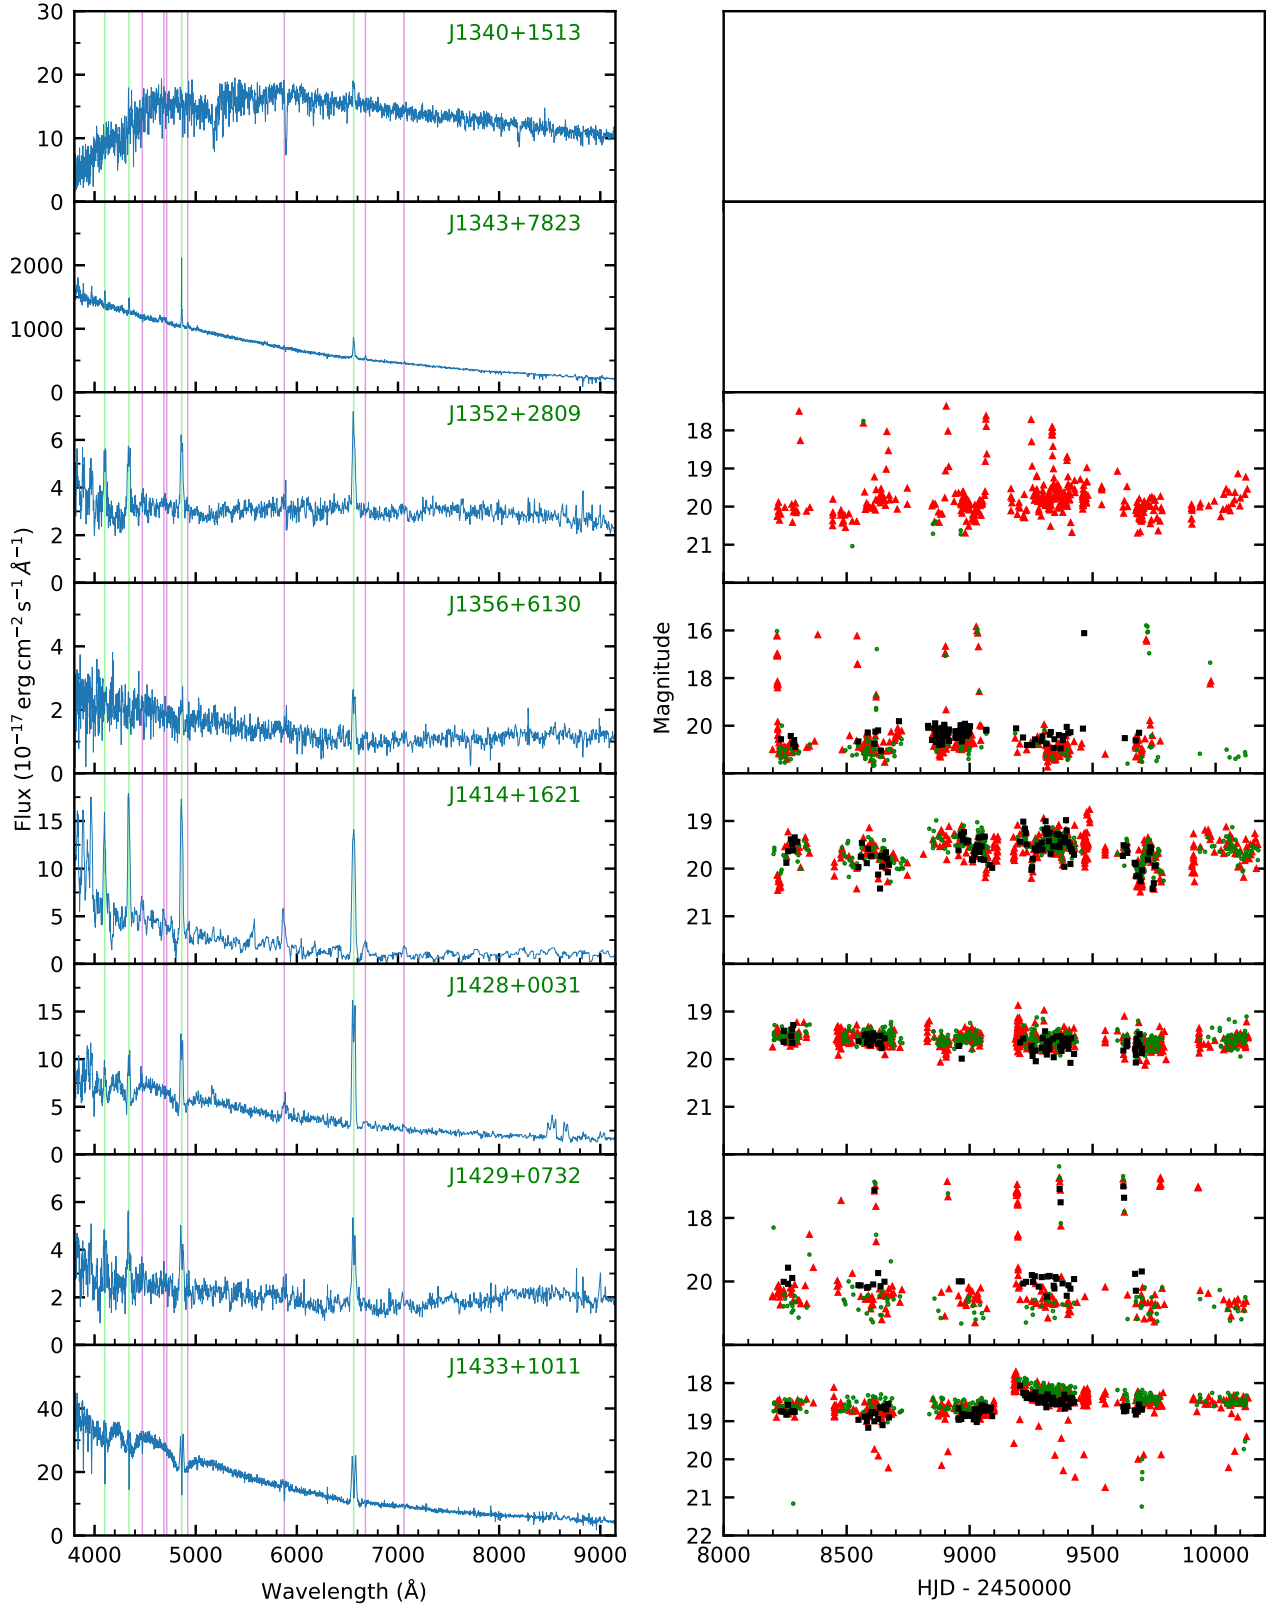

Figure 26: Left panels: Spectra with H lines shown in green and He in pink. Right panels: Light curves with ZTF  $r$ -band shown in red triangles,  $g$ -band in green dots and  $i$ -band in black squares.

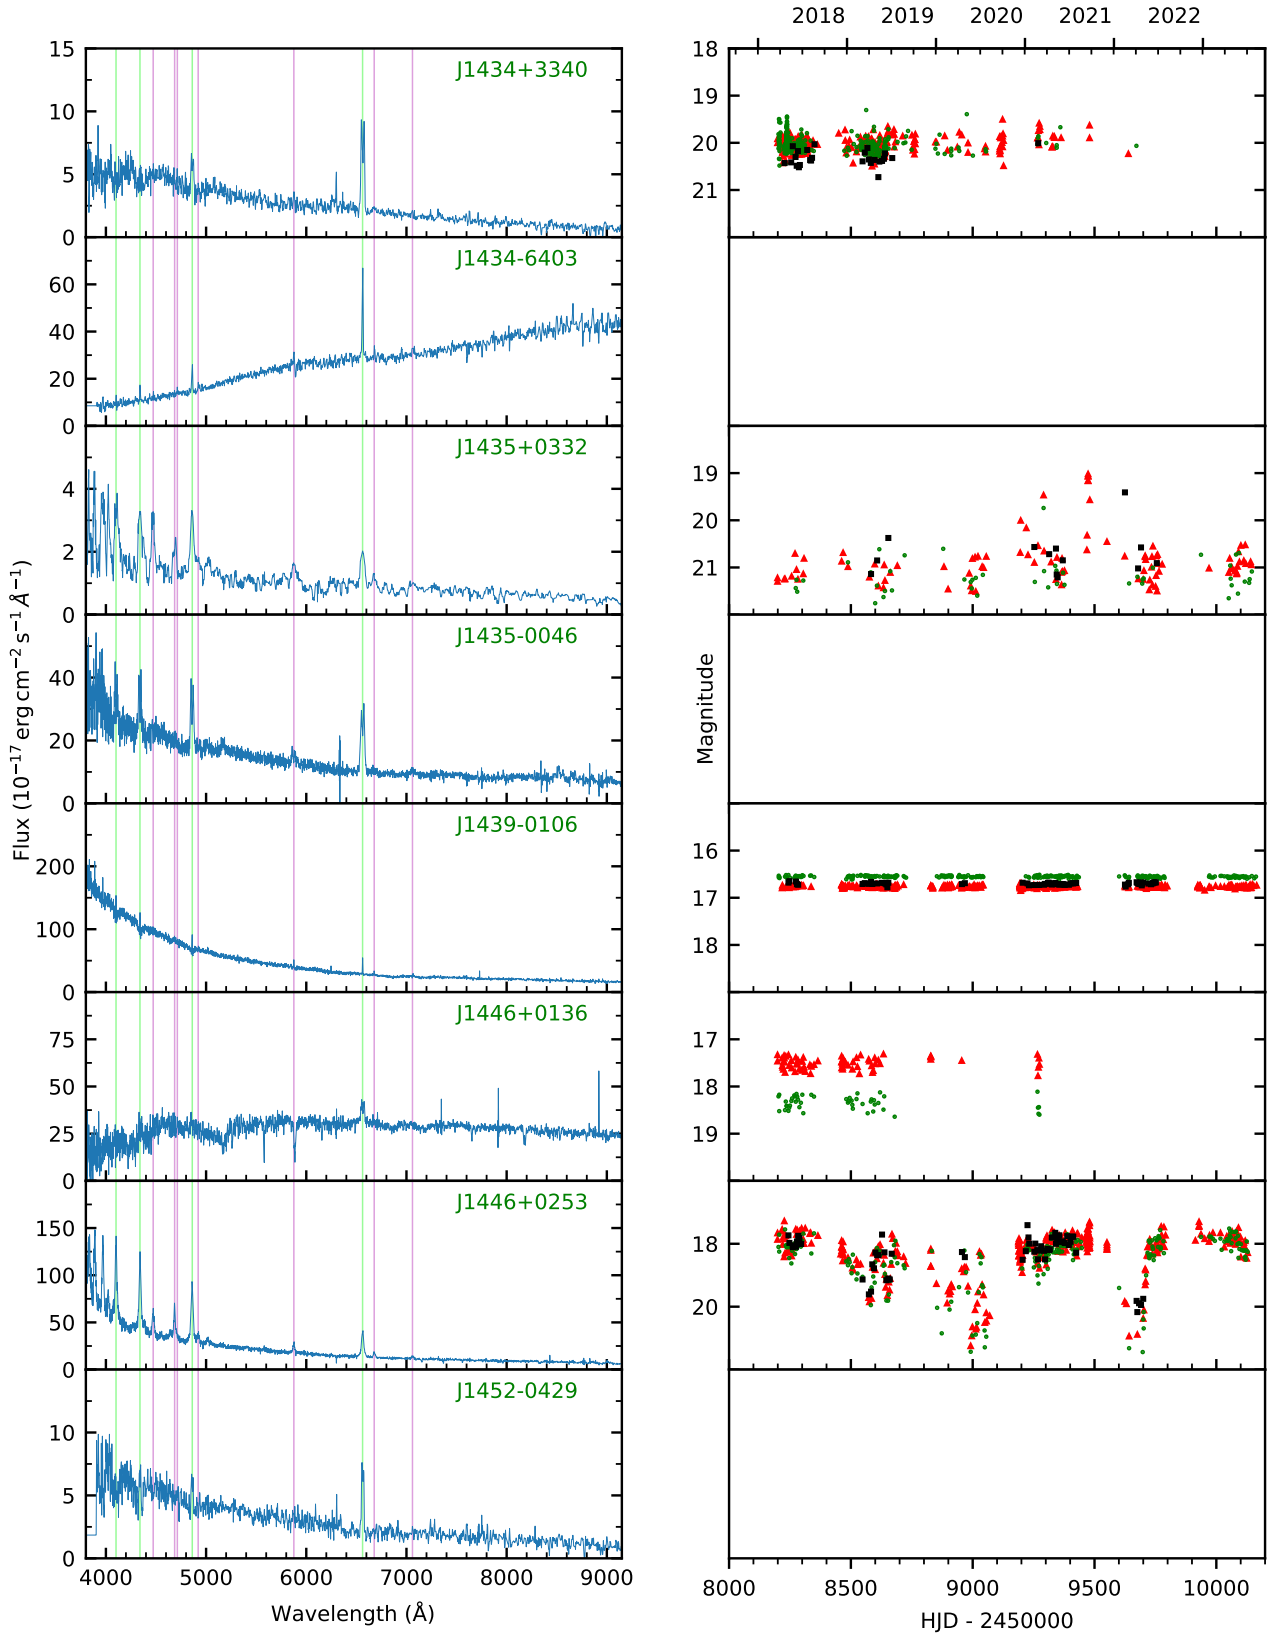

Figure 27: Left panels: Spectra with H lines shown in green and He in pink. Right panels: Light curves with ZTF *r*-band shown in red triangles, *g*-band in green dots and *i*-band in black squares.

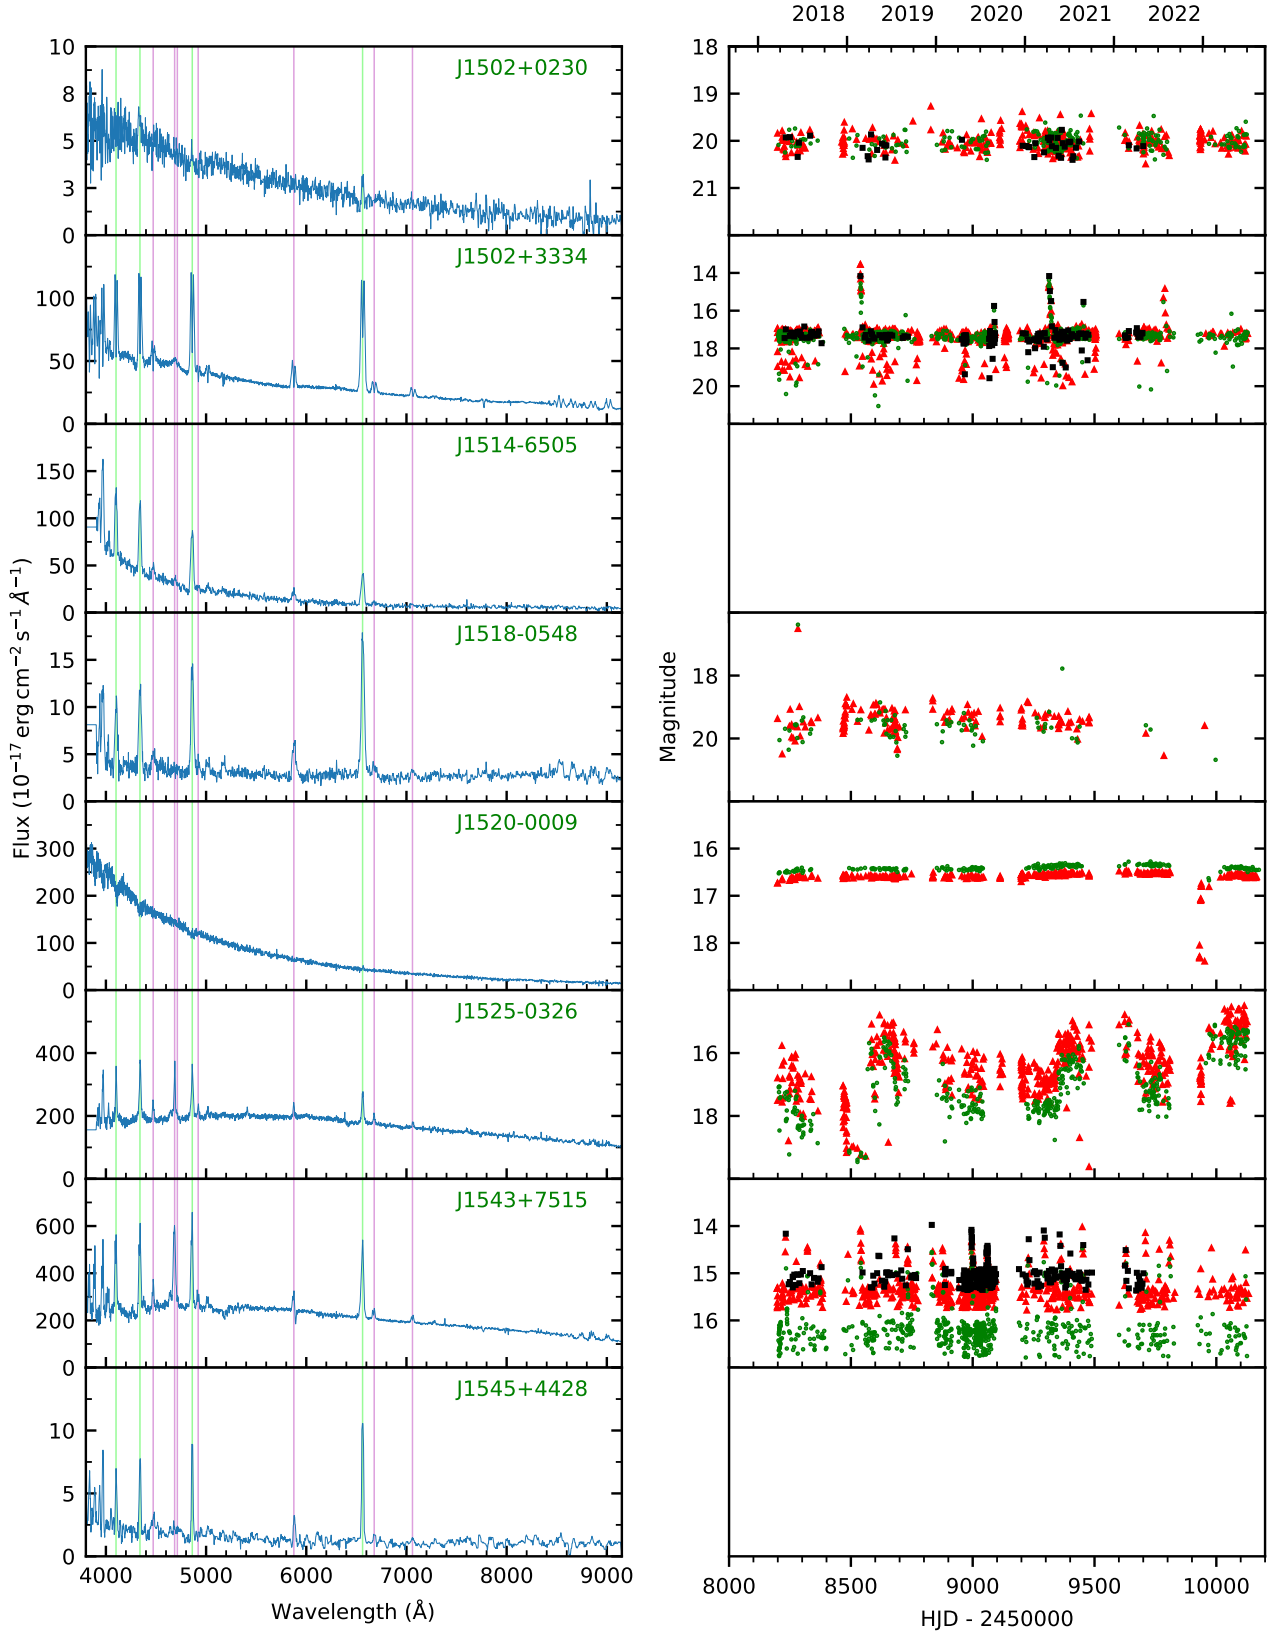

Figure 28: Left panels: Spectra with H lines shown in green and He in pink. Right panels: Light curves with ZTF  $r$ -band shown in red triangles,  $g$ -band in green dots and  $i$ -band in black squares.

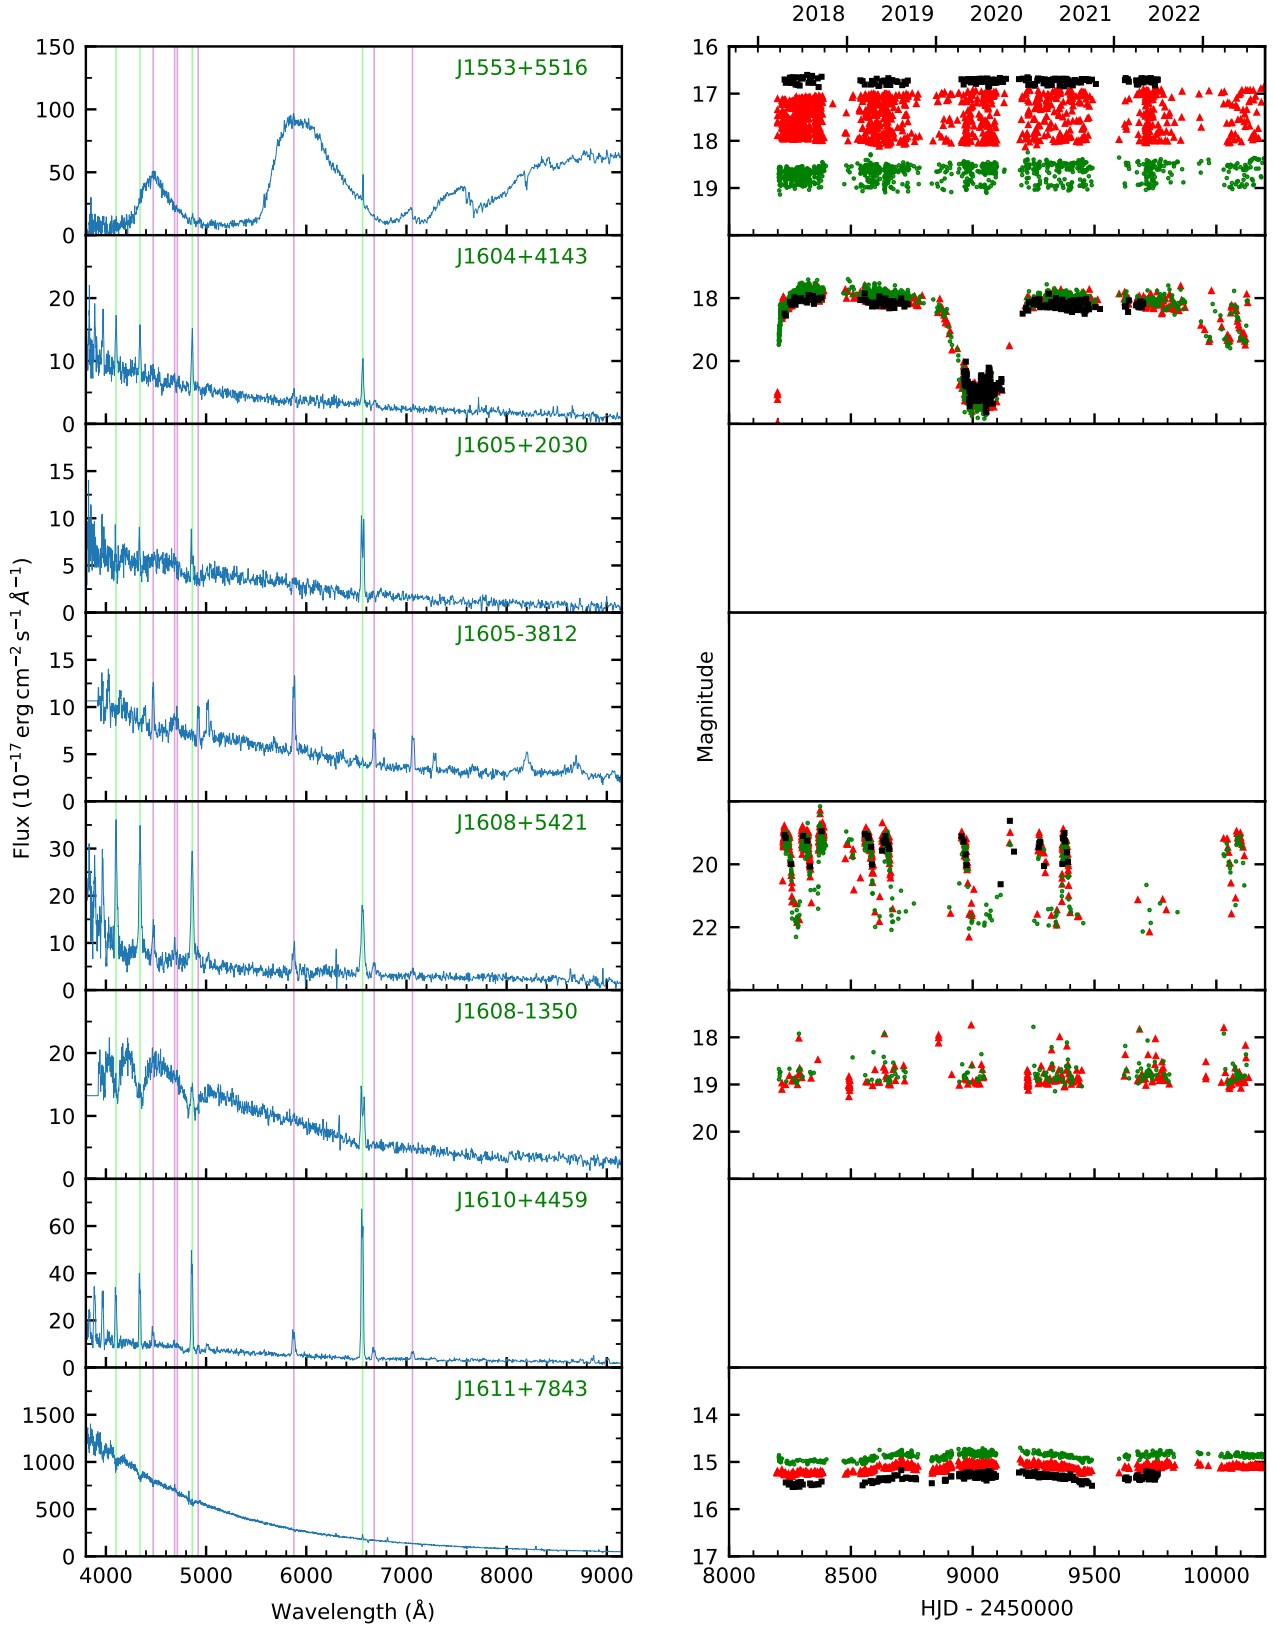

Figure 29: Left panels: Spectra with H lines shown in green and He in pink. Right panels: Light curves with ZTF  $r$ -band shown in red triangles,  $g$ -band in green dots and  $i$ -band in black squares.

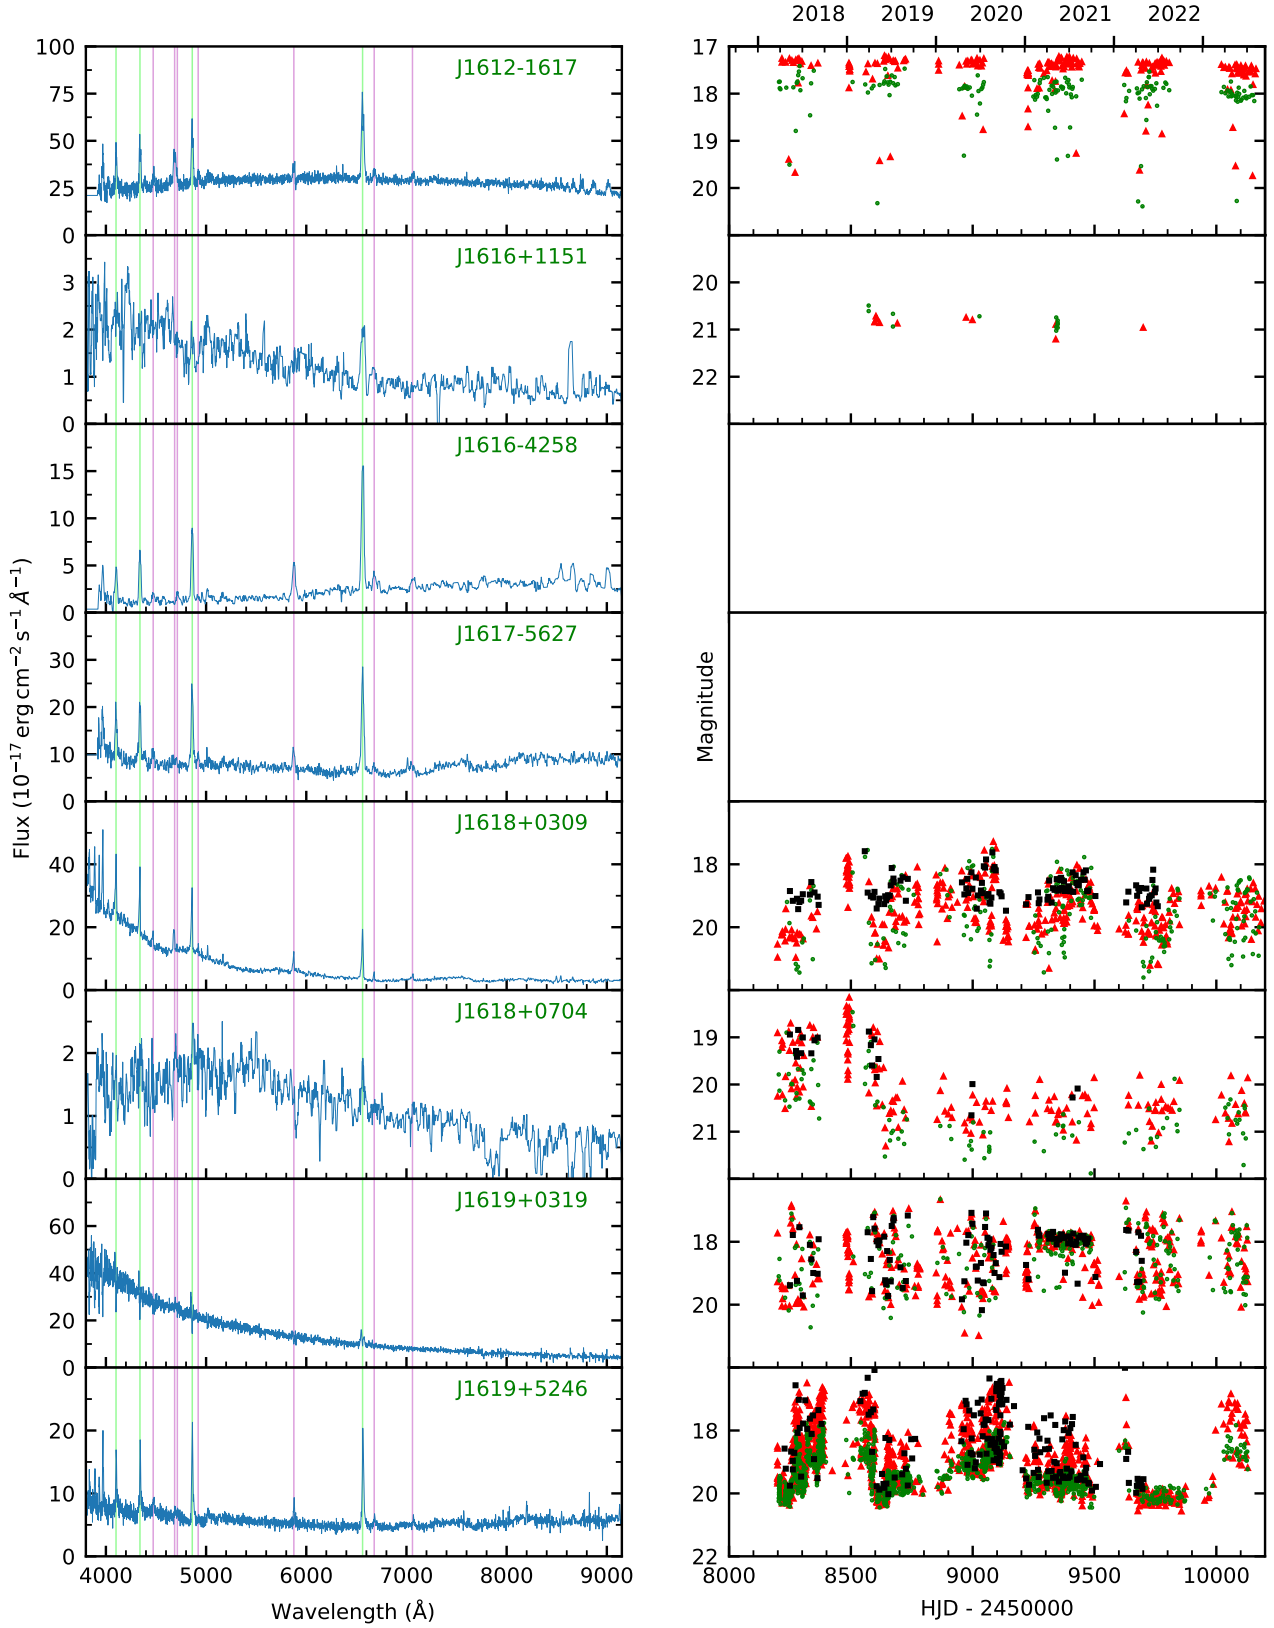

Figure 30: Left panels: Spectra with H lines shown in green and He in pink. Right panels: Light curves with ZTF  $r$ -band shown in red triangles,  $g$ -band in green dots and  $i$ -band in black squares.

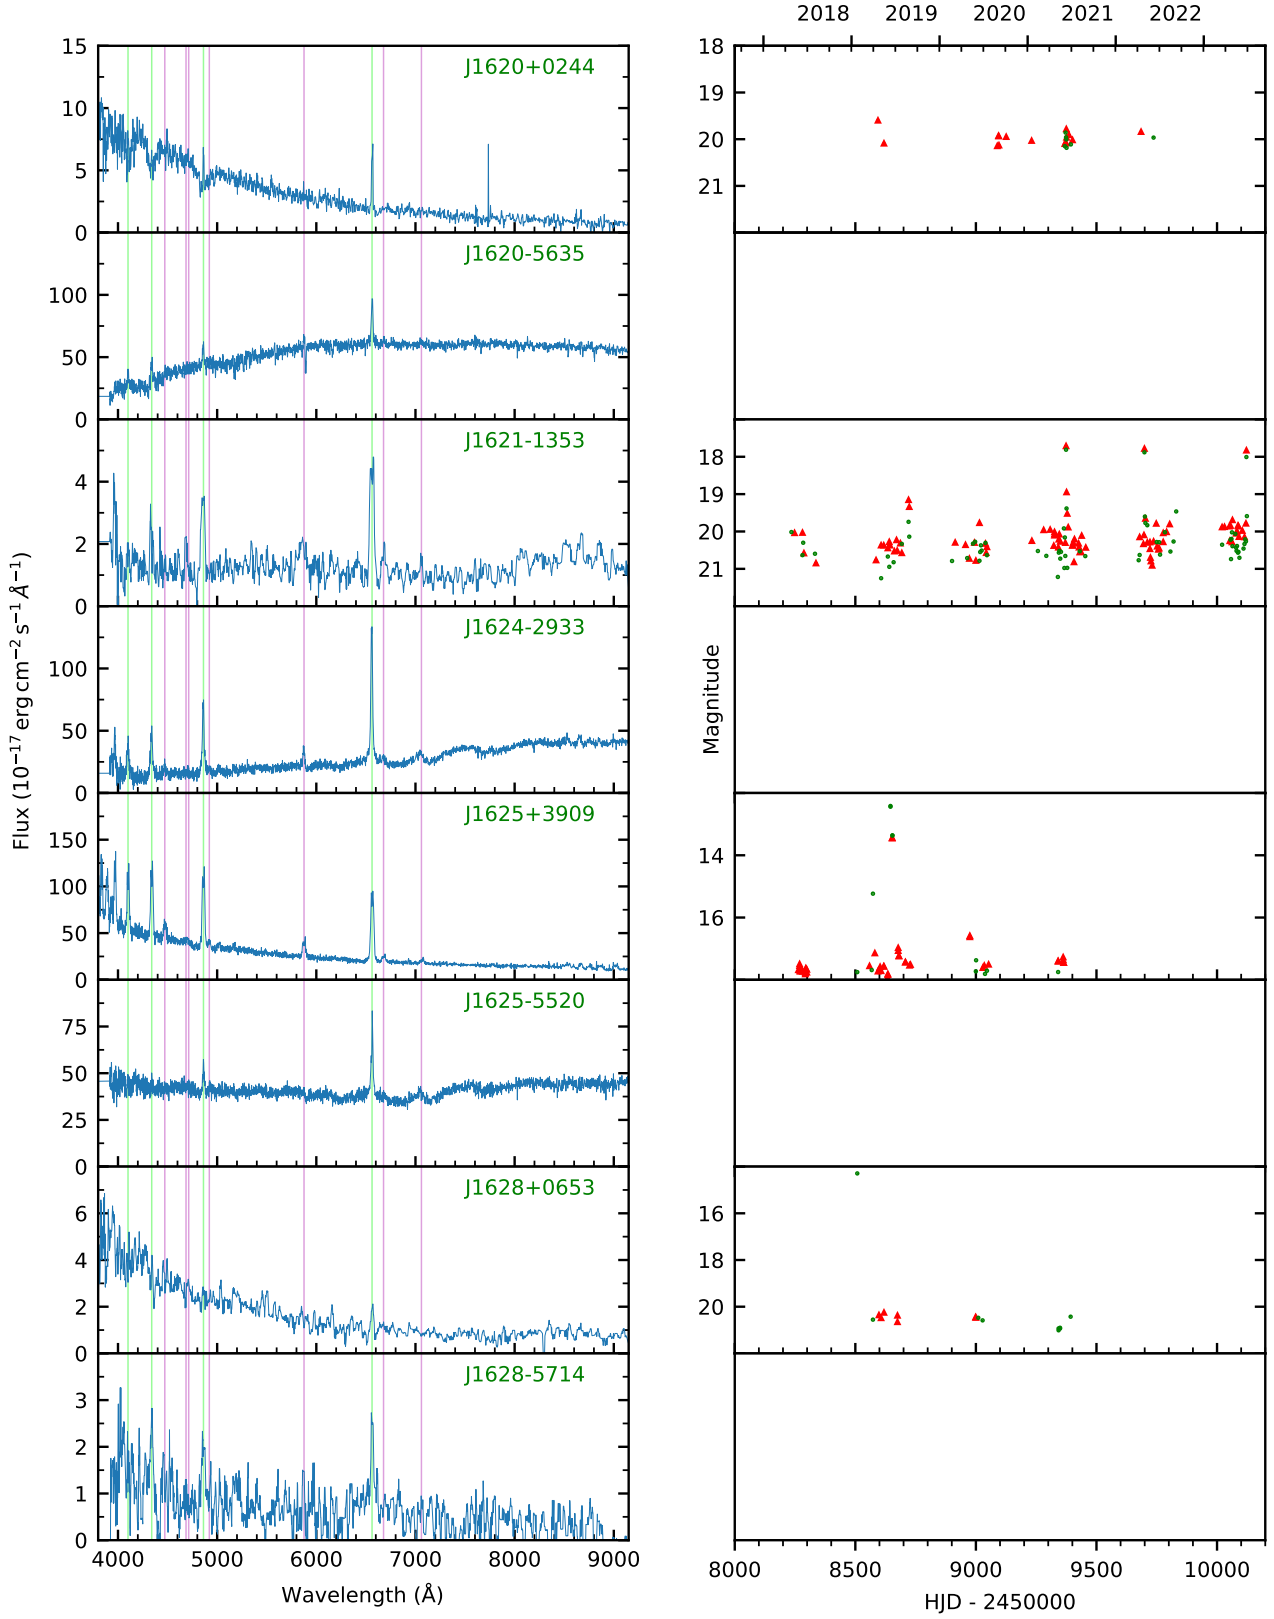

Figure 31: Left panels: Spectra with H lines shown in green and He in pink. Right panels: Light curves with ZTF  $r$ -band shown in red triangles,  $g$ -band in green dots and  $i$ -band in black squares.

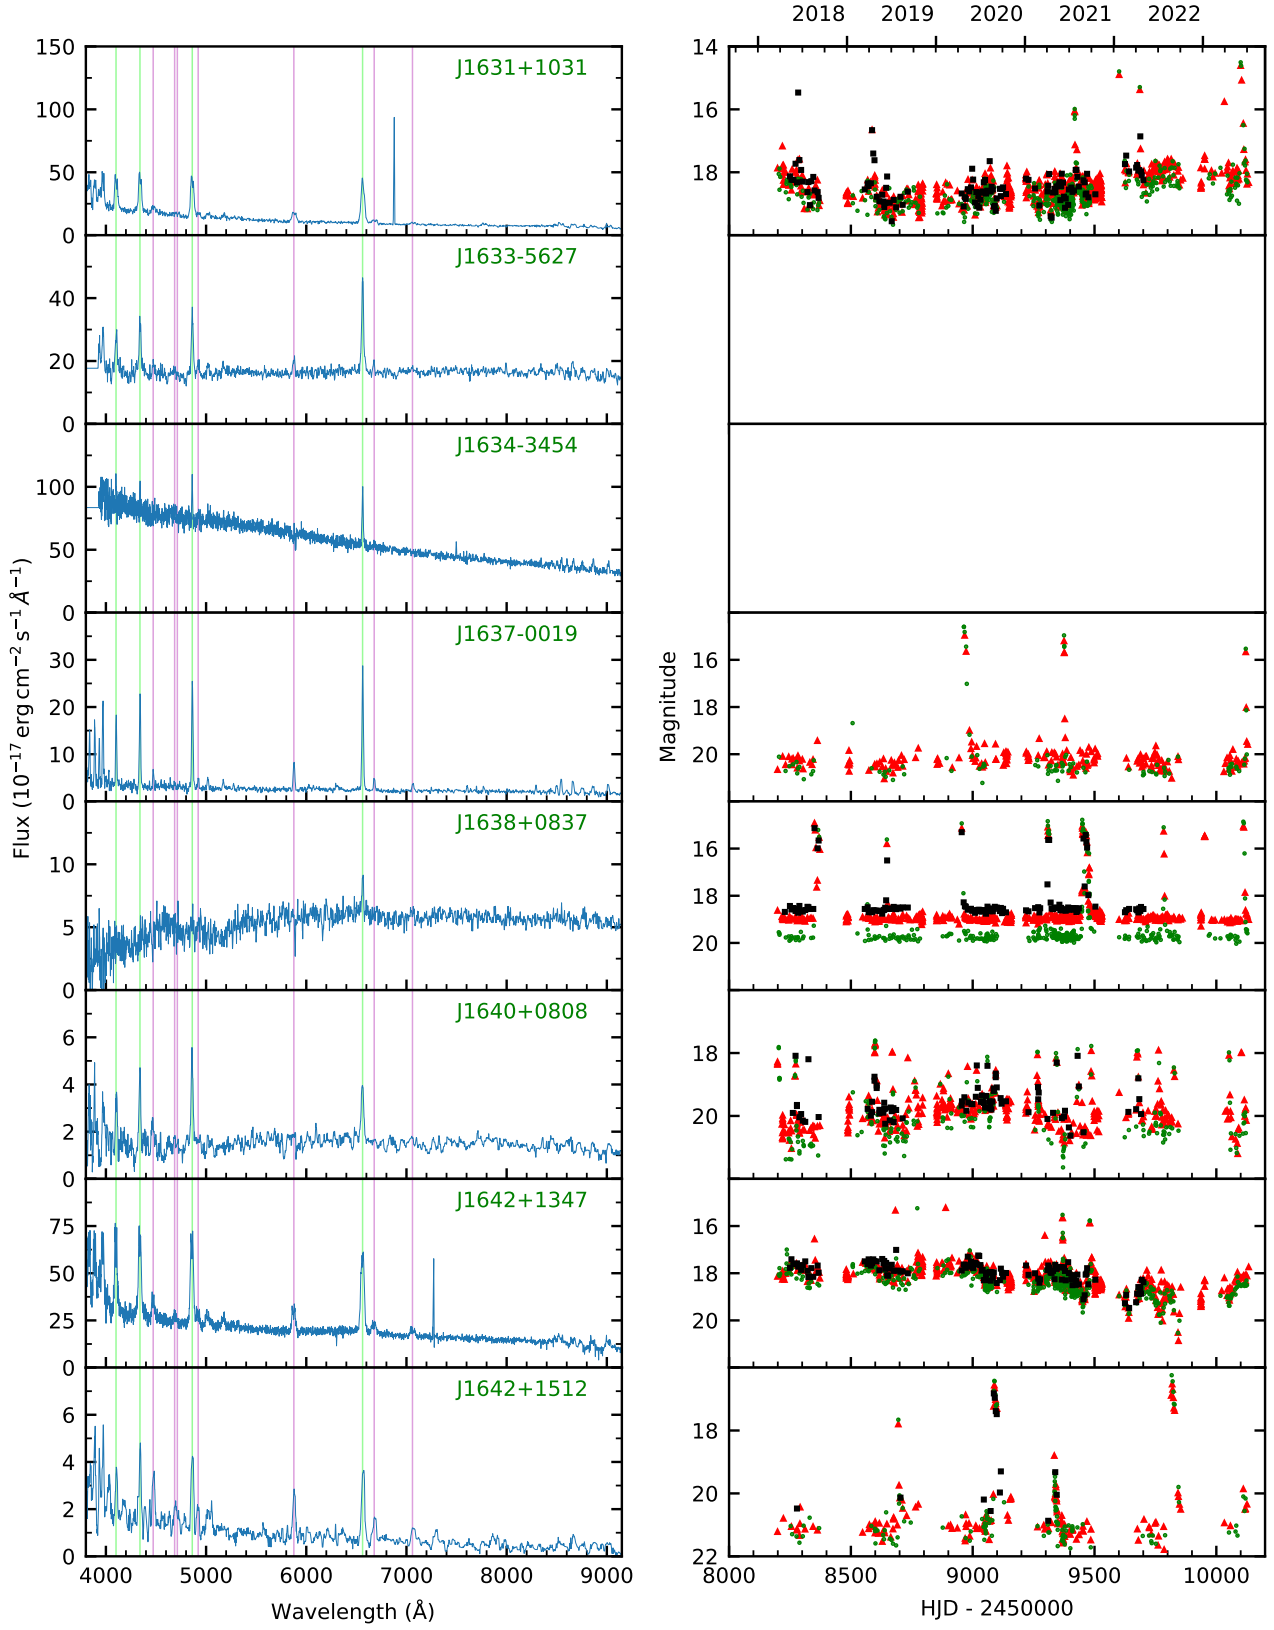

Figure 32: Left panels: Spectra with H lines shown in green and He in pink. Right panels: Light curves with ZTF  $r$ -band shown in red triangles,  $g$ -band in green dots and  $i$ -band in black squares.



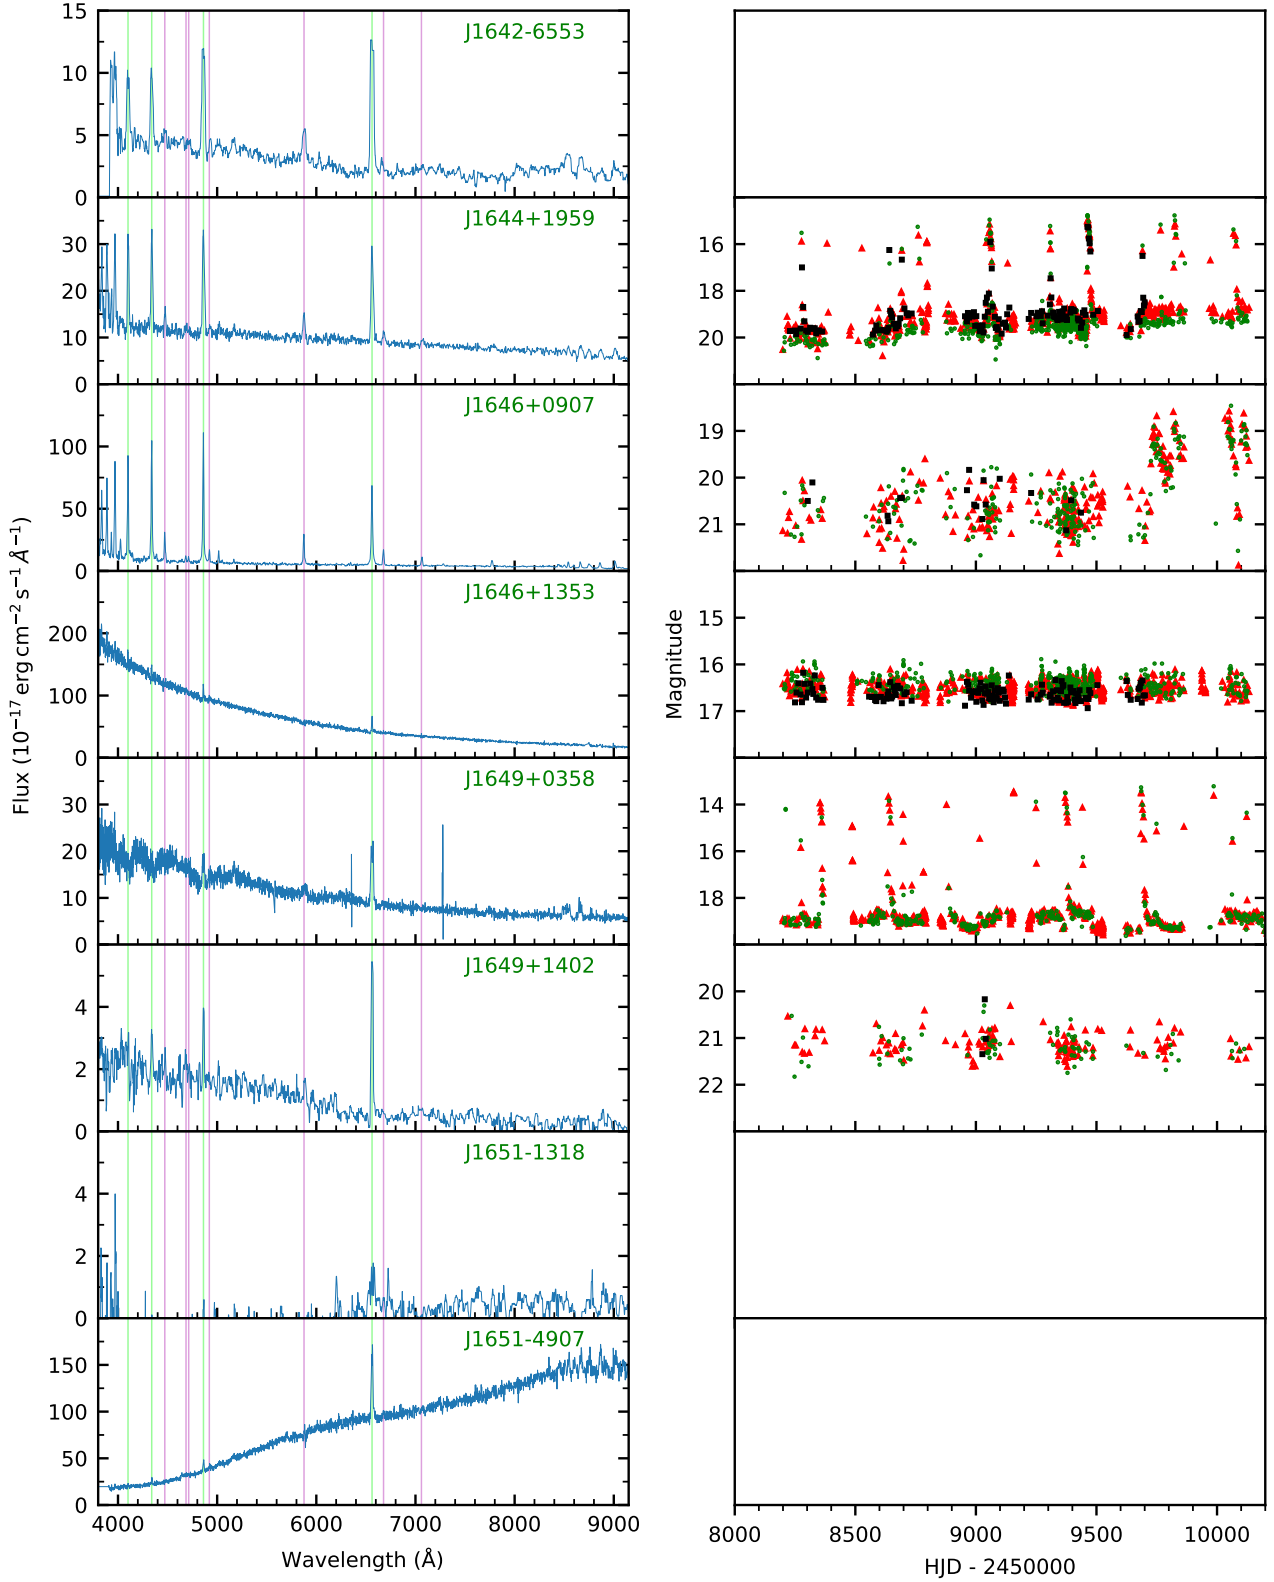

Figure 33: Left panels: Spectra with H lines shown in green and He in pink. Right panels: Light curves with ZTF  $r$ -band shown in red triangles,  $g$ -band in green dots and  $i$ -band in black squares.

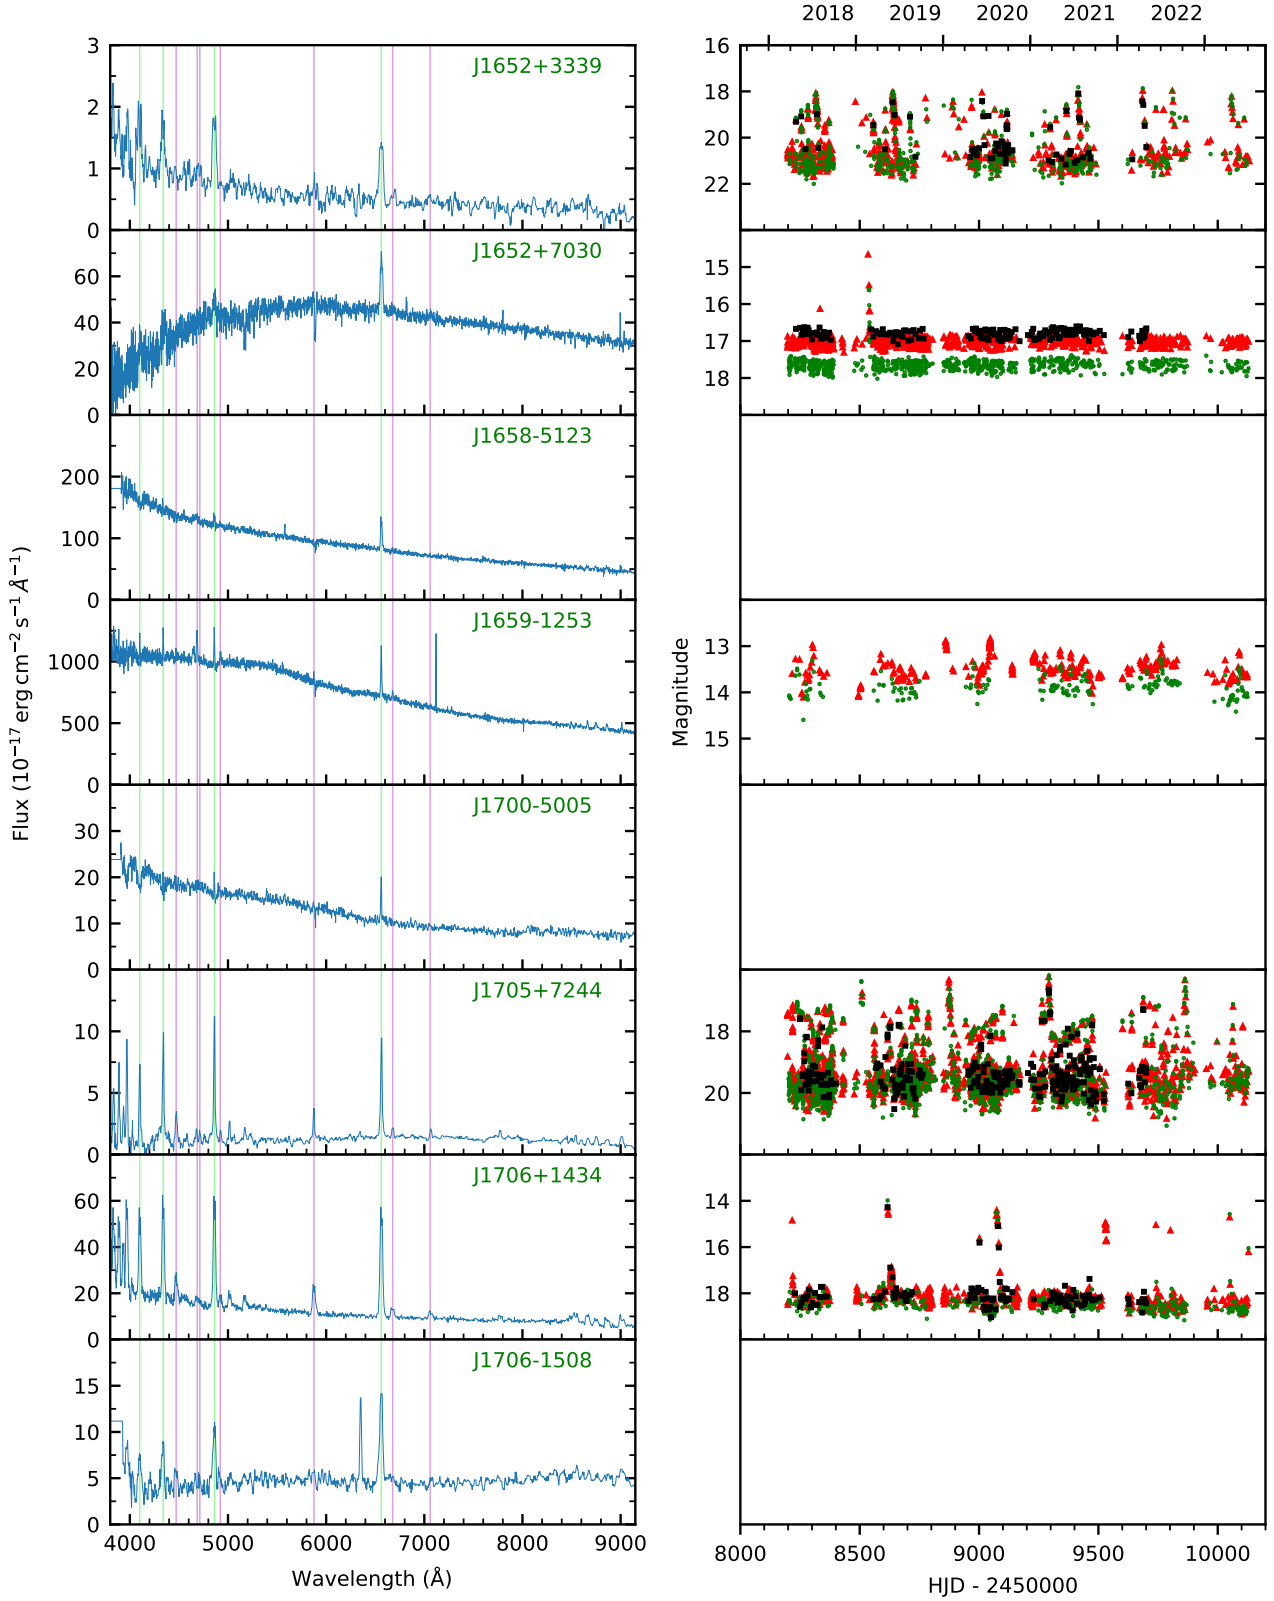

Figure 34: Left panels: Spectra with H lines shown in green and He in pink. Right panels: Light curves with ZTF  $r$ -band shown in red triangles,  $g$ -band in green dots and  $i$ -band in black squares.

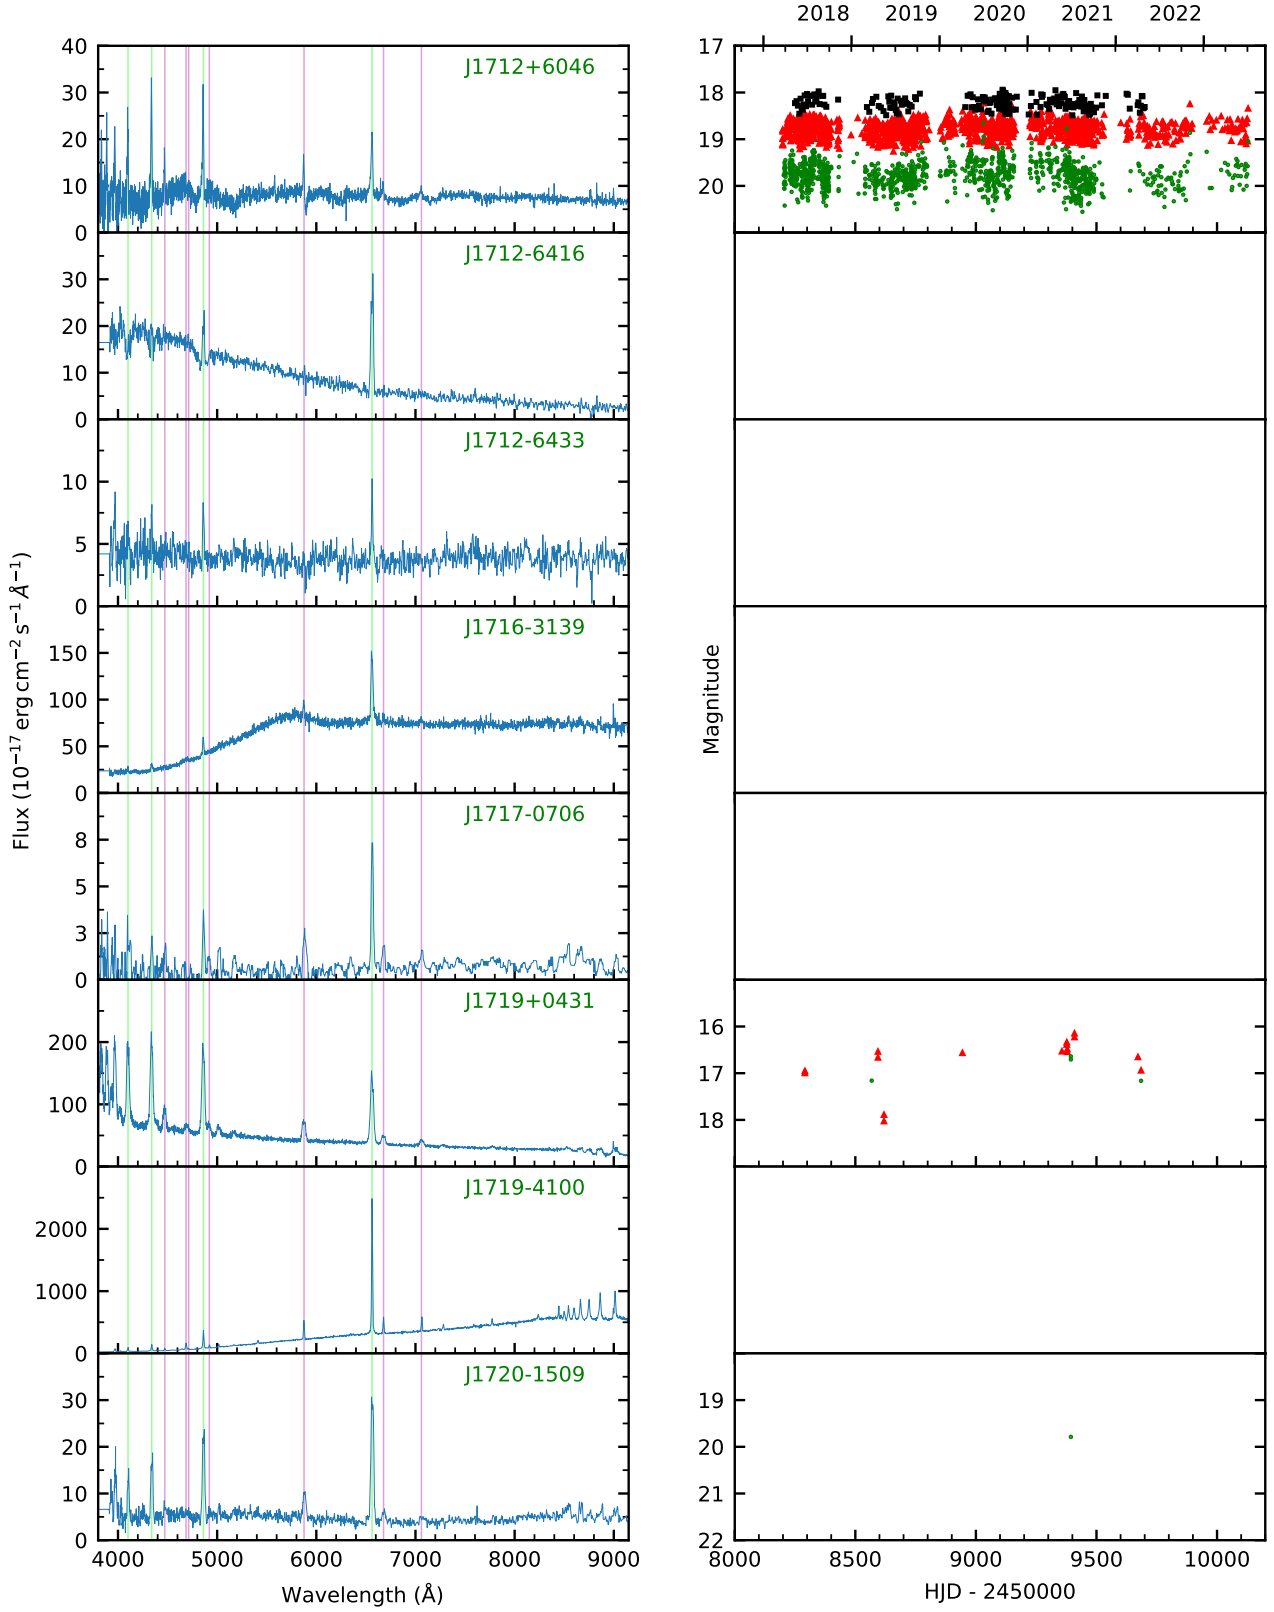

Figure 35: Left panels: Spectra with H lines shown in green and He in pink. Right panels: Light curves with ZTF *r*-band shown in red triangles, *g*-band in green dots and *i*-band in black squares.

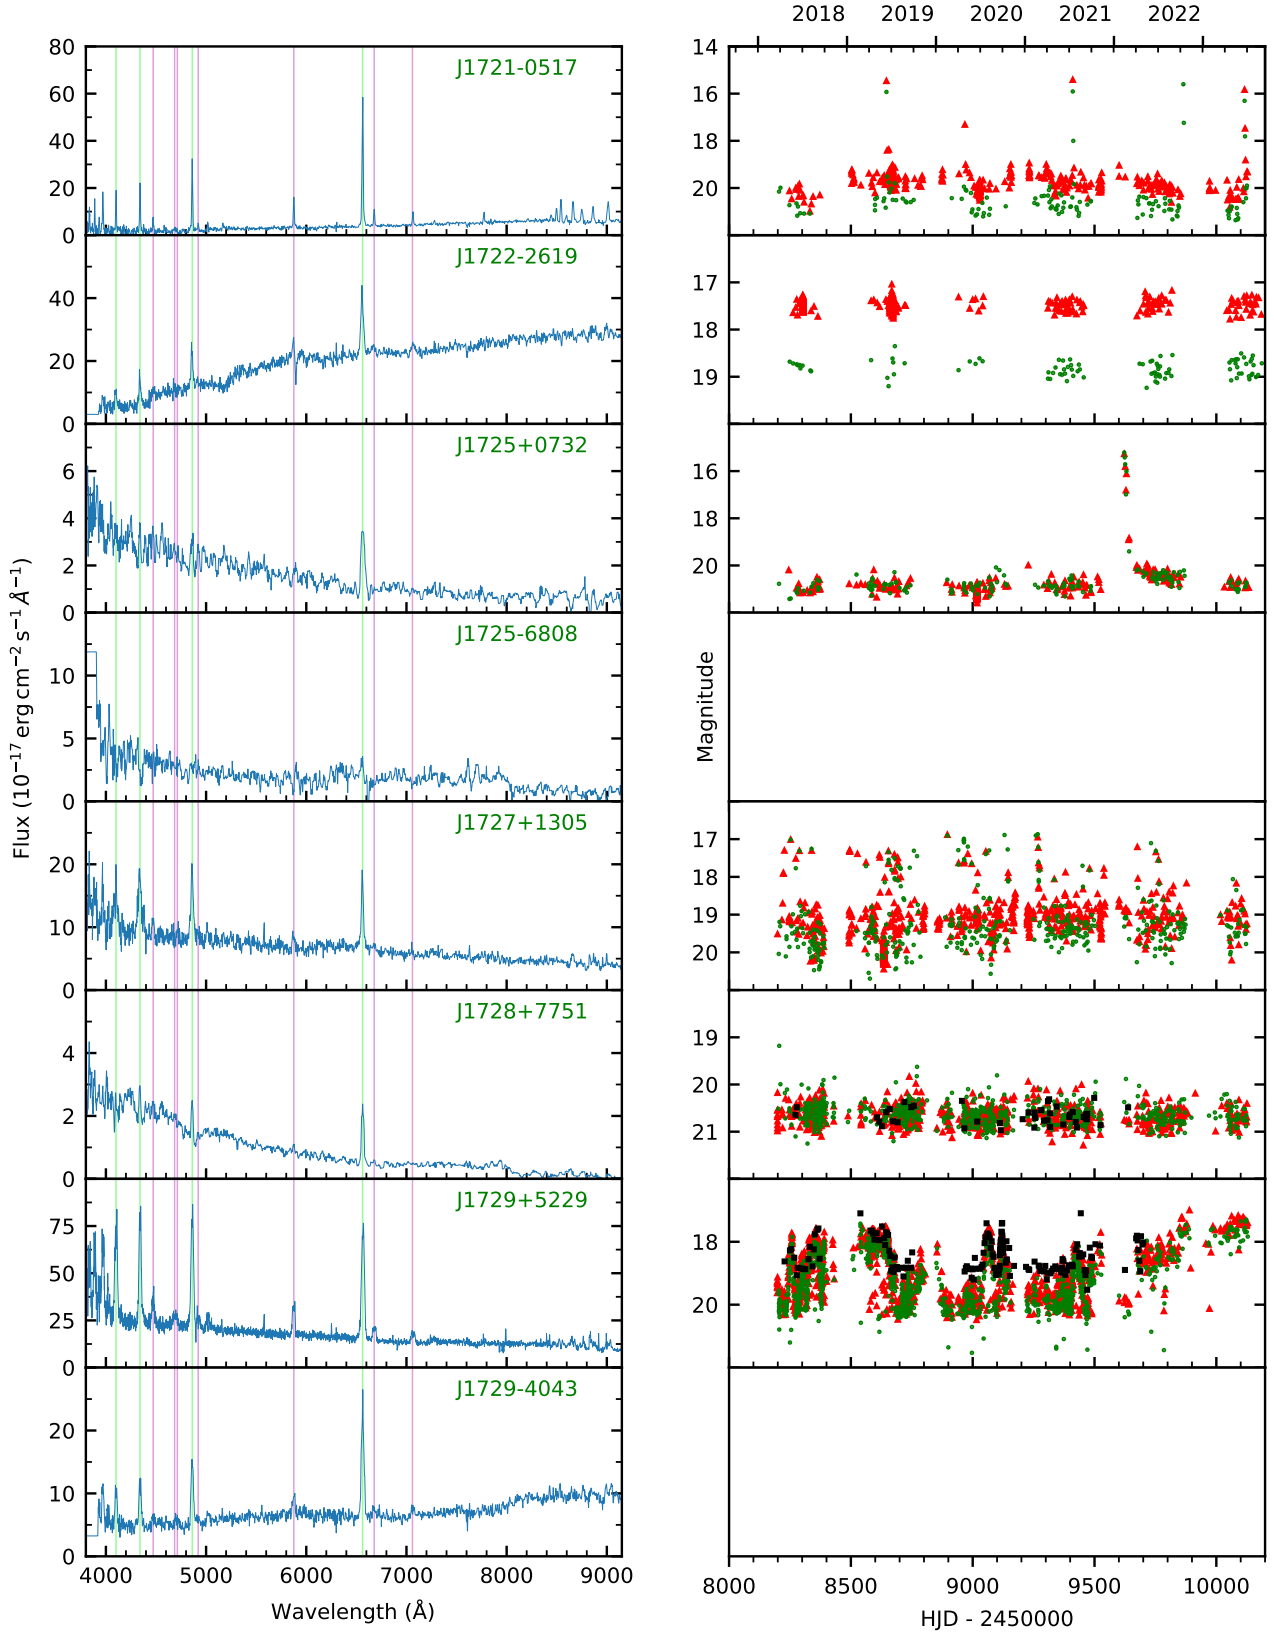

Figure 36: Left panels: Spectra with H lines shown in green and He in pink. Right panels: Light curves with ZTF  $r$ -band shown in red triangles,  $g$ -band in green dots and  $i$ -band in black squares.

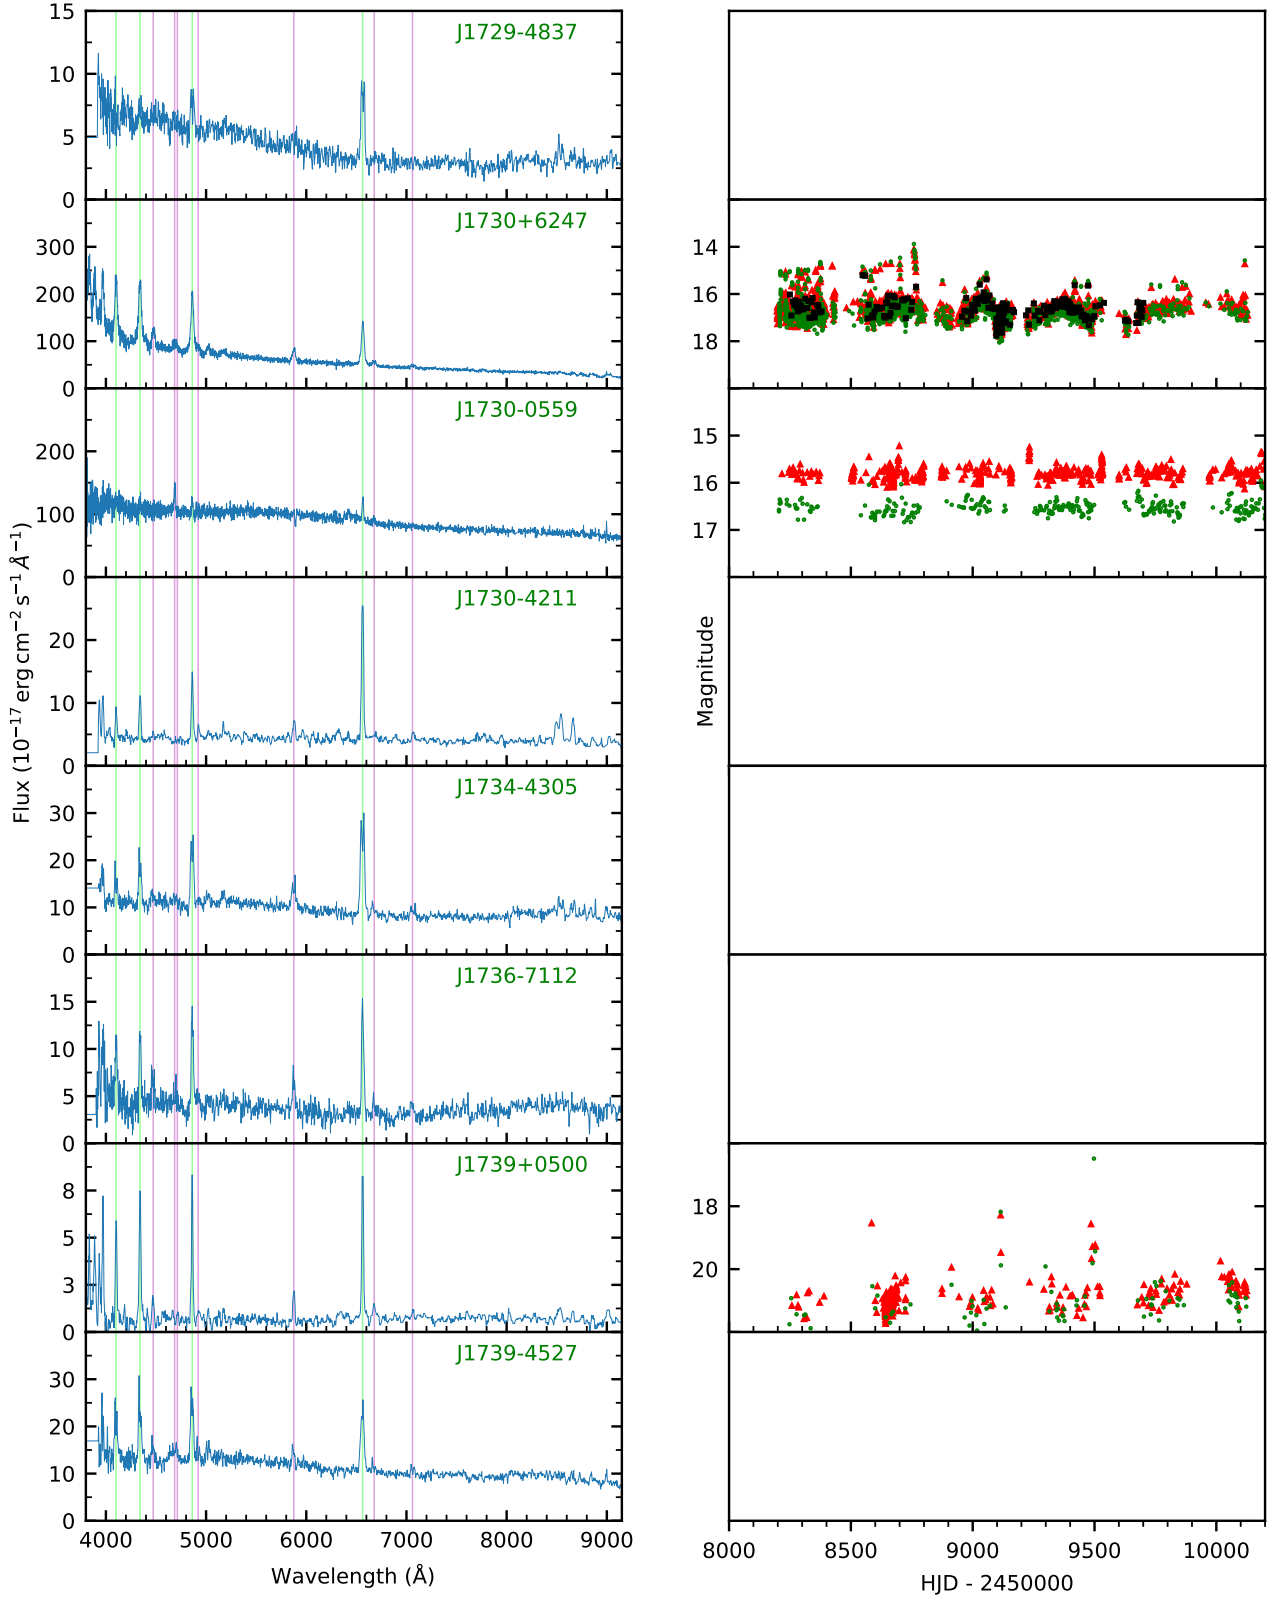

Figure 37: Left panels: Spectra with H lines shown in green and He in pink. Right panels: Light curves with ZTF *r*-band shown in red triangles, *g*-band in green dots and *i*-band in black squares.

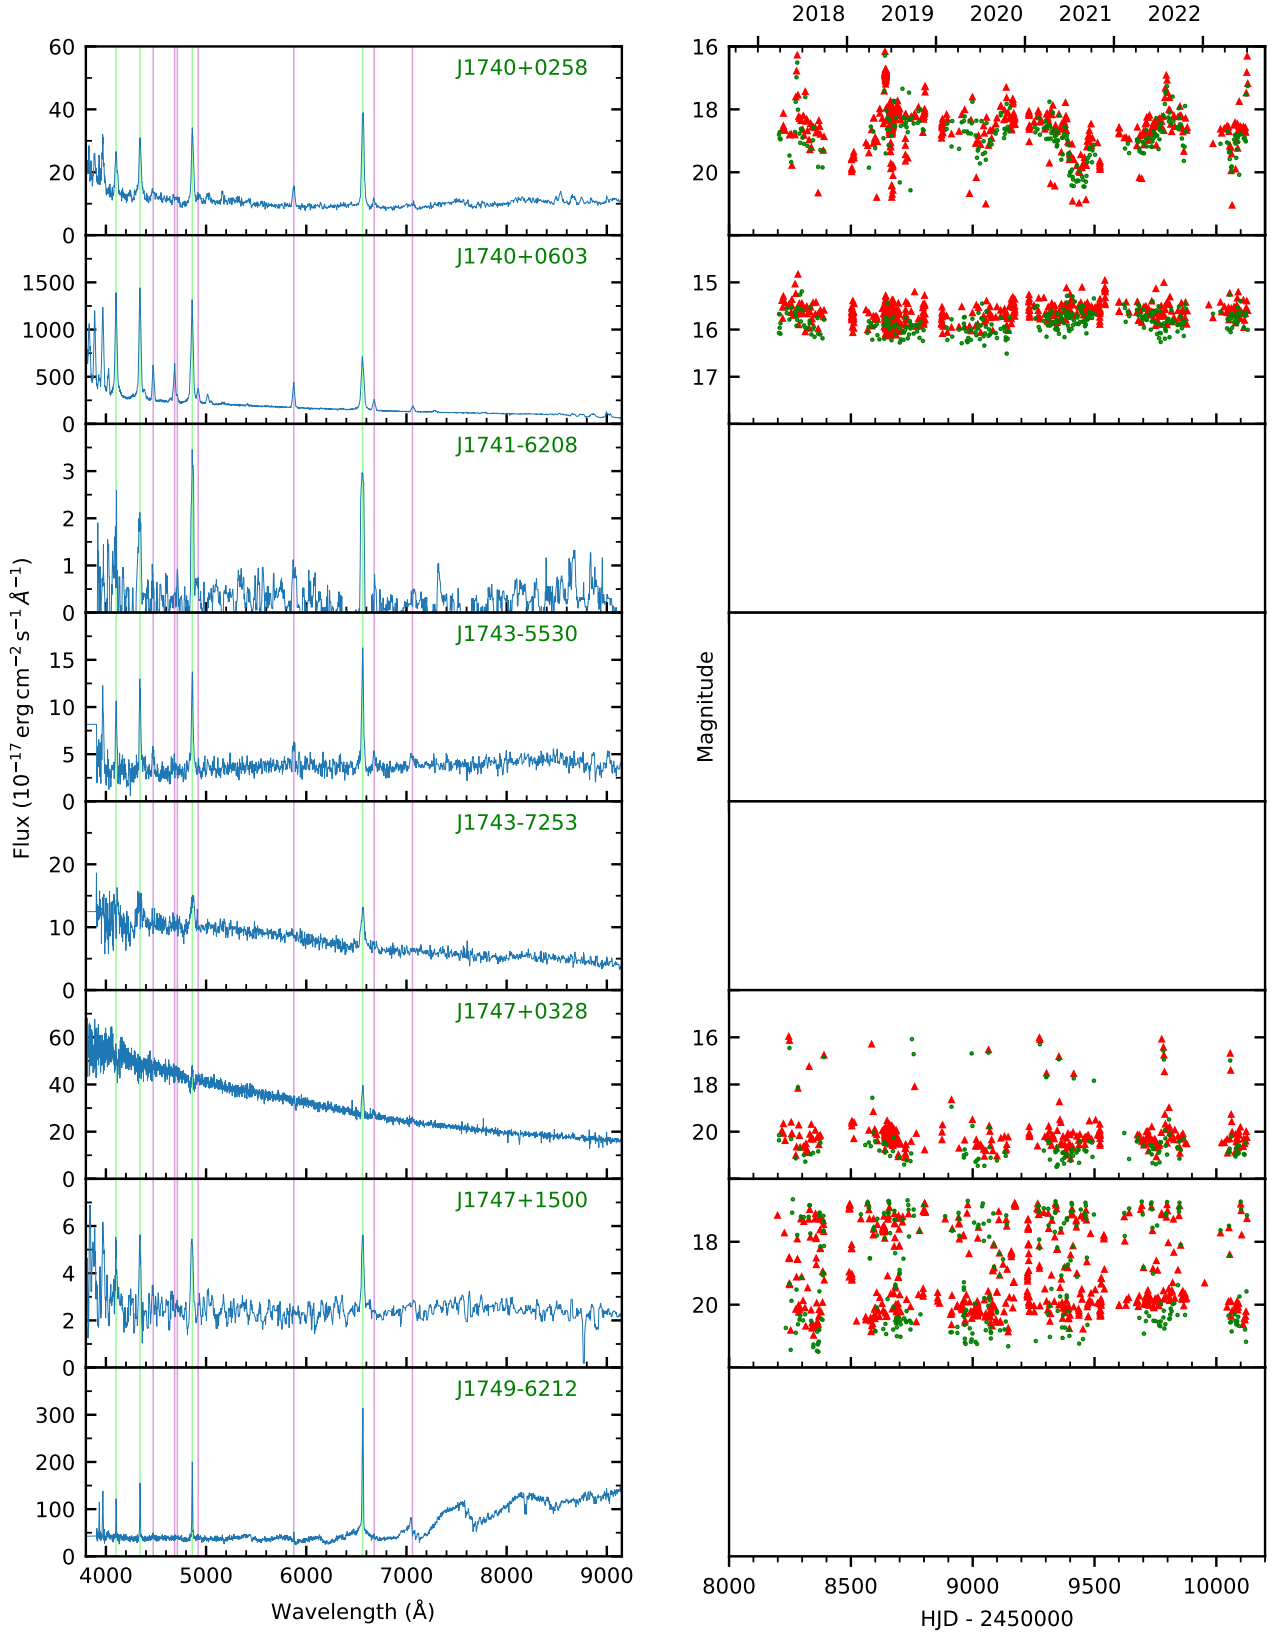

Figure 38: Left panels: Spectra with H lines shown in green and He in pink. Right panels: Light curves with ZTF  $r$ -band shown in red triangles,  $g$ -band in green dots and  $i$ -band in black squares.

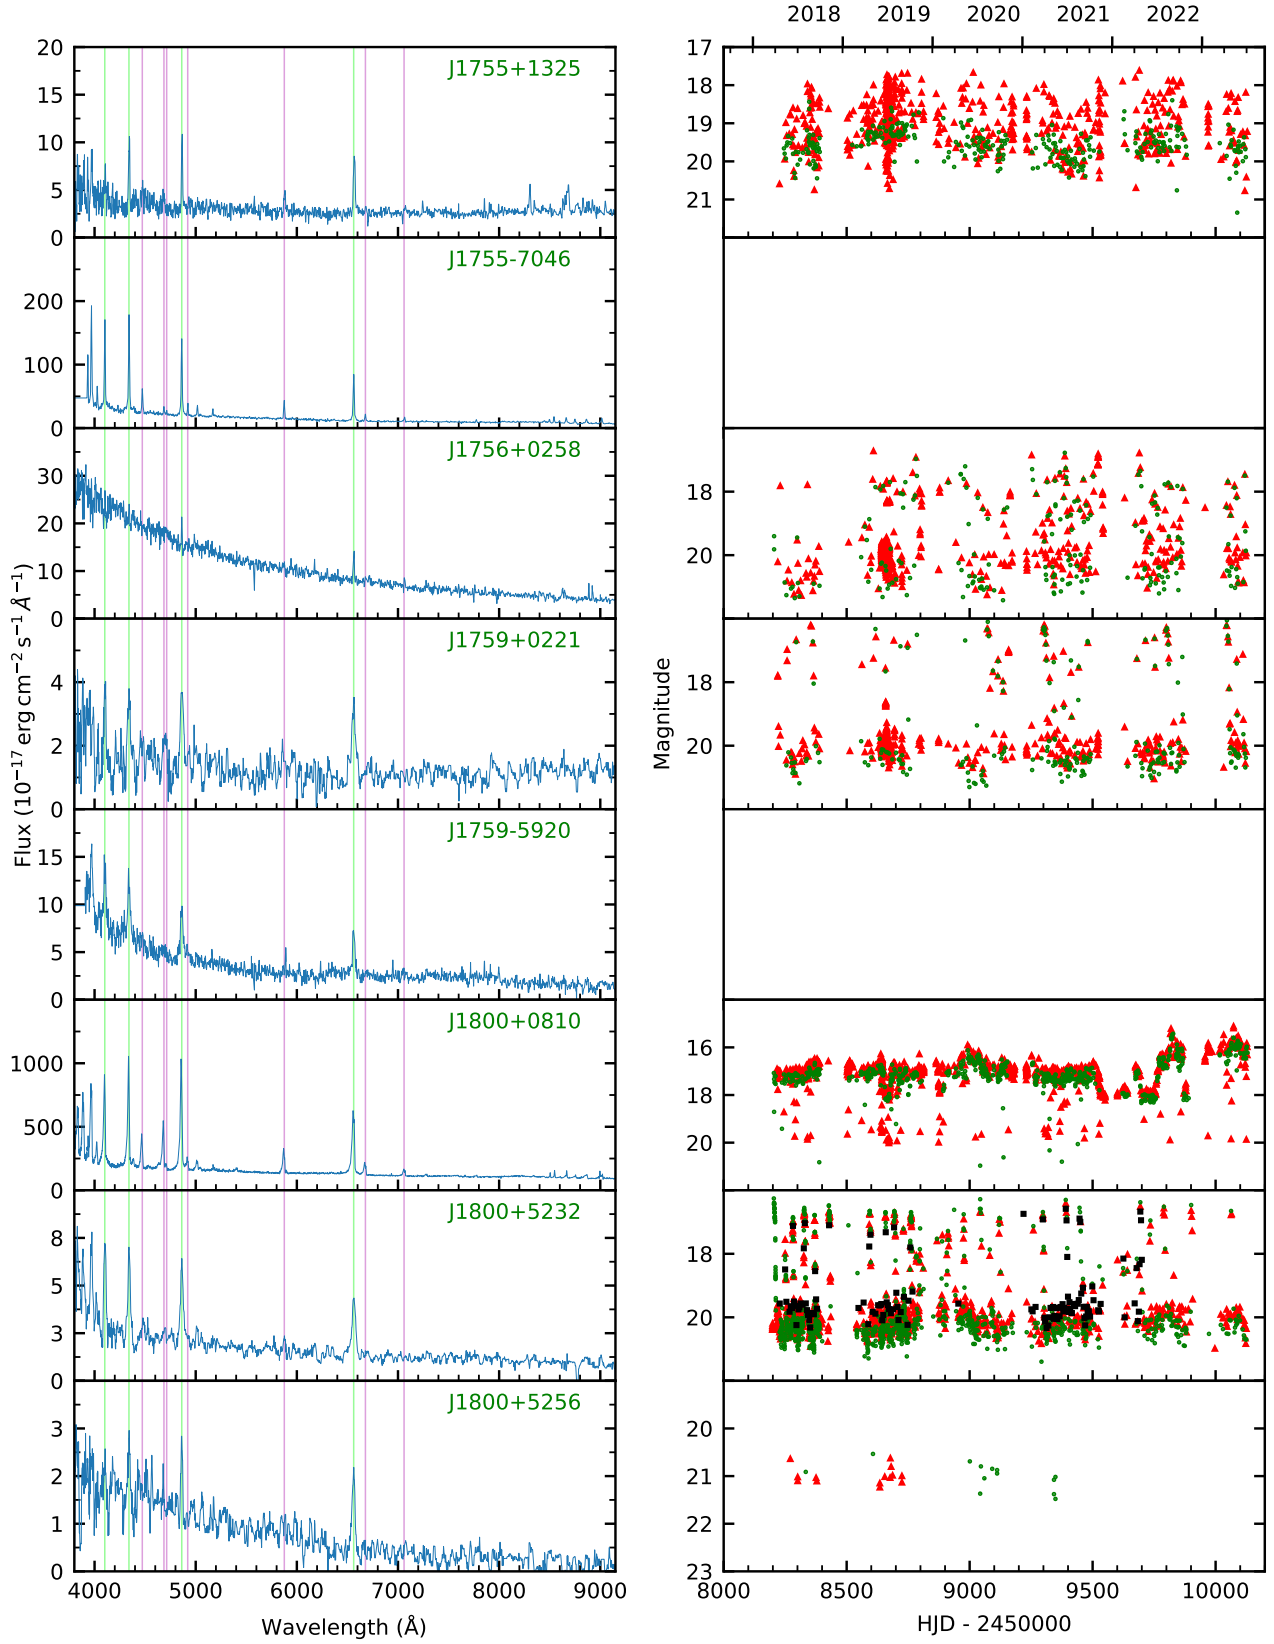

Figure 39: Left panels: Spectra with H lines shown in green and He in pink. Right panels: Light curves with ZTF *r*-band shown in red triangles, *g*-band in green dots and *i*-band in black squares.



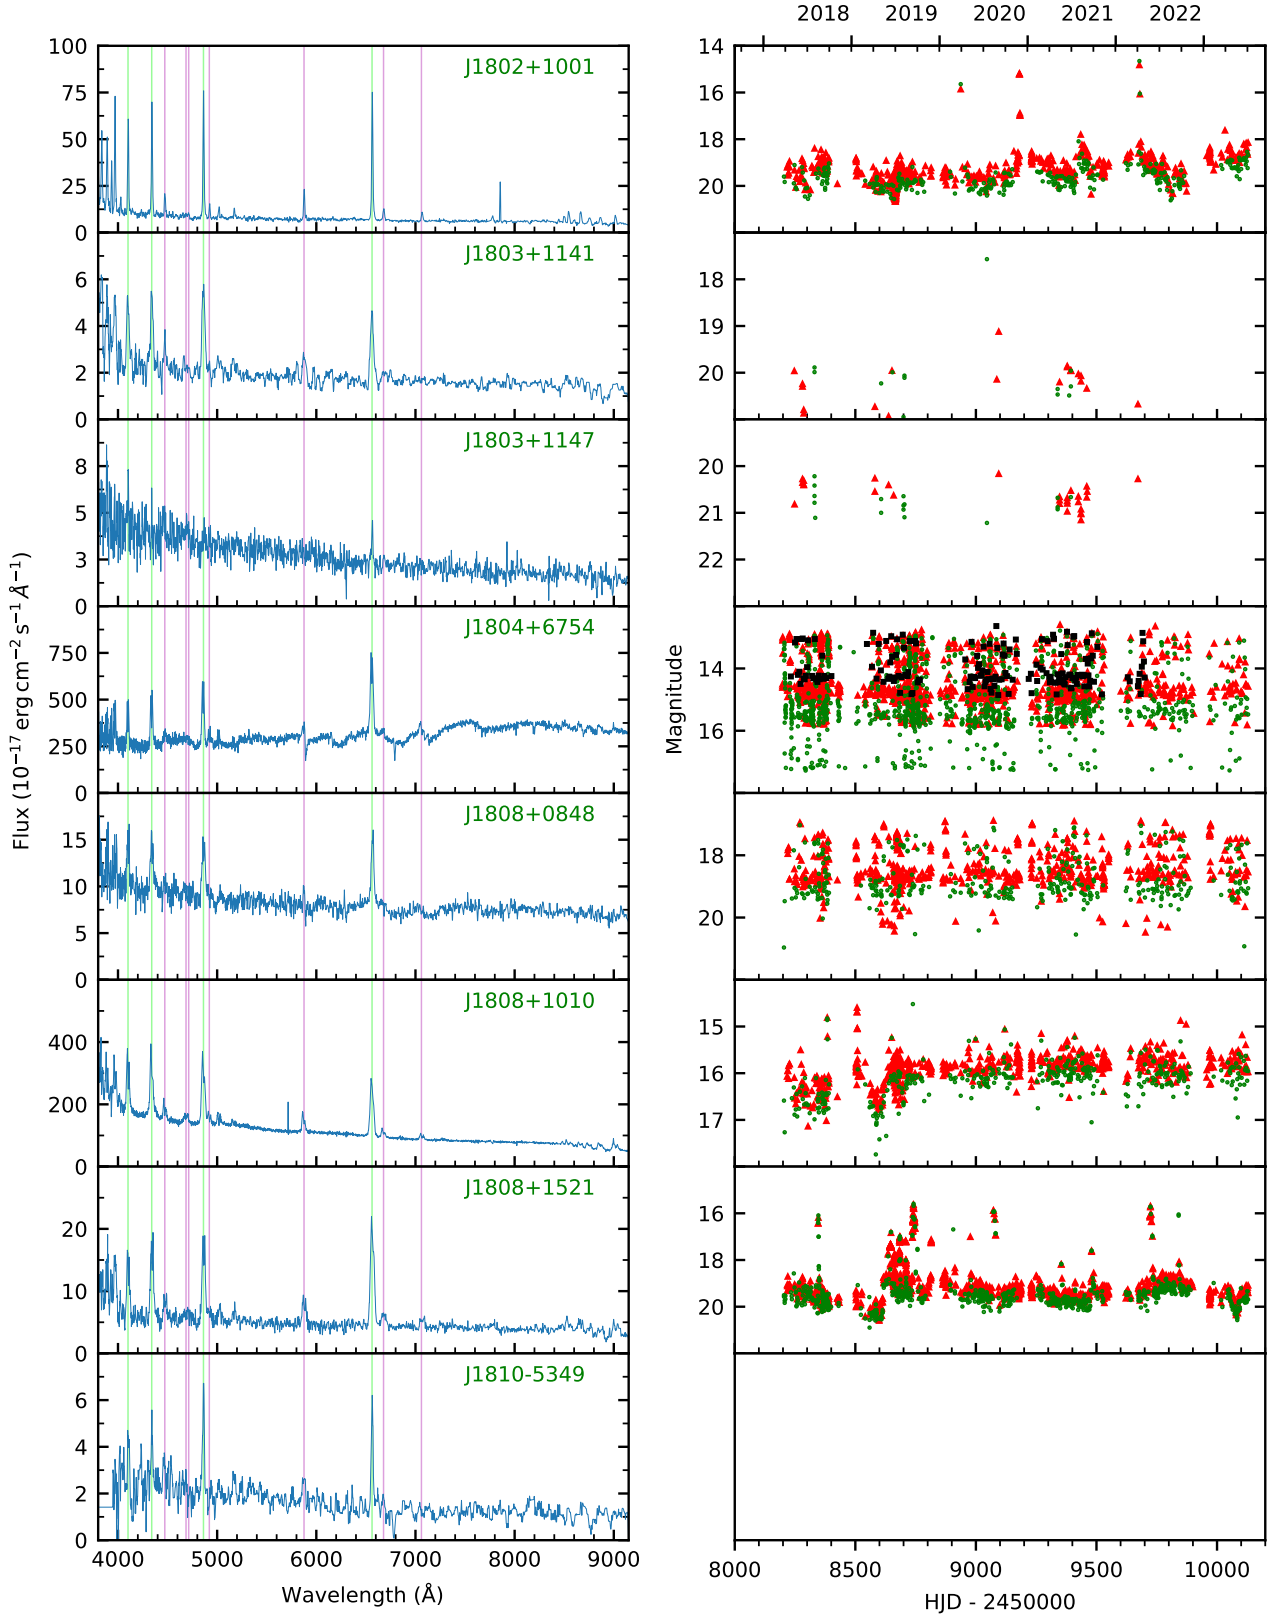

Figure 40: Left panels: Spectra with H lines shown in green and He in pink. Right panels: Light curves with ZTF  $r$ -band shown in red triangles,  $g$ -band in green dots and  $i$ -band in black squares.

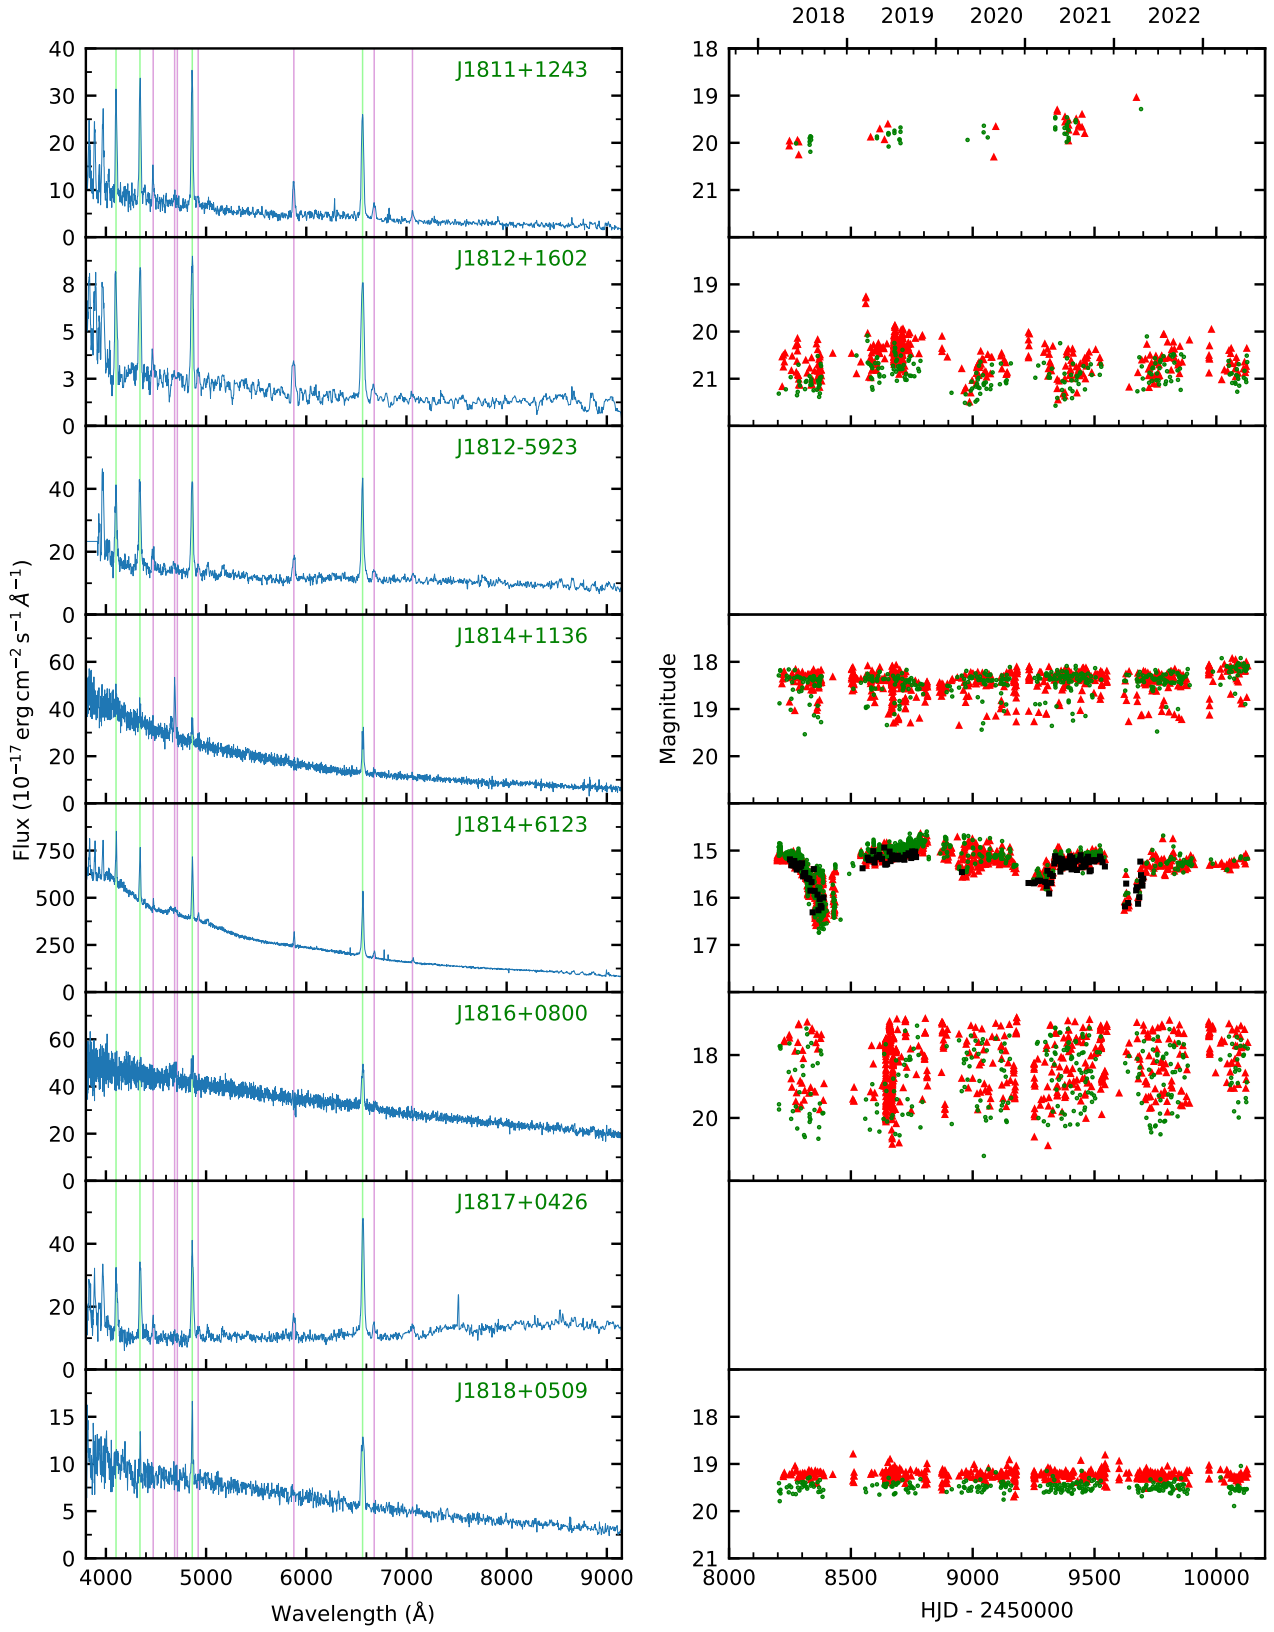

Figure 41: Left panels: Spectra with H lines shown in green and He in pink. Right panels: Light curves with ZTF *r*-band shown in red triangles, *g*-band in green dots and *i*-band in black squares.

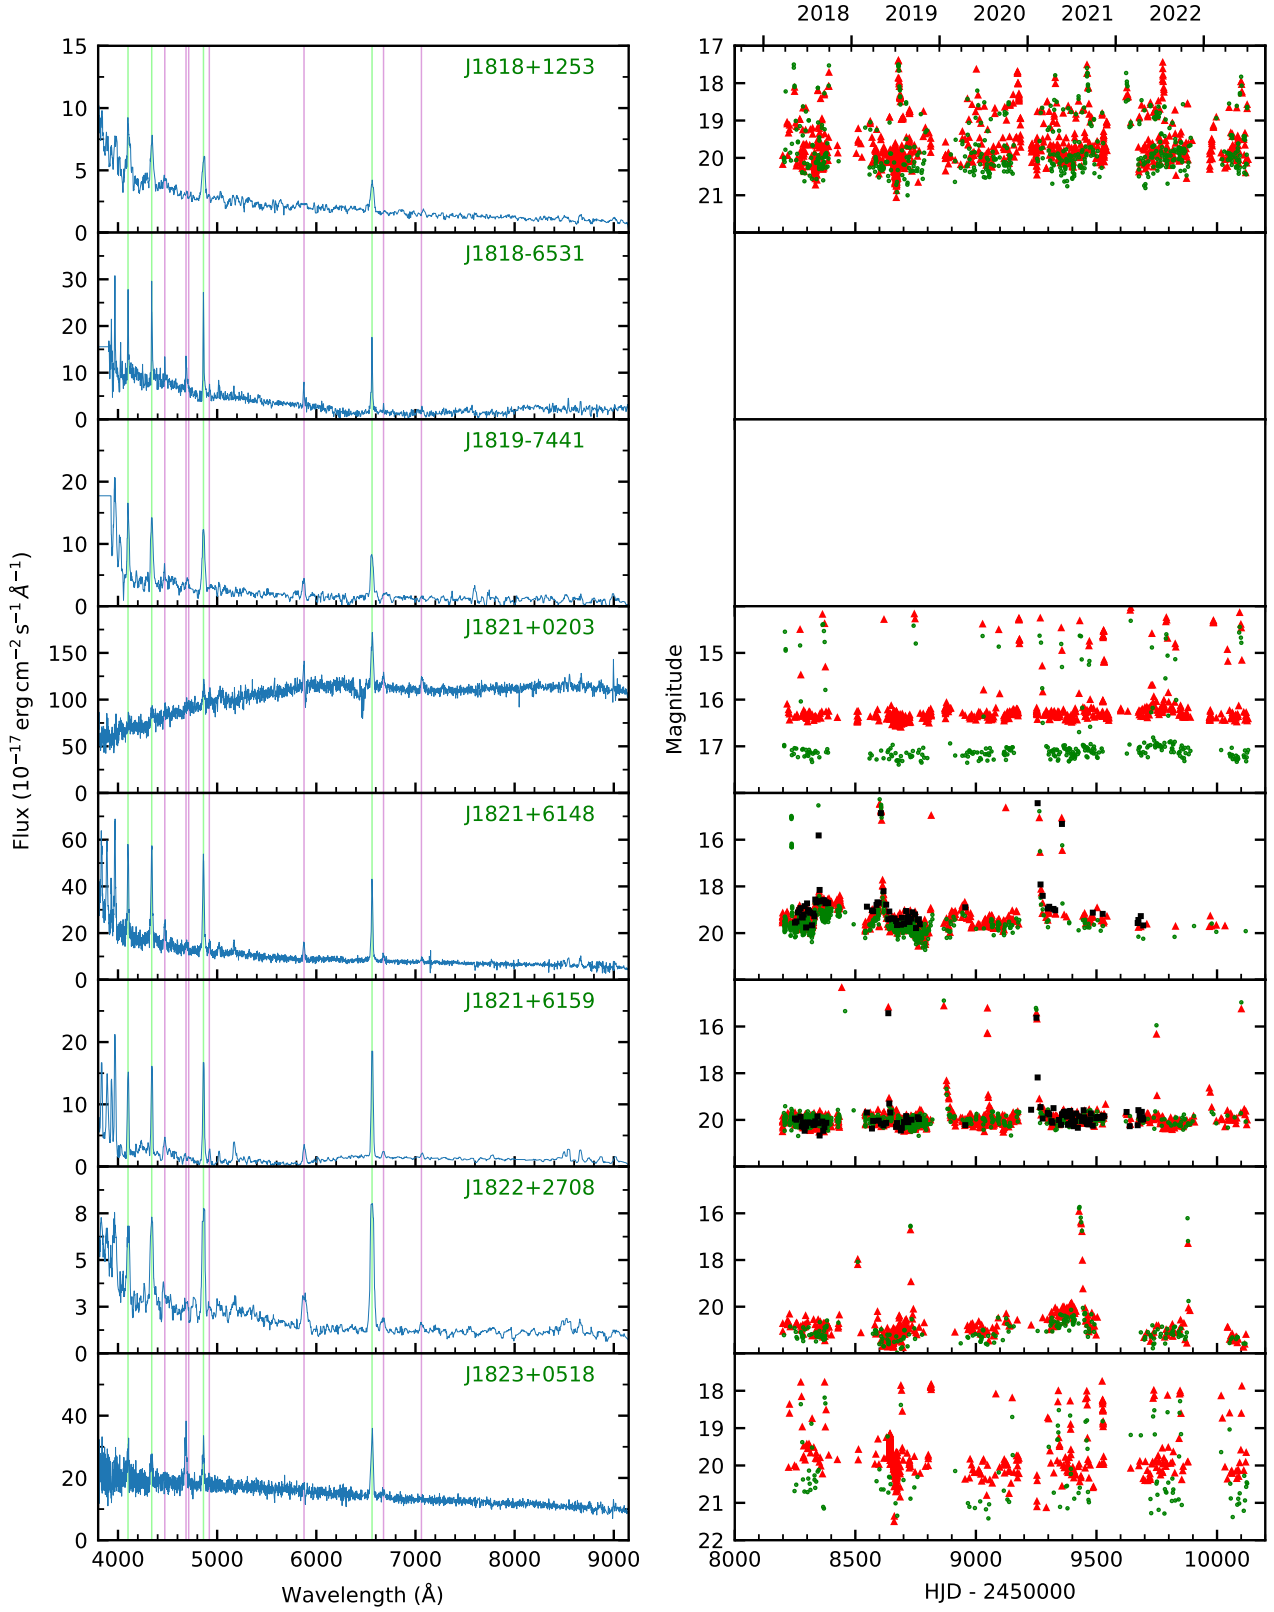

Figure 42: Left panels: Spectra with H lines shown in green and He in pink. Right panels: Light curves with ZTF  $r$ -band shown in red triangles,  $g$ -band in green dots and  $i$ -band in black squares.

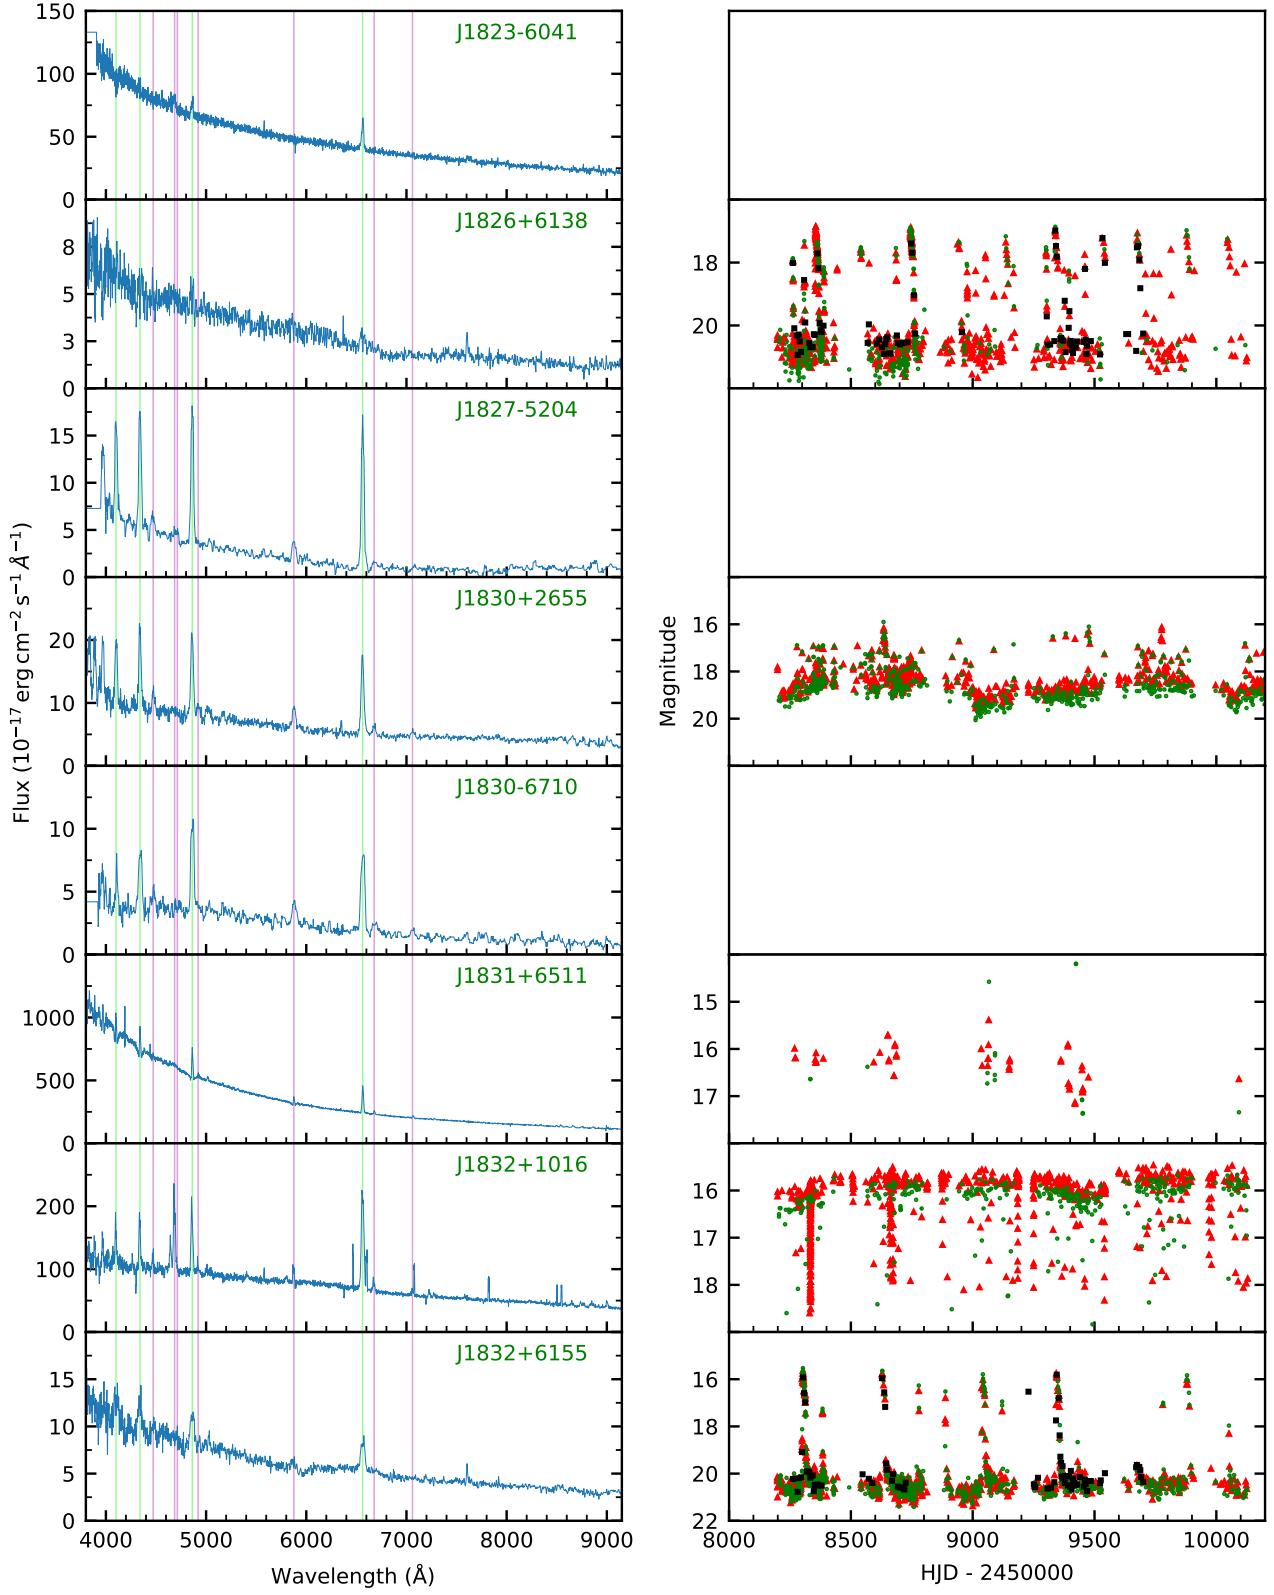

Figure 43: Left panels: Spectra with H lines shown in green and He in pink. Right panels: Light curves with ZTF *r*-band shown in red triangles, *g*-band in green dots and *i*-band in black squares.

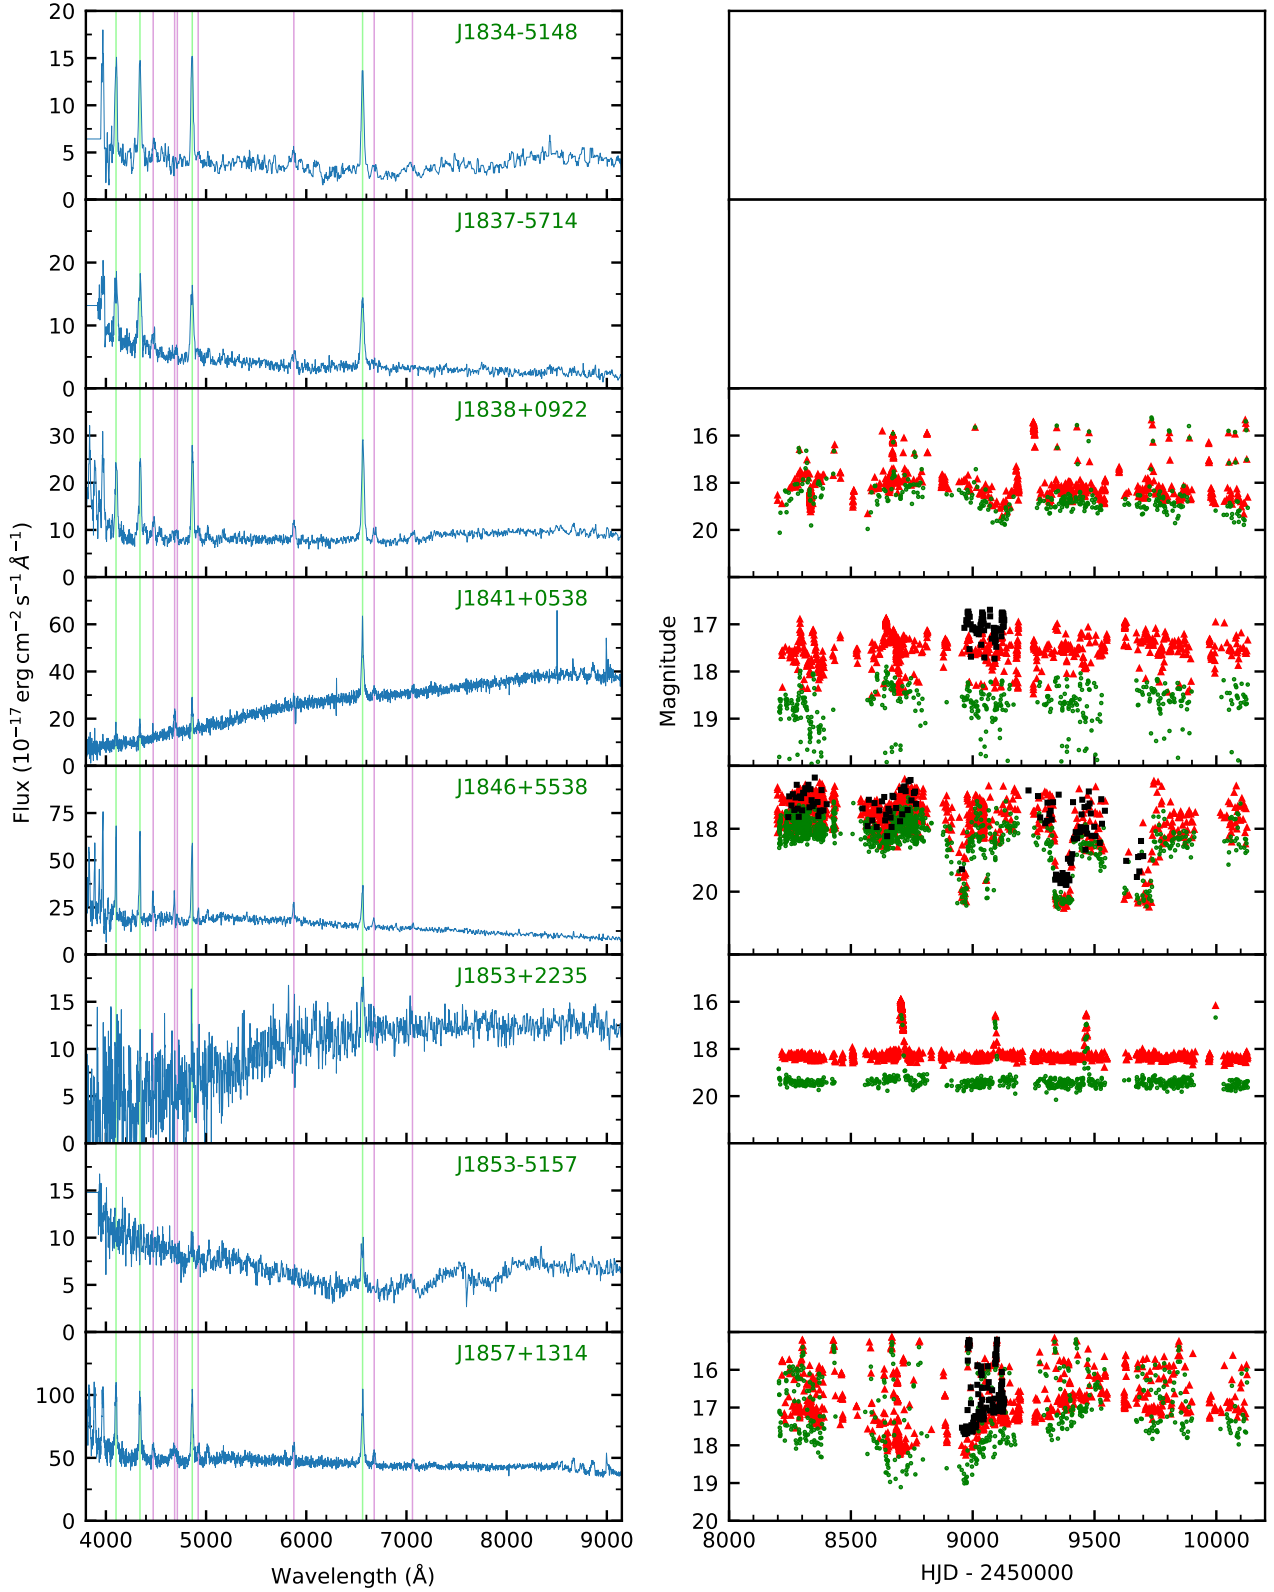

Figure 44: Left panels: Spectra with H lines shown in green and He in pink. Right panels: Light curves with ZTF  $r$ -band shown in red triangles,  $g$ -band in green dots and  $i$ -band in black squares.

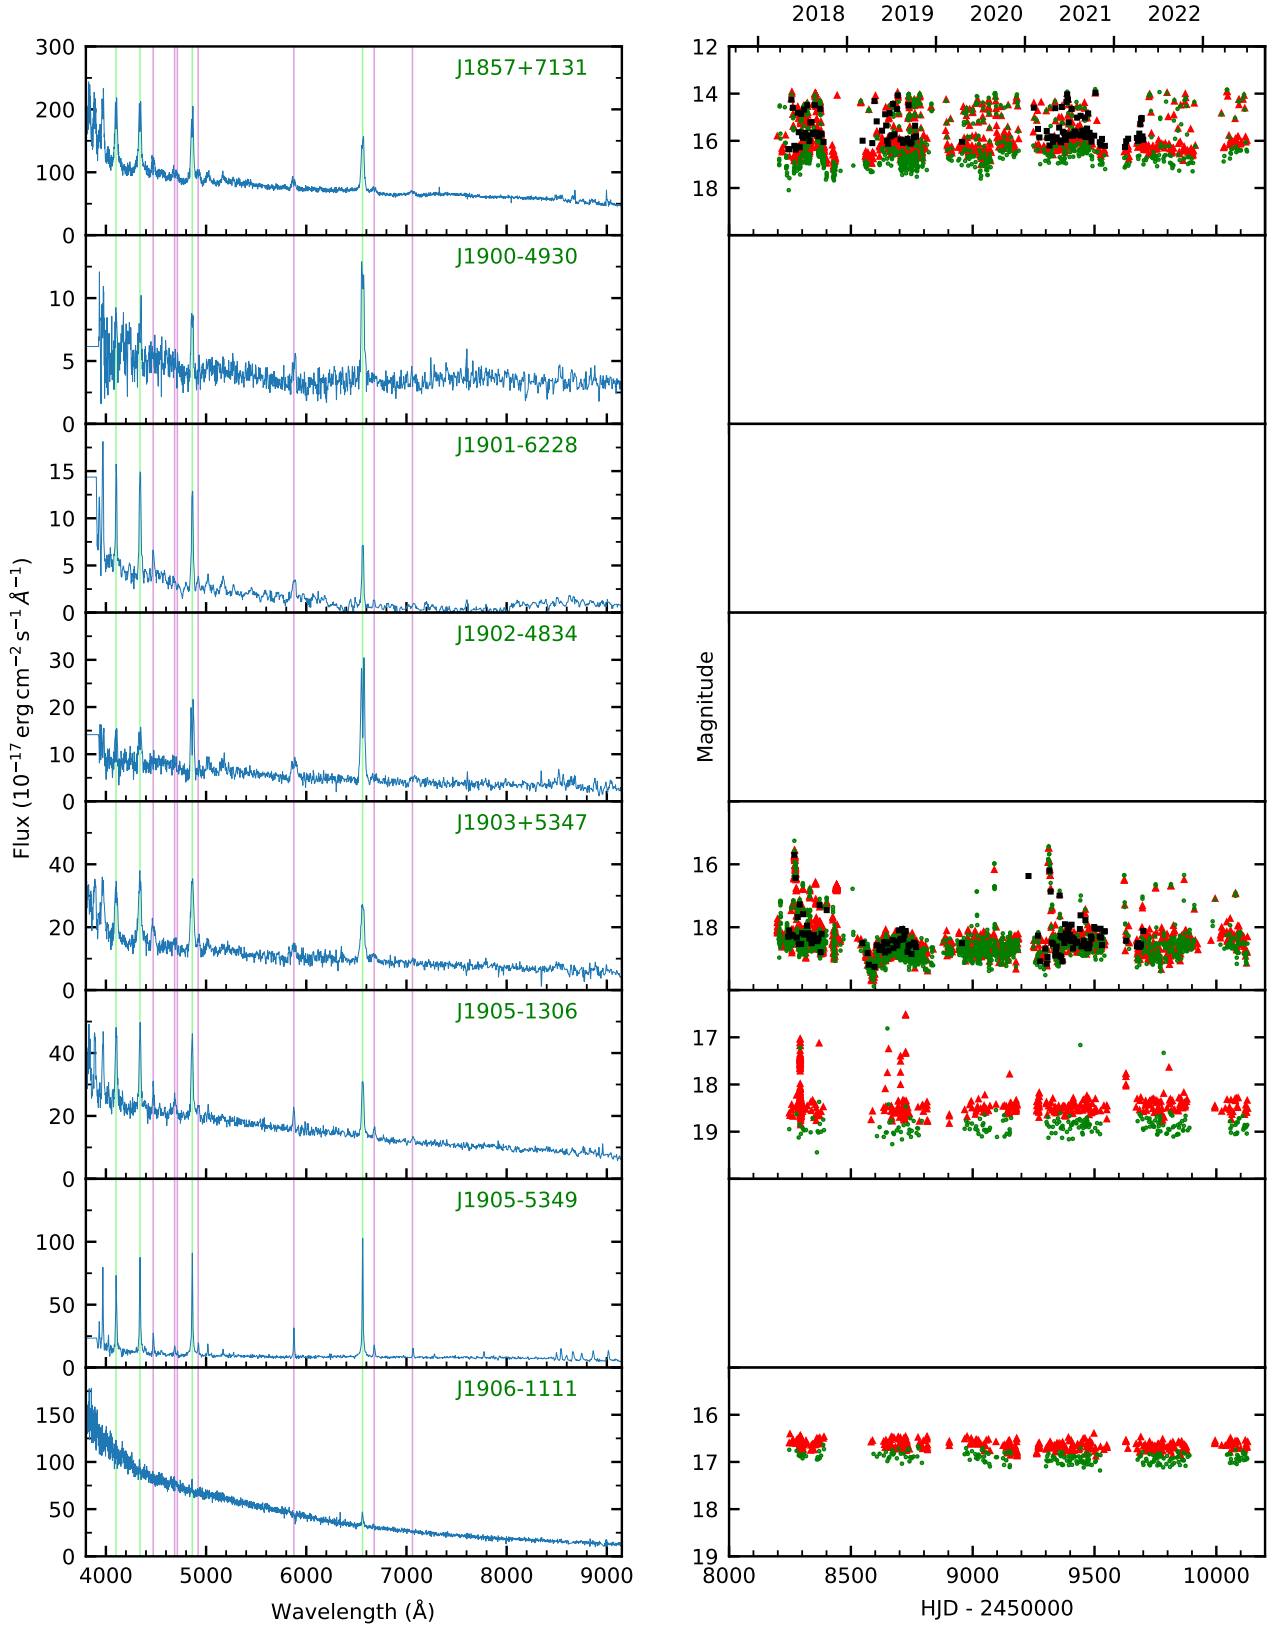

Figure 45: Left panels: Spectra with H lines shown in green and He in pink. Right panels: Light curves with ZTF  $r$ -band shown in red triangles,  $g$ -band in green dots and  $i$ -band in black squares.

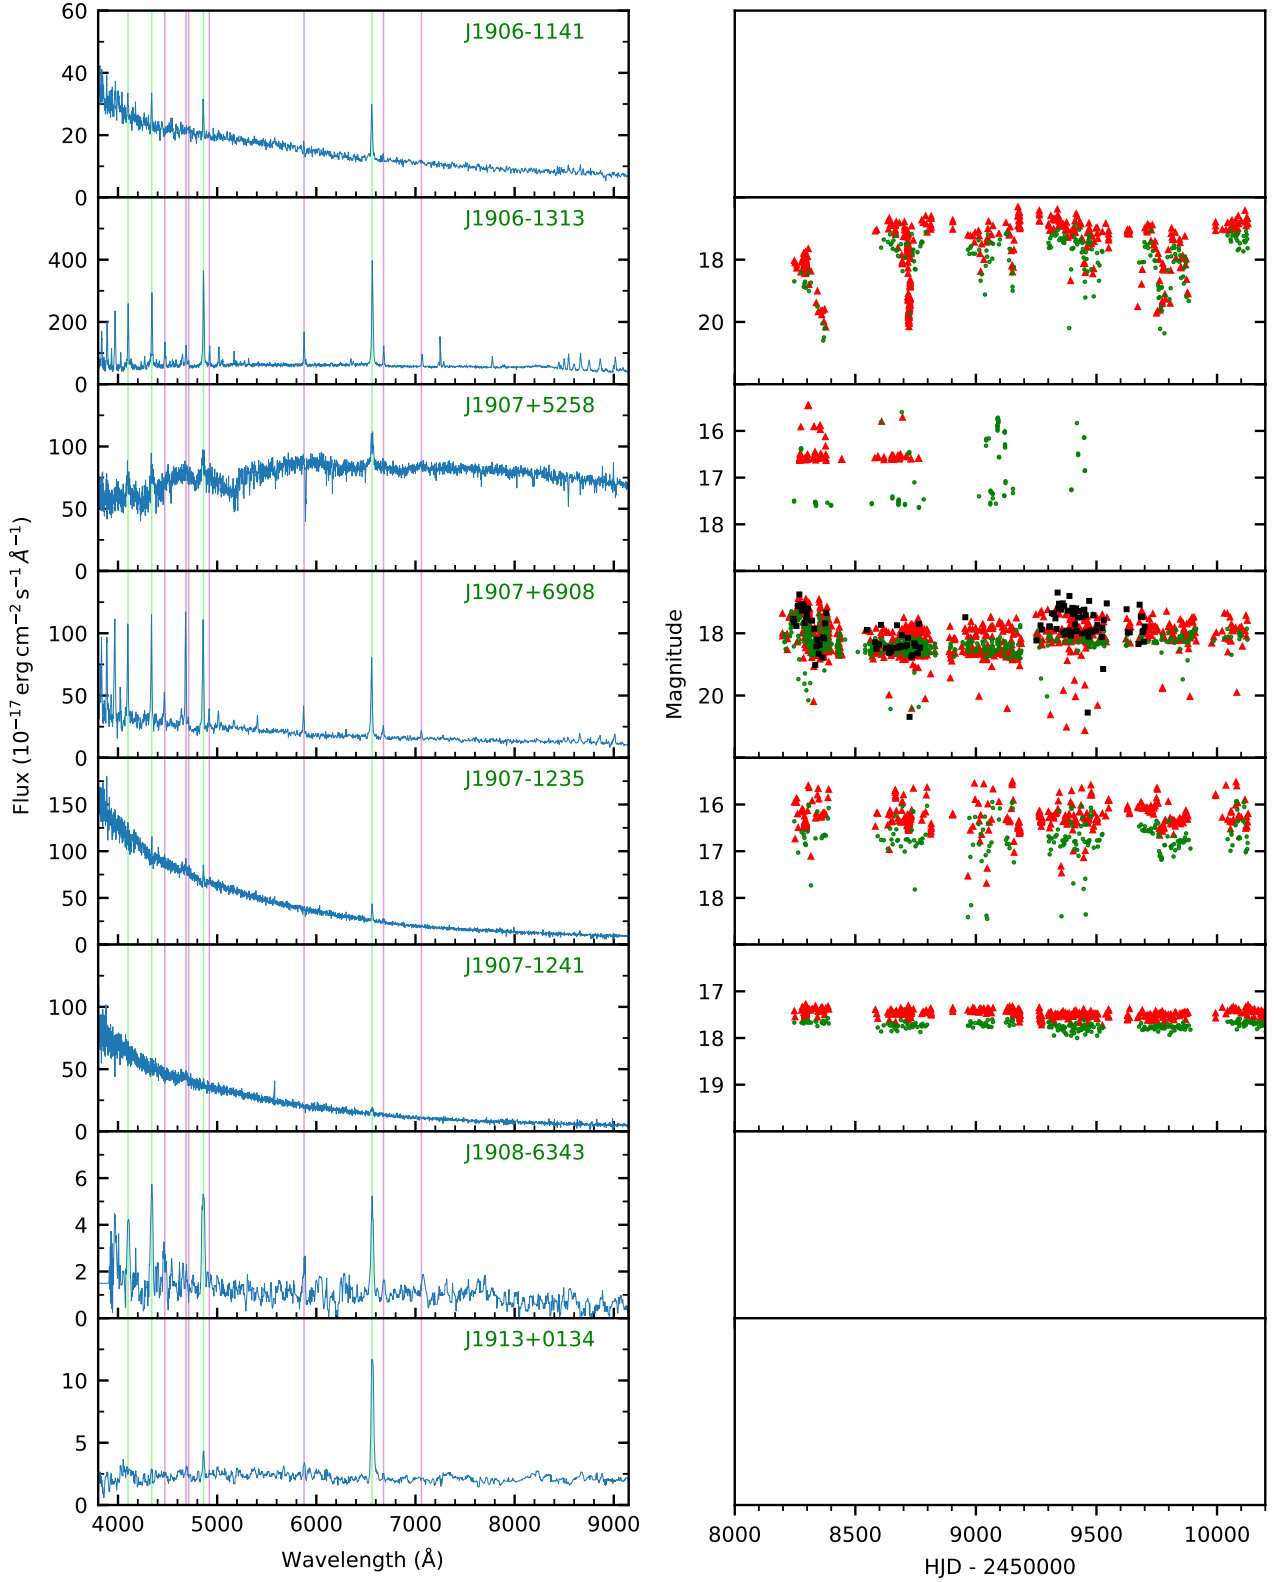

Figure 46: Left panels: Spectra with H lines shown in green and He in pink. Right panels: Light curves with ZTF  $r$ -band shown in red triangles,  $g$ -band in green dots and  $i$ -band in black squares.



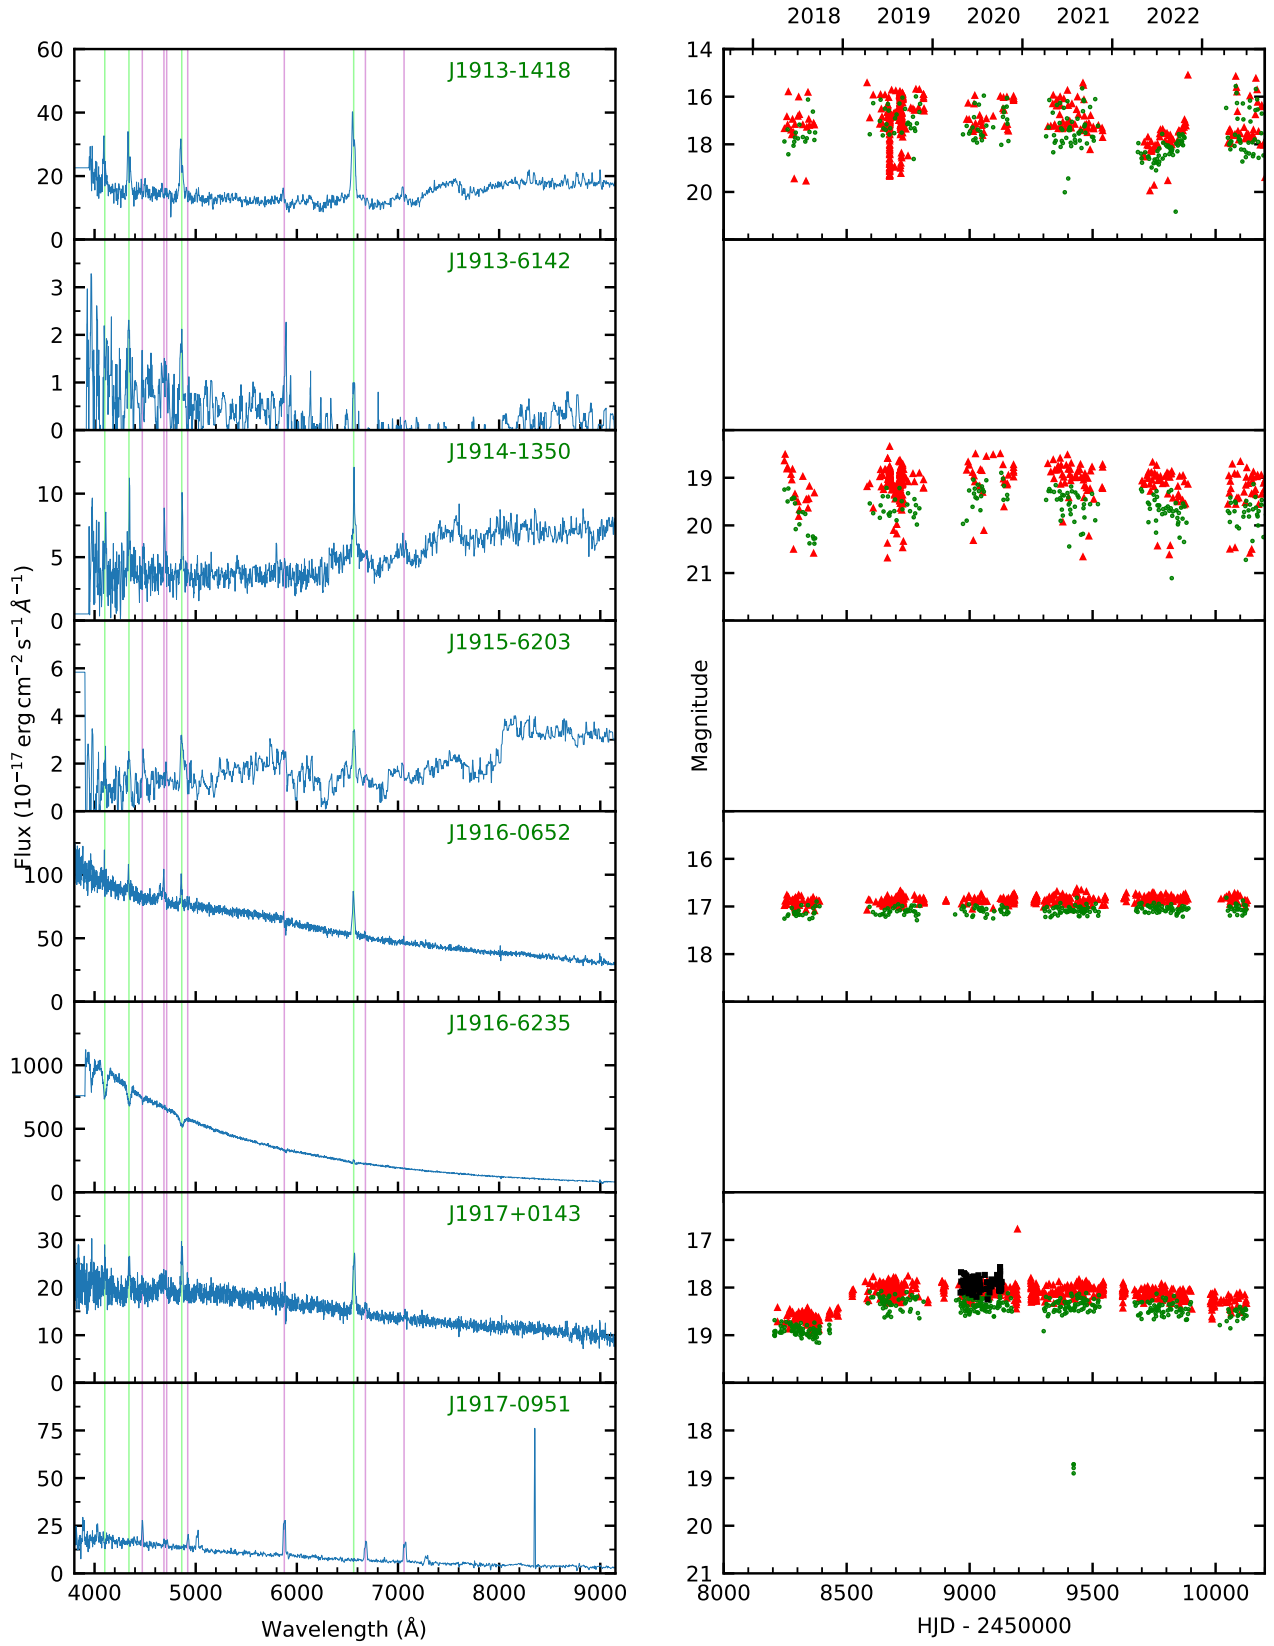

Figure 47: Left panels: Spectra with H lines shown in green and He in pink. Right panels: Light curves with ZTF *r*-band shown in red triangles, *g*-band in green dots and *i*-band in black squares.

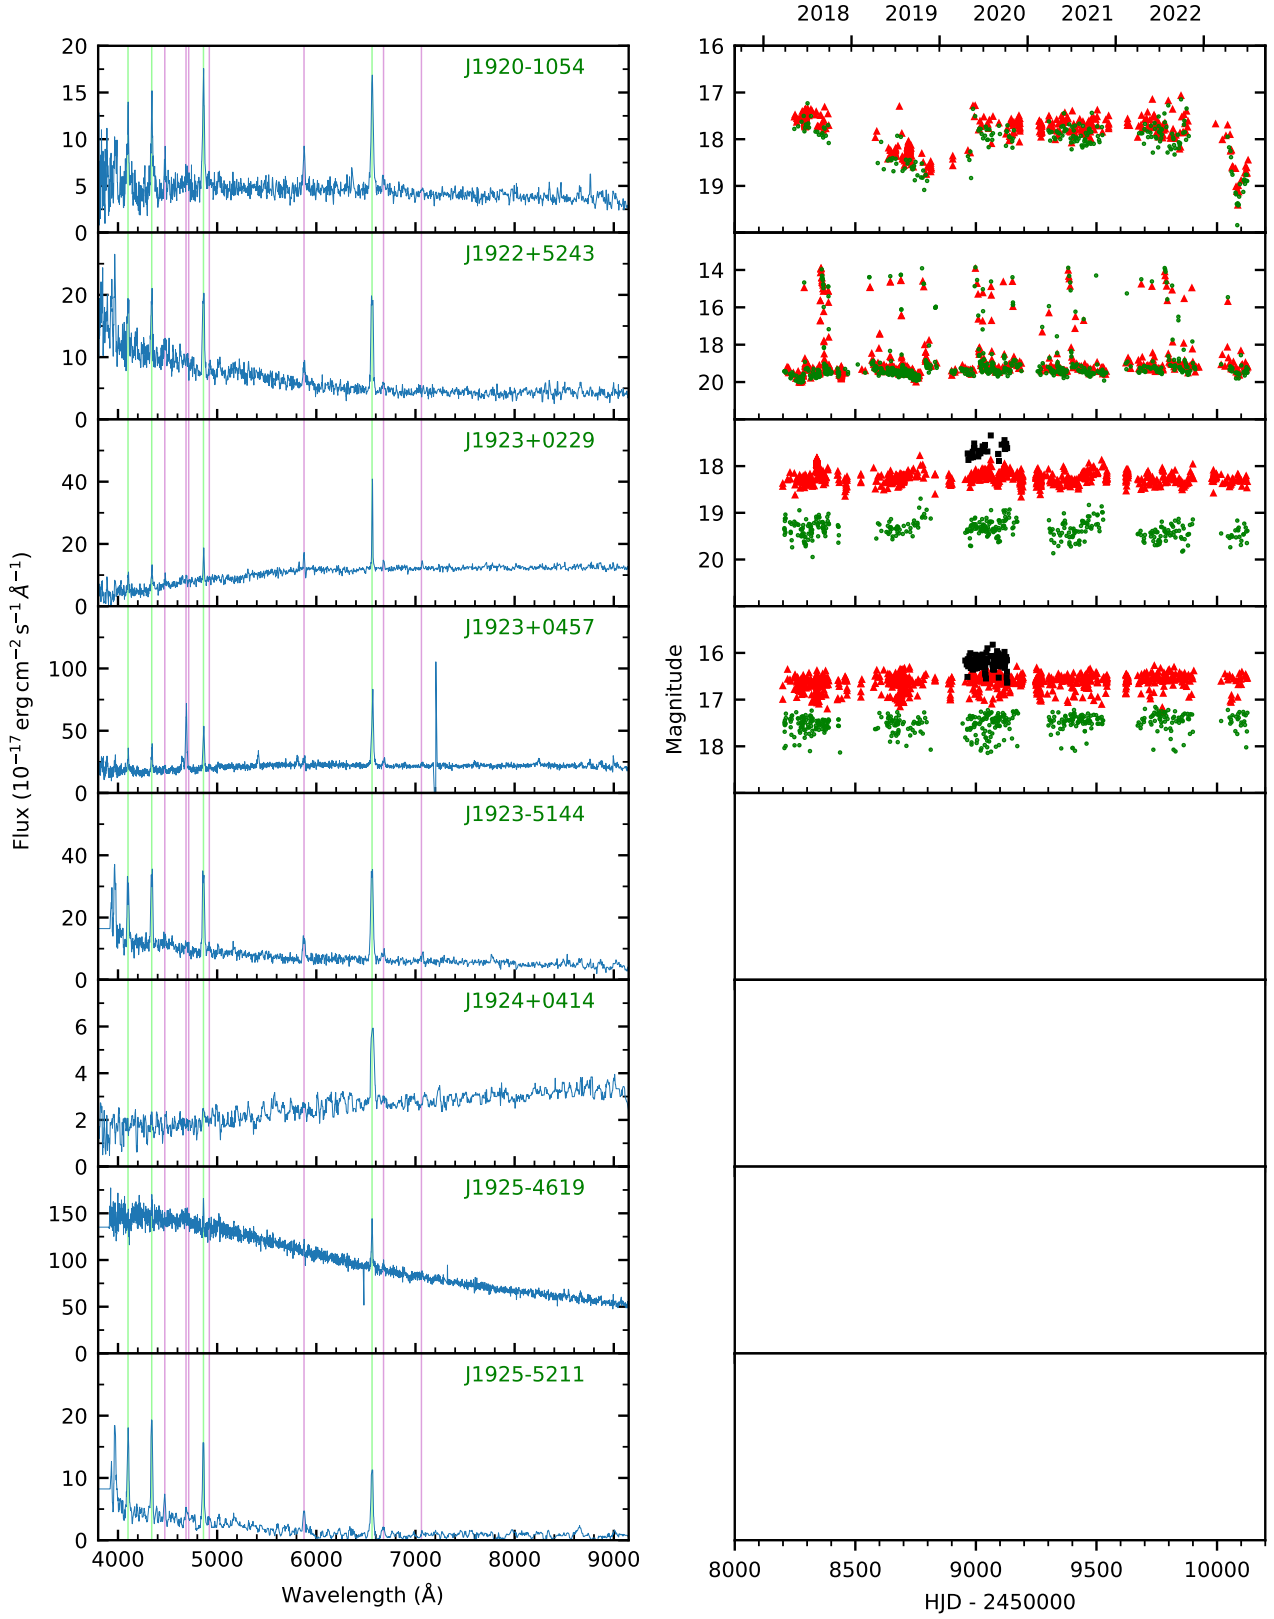

Figure 48: Left panels: Spectra with H lines shown in green and He in pink. Right panels: Light curves with ZTF  $r$ -band shown in red triangles,  $g$ -band in green dots and  $i$ -band in black squares.

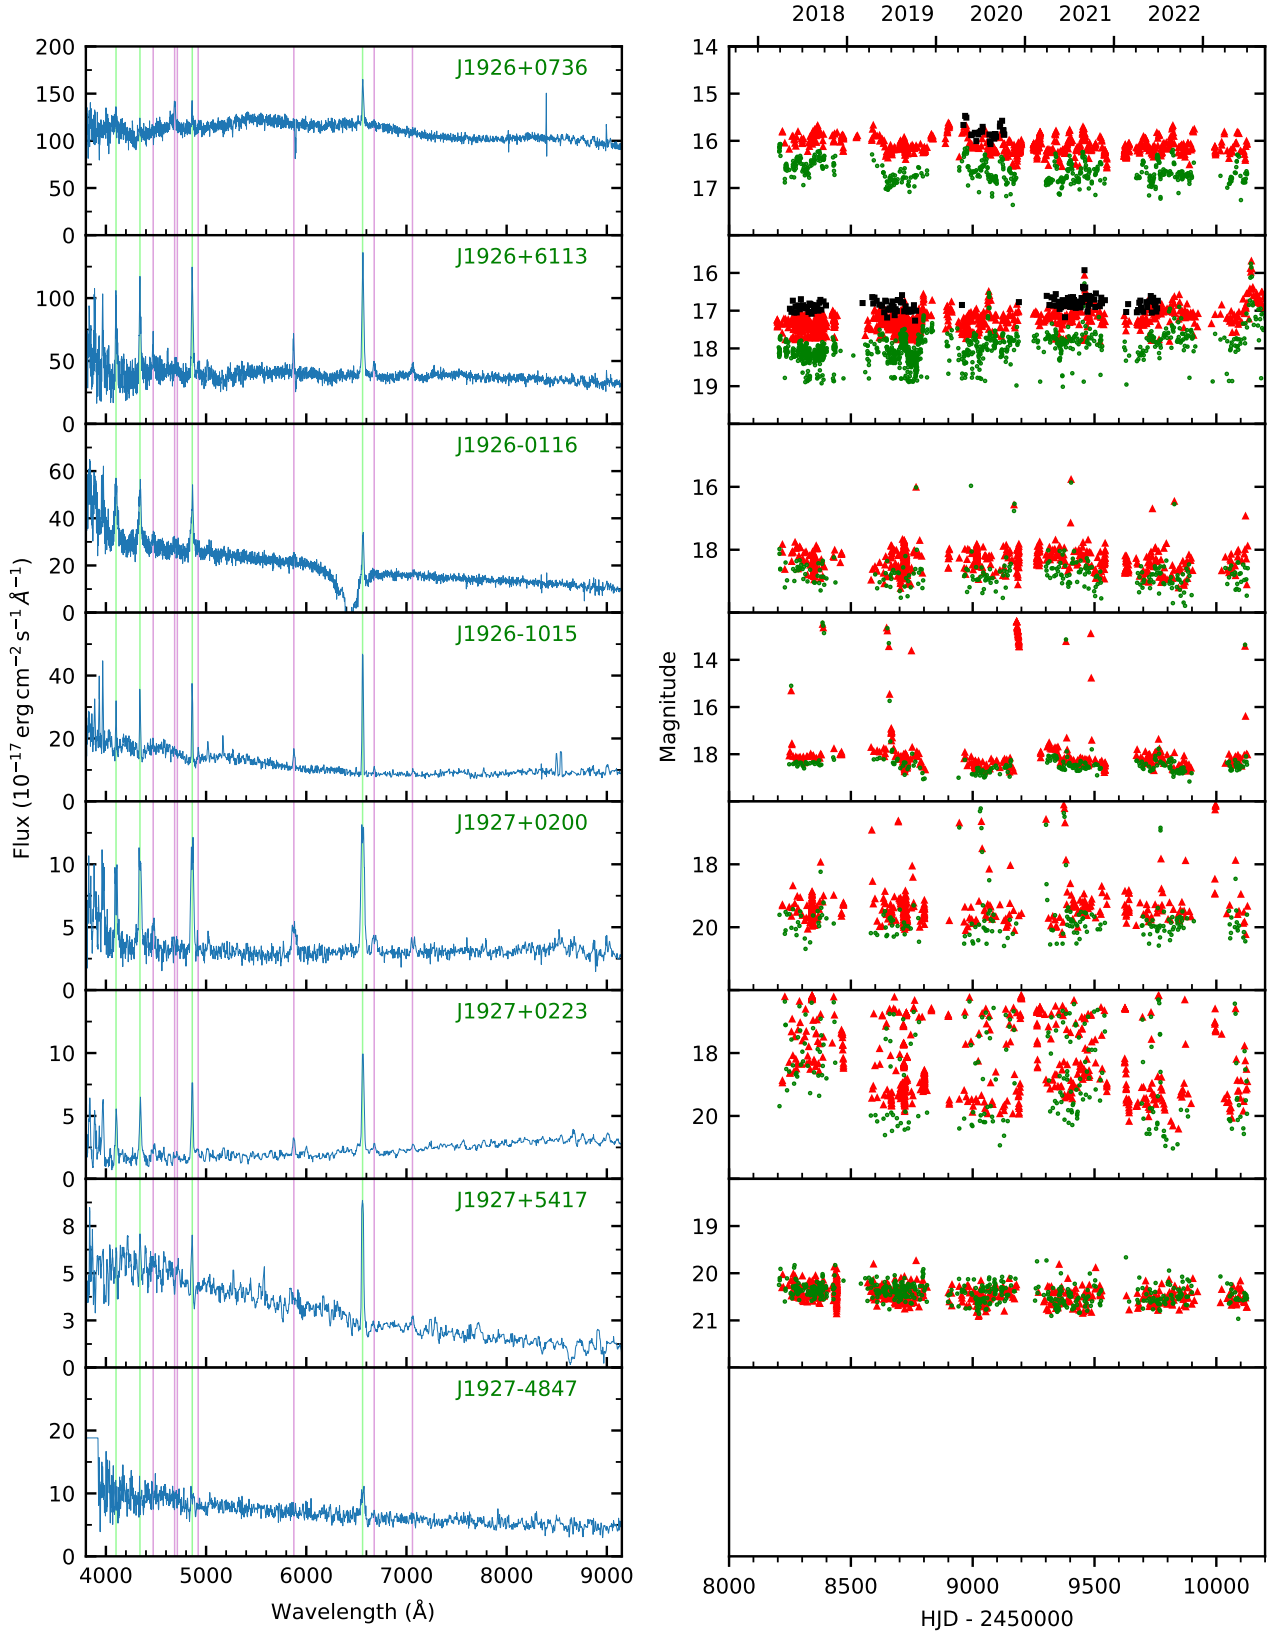

Figure 49: Left panels: Spectra with H lines shown in green and He in pink. Right panels: Light curves with ZTF *r*-band shown in red triangles, *g*-band in green dots and *i*-band in black squares.

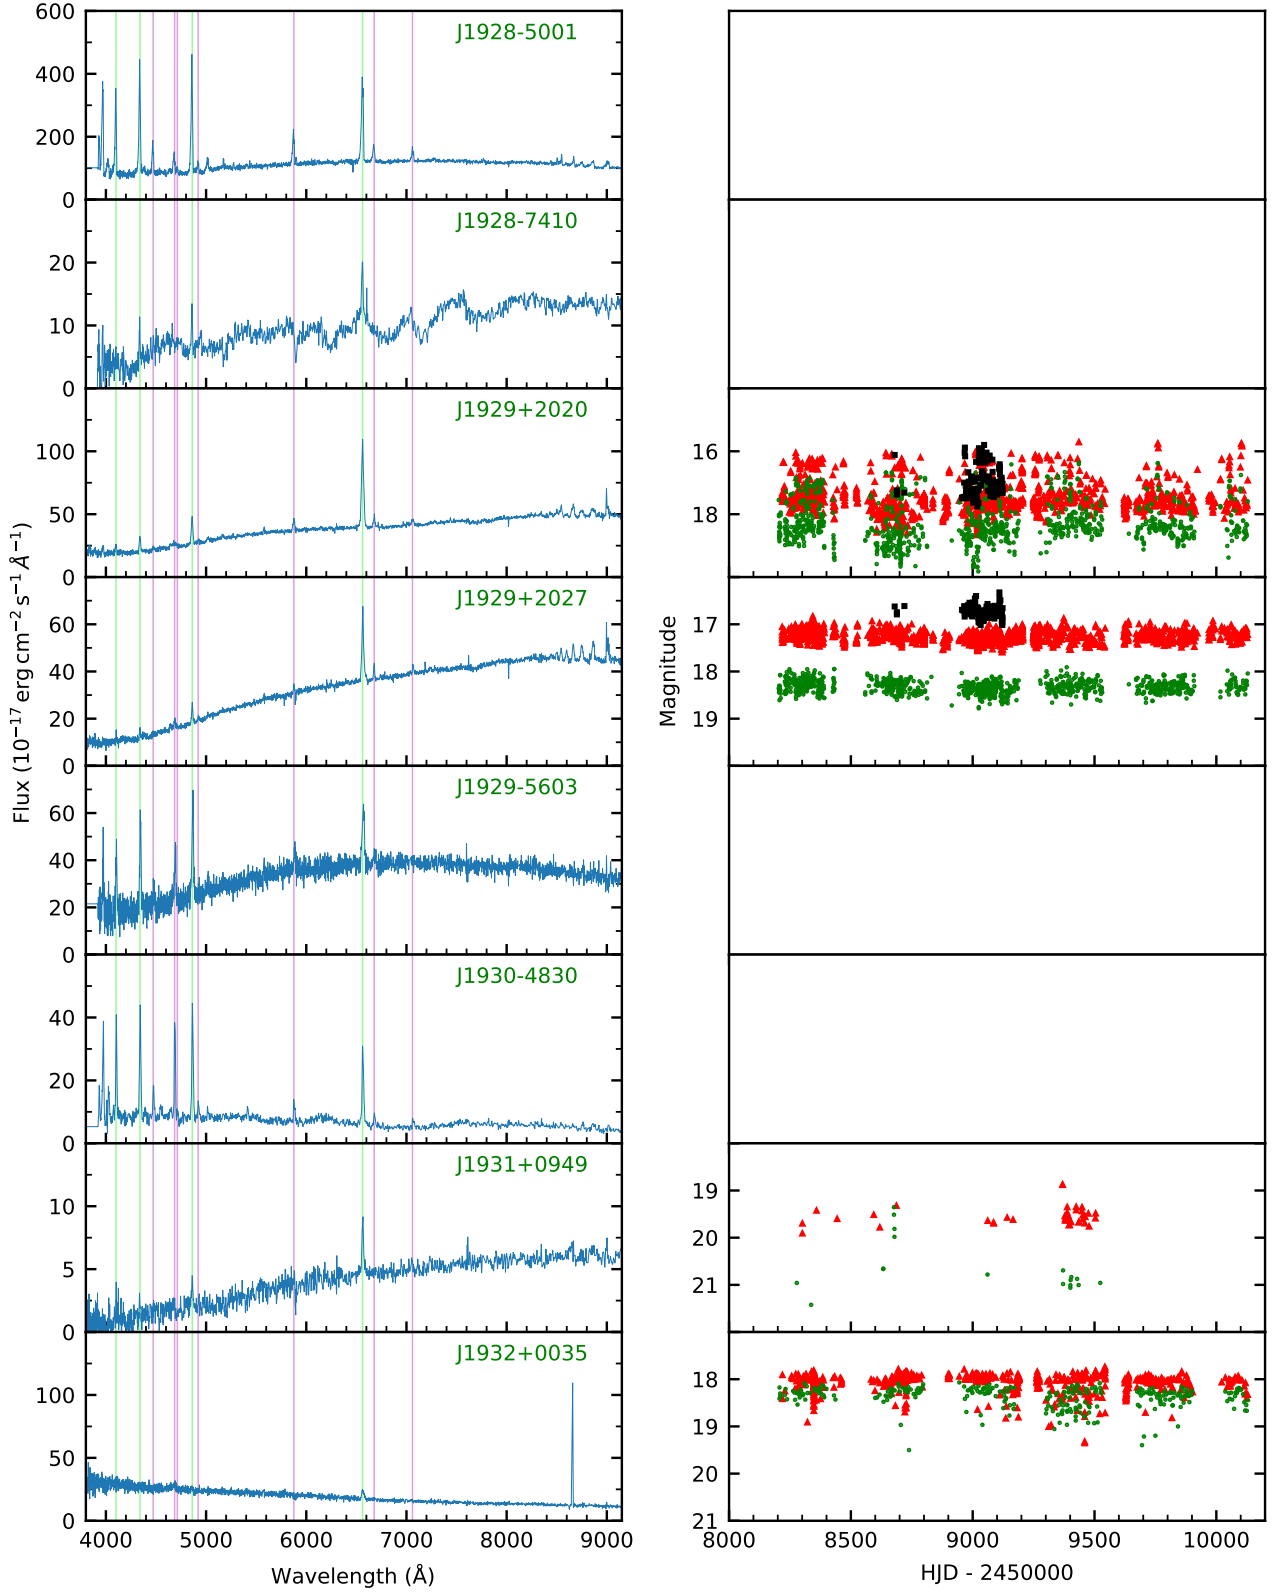

Figure 50: Left panels: Spectra with H lines shown in green and He in pink. Right panels: Light curves with ZTF  $r$ -band shown in red triangles,  $g$ -band in green dots and  $i$ -band in black squares.

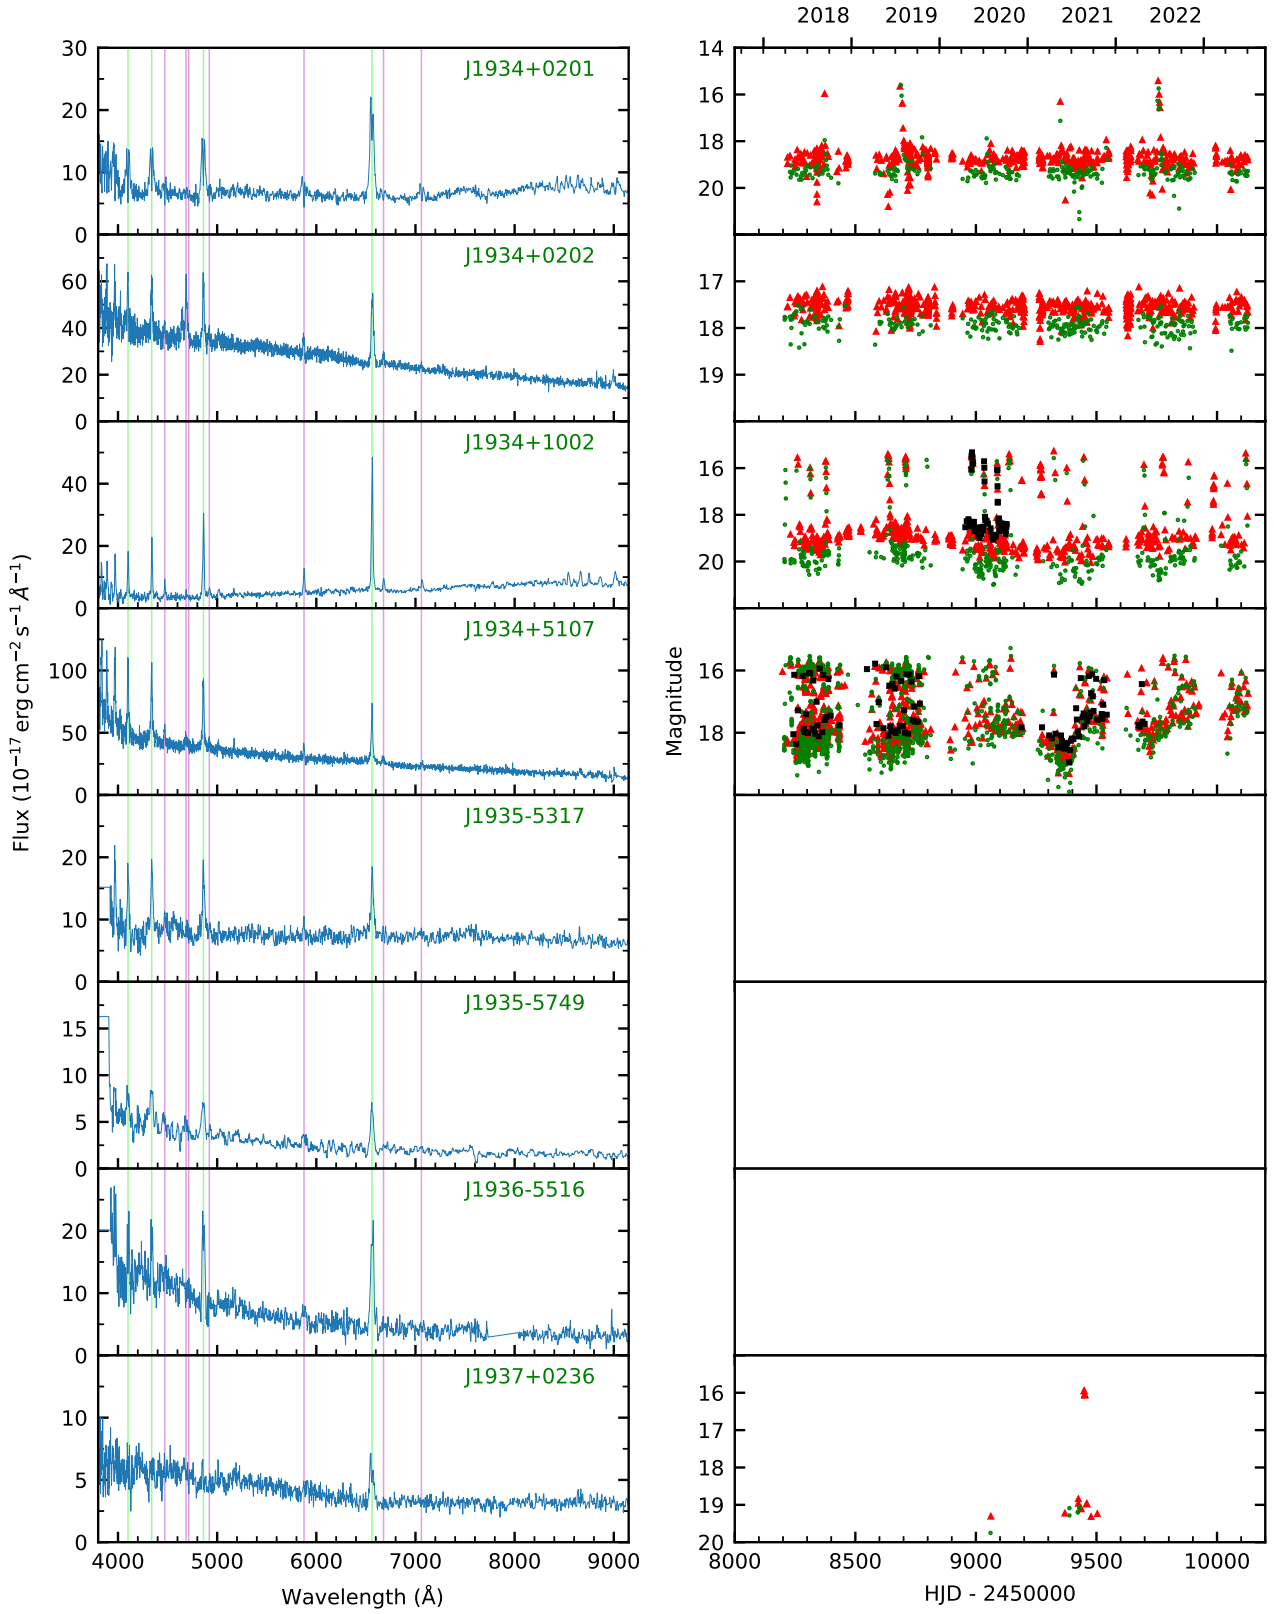

Figure 51: Left panels: Spectra with H lines shown in green and He in pink. Right panels: Light curves with ZTF *r*-band shown in red triangles, *g*-band in green dots and *i*-band in black squares.

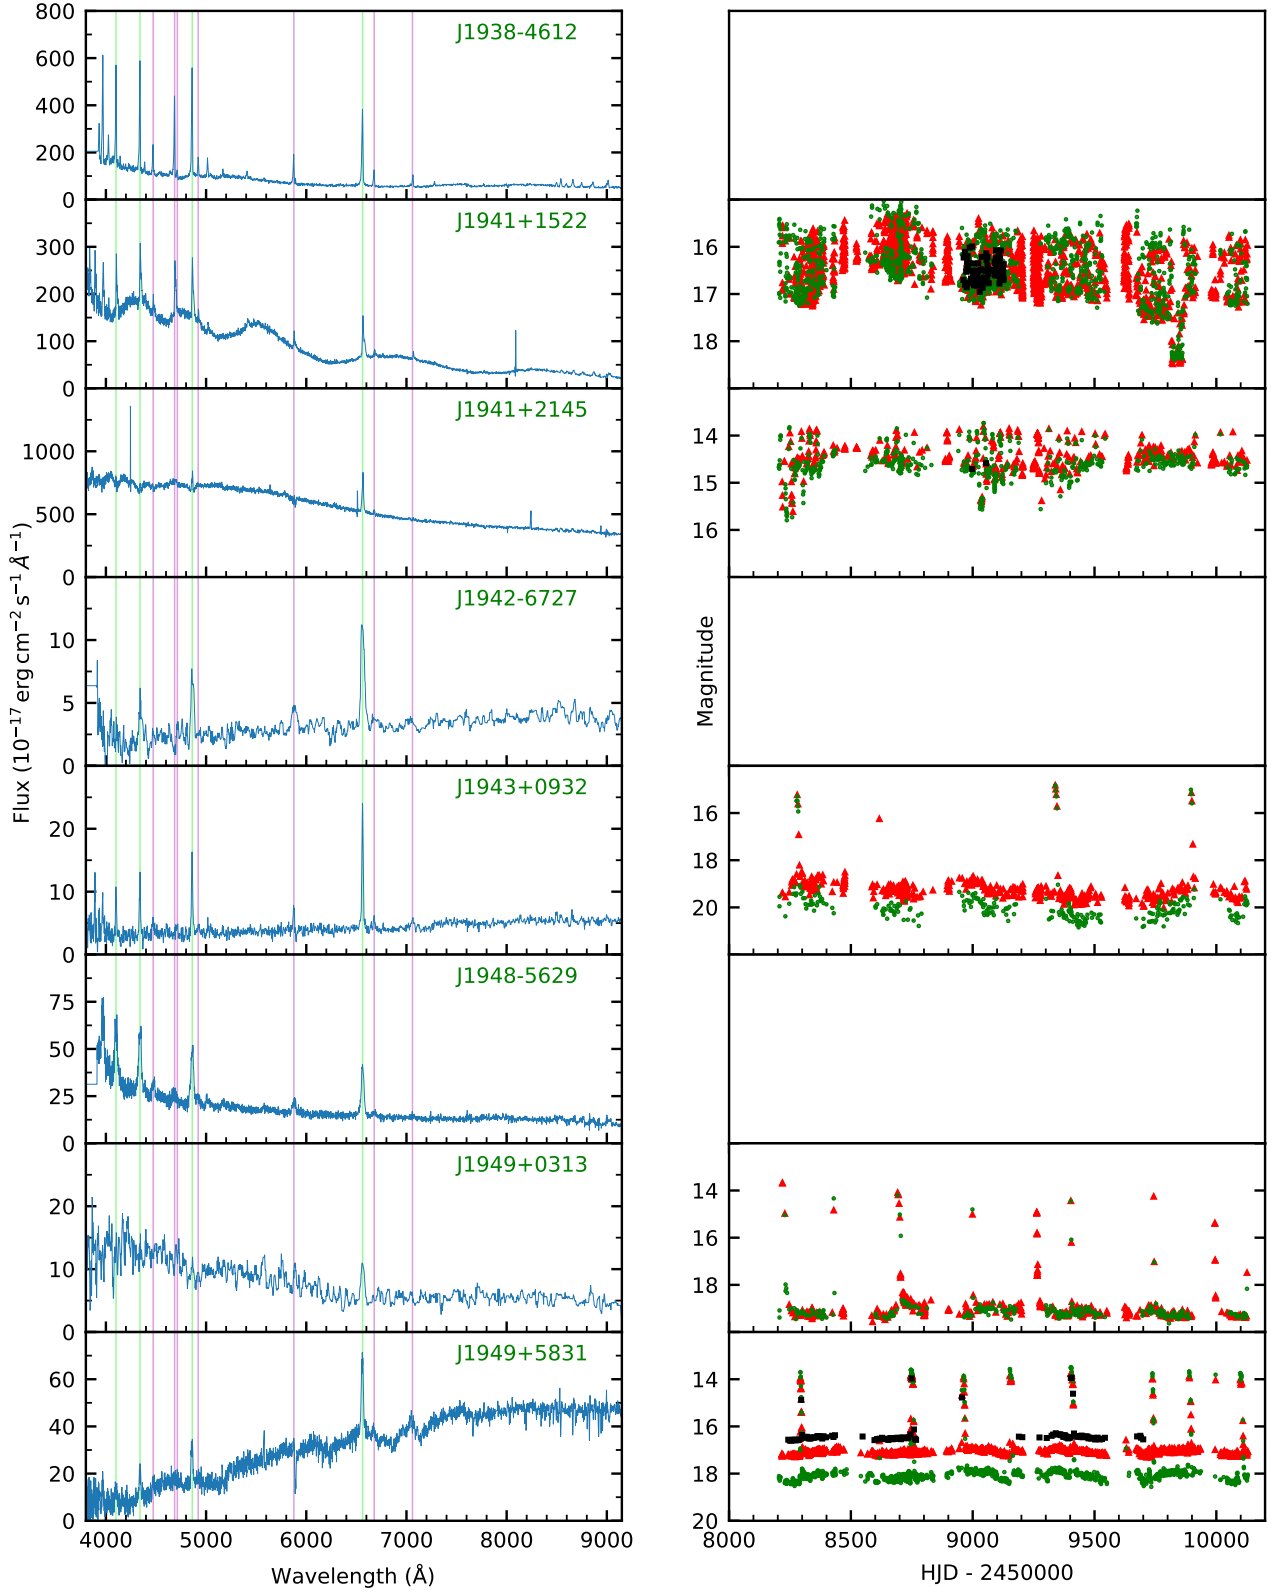

Figure 52: Left panels: Spectra with H lines shown in green and He in pink. Right panels: Light curves with ZTF  $r$ -band shown in red triangles,  $g$ -band in green dots and  $i$ -band in black squares.

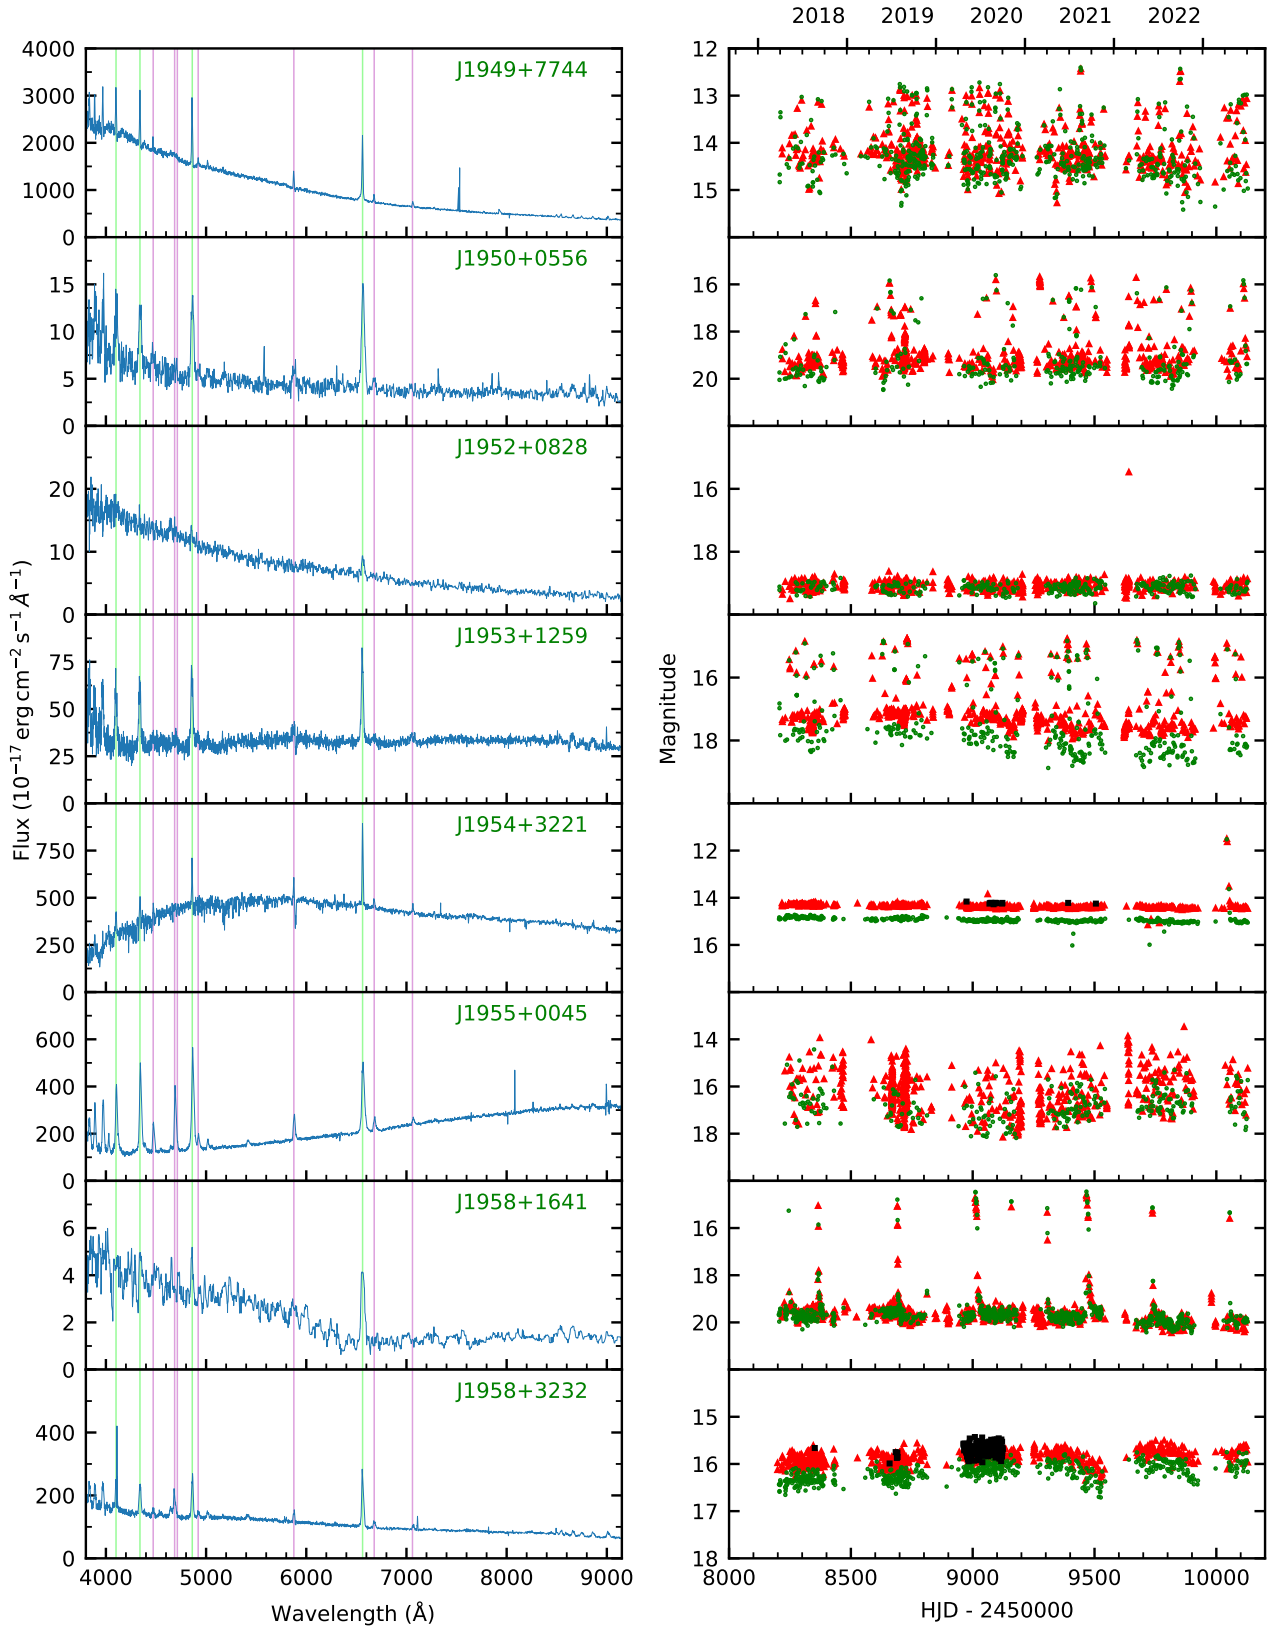

Figure 53: Left panels: Spectra with H lines shown in green and He in pink. Right panels: Light curves with ZTF *r*-band shown in red triangles, *g*-band in green dots and *i*-band in black squares.



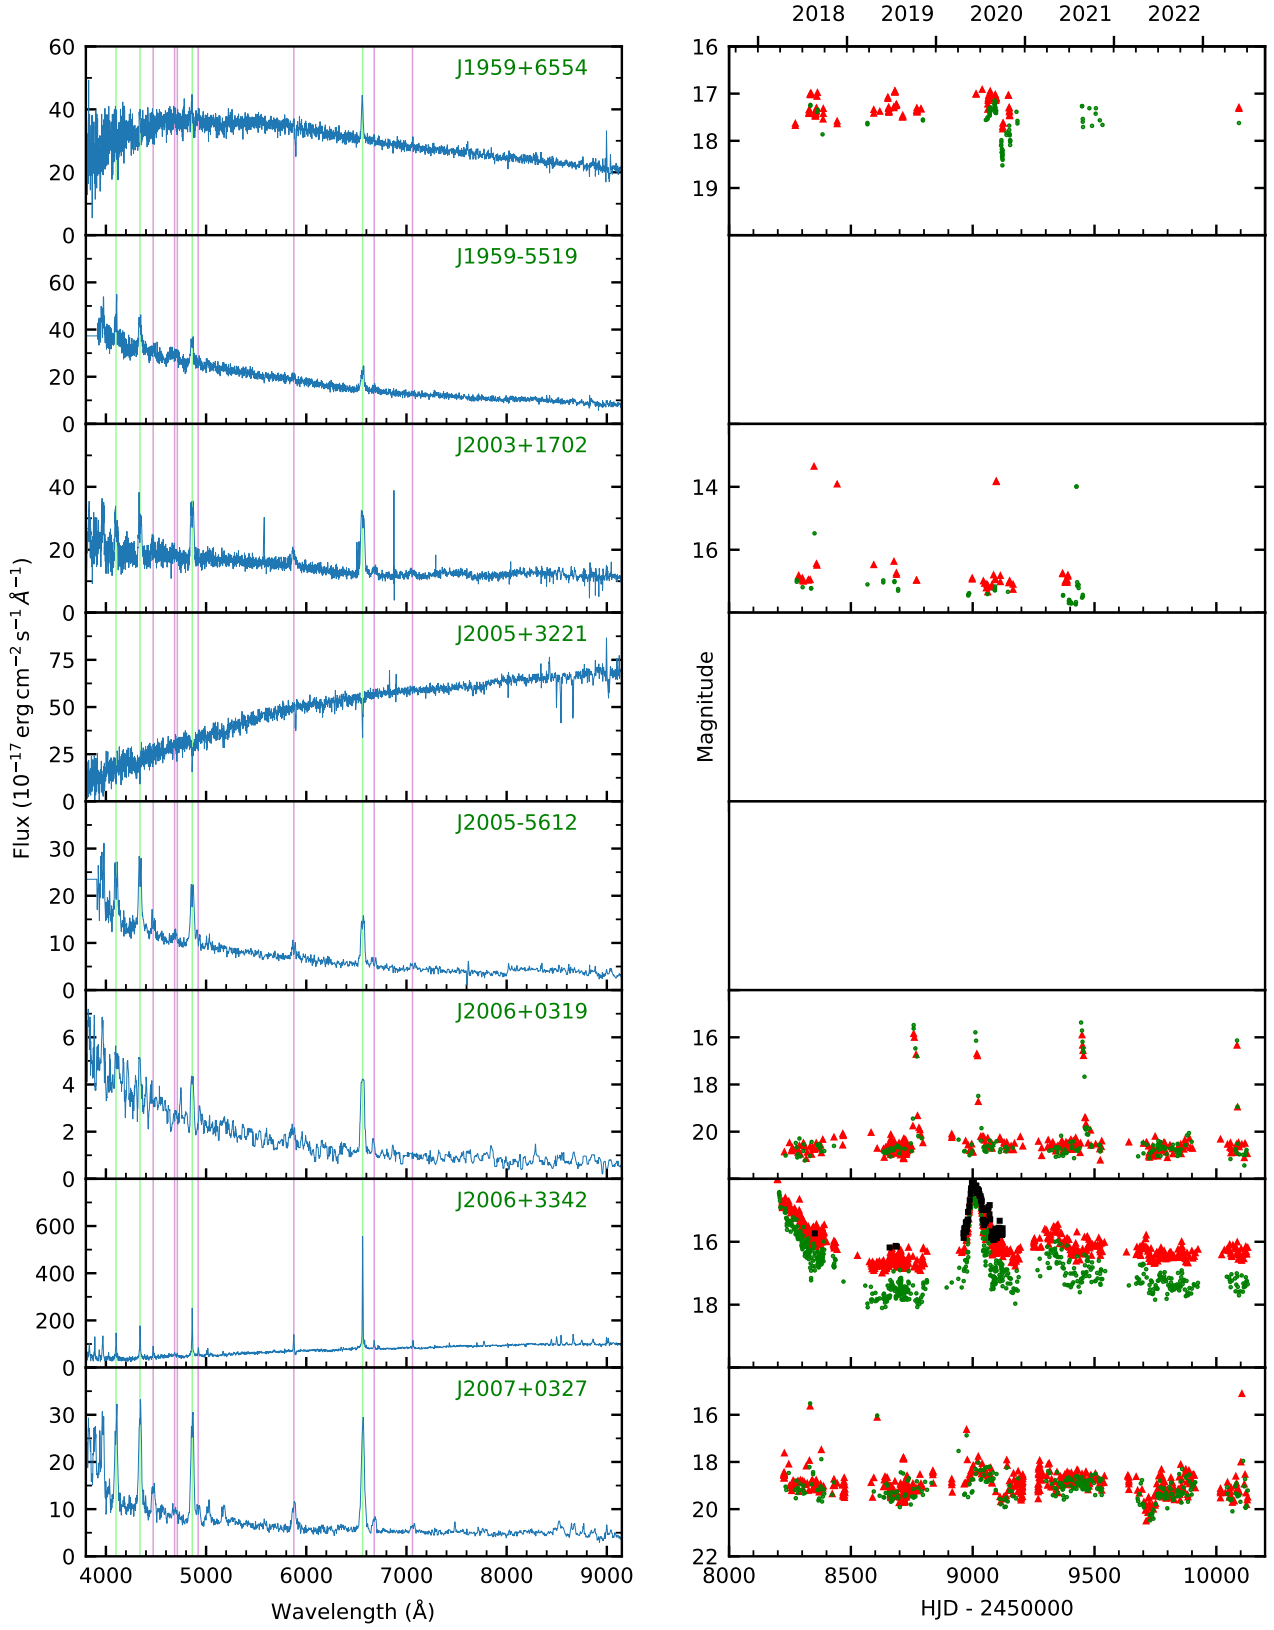

Figure 54: Left panels: Spectra with H lines shown in green and He in pink. Right panels: Light curves with ZTF  $r$ -band shown in red triangles,  $g$ -band in green dots and  $i$ -band in black squares.

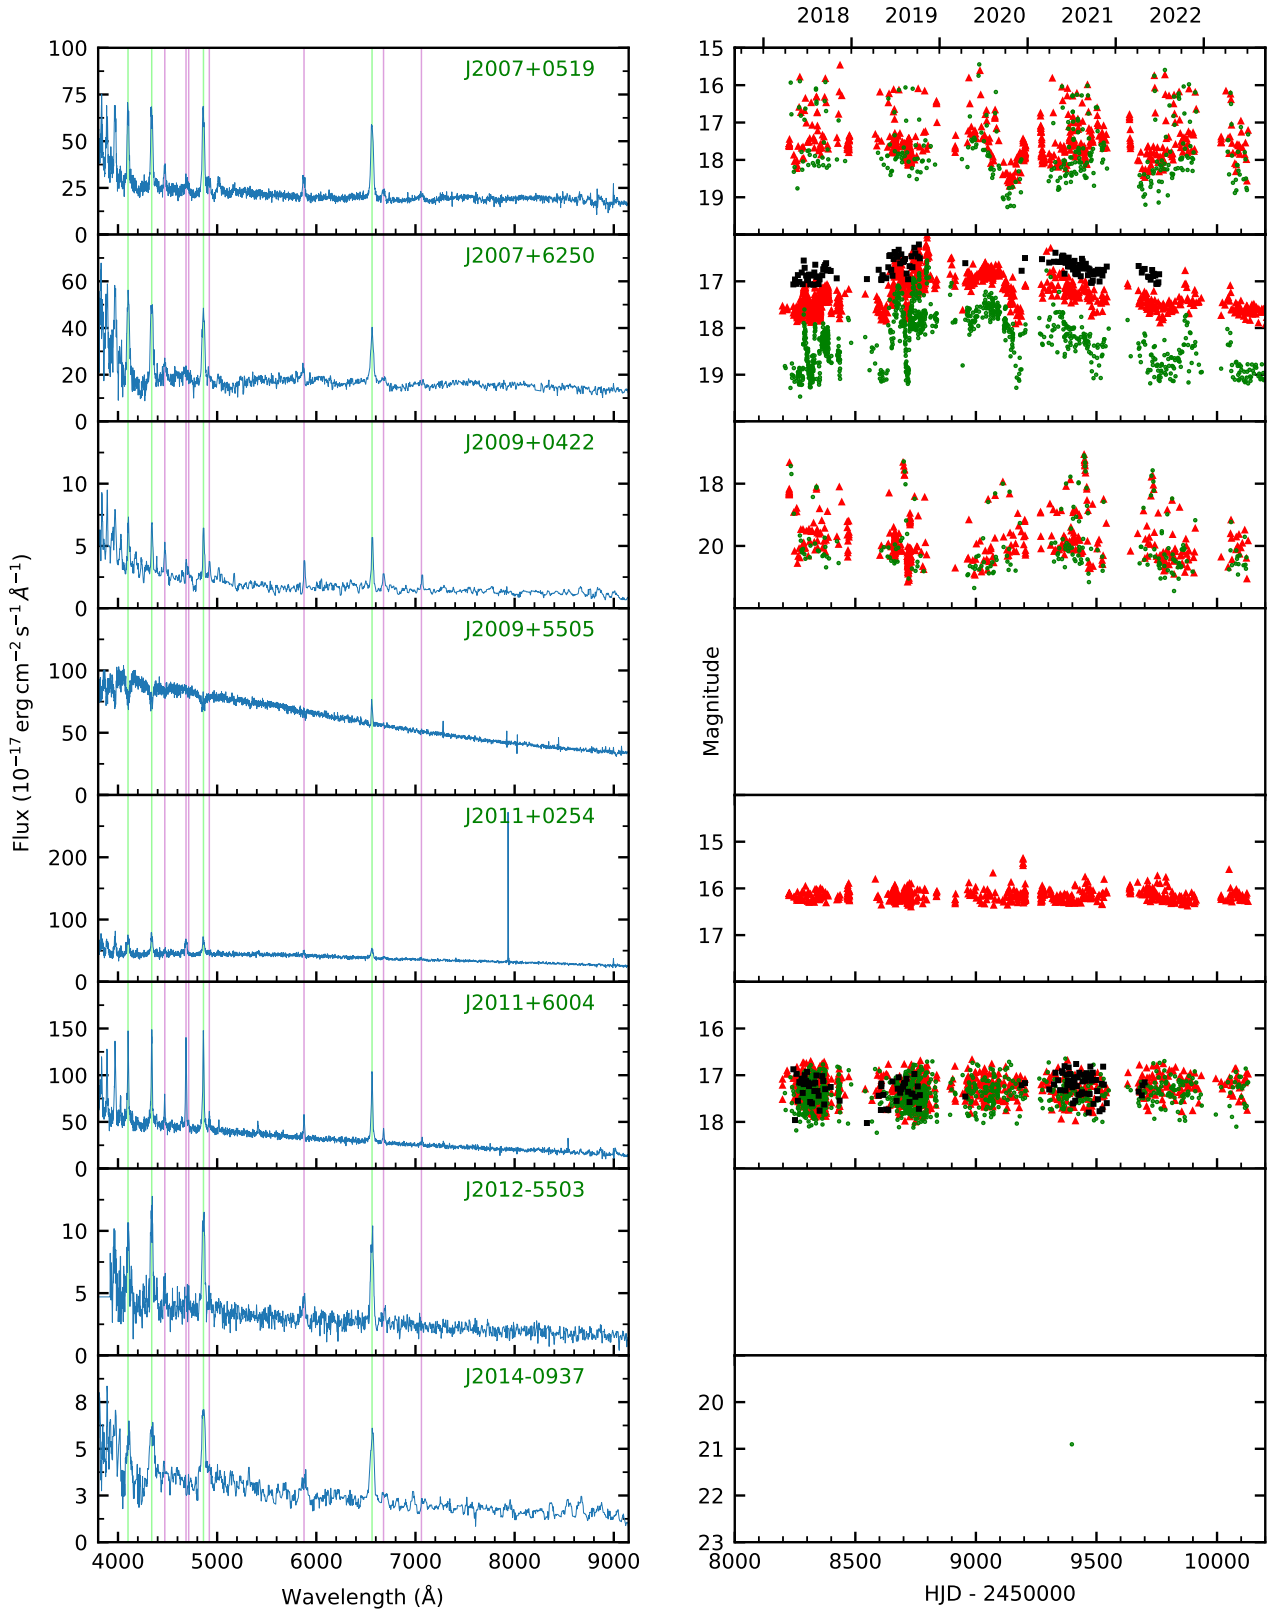

Figure 55: Left panels: Spectra with H lines shown in green and He in pink. Right panels: Light curves with ZTF  $r$ -band shown in red triangles,  $g$ -band in green dots and  $i$ -band in black squares.

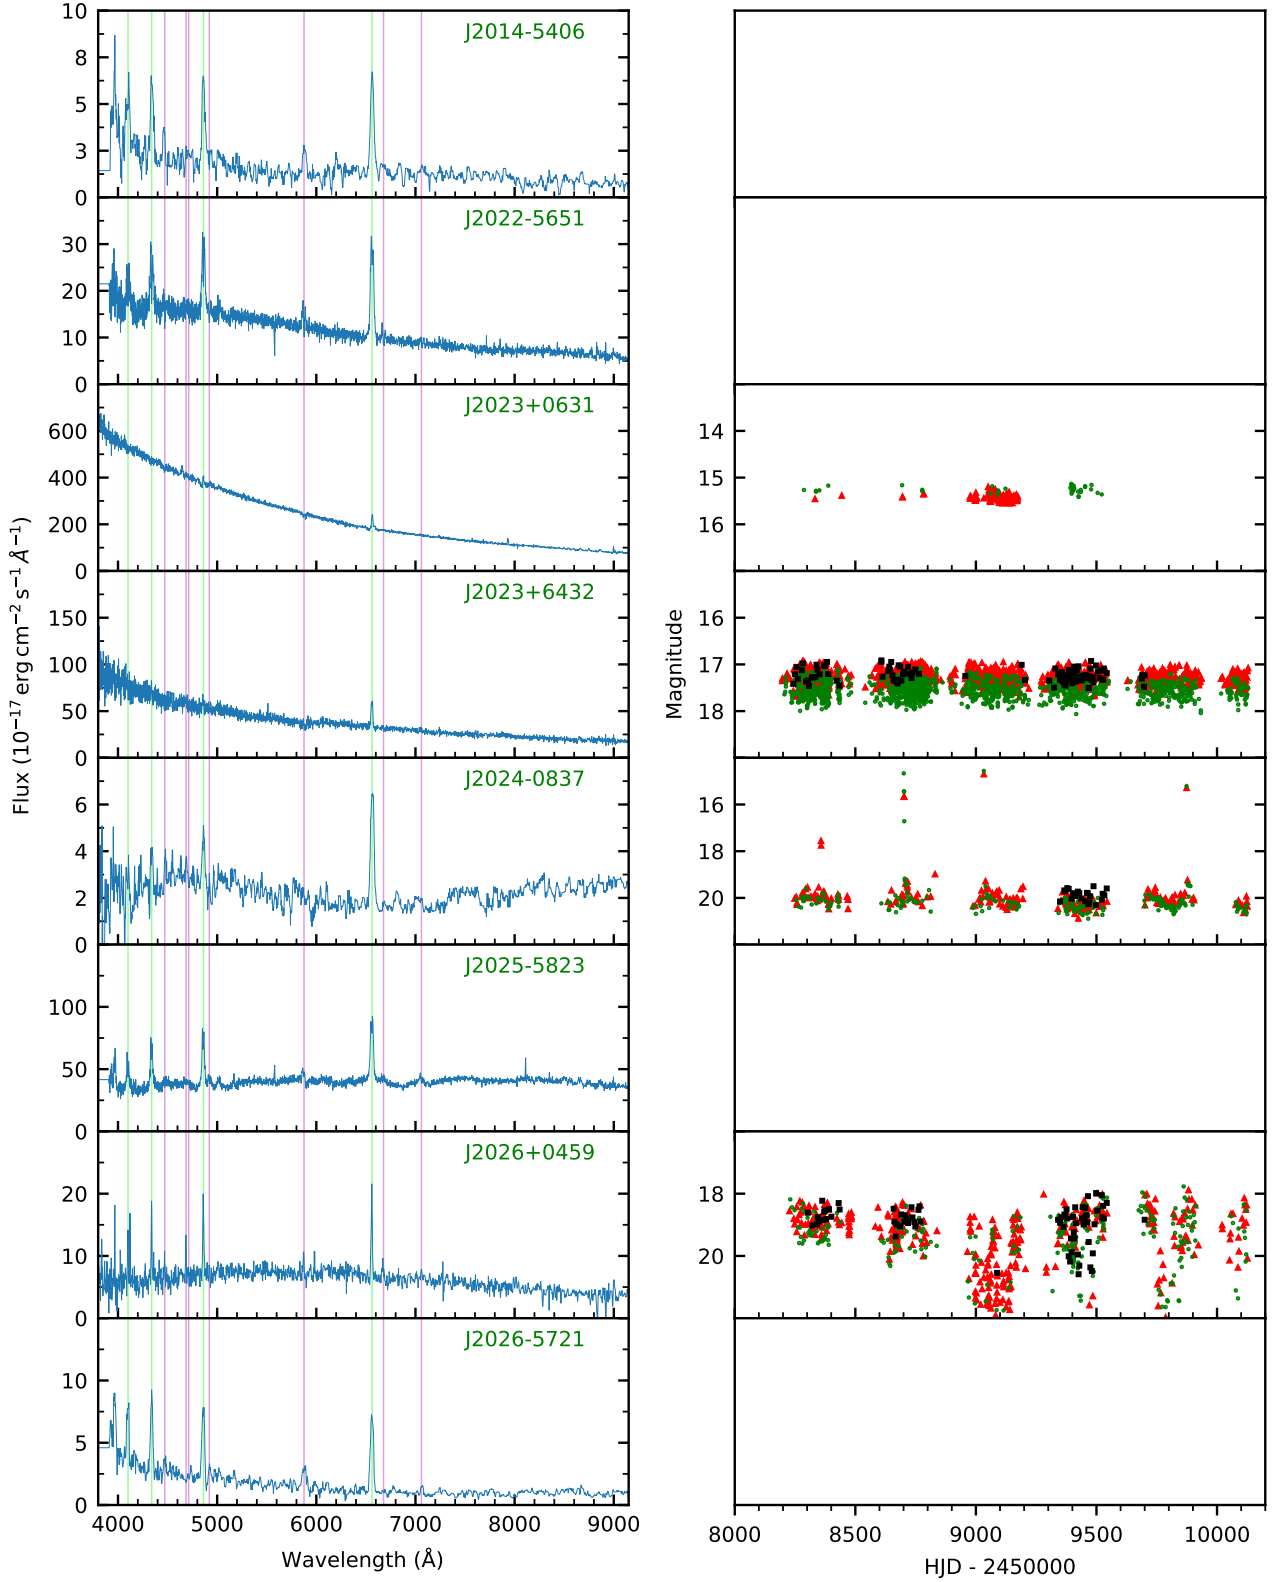

Figure 56: Left panels: Spectra with H lines shown in green and He in pink. Right panels: Light curves with ZTF  $r$ -band shown in red triangles,  $g$ -band in green dots and  $i$ -band in black squares.

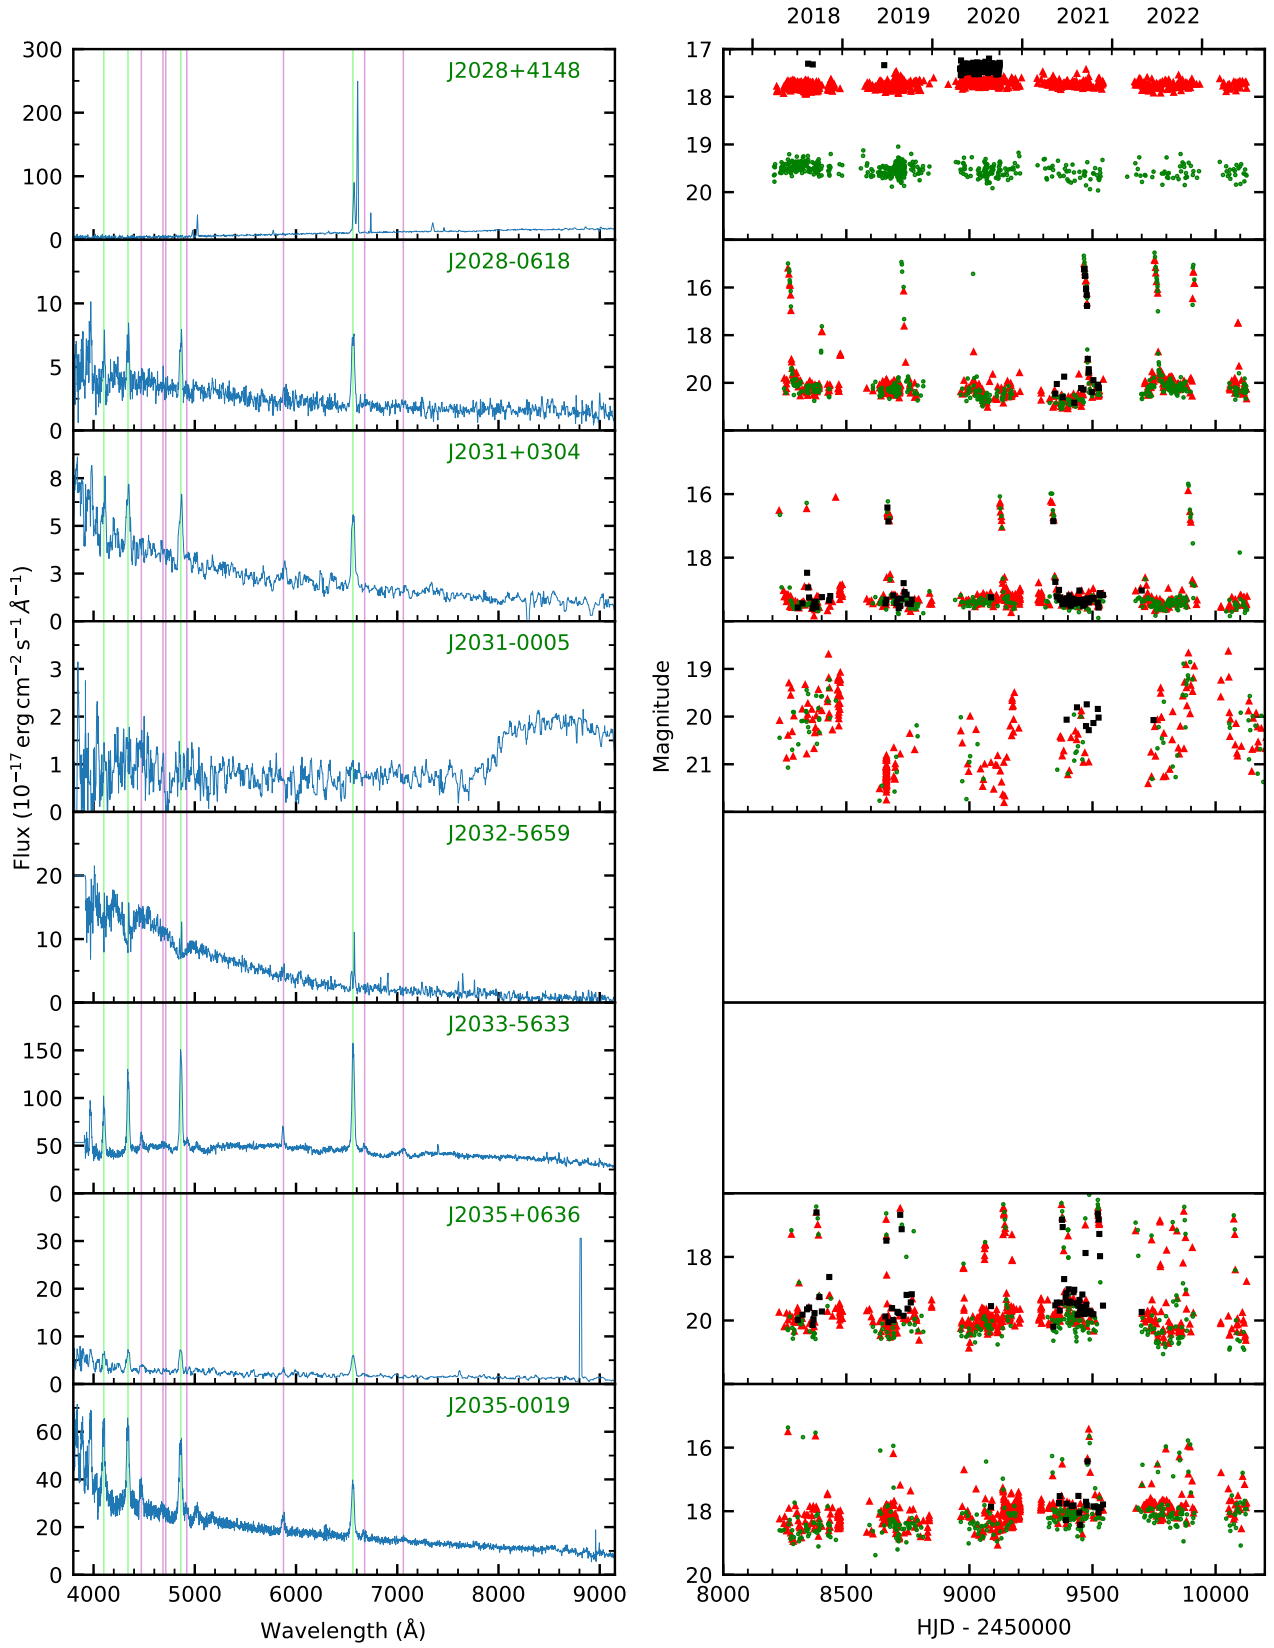

Figure 57: Left panels: Spectra with H lines shown in green and He in pink. Right panels: Light curves with ZTF  $r$ -band shown in red triangles,  $g$ -band in green dots and  $i$ -band in black squares.

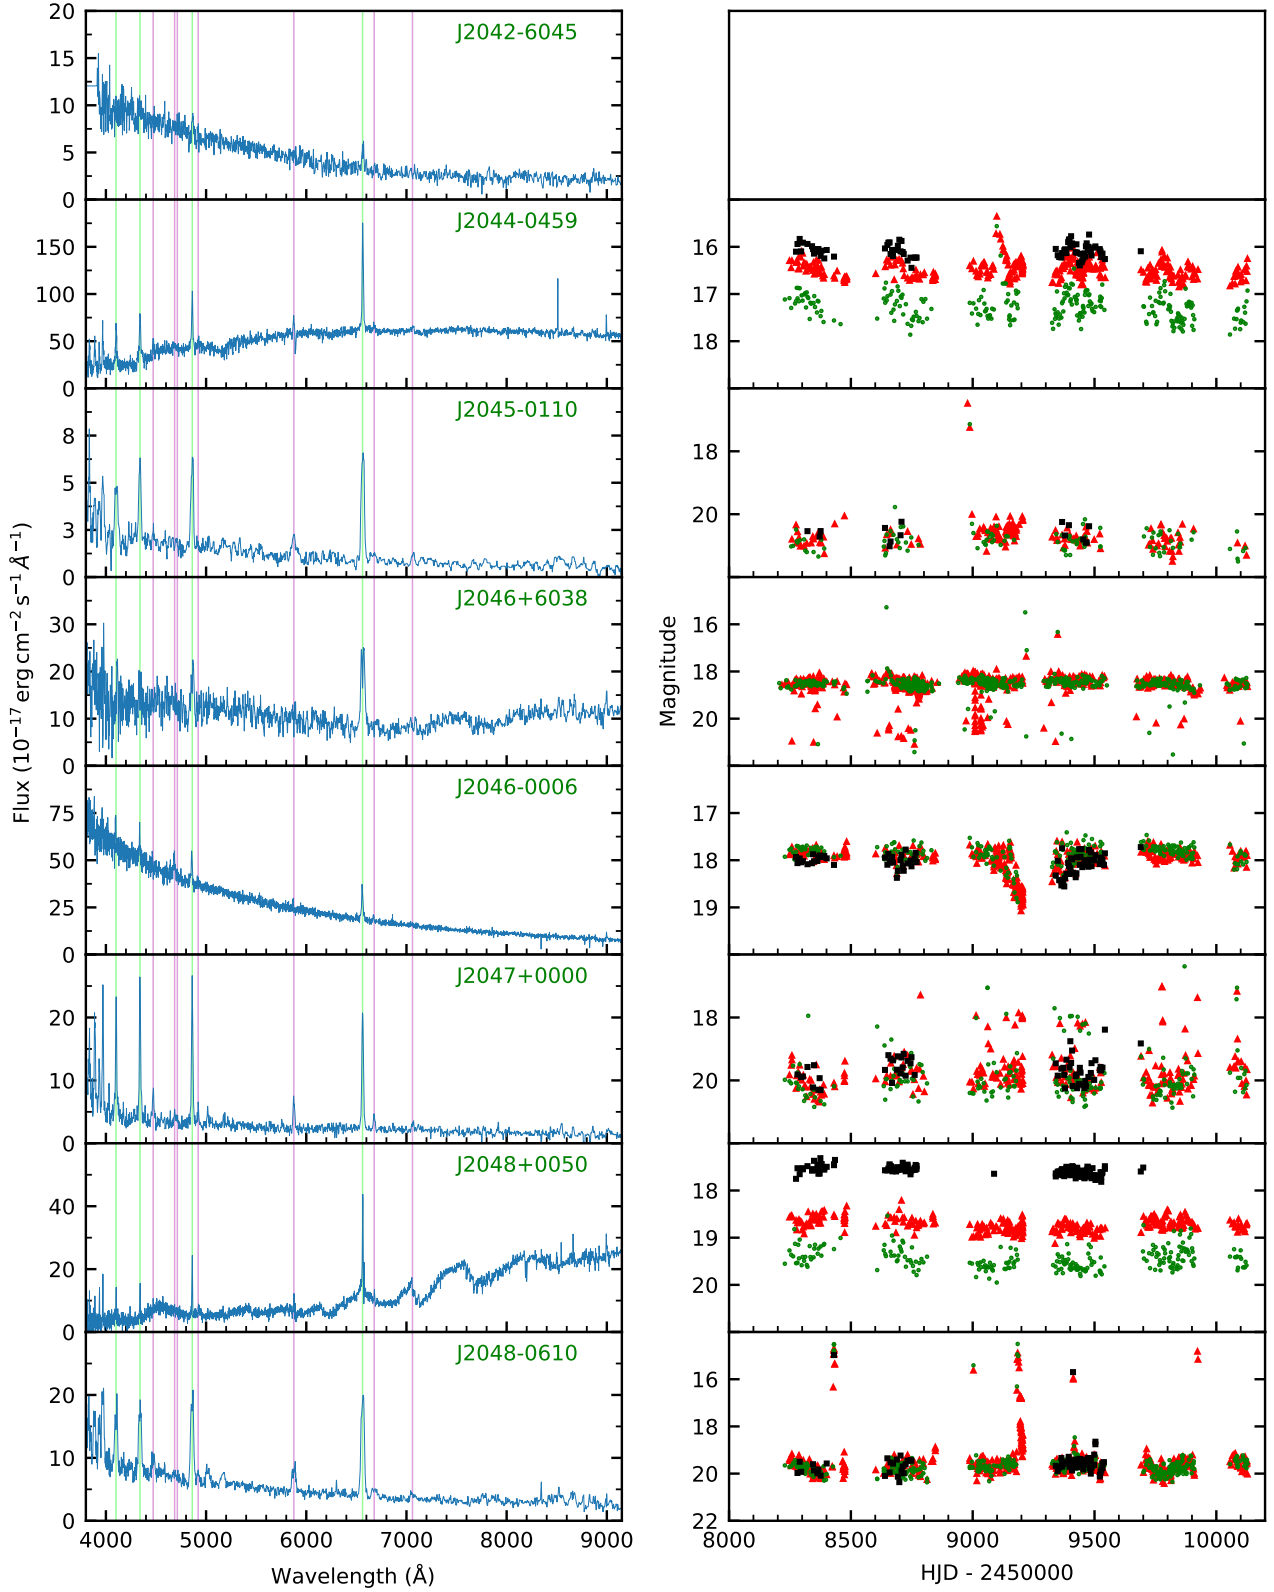

Figure 58: Left panels: Spectra with H lines shown in green and He in pink. Right panels: Light curves with ZTF  $r$ -band shown in red triangles,  $g$ -band in green dots and  $i$ -band in black squares.

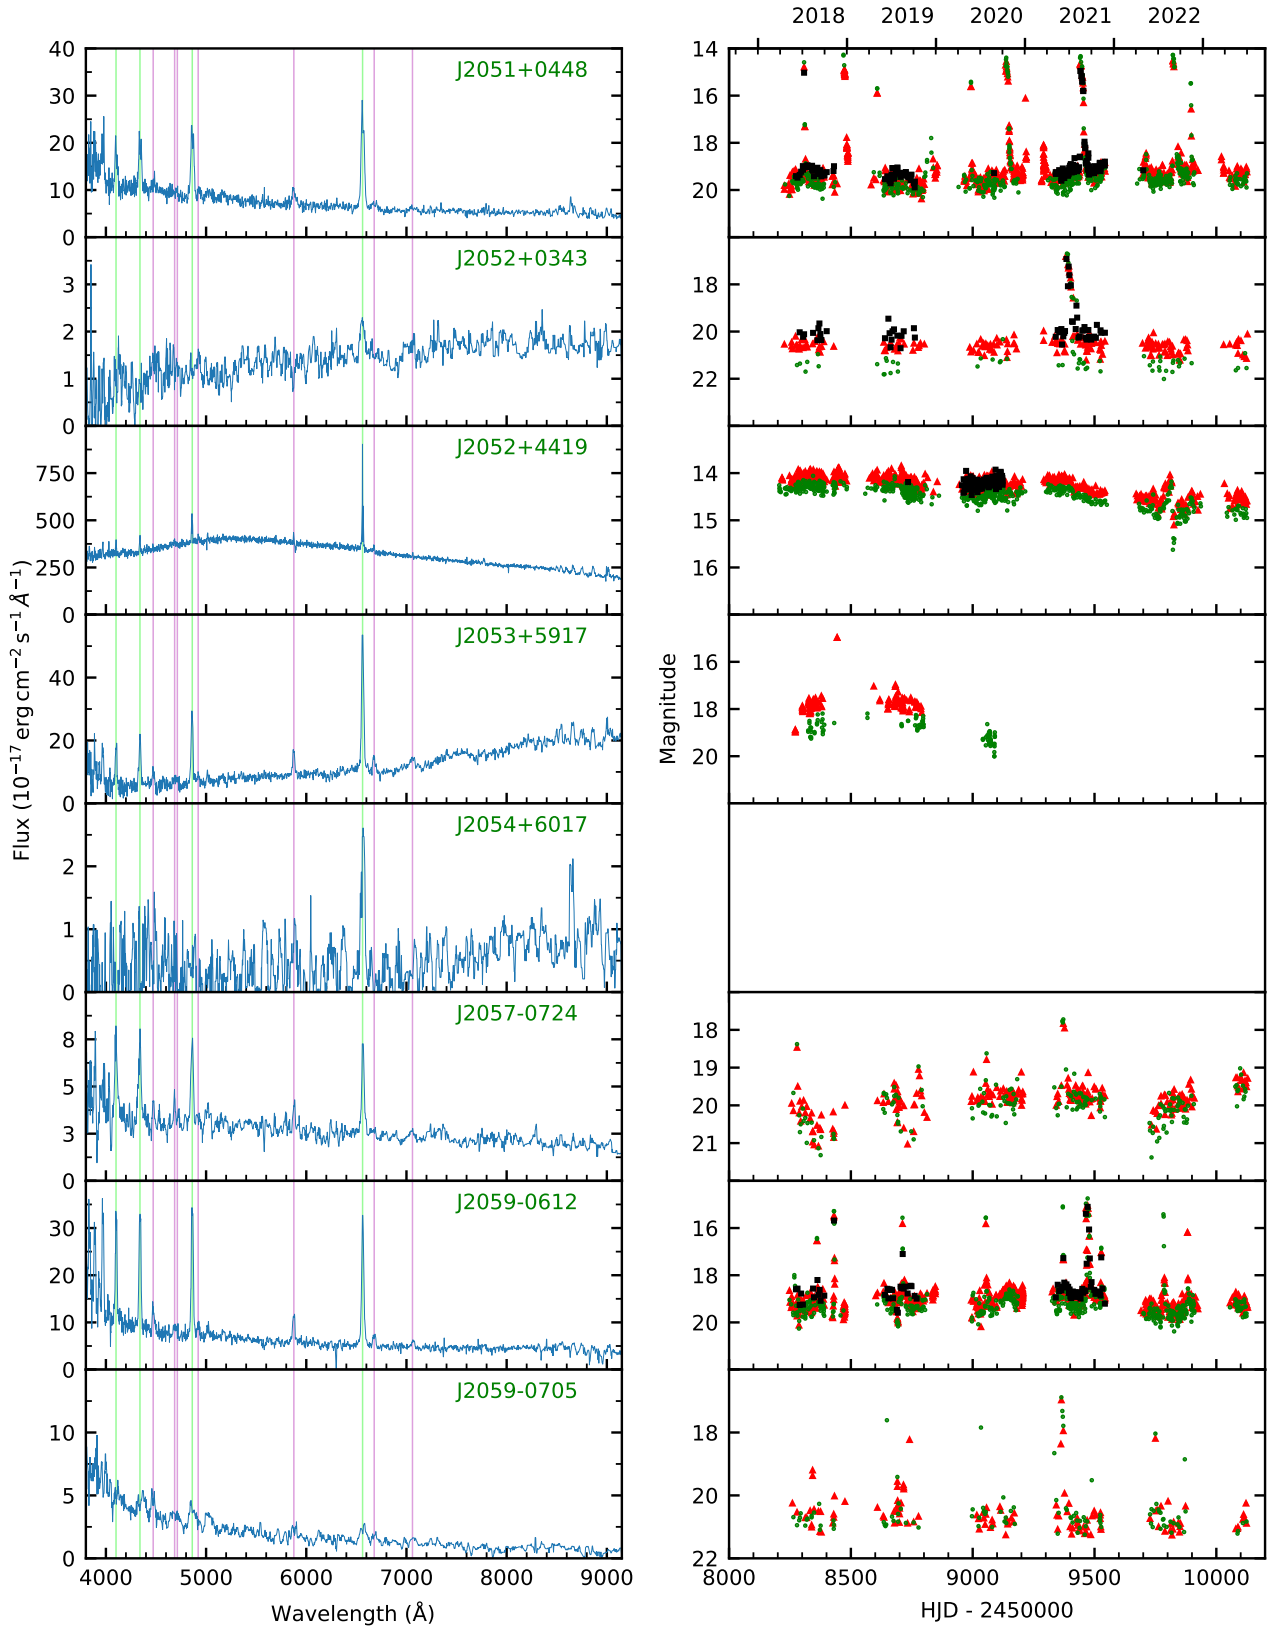

Figure 59: Left panels: Spectra with H lines shown in green and He in pink. Right panels: Light curves with ZTF *r*-band shown in red triangles, *g*-band in green dots and *i*-band in black squares.

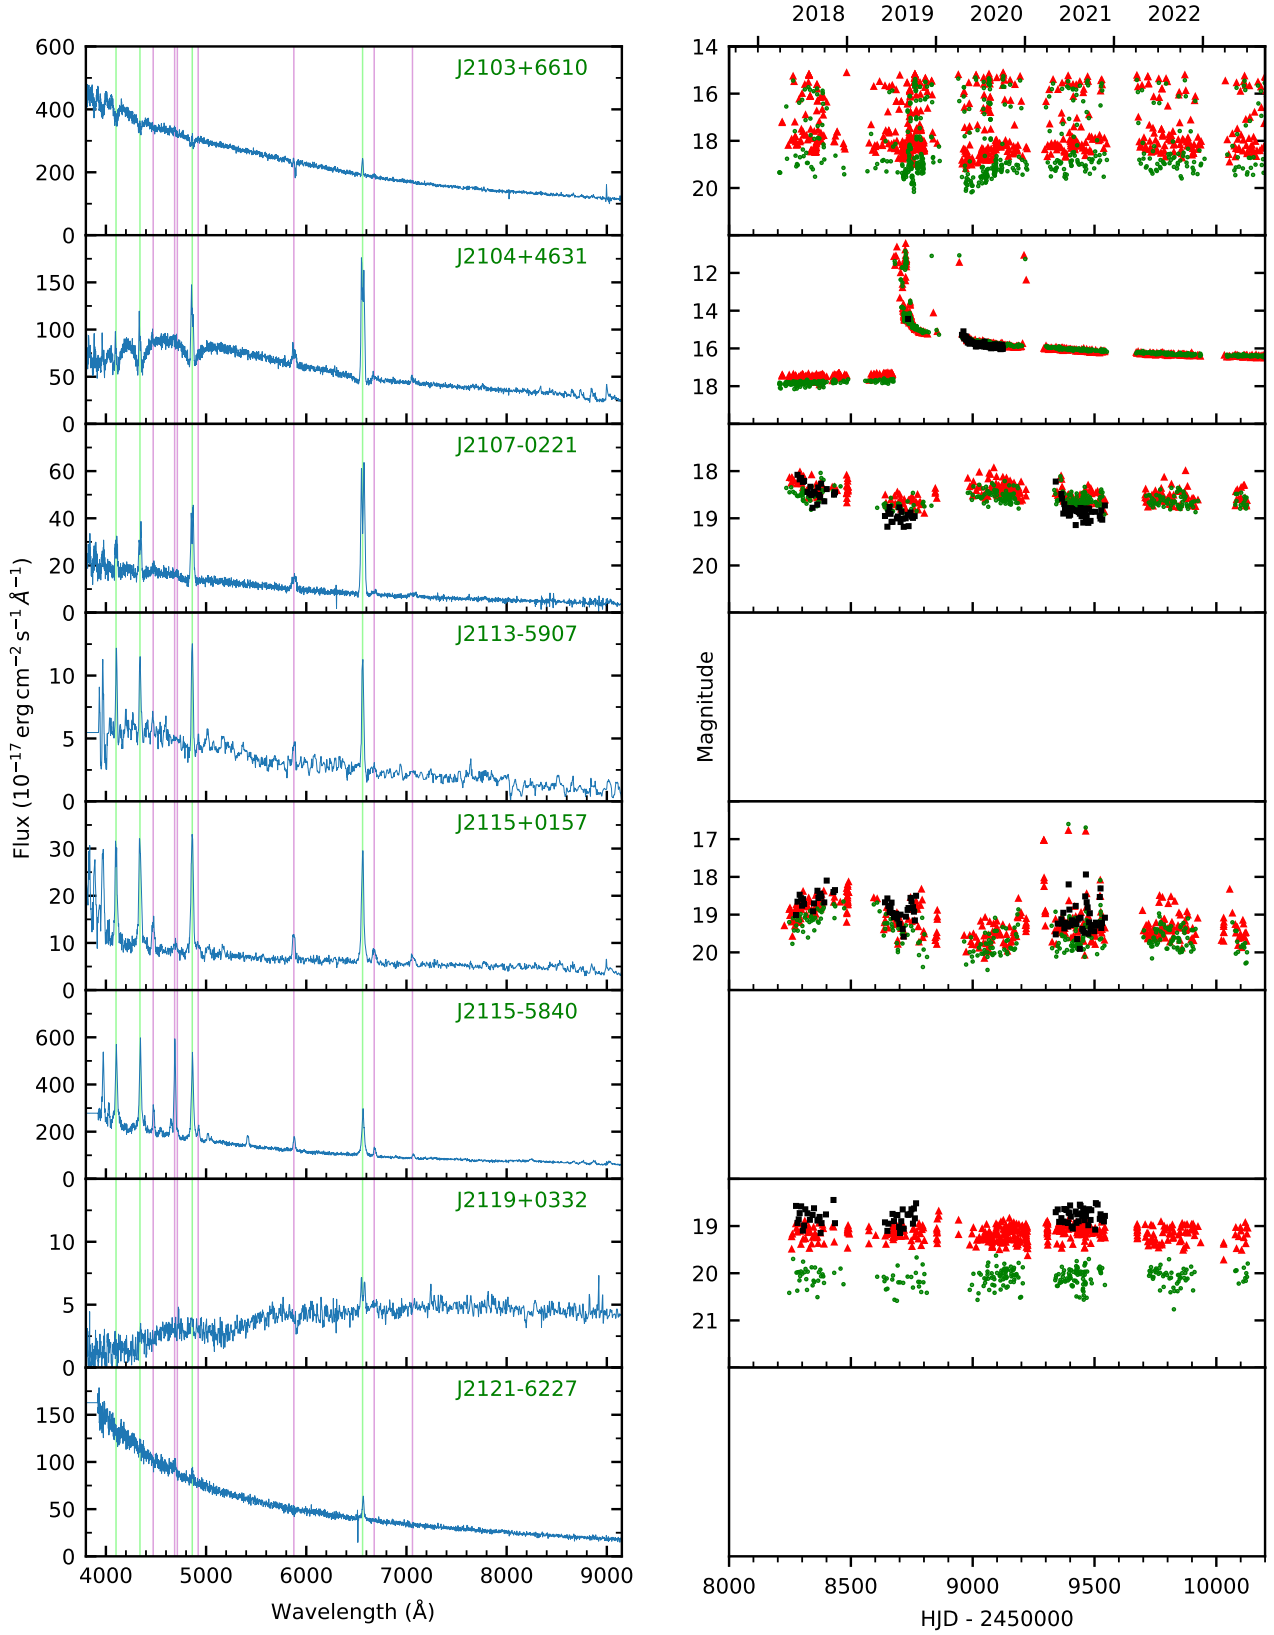

Figure 60: Left panels: Spectra with H lines shown in green and He in pink. Right panels: Light curves with ZTF  $r$ -band shown in red triangles,  $g$ -band in green dots and  $i$ -band in black squares.



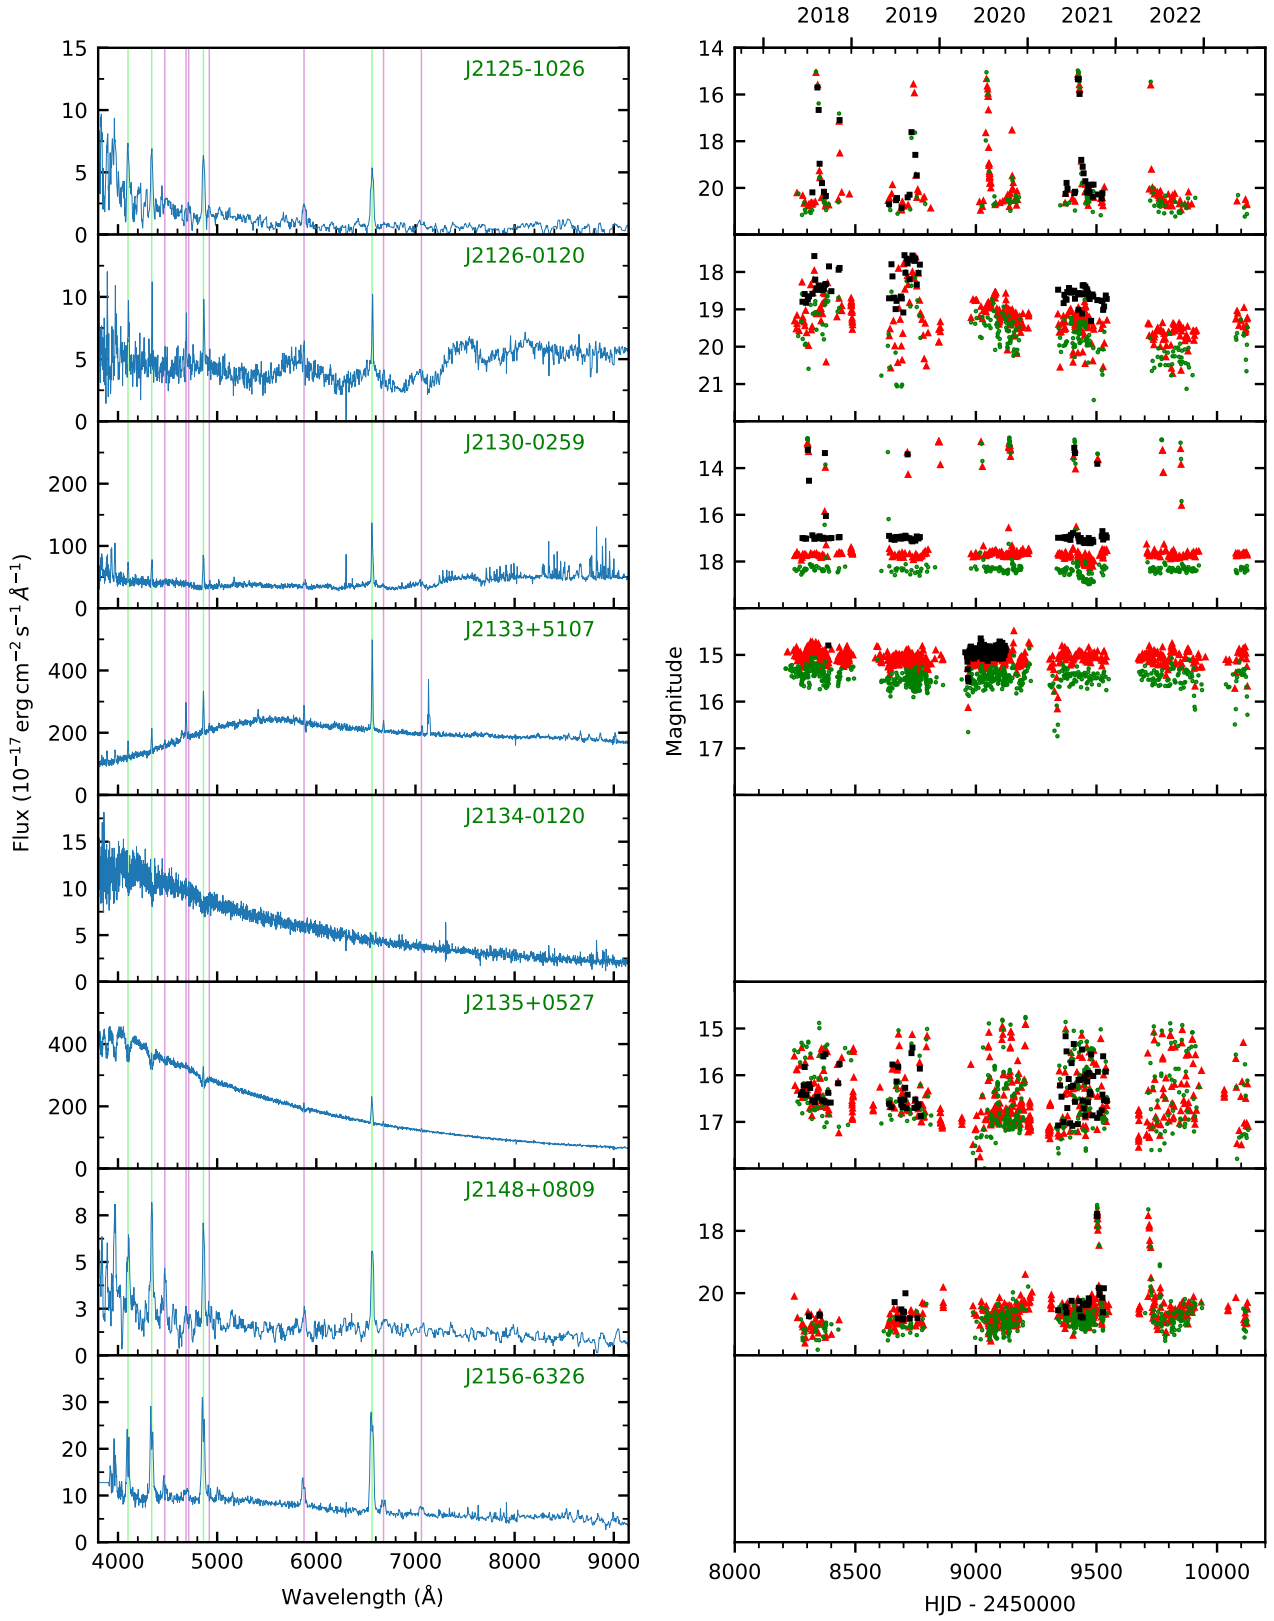

Figure 61: Left panels: Spectra with H lines shown in green and He in pink. Right panels: Light curves with ZTF *r*-band shown in red triangles, *g*-band in green dots and *i*-band in black squares.

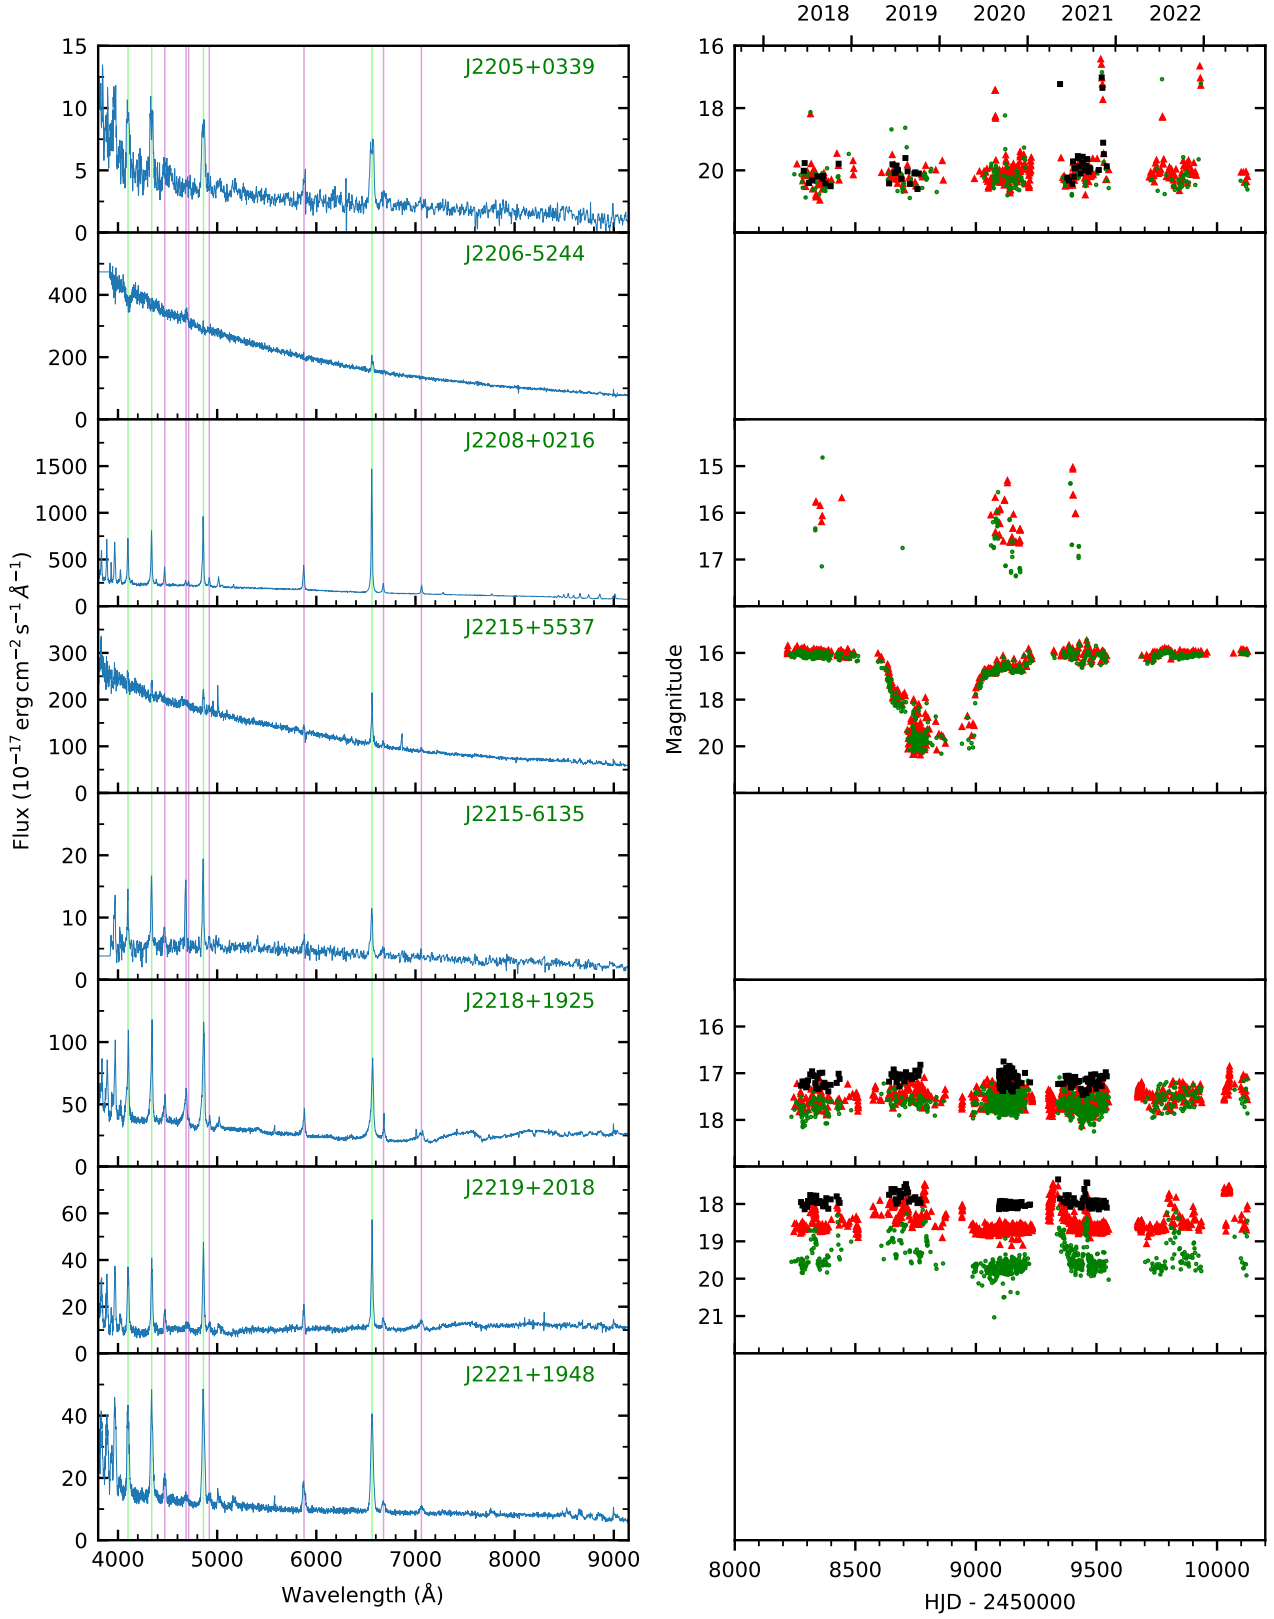

Figure 62: Left panels: Spectra with H lines shown in green and He in pink. Right panels: Light curves with ZTF  $r$ -band shown in red triangles,  $g$ -band in green dots and  $i$ -band in black squares.

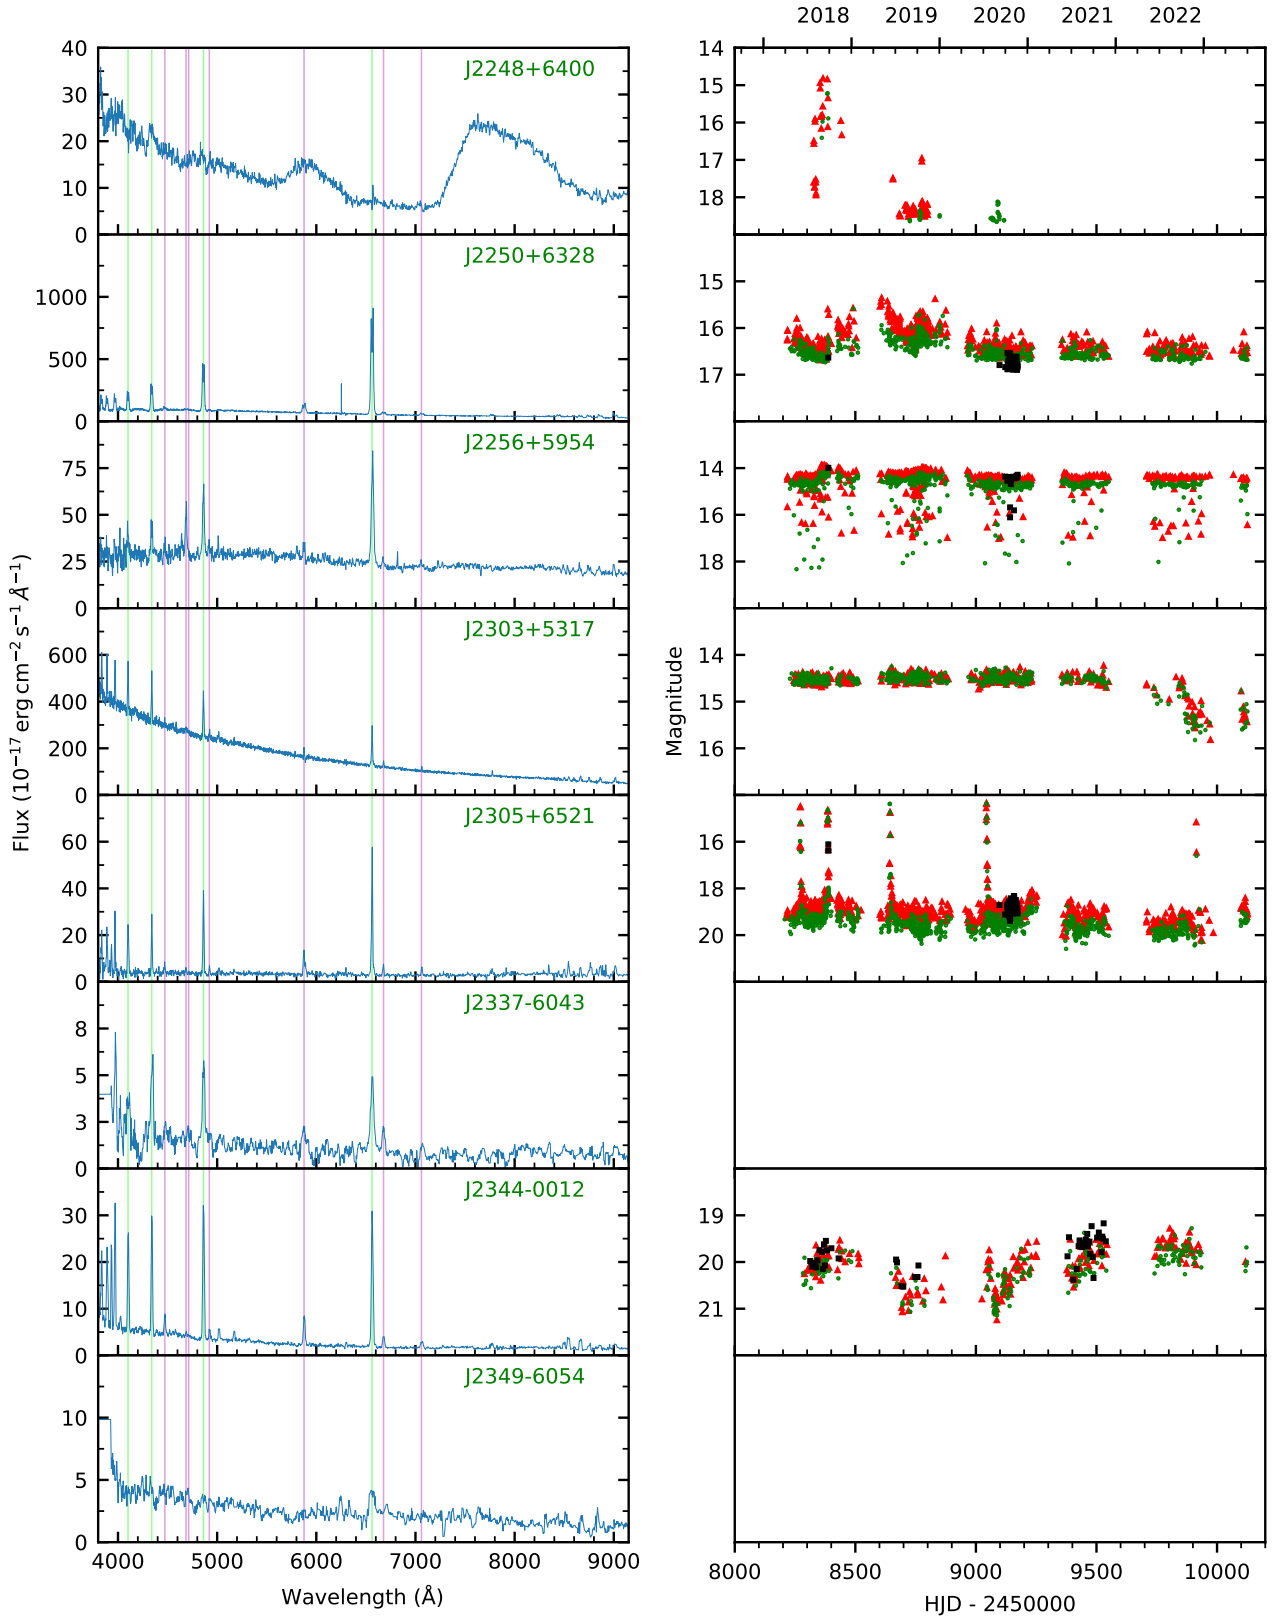

Figure 63: Left panels: Spectra with H lines shown in green and He in pink. Right panels: Light curves with ZTF *r*-band shown in red triangles, *g*-band in green dots and *i*-band in black squares.

## 5 FIELD, MJD AND CATALOG ID LIST

Table 2: Field, MJD and catalog id references for CVs in the paper.

| SDSS name           | Other name                    | Field  | MJD   | Catalog ID        |
|---------------------|-------------------------------|--------|-------|-------------------|
| J000155.14-670743.3 | EF Tuc                        | 028965 | 60158 | 27021599481868177 |
| J000600.15+012129.8 |                               | 015039 | 59202 | 4399110982        |
| J000633.70-690033.8 | HV 8001                       | 028989 | 60131 | 27021599481830608 |
| J000844.33-014014.8 | Gaia15abi                     | 104597 | 59901 | 27021597933082324 |
| J001204.50+020129.6 |                               | 104642 | 59879 | 27021597957512149 |
|                     |                               | 104642 | 59846 | 27021597957512149 |
|                     |                               | 104642 | 59874 | 27021597957512149 |
| J002243.55+061002.7 | MGAB-V295                     | 104593 | 59911 | 27021597957636042 |
| J002257.65+614107.5 | V1033 Cas                     | 100575 | 59886 | 27021597853972413 |
| J002728.02-010828.7 | EN Cet                        | 104578 | 59907 | 27021597933124837 |
| J002848.83+591722.0 | V709 Cas                      | 100193 | 59915 | 27021597853363162 |
| J003529.47-735826.3 |                               | 029039 | 60127 | 27021599477911274 |
| J003827.05+250925.0 | 1RXS J003828.7+250920         | 015006 | 59227 | 4400901787        |
|                     |                               | 104664 | 59906 | 27021597959240780 |
| J003941.08+005427.5 | SDSS J003941.06+005427.5      | 015005 | 59193 | 4399288456        |
|                     |                               | 015005 | 59167 | 4399288456        |
| J004335.16-003729.7 |                               | 015007 | 59187 | 4374673159        |
|                     |                               | 104644 | 59828 | 27021597933263165 |
| J005000.03-760827.3 | BMAM-V424                     | 029059 | 60165 | 27021599455602617 |
| J005050.87+000912.6 | GS Cet                        | 104650 | 59910 | 27021597957693040 |
| J010411.62-031342.2 |                               | 104666 | 59928 | 27021597933568957 |
| J012132.92-740819.5 |                               | 029018 | 60133 | 27021599478861155 |
| J012754.58-581717.5 | ASASSN -15bg                  | 028822 | 60180 | 27021599485906911 |
| J012905.53-580841.2 |                               | 028822 | 60180 | 27021599485908569 |
| J014227.07+001729.8 |                               | 015012 | 59166 | 4399911413        |
|                     |                               | 015012 | 59191 | 4399911413        |
|                     |                               | 015012 | 59220 | 4399911413        |
| J015007.16+302203.9 | ZTF18abtgdwr                  | 100313 | 59817 | 27021597964645433 |
| J015543.47+002807.4 | FL Cet                        | 015013 | 59165 | 4401495339        |
|                     |                               | 015013 | 59221 | 4401495339        |
|                     |                               | 015013 | 59197 | 4401495339        |
| J020712.72-014116.3 |                               | 015045 | 59169 | 4375881540        |
|                     |                               | 015045 | 59202 | 4375881540        |
|                     |                               | 015045 | 59223 | 4375881540        |
| J020809.57+565239.7 |                               | 015106 | 59209 | 4301276266        |
| J021008.36+571121.1 | UV Per                        | 015106 | 59209 | 4301317711        |
| J021315.48+533822.9 | MASTER OT J021315.37+533822.7 | 015217 | 59238 | 4301671409        |
| J022102.78+732245.1 | ASASSN-14jq                   | 015074 | 59189 | 4325309343        |
| J022623.33+711831.5 | AM Cas                        | 015074 | 59189 | 4317455905        |
| J023322.61+005059.2 | HP Cet                        | 104652 | 59935 | 27021597960180417 |
|                     |                               | 015014 | 59165 | 4401862688        |
|                     |                               | 015014 | 59191 | 4401862688        |
|                     |                               | 015014 | 59232 | 4401862688        |
|                     |                               | 104652 | 59881 | 27021597960180417 |
| J024131.07+593630.4 | ASASSN-16jv                   | 015218 | 59245 | 4320105035        |
| J024607.56-633546.0 | RU Hor                        | 028880 | 60167 | 27021599482465174 |
|                     |                               | 028880 | 60168 | 27021599482465174 |
|                     |                               | 028880 | 60170 | 27021599482465174 |
| J024720.92-605050.7 |                               | 028851 | 60178 | 27021599482732702 |
|                     |                               | 028851 | 60177 | 27021599482732702 |
| J031538.60+623314.9 | ASASSN-15qx                   | 103743 | 59955 | 27021597882256421 |
| J032815.90+612517.5 | Gaia19bbb                     | 103743 | 59955 | 27021597882366166 |
| J034515.42-015216.4 | CSS 090219:034515-015216      | 101817 | 59844 | 27021597970642295 |
|                     |                               | 101817 | 59845 | 27021597970642295 |
| J040834.99+511448.2 | FO Per                        | 015107 | 59212 | 4332130940        |
|                     |                               | 103793 | 59971 | 27021597891268484 |

| SDSS name           | Other name                    | Field  | MJD   | Catalog ID        |
|---------------------|-------------------------------|--------|-------|-------------------|
| J041428.92-631946.0 |                               | 029463 | 59940 | 27021599477559814 |
| J041844.43+510731.3 | NS Per                        | 103793 | 59971 | 27021597893345749 |
|                     |                               | 015107 | 59212 | 4334212418        |
| J042609.35+354144.3 | MASTER OT J042609.34+354144.8 | 015223 | 59265 | 4515489221        |
| J043118.90-005534.9 |                               | 103629 | 59939 | 27021597973615410 |
|                     |                               | 103629 | 59941 | 27021597973615410 |
|                     |                               | 103629 | 59934 | 27021597973615410 |
| J043127.01+352713.0 | ASASSN-16og                   | 015223 | 59265 | 4515458902        |
| J044321.37+472125.8 | V392 Per                      | 015224 | 59238 | 4337185134        |
| J044652.51+471408.3 |                               | 015224 | 59238 | 4337774254        |
| J050153.52-034208.6 | ZTF18abwtmcs                  | 103656 | 59871 | 27021597973789185 |
|                     |                               | 103656 | 59872 | 27021597973789185 |
|                     |                               | 103656 | 59878 | 27021597973789185 |
|                     |                               | 103667 | 59882 | 27021597973789185 |
| J050503.07+222529.7 | ASASSN-15su                   | 015072 | 59186 | 4503355683        |
|                     |                               | 015072 | 59216 | 4503355683        |
|                     |                               | 015189 | 59274 | 4503355683        |
| J050906.73-032507.7 | ASASSN-15em                   | 103657 | 59910 | 27021597975125493 |
|                     |                               | 103657 | 59912 | 27021597975125493 |
|                     |                               | 103657 | 59911 | 27021597975125493 |
| J051042.60+513539.9 | MASTER OT J051042.59+513540.0 | 102868 | 59914 | 27021597900942914 |
|                     |                               | 102868 | 59956 | 27021597900942914 |
| J051419.88+011120.9 | CSS 091109:051420+011121      | 103958 | 59901 | 27021598053225858 |
|                     |                               | 103958 | 59906 | 27021598053225858 |
|                     |                               | 103958 | 59907 | 27021598053225858 |
| J051814.55-024503.1 | CSS 090219:051815-024503      | 103612 | 59979 | 27021597975240809 |
| J051949.58+642921.7 | ZTF18acnavqf                  | 103733 | 59893 | 27021597889204245 |
| J052316.13-630728.9 | ASASSN-14ky                   | 029581 | 59971 | 27021599483362979 |
|                     |                               | 029581 | 59968 | 27021599483362979 |
| J052433.47-070527.9 | CSS 101108:052433-070528      | 015111 | 59218 | 4416243172        |
| J052834.08+331821.7 | QZ Aur                        | 015112 | 59238 | 4513598719        |
|                     |                               | 015112 | 59211 | 4513598719        |
| J052859.54-033352.4 | V1159 Ori                     | 015075 | 59216 | 4417020320        |
|                     |                               | 015075 | 59187 | 4417020320        |
| J060602.72-603941.4 | ASASSN-14jf                   | 029663 | 59937 | 27021599421975715 |
|                     |                               | 029663 | 59967 | 27021599421975715 |
|                     |                               | 029663 | 59968 | 27021599421975715 |
|                     |                               | 029663 | 59935 | 27021599421975715 |
|                     |                               | 029663 | 59936 | 27021599421975715 |
|                     |                               | 029663 | 59940 | 27021599421975715 |
|                     |                               | 029663 | 59963 | 27021599421975715 |
|                     |                               | 029663 | 59969 | 27021599421975715 |
|                     |                               | 029663 | 59907 | 27021599421975715 |
| J061204.48+252832.5 | HQ Gem                        | 015085 | 59216 | 4539229700        |
| J061222.10-594449.3 |                               | 029677 | 59935 | 27021599422001425 |
|                     |                               | 029677 | 59964 | 27021599422001425 |
|                     |                               | 029677 | 59941 | 27021599422001425 |
|                     |                               | 029677 | 59998 | 27021599422001425 |
|                     |                               | 029677 | 59997 | 27021599422001425 |
|                     |                               | 029677 | 59999 | 27021599422001425 |
|                     |                               | 029677 | 59934 | 27021599422001425 |
|                     |                               | 029677 | 59937 | 27021599422001425 |
| J061558.69-515423.9 | DDE 100                       | 029640 | 59958 | 27021599423197108 |
| J061643.22+152411.2 | CZ Ori                        | 104052 | 59888 | 27021598092904166 |
| J062157.14+404236.1 | ASASSN-18bz                   | 015197 | 59245 | 4552310569        |
|                     |                               | 015197 | 59271 | 4552310569        |
|                     |                               | 015288 | 59294 | 4552310569        |
| J062406.13+400743.8 |                               | 015197 | 59245 | 4552297765        |
| J062429.71+002105.8 | ASASSN-15cu                   | 015139 | 59205 | 4522186828        |
| J062516.28+733439.1 | MU Cam                        | 102134 | 59979 | 27021597912261811 |
| J062601.53-035522.9 | Gaia17cdo                     | 015279 | 59302 | 4470182587        |

| SDSS name           | Other name                 | Field  | MJD   | Catalog ID        |
|---------------------|----------------------------|--------|-------|-------------------|
| J062724.39+161329.6 | Gaia18atj                  | 015228 | 59269 | 4535621315        |
| J062953.89-033508.4 | 1RXS J062954.6-033520      | 015279 | 59302 | 4471416011        |
|                     |                            | 103458 | 59896 | 27021598029332739 |
| J063047.05+023931.2 | ASASSN-16ow                | 015115 | 59219 | 4523820411        |
| J063301.12+030333.8 |                            | 015115 | 59210 | 4523888653        |
|                     |                            | 015115 | 59219 | 4523888653        |
| J063304.77+032422.7 | Gaia17ber                  | 015115 | 59210 | 4523900017        |
|                     |                            | 015115 | 59219 | 4523900017        |
| J063516.63+030313.6 |                            | 015115 | 59210 | 4523895353        |
|                     |                            | 015115 | 59219 | 4523895353        |
| J063654.60+000217.2 | CW Mon                     | 103456 | 59654 | 27021598081319295 |
|                     |                            | 103456 | 60016 | 27021598081319295 |
| J063844.17+181611.4 | UV Gem                     | 015229 | 59303 | 4537522851        |
| J063938.60+055352.7 | V959 Mon                   | 103472 | 59884 | 27021598082718844 |
|                     |                            | 103472 | 60012 | 27021598082718844 |
|                     |                            | 103472 | 60036 | 27021598082718844 |
| J064949.95+554140.4 | ASASSN-19an                | 102781 | 59913 | 27021597915757969 |
| J064950.93-073741.0 | RX J0649.8-0737            | 103415 | 59954 | 27021598027368848 |
|                     |                            | 103415 | 59955 | 27021598027368848 |
| J065733.66-533422.0 | BMAM-V547                  | 025276 | 59996 | 27021599421562063 |
| J070533.80-125004.8 |                            | 015086 | 59220 | 4473644736        |
|                     |                            | 015086 | 59267 | 4473644736        |
| J070648.97+032448.3 | MG1 400618                 | 103440 | 59896 | 27021602546994073 |
|                     |                            | 103440 | 59895 | 27021602546994073 |
| J070816.61-124544.8 | ASASSN-16an                | 015086 | 59220 | 4473686001        |
|                     |                            | 015086 | 59267 | 4473686001        |
| J072142.29-640050.8 |                            | 027572 | 59986 | 27021599409445614 |
| J072304.79+020437.2 | LAMOST J072304.77+020437.4 | 103410 | 59958 | 27021598089539693 |
| J073143.87+011714.9 | NSV 3626                   | 103397 | 60011 | 27021598089527489 |
| J073339.29+212200.8 | CSS 091111:073339+212201   | 015195 | 59238 | 4543017594        |
|                     |                            | 015195 | 59271 | 4543017594        |
|                     |                            | 015286 | 59276 | 4543017594        |
|                     |                            | 015286 | 59294 | 4543017594        |
| J073758.55+205544.6 |                            | 015195 | 59238 | 4543080695        |
|                     |                            | 015195 | 59271 | 4543080695        |
|                     |                            | 015286 | 59276 | 4543080695        |
|                     |                            | 015286 | 59294 | 4543080695        |
| J073817.74+285519.7 |                            | 015016 | 59168 | 4551094200        |
|                     |                            | 015016 | 59193 | 4551094200        |
|                     |                            | 015016 | 59219 | 4551094200        |
|                     |                            | 015016 | 59248 | 4551094200        |
|                     |                            | 015016 | 59276 | 4551094200        |
| J073835.88+095805.6 | ASASSN-14jk                | 100884 | 60000 | 27021598092319179 |
| J074222.55+172806.7 | MLS 110309:074223+172807   | 015073 | 59212 | 4542234653        |
|                     |                            | 015192 | 59302 | 4542234653        |
| J074419.74+325448.2 | CSS 091029:074420+325448   | 015018 | 59251 | 4551693466        |
|                     |                            | 015018 | 59164 | 4551693466        |
| J074859.55+312512.5 |                            | 015018 | 59164 | 4554606943        |
|                     |                            | 015018 | 59197 | 4554606943        |
|                     |                            | 015018 | 59221 | 4554606943        |
|                     |                            | 015018 | 59251 | 4554606943        |
|                     |                            | 015018 | 59280 | 4554606943        |
| J074917.11+365427.9 | MGAB-V3545                 | 015020 | 59200 | 4555251014        |
|                     |                            | 015020 | 59223 | 4555251014        |
|                     |                            | 015020 | 59248 | 4555251014        |
|                     |                            | 015020 | 59284 | 4555251014        |
| J075107.51+300628.3 |                            | 015019 | 59164 | 4554586605        |
|                     |                            | 015019 | 59199 | 4554586605        |
|                     |                            | 015019 | 59252 | 4554586605        |
|                     |                            | 015019 | 59281 | 4554586605        |
| J075116.99+100016.3 |                            | 100154 | 59940 | 27021598102026488 |

| SDSS name           | Other name                    | Field  | MJD   | Catalog ID        |
|---------------------|-------------------------------|--------|-------|-------------------|
| J075233.17+294339.5 |                               | 015019 | 59164 | 4554593045        |
|                     |                               | 015019 | 59199 | 4554593045        |
|                     |                               | 015019 | 59222 | 4554593045        |
|                     |                               | 015019 | 59252 | 4554593045        |
|                     |                               | 015019 | 59281 | 4554593045        |
| J075240.45+362823.2 | EU Lyn                        | 015020 | 59200 | 4555246166        |
|                     |                               | 015020 | 59223 | 4555246166        |
|                     |                               | 015020 | 59248 | 4555246166        |
|                     |                               | 015020 | 59284 | 4555246166        |
| J075331.98+375800.6 | CSS 100407:075332+375801      | 015020 | 59200 | 4555391061        |
|                     |                               | 015020 | 59223 | 4555391061        |
|                     |                               | 015020 | 59248 | 4555391061        |
|                     |                               | 015020 | 59284 | 4555391061        |
| J075450.15+091019.6 | MASTER OT J075450.18+091020.2 | 100154 | 59940 | 27021598101908464 |
| J075515.20+060439.3 | ASASSN-15tr                   | 104363 | 59935 | 27021598101332981 |
|                     |                               | 104363 | 59936 | 27021598101332981 |
|                     |                               | 104363 | 59937 | 27021598101332981 |
| J075522.38+040719.3 |                               | 104365 | 59881 | 27021598101254790 |
| J075540.64+264618.1 | V516 Gem                      | 015021 | 59165 | 4554360127        |
| J075648.85-124653.9 | ATO J119.2035-12.7816         | 104357 | 59653 | 27021598043765451 |
|                     |                               | 104357 | 59651 | 27021598043765451 |
|                     |                               | 104357 | 59655 | 27021598043765451 |
| J075653.12+085831.9 |                               | 100154 | 59940 | 27021598101909805 |
| J075655.95+062646.7 |                               | 104363 | 59937 | 27021598101827626 |
|                     |                               | 104363 | 59936 | 27021598101827626 |
| J075939.78+191417.3 |                               | 101944 | 59884 | 27021598103725375 |
| J080033.86+192416.6 | CRTS J080033.8+192416         | 101944 | 59884 | 27021598103748289 |
| J080407.93-002216.4 | MGAB-V3549                    | 104378 | 59910 | 27021598048577276 |
| J080448.88+024853.5 | ASASSN-16ac                   | 104371 | 59911 | 27021598101175327 |
| J080534.48+072029.1 |                               | 104367 | 59994 | 27021598101960384 |
|                     |                               | 104367 | 59967 | 27021598101960384 |
| J080538.98+354054.9 | CSS 170417:080539+354055      | 015022 | 59165 | 4555277564        |
|                     |                               | 015022 | 59231 | 4555277564        |
|                     |                               | 015022 | 59252 | 4555277564        |
| J080727.59-763159.8 | Z Cha                         | 027498 | 59948 | 27021599406316148 |
|                     |                               | 027498 | 59952 | 27021599406316148 |
|                     |                               | 027498 | 59982 | 27021599406316148 |
|                     |                               | 027498 | 59981 | 27021599406316148 |
| J080818.98+005859.8 | ASASSN-15cw                   | 104379 | 59994 | 27021598101465688 |
|                     |                               | 104379 | 59999 | 27021598101465688 |
| J080837.79-694712.8 | ASASSN-14jd                   | 027533 | 60010 | 27021599408236414 |
|                     |                               | 027533 | 59983 | 27021599408236414 |
|                     |                               | 027533 | 59983 | 27021599408236413 |
|                     |                               | 027533 | 60010 | 27021599408236413 |
| J080853.73+355053.6 | CSS 080416:080854+355053      | 015025 | 59169 | 4555351659        |
|                     |                               | 015025 | 59255 | 4555351659        |
| J081210.23+040351.3 | CSS 091017:081210+040352      | 104372 | 59965 | 27021598101645021 |
|                     |                               | 104372 | 59958 | 27021598101645021 |
| J081225.44-711437.2 | ASASSN-15qb                   | 027534 | 59981 | 27021599408538428 |
| J081228.29+623621.9 | SU UMa                        | 102962 | 59899 | 27021597914287058 |
| J081318.41-010326.7 | ASASSN -14ag                  | 104377 | 59900 | 27021598048898985 |
| J081321.93+452809.2 | FH Lyn                        | 102888 | 60003 | 27021597919961171 |
|                     |                               | 102888 | 60011 | 27021597919961171 |
| J081931.24+213338.0 | MLS 151206:081931+213338      | 015054 | 59232 | 4546499229        |
|                     |                               | 101956 | 59913 | 27021598104043260 |
|                     |                               | 101946 | 59914 | 27021598104043260 |
| J082236.02+510524.4 | BH Lyn                        | 102905 | 59975 | 27021597917798186 |
| J082253.13+231300.6 | SDSS J082253.12+231300.6      | 015054 | 59232 | 4554489546        |
| J082603.71+113820.8 | CSS 110124:082604+113821      | 101992 | 59883 | 27021598103509778 |
| J082827.50-632958.8 | ASASSN-18aau                  | 027510 | 60002 | 27021599403239550 |
|                     |                               | 027510 | 60032 | 27021599403239550 |



| SDSS name           | Other name               | Field  | MJD   | Catalog ID        |
|---------------------|--------------------------|--------|-------|-------------------|
|                     |                          | 027510 | 59977 | 27021599403239550 |
|                     |                          | 027510 | 60034 | 27021599403239550 |
| J083619.15+212105.2 | CC Cnc                   | 015061 | 59226 | 4554852893        |
| J083642.66+532838.0 | SW UMa                   | 102904 | 59973 | 27021597917690874 |
|                     |                          | 102913 | 59973 | 27021597917690874 |
| J083821.98+483802.1 | EI UMa                   | 102890 | 59977 | 27021597919712335 |
| J084054.15+045518.4 |                          | 104393 | 59900 | 27021598102676247 |
| J084400.09+023919.2 | V495 Hya                 | 015143 | 59205 | 4545021122        |
|                     |                          | 015146 | 59206 | 4545021122        |
|                     |                          | 015146 | 59226 | 4545021122        |
|                     |                          | 015165 | 59202 | 4545021122        |
|                     |                          | 015258 | 59291 | 4545021122        |
| J084413.66-012808.0 | CSS 090331:084414-012807 | 015144 | 59222 | 4491926290        |
| J084555.07+033929.3 | V498 Hya                 | 015258 | 59291 | 4545200947        |
| J084708.28+011939.1 |                          | 015146 | 59226 | 6747473942        |
|                     |                          | 015146 | 59206 | 6747473942        |
|                     |                          | 015165 | 59202 | 6747473942        |
| J084735.40+014533.9 |                          | 015146 | 59226 | 6747618982        |
|                     |                          | 015146 | 59206 | 6747618982        |
|                     |                          | 015165 | 59202 | 6747618982        |
| J084740.11-474318.5 | GDS_J0847401-474318      | 025149 | 59982 | 27021599362308167 |
|                     |                          | 025149 | 59957 | 27021599362308167 |
| J085107.39+030834.6 | CT Hya                   | 015259 | 59292 | 4545208616        |
|                     |                          | 104405 | 59664 | 27021598102768361 |
| J085210.44+783246.7 |                          | 102172 | 59651 | 27021597911945951 |
|                     |                          | 102172 | 59653 | 27021597911945951 |
|                     |                          | 102172 | 59654 | 27021597911945951 |
| J085300.55+020424.2 | CSS 131207:085301+020425 | 104405 | 59664 | 27021600110830754 |
|                     |                          | 015165 | 59202 | 6747990436        |
| J085550.85-015428.6 |                          | 015166 | 59251 | 4492095625        |
| J085603.78+322109.1 | CSS 100508:085604+322109 | 018151 | 59604 | 27021598113212589 |
|                     |                          | 018151 | 59621 | 27021598113212589 |
| J085640.28-040439.7 | ASASSN-15ds              | 030743 | 60058 | 27021598049848372 |
|                     |                          | 030743 | 60026 | 27021598049848372 |
| J085909.20+053654.4 | RX J0859.1+0537          | 104406 | 59883 | 27021598103032049 |
| J090246.54-014201.9 | ASASSN-15gv              | 015168 | 59253 | 4570350599        |
| J090344.25-013326.1 |                          | 015168 | 59253 | 4570357060        |
| J090403.48+035501.1 |                          | 104406 | 59883 | 27021598149747578 |
|                     |                          | 015261 | 59306 | 4592577533        |
| J090756.67+715859.2 |                          | 103006 | 59657 | 27021597912176668 |
| J090947.82+110636.4 |                          | 102041 | 59912 | 27021598150551204 |
|                     |                          | 102041 | 59646 | 27021598150551204 |
| J091001.64+164820.0 |                          | 102025 | 60018 | 27021598150724950 |
| J091248.24-000721.3 |                          | 015156 | 59318 | 4570404979        |
| J091410.72+013732.9 | ASASSN-16as              | 015155 | 59256 | 4592552649        |
| J091453.59+113401.5 | CSS 081107:091454+113402 | 102041 | 59911 | 27021598150557208 |
|                     |                          | 102041 | 59912 | 27021598150557208 |
| J091551.64+090049.2 | GZ Cnc                   | 102045 | 59949 | 27021598150038545 |
| J091818.55+043610.0 |                          | 015263 | 59309 | 6872645243        |
|                     |                          | 015263 | 59315 | 6872645243        |
| J092042.64+001903.2 | CSS_J092042.6+001903     | 104395 | 59686 | 27021598149789122 |
| J092534.78+434917.3 | 2MASS J09253483+4349179  | 103065 | 60031 | 27021597920327394 |
| J092614.29+010557.4 |                          | 101297 | 59662 | 27021598149816047 |
|                     |                          | 015159 | 59232 | 4592646933        |
|                     |                          | 015268 | 59310 | 4592646933        |
| J092620.40+034542.0 | GUVV J092620.4+034541.8  | 101301 | 59937 | 27021598149870587 |
|                     |                          | 015265 | 59292 | 4592702225        |
| J092902.86+005334.0 |                          | 015268 | 59309 | 6872105161        |
| J093205.23+034332.4 | ASASSN-17od              | 015266 | 59306 | 4592709462        |
|                     |                          | 015266 | 59345 | 4592709462        |
|                     |                          | 015269 | 59280 | 4592709462        |

| SDSS name           | Other name                    | Field  | MJD   | Catalog ID        |
|---------------------|-------------------------------|--------|-------|-------------------|
|                     |                               | 015269 | 59318 | 4592709462        |
|                     |                               | 015269 | 59340 | 4592709462        |
| J093214.82+495054.6 | QS UMa                        | 103091 | 59978 | 27021597919793333 |
| J093238.20+010902.5 |                               | 015268 | 59310 | 4592920652        |
| J093836.99+071454.6 | HM Leo                        | 101291 | 60017 | 27021598150329308 |
|                     |                               | 101291 | 60023 | 27021598150329308 |
| J094431.71+035805.7 | VZ Sex                        | 101300 | 59665 | 27021598150172166 |
| J095312.66-042732.0 |                               | 024629 | 59993 | 27021599965544089 |
|                     |                               | 024629 | 59991 | 27021599965544089 |
| J100243.11-024636.0 |                               | 024633 | 59967 | 27021599988244380 |
| J100434.76+662914.9 | LN UMa                        | 102973 | 59686 | 27021597913981835 |
| J100515.36+191107.7 |                               | 101975 | 59672 | 27021598151136770 |
| J100700.72+673247.0 | CH UMa                        | 102986 | 59657 | 27021597913806128 |
| J102026.51+530432.9 | KS UMa                        | 103092 | 60033 | 27021597919022515 |
| J102215.84-035927.8 |                               | 024602 | 60002 | 27021598130857776 |
| J102320.27+440509.6 | NSV 4838                      | 103131 | 60064 | 27021597919572984 |
| J103317.24+072118.6 | CSS 080208:103317+072119      | 101240 | 60053 | 27021598151505693 |
|                     |                               | 101240 | 59690 | 27021598151505693 |
| J103352.90+584654.7 | DW UMa                        | 102929 | 59974 | 27021597918609354 |
| J104245.16+371819.9 |                               | 015291 | 59350 | 4597584648        |
| J104818.02+521829.3 | LY UMa                        | 103094 | 60033 | 27021597918791100 |
| J105656.94+494118.4 | CY UMa                        | 103110 | 60042 | 27021597919259145 |
| J105756.29+092315.0 | IU Leo                        | 101223 | 60031 | 27021598151638729 |
| J110425.55+450313.3 | AN UMa                        | 103135 | 60063 | 27021597919371447 |
| J112238.73-053949.4 | MASTER OT J112238.72-053950.1 | 026381 | 60077 | 27021598131626826 |
|                     |                               | 026381 | 60078 | 27021598131626826 |
|                     |                               | 026381 | 60080 | 27021598131626826 |
| J112332.02+431717.6 | CSS 090602:112332+431717      | 104638 | 59640 | 27021598154929169 |
|                     |                               | 015234 | 59252 | 4597890299        |
|                     |                               | 015234 | 59280 | 4597890299        |
|                     |                               | 015234 | 59309 | 4597890299        |
|                     |                               | 104638 | 59972 | 27021598154929169 |
|                     |                               | 104638 | 59641 | 27021598154929169 |
| J112555.65-001639.0 | 2QZ J112555.7-001639          | 101212 | 59676 | 27021598131744996 |
| J113122.38+432238.7 | MR UMa                        | 015234 | 59252 | 4597892495        |
|                     |                               | 015234 | 59280 | 4597892495        |
|                     |                               | 015234 | 59309 | 4597892495        |
|                     |                               | 015234 | 59337 | 4597892495        |
| J113542.62-581515.9 |                               | 026103 | 60097 | 27021599313834870 |
| J114338.55+714120.9 | DO Dra                        | 017017 | 59626 | 27021597913582088 |
|                     |                               | 100817 | 59981 | 27021597913582088 |
| J114521.19-042606.2 | TW Vir                        | 026378 | 60078 | 27021598131795219 |
|                     |                               | 026378 | 60083 | 27021598131795219 |
|                     |                               | 026378 | 60084 | 27021598131795219 |
| J115223.94-673828.2 | ASASSN-19ob                   | 027291 | 60100 | 27021599374523302 |
|                     |                               | 027291 | 60071 | 27021599374523302 |
| J115419.06+575750.8 |                               | 015236 | 59255 | 4359775558        |
|                     |                               | 015236 | 59290 | 4359775558        |
|                     |                               | 015236 | 59317 | 4359775558        |
|                     |                               | 015236 | 59351 | 4359775558        |
|                     |                               | 104632 | 60073 | 27021597918627636 |
|                     |                               | 104632 | 59644 | 27021597918627636 |
| J120619.85-032838.6 | CSS 120202:120620-032838      | 026981 | 59999 | 27021598145804010 |
|                     |                               | 026981 | 60000 | 27021598145804010 |
| J121005.31-025544.1 | 2QZ J121005.3-025543          | 026990 | 59992 | 27021598145814920 |
|                     |                               | 026990 | 59990 | 27021598145814920 |
| J121913.07+204937.2 |                               | 015295 | 59294 | 4599536987        |
|                     |                               | 015295 | 59318 | 4599536987        |
|                     |                               | 015295 | 59352 | 4599536987        |
| J122321.22-614758.1 |                               | 026065 | 60037 | 27021599057244080 |
|                     |                               | 026065 | 60008 | 27021599057244080 |

| SDSS name           | Other name               | Field  | MJD   | Catalog ID        |
|---------------------|--------------------------|--------|-------|-------------------|
| J122508.13-034721.0 | MLS 180415:122508-034721 | 027012 | 60001 | 27021598145798265 |
|                     |                          | 027012 | 60002 | 27021598145798265 |
| J122740.88+513924.8 |                          | 015237 | 59256 | 4351895227        |
|                     |                          | 015237 | 59291 | 4351895227        |
|                     |                          | 015237 | 59338 | 4351895227        |
|                     |                          | 015237 | 59370 | 4351895227        |
| J123813.51-033933.9 | V406 Vir                 | 027058 | 60023 | 27021598145950991 |
|                     |                          | 027058 | 60026 | 27021598145950991 |
|                     |                          | 027058 | 60027 | 27021598145950991 |
| J124100.45-593033.4 |                          | 028050 | 60078 | 27021599051261026 |
| J124426.25+613514.5 | V351 UMa                 | 100767 | 59986 | 27021597910317412 |
| J124823.06-040100.9 | MLS 140522:124823-040100 | 027095 | 60052 | 27021598145993998 |
|                     |                          | 027095 | 60057 | 27021598145993998 |
|                     |                          | 027095 | 60058 | 27021598145993998 |
|                     |                          | 027095 | 60059 | 27021598145993998 |
|                     |                          | 027095 | 60060 | 27021598145993998 |
|                     |                          | 027095 | 60053 | 27021598145993998 |
| J130030.27+115101.2 | CSS 080702:130030+115101 | 103317 | 59646 | 27021598156060425 |
| J130514.73+582856.2 |                          | 015198 | 59269 | 4351309920        |
|                     |                          | 015198 | 59273 | 4351309920        |
|                     |                          | 015348 | 59302 | 4351309920        |
|                     |                          | 015348 | 59329 | 4351309920        |
| J131042.66-042600.6 | CSS 120313:131043-042600 | 027161 | 60087 | 27021598146601205 |
|                     |                          | 027161 | 60086 | 27021598146601205 |
| J133200.79-045410.5 | DDE 139                  | 027685 | 60079 | 27021598146755506 |
|                     |                          | 027685 | 60089 | 27021598146755506 |
| J133309.18+143706.9 |                          | 015298 | 59292 | 4599897681        |
|                     |                          | 015298 | 59310 | 4599897681        |
|                     |                          | 015298 | 59351 | 4599897681        |
| J133941.06+484727.6 | V355 UMa                 | 015297 | 59291 | 4351662016        |
|                     |                          | 015297 | 59309 | 4351662016        |
|                     |                          | 015297 | 59347 | 4351662016        |
| J134052.05+151340.9 | CSS 100531:134052+151341 | 015298 | 59292 | 4599929199        |
|                     |                          | 015298 | 59310 | 4599929199        |
|                     |                          | 015298 | 59351 | 4599929199        |
| J134309.43+782312.7 | DDE 75                   | 100775 | 60037 | 27021597907634713 |
| J135218.95+280917.0 | CSS 090705:135219+280917 | 015301 | 59314 | 4603052231        |
|                     |                          | 015301 | 59338 | 4603052231        |
|                     |                          | 015301 | 59375 | 4603052231        |
| J135642.40+613024.4 | V427 UMa                 | 015303 | 59280 | 4349299466        |
|                     |                          | 015303 | 59309 | 4349299466        |
|                     |                          | 015303 | 59340 | 4349299466        |
|                     |                          | 015303 | 59381 | 4349299466        |
| J141436.78+162104.2 |                          | 101683 | 60016 | 27021598158287650 |
| J142833.38+003100.4 | 2QZ J142833.5+003100     | 102383 | 60050 | 27021598157695363 |
| J142953.55+073231.2 |                          | 015202 | 59250 | 4600955019        |
|                     |                          | 015202 | 59309 | 4600955019        |
|                     |                          | 015202 | 59324 | 4600955019        |
| J143317.77+101122.4 |                          | 015202 | 59250 | 4601012187        |
|                     |                          | 015202 | 59276 | 4601012187        |
|                     |                          | 015202 | 59309 | 4601012187        |
|                     |                          | 015202 | 59324 | 4601012187        |
| J143427.17-640303.1 |                          | 031425 | 60126 | 27021599195865692 |
| J143435.34+334050.2 |                          | 104536 | 60119 | 27021598160703560 |
|                     |                          | 015325 | 59347 | 4603792677        |
|                     |                          | 104536 | 60116 | 27021598160703560 |
| J143500.23-004606.5 | OU Vir                   | 102371 | 60051 | 27021598149510988 |
|                     |                          | 102371 | 60074 | 27021598149510988 |
|                     |                          | 102371 | 60076 | 27021598149510988 |
| J143558.50+033217.6 |                          | 102369 | 60061 | 27021600131348321 |
| J143947.62-010606.8 | LBQS 1437-0053           | 102371 | 60074 | 27021598149535306 |

| SDSS name           | Other name               | Field  | MJD   | Catalog ID        |
|---------------------|--------------------------|--------|-------|-------------------|
| J144609.22+013604.5 | ZTF J144609.22+013604.7  | 102357 | 60053 | 27021598157828048 |
|                     |                          | 102357 | 60057 | 27021598157828048 |
| J144659.96+025330.1 |                          | 102357 | 60053 | 27021598157870115 |
|                     |                          | 102357 | 60057 | 27021598157870115 |
| J145225.24-042931.9 |                          | 025333 | 60089 | 27021598149563966 |
| J150218.82+023055.2 |                          | 104547 | 59666 | 27021598726455776 |
| J150240.87+333423.4 | NZ Boo                   | 015271 | 59302 | 5188443683        |
|                     |                          | 015271 | 59361 | 5188443683        |
| J151400.10-650536.6 | EK TrA                   | 031436 | 60071 | 27021599217692647 |
|                     |                          | 031436 | 60100 | 27021599217692647 |
|                     |                          | 031436 | 60129 | 27021599217692647 |
| J151836.03-054803.6 | CSS 120330:151836-054803 | 025318 | 60088 | 27021598333055479 |
|                     |                          | 025318 | 60089 | 27021598333055479 |
| J152020.39-000948.3 |                          | 102321 | 60094 | 27021598333397076 |
| J152506.86-032655.4 | 1RXS J152506.9-032647    | 025313 | 60035 | 27021598333342324 |
|                     |                          | 025313 | 60052 | 27021598333342324 |
|                     |                          | 025313 | 60053 | 27021598333342324 |
|                     |                          | 025313 | 60054 | 27021598333342324 |
| J154336.53+751541.4 | GSC 04560-02157          | 100736 | 59712 | 27021597907393150 |
|                     |                          | 100736 | 59681 | 27021597907393150 |
|                     |                          | 100736 | 59680 | 27021597907393150 |
|                     |                          | 100736 | 59686 | 27021597907393150 |
| J154544.90+442829.9 | CSS 110428:154545+442830 | 101335 | 60106 | 27021597909012327 |
| J155331.03+551614.4 | MQ Dra                   | 101102 | 60065 | 27021597905600551 |
| J160450.19+414328.3 |                          | 101356 | 60114 | 27021597908906705 |
| J160501.32+203056.4 |                          | 102629 | 60106 | 27021598729065552 |
| J160525.27-381212.1 | ASASSN-21hc              | 024872 | 60113 | 27021598165899269 |
| J160809.53+542131.4 | ELAISN1 MOS15-02         | 104560 | 60052 | 27021597905481500 |
|                     |                          | 015329 | 59343 | 4346408603        |
|                     |                          | 015330 | 59324 | 4346408603        |
|                     |                          | 015330 | 59344 | 4346408603        |
| J160811.26-135058.2 | USNO-A2.0 0750-09453854  | 024648 | 60140 | 27021598332698583 |
| J161030.19+445900.8 |                          | 101357 | 60106 | 27021597905255254 |
| J161132.67+784319.4 |                          | 100746 | 59647 | 27021597907015183 |
| J161259.87-161715.6 | ZTF19aaqrldn             | 024665 | 60107 | 27021598332420922 |
| J161615.09-425825.4 | ASASSN-17fj              | 024920 | 60142 | 27021599059934773 |
| J161618.69+115104.6 | PNV J16161867+1151058    | 102623 | 60086 | 27021598730934595 |
| J161707.15-562720.0 | ASASSN-17db              | 031592 | 60033 | 27021599120201958 |
| J161817.28+030936.8 | BMAM-V636                | 102559 | 59678 | 27021598729267716 |
| J161853.17+070427.2 | PS15awk                  | 102581 | 60063 | 27021598730659289 |
| J161935.78+524631.7 | DDE 32                   | 015330 | 59324 | 4346373583        |
|                     |                          | 015330 | 59344 | 4346373583        |
| J161953.25+031908.8 | WFI J161953.3+031909     | 102559 | 59678 | 27021598729500022 |
| J162008.82+024414.6 |                          | 102559 | 59678 | 27021598729287104 |
| J162032.33-563519.8 | BESTII F19_123203        | 031592 | 60033 | 27021599121686765 |
| J162109.00-135307.6 | CSS 140211:162109-135307 | 024638 | 60142 | 27021598341837765 |
| J162433.30-293337.1 | ASASSN-14hd              | 024807 | 60124 | 27021598246871736 |
| J162501.76+390926.3 | V844 Her                 | 101382 | 60119 | 27021598748234535 |
| J162528.90-552003.6 | IK Nor                   | 031614 | 60049 | 27021599109591629 |
|                     |                          | 031614 | 60051 | 27021599109591629 |
| J162806.14+065315.3 | CSS 110611:162806+065316 | 102580 | 60061 | 27021598730755211 |
| J162830.61-571407.3 | Gaia17cus                | 031591 | 60036 | 27021599122881567 |
| J163120.88+103133.8 | CSS 080505:163121+103134 | 102606 | 60086 | 27021598730986846 |
| J163353.63-562759.2 | LR Nor                   | 031591 | 60036 | 27021599162531219 |
| J163447.70-345423.6 |                          | 024876 | 60157 | 27021598232228754 |
|                     |                          | 024876 | 60156 | 27021598232228754 |
| J163722.20-001957.1 | V2690 Oph                | 015275 | 59337 | 4863034442        |
|                     |                          | 015275 | 59367 | 4863034442        |
|                     |                          | 015275 | 59391 | 4863034442        |
|                     |                          | 102548 | 59671 | 27021598419826301 |
|                     |                          | 102548 | 59674 | 27021598419826301 |

| SDSS name           | Other name                    | Field  | MJD   | Catalog ID        |
|---------------------|-------------------------------|--------|-------|-------------------|
| J163805.39+083758.3 | V544 Her                      | 102591 | 60063 | 27021598731170690 |
| J164017.89+080823.0 | CSS 090711:164018+080823      | 102591 | 60063 | 27021598731116595 |
| J164204.25+151218.1 | CSS 170628:164204+151218      | 102634 | 60087 | 27021598739435105 |
| J164205.37-655335.8 | ASASSN-20gs                   | 031462 | 60030 | 27021599274190584 |
| J164248.50+134751.6 |                               | 102620 | 60086 | 27021598739376641 |
| J164449.42+195940.1 | V611 Her                      | 102651 | 60089 | 27021598740143506 |
| J164653.53+090726.1 | CSS 160705:164654+090726      | 102590 | 60061 | 27021598731214938 |
| J164654.82+135359.4 | DDE 152                       | 102620 | 60086 | 27021598739399786 |
| J164925.44+140243.3 | ASASSN-15jd                   | 102620 | 60086 | 27021598739409019 |
| J164950.38+035834.5 | CSS 100707:164950+035835      | 102566 | 60035 | 27021598730300828 |
| J165127.25-131809.2 | SSS 130510:165127-131809      | 015233 | 59275 | 4861314481        |
| J165141.45-490712.2 |                               | 025977 | 60083 | 27021599079487450 |
| J165242.98+703014.8 | PTFS1116cc                    | 101179 | 59744 | 27021597906308454 |
| J165244.82+333925.5 |                               | 015310 | 59315 | 5189686636        |
|                     |                               | 015310 | 59339 | 5189686636        |
|                     |                               | 015310 | 59347 | 5189686636        |
|                     |                               | 015310 | 59352 | 5189686636        |
|                     |                               | 015310 | 59375 | 5189686636        |
| J165859.91-512331.3 |                               | 025958 | 60079 | 27021599138492070 |
| J165930.37-125327.2 | V841 Oph                      | 103169 | 59986 | 27021598418256983 |
|                     |                               | 015233 | 59275 | 4861461131        |
| J170044.63-500505.3 | USNO-B1.0 0399-0591734        | 025968 | 60082 | 27021599137774000 |
| J170515.33+724403.3 | MASTER OT J170515.37+724402.5 | 015369 | 59335 | 4347265822        |
|                     |                               | 015369 | 59360 | 4347265822        |
| J170609.67+143451.6 | CSS 090205:170610+143452      | 102618 | 60119 | 27021598740513183 |
| J170655.18-150852.5 | ASASSN-15fe                   | 027622 | 60161 | 27021598389142723 |
|                     |                               | 027622 | 60162 | 27021598389142723 |
|                     |                               | 027613 | 60161 | 27021598389142723 |
| J171226.57-641656.8 |                               | 031497 | 60031 | 27021599279422759 |
| J171233.50-643342.6 | MASTER OT J171233.67-643342.6 | 031497 | 60031 | 27021599279571526 |
| J171247.71+604602.9 |                               | 101159 | 59806 | 27021597904563346 |
| J171658.14-313958.4 | ASASSN-21jw                   | 024842 | 60075 | 27021598269961876 |
|                     |                               | 024842 | 60076 | 27021598269961876 |
| J171752.03-070654.2 | MASTER OT J171752.02-070654.6 | 015340 | 59308 | 4866985473        |
| J171935.88-410053.6 | IGR J17195-4100               | 025929 | 60174 | 27021598200288479 |
| J171937.17+043123.3 | ASASSN-15kw                   | 102563 | 59820 | 27021598732904335 |
| J172021.48-150928.9 | ASASSN-18jc                   | 027641 | 60149 | 27021598391250534 |
| J172148.84-051713.3 | CSS 120611:172149-051713      | 015340 | 59308 | 4875329381        |
| J172256.18-261906.8 |                               | 024792 | 60180 | 27021598310687716 |
| J172515.56+073249.2 | CSS 100706:172516+073249      | 102574 | 60063 | 27021598736432660 |
| J172527.50-680822.4 | ASASSN-14is                   | 030413 | 60079 | 27021599281475783 |
|                     |                               | 030413 | 60080 | 27021599281475783 |
| J172733.67+130512.4 | CSS 090929:172734+130513      | 100087 | 60118 | 27021598737120439 |
| J172805.33+775117.3 |                               | 015370 | 59338 | 4347758086        |
|                     |                               | 015370 | 59363 | 4347758086        |
|                     |                               | 015370 | 59382 | 4347758086        |
| J172904.97-483742.0 |                               | 025950 | 60113 | 27021599148780010 |
| J172925.15-404335.8 | ASASSN-18hl                   | 025910 | 60178 | 27021598211591682 |
| J172959.01+522947.8 | MGAB-V705                     | 101141 | 60114 | 27021597903804760 |
| J173008.35+624754.4 |                               | 101188 | 59745 | 27021597904544927 |
|                     |                               | 101188 | 59715 | 27021597904544927 |
| J173021.89-055931.2 | V2731 Oph                     | 103211 | 59746 | 27021598432244667 |
| J173045.23-421143.3 | MM Sco                        | 025930 | 60169 | 27021598199945670 |
| J173408.80-430550.9 | ASASSN-18cs                   | 025911 | 60170 | 27021598202419829 |
| J173634.28-711258.6 | ASASSN-14dk                   | 030462 | 60107 | 27021599283243580 |
|                     |                               | 030462 | 60092 | 27021599283243580 |
| J173905.58-452714.5 | V728 Sco                      | 025913 | 60141 | 27021599144124665 |
| J173924.38+050049.7 | ASASSN-15mk                   | 015342 | 59328 | 5178467413        |
|                     |                               | 103184 | 59789 | 27021598735016593 |
| J174045.86+060350.1 | 4PBC J1740.7+0603             | 103184 | 59789 | 27021598735221261 |
|                     |                               | 015342 | 59328 | 5178672672        |

| SDSS name           | Other name                    | Field  | MJD   | Catalog ID        |
|---------------------|-------------------------------|--------|-------|-------------------|
| J174056.31+025831.5 | MG1 995493                    | 103193 | 59731 | 27021598733809394 |
|                     |                               | 015344 | 59302 | 5177258558        |
| J174155.61-620817.9 | MASTER OT J174155.54-620817.1 | 025834 | 60056 | 27021599176123896 |
| J174342.09-553005.7 | MASTER OT J174342.12-553006.3 | 025923 | 60089 | 27021599172676084 |
| J174345.53-725309.1 |                               | 030485 | 60106 | 27021599283723319 |
| J174714.34+150047.5 | CSS 080409:174714+150048      | 100085 | 60117 | 27021598741625707 |
| J174759.87+032859.6 | ASASSN-15fm                   | 015344 | 59302 | 5177926765        |
| J174907.74-621227.0 |                               | 025812 | 60056 | 27021599176343780 |
| J175505.10+132519.4 | ZTF18abdjpb0                  | 100084 | 60114 | 27021598738975158 |
|                     |                               | 100084 | 60113 | 27021598738975158 |
|                     |                               | 100084 | 60109 | 27021598738975158 |
| J175545.04-704634.3 | ASASSN-14fh                   | 030463 | 60167 | 27021599283383210 |
| J175622.38+025804.1 | DDE 155                       | 103195 | 59707 | 27021598734694448 |
| J175951.66-592000.2 | V437 Pav                      | 025856 | 60088 | 27021599175814873 |
| J175957.70+022144.5 | Gaia17bdz                     | 103195 | 59707 | 27021598734656568 |
| J180005.86+525632.7 | ASASSN-13ax                   | 101170 | 60108 | 27021597827075097 |
| J180035.52+081014.8 | V2301 Oph                     | 100033 | 60082 | 27021598762697711 |
| J180048.99+523234.5 | CSS 121025:180049+523235      | 101170 | 60108 | 27021597827071312 |
| J180245.76+100146.4 | ASASSN-17lh                   | 100068 | 60087 | 27021598763161255 |
| J180312.65+114154.5 | MASTER OT J180312.78+114154.7 | 100068 | 60087 | 27021598764985673 |
| J180324.99+114757.1 | V2104 Oph                     | 100068 | 60087 | 27021598764986270 |
| J180414.38+675412.5 | EX Dra                        | 101192 | 59956 | 27021597843534392 |
|                     |                               | 101192 | 60017 | 27021597843534392 |
|                     |                               | 101192 | 59957 | 27021597843534392 |
|                     |                               | 101192 | 59979 | 27021597843534392 |
| J180835.15+084829.1 | MGAB-V361                     | 100481 | 60065 | 27021598762970556 |
| J180835.86+101029.6 | V2779 Oph                     | 100481 | 60065 | 27021598763360095 |
| J180845.59+152101.1 | ASASSN-19wr                   | 100096 | 60121 | 27021598816134186 |
| J181033.82-534946.0 | ASASSN-15ia                   | 025919 | 60170 | 27021599431023889 |
| J181111.75+124301.7 |                               | 015346 | 59300 | 5209036455        |
|                     |                               | 015346 | 59307 | 5209036455        |
| J181244.08-592315.5 | AS Pav                        | 025855 | 60090 | 27021599432803220 |
| J181258.29+160247.1 | MASTER OT J181258.26+160246.8 | 100096 | 60121 | 27021598816359385 |
| J181407.30+113642.1 | V849 Oph                      | 100024 | 60086 | 27021598765226900 |
| J181429.83+612334.0 | HS 1813+6122                  | 101197 | 59738 | 27021597828699392 |
|                     |                               | 101197 | 59710 | 27021597828699392 |
| J181647.37+080014.9 | MGAB-V467                     | 100482 | 60064 | 27021598763648474 |
| J181738.37+042644.3 |                               | 100506 | 59709 | 27021598753751433 |
|                     |                               | 100506 | 59737 | 27021598753751433 |
| J181809.14-653136.0 | Gaia23apm                     | 025482 | 60109 | 27021599440116150 |
| J181810.72+050958.5 |                               | 100506 | 59737 | 27021598754048948 |
|                     |                               | 100506 | 59709 | 27021598754048948 |
| J181821.01+125350.2 | MGAB-V242                     | 100082 | 60089 | 27021598766229965 |
| J181904.82-744123.8 | Gaia16aoh                     | 030522 | 60174 | 27021599441573055 |
| J182122.52+614855.2 | ASASSN-13at                   | 015385 | 59359 | 4269312788        |
|                     |                               | 015385 | 59387 | 4269312788        |
|                     |                               | 015385 | 59366 | 4269312788        |
| J182134.65+020307.1 | ASASSN-15kd                   | 100521 | 59736 | 27021598751973250 |
| J182138.61+615904.0 | ASASSN-14gg                   | 015385 | 59359 | 4269327061        |
|                     |                               | 015385 | 59366 | 4269327061        |
|                     |                               | 015385 | 59387 | 4269327061        |
| J182205.84+270849.8 | MASTER OT J182205.85+270849.7 | 015331 | 59302 | 5342487136        |
|                     |                               | 015331 | 59328 | 5342487136        |
| J182313.80-604106.1 | Gaia19azx                     | 025831 | 60089 | 27021599433190563 |
| J182319.26+051857.1 | Gaia17cbl                     | 100506 | 59737 | 27021598754482424 |
|                     |                               | 100506 | 59709 | 27021598754482424 |
| J182643.55+613816.5 | MASTER OT J182643.42+613816.2 | 015385 | 59366 | 4269201343        |
|                     |                               | 015385 | 59387 | 4269201343        |
| J182707.63-520430.0 |                               | 106542 | 60193 | 63050396487016473 |
| J183014.15-671032.9 | ASASSN-17lw                   | 025503 | 60140 | 27021599440463127 |
| J183052.72+265514.8 | MGAB-V733                     | 015331 | 59302 | 5343123194        |



| SDSS name           | Other name                    | Field  | MJD   | Catalog ID        |
|---------------------|-------------------------------|--------|-------|-------------------|
| J183144.55+651130.2 | RX J1831.7+6511               | 101201 | 59711 | 27021597843259227 |
|                     |                               | 101201 | 59710 | 27021597843259227 |
| J183211.36+615505.9 | ASASSN-13ah                   | 015385 | 59359 | 4269213887        |
|                     |                               | 015385 | 59366 | 4269213887        |
|                     |                               | 015385 | 59387 | 4269213887        |
| J183228.19+101654.1 | MGAB-V1268                    | 100473 | 60109 | 27021598768356907 |
| J183442.34-514858.7 | ASASSN-21ij                   | 106519 | 60193 | 63050396487433207 |
| J183722.86-571407.2 | ASASSN-14jj                   | 025877 | 60141 | 27021599432406002 |
|                     |                               | 025899 | 60143 | 27021599432406002 |
| J183840.12+092222.5 | V651 Oph                      | 100484 | 60089 | 27021598768544248 |
| J184127.11+053821.9 | 2MASS J18412712+0538217       | 100496 | 59847 | 27021598760488882 |
|                     |                               | 100496 | 60127 | 27021598760488882 |
| J184658.80+553829.0 | MT Dra                        | 104529 | 60045 | 27021597827523704 |
| J185306.11-515722.1 | ASASSN-14fm                   | 025808 | 60165 | 27021599430206682 |
| J185333.52+223559.1 | Gaia17aqz                     | 100022 | 60128 | 27021598826491905 |
| J185720.40+713118.7 | V416 Dra                      | 101773 | 59737 | 27021597843634999 |
| J185721.58+131429.1 | V446 Her                      | 100466 | 60118 | 27021598801164061 |
| J190005.28-493034.6 | ASASSN-14fz                   | 025789 | 60168 | 27021599430418895 |
| J190121.32-622804.4 | ASASSN-15kt                   | 025467 | 60061 | 27021599435218720 |
| J190243.24-483406.0 | ASASSN-18ik                   | 025770 | 60170 | 27021599430394788 |
| J190342.14+534745.8 | ASASSN-15fv                   | 104532 | 60117 | 27021597827193697 |
| J190508.92-130608.6 |                               | 104193 | 60086 | 27021598685350132 |
|                     |                               | 104193 | 60087 | 27021598685350132 |
| J190531.87-534944.4 | ASASSN-22fs                   | 025830 | 60140 | 27021599434576354 |
| J190625.62-111156.8 |                               | 104193 | 60087 | 27021598686898259 |
| J190645.39-131314.2 |                               | 104193 | 60087 | 27021598685452604 |
|                     |                               | 104193 | 60086 | 27021598685452604 |
| J190651.05-114103.3 | Gaia21ban                     | 104193 | 60086 | 27021598686836248 |
|                     |                               | 104193 | 60087 | 27021598686836248 |
| J190706.25+690844.6 | EP Dra                        | 101787 | 59979 | 27021597843548805 |
|                     |                               | 101787 | 60035 | 27021597843548805 |
| J190708.20-123552.9 | ZTF18abdli fh                 | 104193 | 60087 | 27021598685731403 |
| J190732.76+525828.5 | CG Dra                        | 104532 | 60117 | 27021597827109781 |
| J190739.31-124117.5 | ZTFJ190739.31-124117.3        | 104193 | 60086 | 27021598685531157 |
| J190811.74-634331.2 | ASASSN-15mo                   | 025467 | 60061 | 27021599442262180 |
| J191306.79+013423.2 | V1419 Aql                     | 100526 | 59740 | 27021598779561106 |
| J191339.74-614257.0 | MASTER OT J191339.65-614257.6 | 025449 | 60079 | 27021599435388246 |
| J191343.58-141831.6 | MGAB-V390                     | 109975 | 60194 | 63050395562626130 |
| J191421.38-135026.9 | ZTF18abssftk                  | 109975 | 60194 | 63050395562678408 |
| J191534.92-620318.5 | MASTER OT J191535.00-620318.7 | 025468 | 60080 | 27021599435392152 |
| J191609.69-623551.7 | V344 Pav                      | 025468 | 60080 | 27021599442342676 |
| J191630.00-065204.4 |                               | 100547 | 59845 | 27021598694222622 |
| J191705.21-095144.8 |                               | 100534 | 60083 | 27021598693081401 |
| J191713.68+014321.7 | V356 Aql                      | 100526 | 59740 | 27021598781616730 |
| J192002.30-105446.5 | Gaia19fhp                     | 100534 | 60083 | 27021598688526500 |
| J192241.96+524359.0 | V1113 Cyg                     | 104524 | 60120 | 27021597824579927 |
| J192305.36+045719.7 | V1494 Aql                     | 100512 | 59794 | 27021598790841429 |
| J192321.24+022926.2 | V1370 Aql                     | 100527 | 59789 | 27021598788155977 |
| J192336.67-514444.0 | ASASSN-14ga                   | 025773 | 60148 | 27021599438057771 |
| J192444.60+041446.6 | V1229 Aql                     | 100512 | 59794 | 27021598790782524 |
| J192513.82-521137.3 | MASTER OT J192513.88-521137.6 | 025773 | 60148 | 27021599438067263 |
| J192554.81-461903.5 | Gaia16akr                     | 106383 | 60196 | 63050396489261267 |
| J192609.70+611312.7 | ZTF J192609.69+611312.7       | 101811 | 59829 | 27021597827853319 |
| J192610.82-101530.6 | DH Aql                        | 100534 | 60083 | 27021598695038681 |
| J192632.51-011612.0 | Gaia19eop                     | 100544 | 59736 | 27021598713279496 |
| J192634.45+073613.8 | V368 Aql                      | 100500 | 59846 | 27021598805423011 |
| J192710.18-484752.7 | ASASSN-14gq                   | 025740 | 60170 | 27021599436914051 |
| J192711.75+541750.4 | V2176 Cyg                     | 104523 | 60114 | 27021597824726647 |
| J192725.39+022303.3 | V1233 Aql                     | 100527 | 59789 | 27021598788336539 |
| J192739.29+020013.8 | MASTER OT J192739.31+020014.3 | 100527 | 59789 | 27021598788262895 |
| J192830.04-741053.1 | Gaia19efo                     | 030525 | 60141 | 27021599442179406 |



| SDSS name           | Other name                    | Field  | MJD   | Catalog ID        |
|---------------------|-------------------------------|--------|-------|-------------------|
| J192832.32-500134.9 | V379 Tel                      | 025741 | 60169 | 27021599437035859 |
| J192914.76+202759.5 | NQ Vul                        | 015334 | 59309 | 5299504775        |
| J192927.83+202035.0 | 1RXS J192926.6+202038         | 015334 | 59309 | 5299491324        |
| J192933.11-560343.0 |                               | 025407 | 60118 | 27021599438536411 |
| J193025.79-483052.4 |                               | 025727 | 60172 | 27021599436931962 |
| J193149.51+094939.4 | Gaia16asd                     | 100479 | 60094 | 27021598811144234 |
| J193244.66+003559.9 |                               | 100543 | 59737 | 27021598787799502 |
| J193423.17+020252.7 |                               | 100528 | 59789 | 27021598788873489 |
| J193430.49+020110.3 | ASASSN-19sg                   | 100528 | 59789 | 27021598788873416 |
| J193436.19+510742.1 | V2289 Cyg                     | 104513 | 60121 | 27021597824127944 |
| J193436.97+100213.3 | Gaia17cuh                     | 100479 | 60094 | 27021598813383471 |
| J193504.85-574934.9 |                               | 025420 | 60107 | 27021599438584134 |
| J193511.46-531745.8 | CRTS J193511.4-531746         | 025385 | 60142 | 27021599438232248 |
| J193628.84-551642.2 |                               | 025407 | 60118 | 27021599438259987 |
| J193709.85+023600.9 | V1141 Aql                     | 100528 | 59789 | 27021598789956242 |
| J193835.89-461257.8 | QS Tel                        | 025704 | 60178 | 27021599437590515 |
| J194124.99+152254.2 | 2MASS J19412506+1522553       | 100449 | 60123 | 27021598843153483 |
| J194139.92+214557.8 | FY Vul                        | 100127 | 59888 | 27021598862581317 |
| J194255.82-672725.6 | ASASSN-16ku                   | 025552 | 60108 | 27021599443117112 |
| J194309.99+093227.9 | ASASSN-15qv                   | 100490 | 60094 | 27021598810175811 |
| J194829.02-562939.5 | ASASSN-15in                   | 025421 | 60109 | 27021599438670413 |
| J194906.45+774423.1 | AB Dra                        | 101731 | 59893 | 27021597845383356 |
|                     |                               | 101731 | 59922 | 27021597845383356 |
|                     |                               | 101731 | 59894 | 27021597845383356 |
|                     |                               | 101731 | 59916 | 27021597845383356 |
|                     |                               | 101731 | 59834 | 27021597845383356 |
|                     |                               | 101731 | 59892 | 27021597845383356 |
|                     |                               | 101731 | 59895 | 27021597845383356 |
|                     |                               | 101731 | 59806 | 27021597845383356 |
| J194910.48+583159.4 | V542 Cyg                      | 101805 | 60089 | 27021597825631649 |
| J194947.62+031304.8 | MGAB-V300                     | 100463 | 59821 | 27021598865290249 |
|                     |                               | 100463 | 59840 | 27021598865290249 |
| J195039.55+055619.9 | ASASSN-15qr                   | 100457 | 60086 | 27021598865966628 |
| J195227.99+082846.9 | V500 Aql                      | 100966 | 60094 | 27021598868972983 |
| J195306.68+125900.8 | PQ Aql                        | 100961 | 60120 | 27021598876658238 |
| J195436.76+322155.1 | EY Cyg                        | 104415 | 59890 | 27021598943598337 |
| J195512.47+004536.3 | 2MASS J19551247+0045365       | 100980 | 59838 | 27021598864184655 |
| J195814.47+323241.9 | V2306 Cyg                     | 104415 | 59890 | 27021598944686851 |
| J195837.08+164128.4 | AW Sge                        | 015381 | 59391 | 5325695478        |
| J195938.44-551902.4 |                               | 025423 | 60149 | 27021599438904051 |
|                     |                               | 025423 | 60148 | 27021599438904051 |
| J195939.71+655440.9 |                               | 101789 | 59834 | 27021597842227530 |
|                     |                               | 101789 | 59832 | 27021597842227530 |
|                     |                               | 101789 | 59804 | 27021597842227530 |
| J200318.50+170251.5 | RZ Sge                        | 015381 | 59391 | 5326099056        |
| J200504.93+322122.5 | V550 Cyg                      | 015089 | 59391 | 5388888865        |
| J200512.34-561255.4 |                               | 025438 | 60139 | 27021599438931997 |
|                     |                               | 025438 | 60140 | 27021599438931997 |
| J200611.52+334237.5 | V1363 Cyg                     | 015089 | 59391 | 5398577299        |
| J200622.88+031935.3 | MASTER OT J200622.89+031935.3 | 100992 | 59762 | 27021598866414188 |
| J200703.00+051927.3 | MNIC V88                      | 100982 | 59794 | 27021598866807196 |
| J200729.55+625047.6 | ZTF J200729.55+625047.6       | 101800 | 59914 | 27021597833861929 |
| J200754.82+032738.0 | MGAB-V903                     | 100992 | 59762 | 27021598866434833 |
| J200934.41+550525.7 |                               | 015383 | 59363 | 4265451667        |
| J200946.47+042232.6 | USNO-B1.0 0943-0510775        | 100992 | 59762 | 27021598867479791 |
| J201116.80+600428.1 | Romanov V48                   | 101803 | 59838 | 27021597833533045 |
| J201135.94+025435.1 | MG1 1818424                   | 100992 | 59762 | 27021598867086181 |
| J201234.82-550304.4 |                               | 025424 | 60165 | 27021599439478314 |
|                     |                               | 025424 | 60167 | 27021599439478314 |
| J201403.80-540624.9 | SSS 110626:201404-540625      | 025424 | 60165 | 27021599439473042 |
|                     |                               | 025424 | 60167 | 27021599439473042 |

| SDSS name           | Other name                    | Field  | MJD   | Catalog ID        |
|---------------------|-------------------------------|--------|-------|-------------------|
| J201439.78-093715.2 | ASASSN-14hy                   | 104203 | 59847 | 27021598721166489 |
| J202206.39-565101.7 | ASASSN-14kx                   | 025456 | 60142 | 27021599439555821 |
|                     |                               | 025456 | 60143 | 27021599439555821 |
| J202300.38+063142.3 | LAMOST J202300.37+063142.4    | 101005 | 60118 | 27021598872663356 |
| J202310.39+643244.0 |                               | 101790 | 59805 | 27021597833920038 |
| J202422.01-083744.3 | ASASSN-16fk                   | 104206 | 60117 | 27021598721360324 |
| J202543.97-582334.2 | Gaia19cho                     | 025474 | 60120 | 27021599446521050 |
|                     |                               | 025474 | 60122 | 27021599446521050 |
| J202640.97+045901.2 | ZTF18abtvjuf                  | 101017 | 59844 | 27021598868032162 |
|                     |                               | 101017 | 59846 | 27021598868032162 |
| J202642.06-572154.5 | ASASSN-15en                   | 025474 | 60120 | 27021599439578419 |
|                     |                               | 025474 | 60122 | 27021599439578419 |
| J202812.47+414836.3 | V2467 Cyg                     | 015371 | 59367 | 4216010801        |
|                     |                               | 015371 | 59387 | 4216010801        |
| J202857.08-061803.5 | CSS 110621:202857-061803      | 101043 | 59844 | 27021598725007129 |
| J203134.50+030422.0 | MASTER OT J203134.48+030423.4 | 101031 | 59838 | 27021598874081514 |
| J203137.56-000512.2 | V1901 Aql                     | 101030 | 59741 | 27021598725900497 |
| J203256.81-565951.8 |                               | 025475 | 60140 | 27021599439592679 |
|                     |                               | 025475 | 60141 | 27021599439592679 |
| J203337.17-563345.4 | TT Ind                        | 025475 | 60140 | 27021599439619855 |
|                     |                               | 025475 | 60141 | 27021599439619855 |
| J203501.48-001946.3 | ZTF18abssrbs                  | 101030 | 59741 | 27021598725935846 |
| J203529.78+063652.7 | MASTER OT J203529.80+063652.8 | 101018 | 60120 | 27021598874928634 |
| J204247.17-604524.2 | SSS 110526:204247-604523      | 025534 | 60120 | 27021599446630801 |
| J204448.92-045928.9 | V485 Aqr                      | 101057 | 59847 | 27021598726075393 |
| J204522.73-011004.5 | CSS 110930:204523-011004      | 101059 | 59797 | 27021598726300998 |
| J204638.68+603802.9 | V713 Cep                      | 015384 | 59392 | 4273881073        |
| J204643.26-000630.2 |                               | 101059 | 59797 | 27021598726320259 |
| J204720.74+000007.8 |                               | 101059 | 59797 | 27021598874427854 |
| J204817.87-061045.3 |                               | 101068 | 59866 | 27021598725382763 |
| J204827.92+005008.9 |                               | 101060 | 59840 | 27021598874444975 |
| J205110.37+044842.1 | MASTER OT J205110.36+044842.2 | 101048 | 60118 | 27021598874726754 |
| J205212.78+441926.1 | V751 Cyg                      | 102435 | 59831 | 27021597780310749 |
|                     |                               | 102435 | 60128 | 27021597780310749 |
| J205227.38+034355.2 | MASTER OT J205227.38+034355.1 | 101061 | 59866 | 27021598874671550 |
| J205305.37+591732.2 | ASASSN-15rz                   | 101794 | 60115 | 27021597830238271 |
|                     |                               | 101794 | 60117 | 27021597830238271 |
| J205423.75+601706.8 | V962 Cep                      | 101794 | 60117 | 27021597830391881 |
|                     |                               | 101794 | 60115 | 27021597830391881 |
| J205705.32-072426.1 | Gaia17avi                     | 104220 | 59878 | 27021598725437550 |
| J205914.87-061220.6 | QT Aqr                        | 104220 | 59878 | 27021598725478960 |
| J205931.86-070516.9 |                               | 104220 | 59878 | 27021598725444309 |
| J210306.63+661032.5 | FX Cep                        | 101762 | 59763 | 27021597834457561 |
| J210404.68+463113.4 | V3101 Cyg                     | 102457 | 59890 | 27021597782056141 |
| J210720.93-022145.9 |                               | 101077 | 59845 | 27021597926204352 |
| J211312.23-590715.2 |                               | 025560 | 60167 | 27021599447392530 |
|                     |                               | 025560 | 60168 | 27021599447392530 |
|                     |                               | 025560 | 60169 | 27021599447392530 |
| J211508.00+015715.1 | ASASSN-14dg                   | 101073 | 59847 | 27021597934906880 |
| J211541.12-584054.6 | CD Ind                        | 025560 | 60167 | 27021599447399412 |
|                     |                               | 025560 | 60168 | 27021599447399412 |
|                     |                               | 025560 | 60169 | 27021599447399412 |
| J211936.94+033211.6 | CSS 150520:211937+033212      | 101066 | 59866 | 27021597935217675 |
| J212114.67-622749.7 |                               | 025605 | 60120 | 27021599447481200 |
|                     |                               | 025605 | 60122 | 27021599447481200 |
| J212521.76-102628.3 | CSS 080927:212522-102627      | 104221 | 60119 | 27021597925909873 |
| J212654.54-012054.3 | CRTS J212654.5-012054         | 015027 | 59159 | 4367796847        |
|                     |                               | 015027 | 59370 | 4367796847        |
|                     |                               | 104646 | 59844 | 27021597926521711 |
|                     |                               | 104646 | 59789 | 27021597926521711 |
|                     |                               | 104646 | 59793 | 27021597926521711 |

| SDSS name           | Other name                | Field  | MJD   | Catalog ID        |
|---------------------|---------------------------|--------|-------|-------------------|
| J213024.64-025917.7 | VZ Aqr                    | 103582 | 59873 | 27021597926423754 |
| J213343.63+510724.6 | 1RXS J213344.1+510725     | 101718 | 59888 | 27021597798184034 |
| J213432.34-012040.5 | CSS 081120:213432-012040  | 015064 | 59375 | 4368348605        |
| J213559.33+052700.6 | HS 2133+0513              | 101042 | 59882 | 27021597936115639 |
| J214804.43+080950.3 | CSS 080505:214804+080951  | 103529 | 60123 | 27021597936536466 |
| J215637.24-632655.5 | SSS 101124:215637-632655  | 025611 | 60119 | 27021599447608103 |
|                     |                           | 025611 | 60124 | 27021599447608103 |
| J220542.33+033917.1 | ASASSN-17jb               | 103532 | 59899 | 27021597936367269 |
| J220630.83-524419.8 | DDE 99                    | 027764 | 60100 | 27021599452528485 |
| J220807.49+021618.8 | HS 2205+0201              | 103532 | 59899 | 27021597936292061 |
| J221541.08+553701.3 | CP Lac                    | 101701 | 59913 | 27021597805534918 |
| J221552.06-613545.1 |                           | 025569 | 60177 | 27021599448686856 |
|                     |                           | 025569 | 60179 | 27021599448686856 |
| J221832.75+192520.2 | Swift J2218.5+1925        | 015030 | 59376 | 4383253183        |
| J221900.24+201831.2 |                           | 015030 | 59376 | 4383285955        |
| J222117.33+194817.6 |                           | 015030 | 59376 | 4383272764        |
| J224813.46+640023.1 |                           | 101716 | 59898 | 27021597836078496 |
| J225040.37+632837.3 | GD 552                    | 101717 | 59902 | 27021597835858639 |
| J225608.49+595430.2 | 2MASS J22560844+5954299   | 101690 | 59865 | 27021597813952034 |
| J230346.67+531714.9 | V425 Cas                  | 100602 | 59925 | 27021597808350943 |
| J230538.41+652158.8 | IPHAS J230538.39+652158.7 | 101707 | 59901 | 27021597837629582 |
| J233737.44-604358.2 | Gaia21ebk                 | 028901 | 60180 | 27021599452945406 |
| J234440.54-001206.1 | MLS 100904:234441-001206  | 015034 | 59165 | 4371155462        |
|                     |                           | 015034 | 59192 | 4371155462        |
| J234955.19-605417.1 | ASASSN-14hl               | 028902 | 60180 | 27021599452955982 |

## 6 CVS OMITTED FROM THE TRAINING/TEST DATASET

Table 3: Spectra omitted from the training/test dataset.

| Spectrum file name               | SDSS name               | Reason for exclusion   |
|----------------------------------|-------------------------|------------------------|
| spec-05985-56089-0232.fits       | SDSSJ123931.99+210806.2 | Not like a CV          |
| spec-03674-55182-0714.fits       | SDSSJ074716.80+424849.0 | Novalike               |
| spec-15384-59392-4271017394.fits | SDSSJ205423.76+601706.7 | Poor quality           |
| spec-01401-53144-0443.fits       | SDSSJ153213.68+370104.9 | Novalike               |
| spec-15115-59210-4523820411.fits | SDSSJ063047.05+023931.2 | Poor quality           |
| spec-01274-52995-0505.fits       | SDSSJ092638.71+362402.4 | He absorption/emission |
| spec-15233-59275-4861314481.fits | SDSSJ165127.25-131809.2 | Poor quality           |
| spec-15075-59187-4417020320.fits | SDSSJ052859.54-033352.4 | Poor quality           |
| spec-15385-59359-4269201343.fits | SDSSJ182643.55+613816.5 | Poor quality           |
| spec-01909-53261-0601.fits       | SDSSJ204827.91+005008.9 | Humps                  |
| spec-15224-59238-4337185134.fits | SDSSJ044321.37+472125.8 | Nova                   |
| spec-02252-53565-0239.fits       | SDSSJ224303.83+221456.0 | Novalike               |
| spec-05487-55982-0180.fits       | SDSSJ151415.61+074445.9 | No reason              |
| spec-06700-56384-0434.fits       | SDSSJ105656.97+494118.4 | Poor quality           |
| spec-02578-54093-0620.fits       | SDSSJ093220.93+133122.3 | Novalike               |
| spec-02062-53381-0022.fits       | SDSSJ012940.05+384210.4 | He absorption/emission |
| spec-00336-51999-0358.fits       | SDSSJ124058.03-015919.2 | He absorption/emission |
| spec-15228-59242-4535621315.fits | SDSSJ062724.39+161329.6 | High Mass donor        |
| spec-02434-53826-0400.fits       | SDSSJ090113.51+144704.7 | Novalike               |
| spec-04686-56013-0580.fits       | SDSSJ111544.51+425822.4 | Humps                  |
| spec-10736-58274-0986.fits       | SDSSJ155538.13+380250.6 | Humps                  |
| spec-15233-59275-4861461131.fits | SDSSJ165930.37-125327.2 | Nova                   |
| spec-07859-57282-0723.fits       | SDSSJ010844.13+022638.9 | Humps                  |
| spec-06586-56485-0020.fits       | SDSSJ223606.51+291600.0 | Humps                  |
| spec-00861-52318-0352.fits       | SDSSJ080846.19+313106.0 | Outburst               |
| spec-00518-52282-0285.fits       | SDSSJ121209.31+013627.7 | Zeeman splitting       |
| spec-01721-53857-0021.fits       | SDSSJ152613.96+081802.3 | Outburst               |
| spec-15229-59303-4537522851.fits | SDSSJ063844.17+181611.5 | Outburst               |
| spec-04012-55327-0578.fits       | SDSSJ152020.40-000948.3 | Novalike               |
| spec-15005-59167-4399288456.fits | SDSSJ003941.08+005427.5 | Poor quality           |
| spec-15383-59363-4265451667.fits | SDSSJ200934.41+550525.6 | Novalike               |
| spec-08177-57374-0696.fits       | SDSSJ111126.83+571239.0 | Outburst               |
| spec-01187-52708-0099.fits       | SDSSJ084054.15+045519.2 | Novalike               |
| spec-02212-53789-0201.fits       | SDSSJ110539.77+250628.6 | Humps                  |
| spec-01192-52649-0543.fits       | SDSSJ090628.25+052656.9 | Outburst               |
| spec-15298-59292-4599929199.fits | SDSSJ134052.04+151340.9 | Outburst               |
| spec-02919-54537-0415.fits       | SDSSJ120615.74+510047.1 | Humps                  |
| spec-15073-59186-4542234653.fits | SDSSJ074222.55+172806.7 | No reason              |
| spec-15054-59232-4554489546.fits | SDSSJ082253.13+231300.6 | Poor quality           |
| spec-00732-52221-0589.fits       | SDSSJ214354.60+124457.9 | Not like a CV          |
| spec-01234-52724-0304.fits       | SDSSJ093946.04+065209.5 | Outburst               |
| spec-15112-59211-4513598719.fits | SDSSJ052834.08+331821.7 | Nova                   |
| spec-05293-55953-0322.fits       | SDSSJ085521.18+111815.3 | Outburst               |
| spec-00527-52342-0323.fits       | SDSSJ132411.57+032050.5 | Poor quality           |
| spec-02798-54397-0340.fits       | SDSSJ183131.64+420220.3 | He absorption/emission |
| spec-15018-59164-4551693466.fits | SDSSJ074419.74+325448.2 | Poor quality           |
| spec-02533-54585-0156.fits       | SDSSJ163545.72+112458.1 | Not like a CV          |
| spec-15197-59245-4552297765.fits | SDSSJ062406.13+400743.8 | Novalike               |
| spec-00619-52056-0437.fits       | SDSSJ155331.12+551614.5 | Humps                  |
| spec-06621-56366-0467.fits       | SDSSJ130147.98+434549.4 | Humps                  |
| spec-01689-53177-0342.fits       | SDSSJ170244.09+223547.9 | Novalike               |
| spec-02888-54529-0252.fits       | SDSSJ085300.56+020424.8 | Poor quality           |
| spec-01852-53534-0153.fits       | SDSSJ161012.53+222110.9 | Novalike               |
| spec-07914-57331-0531.fits       | SDSSJ011331.69-033233.6 | Humps                  |

Continued on next page

Table 3: Spectra omitted from the training/test dataset.

| Spectrum file name               | SDSS name               | Reason for exclusion |
|----------------------------------|-------------------------|----------------------|
| spec-15279-59302-4471416011.fits | SDSSJ062953.89-033508.4 | Poor quality         |
| spec-02382-54169-0502.fits       | SDSSJ092809.84+071130.6 | Not like a CV        |
| spec-01064-52577-0459.fits       | SDSSJ032651.73+011513.3 | Poor quality         |
| spec-15064-59375-4368348605.fits | SDSSJ213432.34-012040.5 | Outburst             |
| spec-02359-53800-0051.fits       | SDSSJ105905.07+272755.5 | Humps                |
| spec-01770-53171-0530.fits       | SDSSJ125044.43+154957.4 | Zeeman splitting     |

**Table 4.** Objects, previously classified as CVs, that are no longer regarded as CVs based on new evidence.

| SDSS name               | Notes                                                                                                                                                                                                                                                                                                                                                                                                                                   |
|-------------------------|-----------------------------------------------------------------------------------------------------------------------------------------------------------------------------------------------------------------------------------------------------------------------------------------------------------------------------------------------------------------------------------------------------------------------------------------|
| SDSSJ064939.16-060005.0 | <a href="#">Kabath et al. (2009)</a> categorise this object ( BEST-II Ira2b_01098) as either a cepheid or a CV. The spectrum has a strong red continuum consistent with a star and there is no evidence of emission lines. It is above the main sequence in the HR diagram.                                                                                                                                                             |
| SDSSJ021229.78+570519.4 | This is UW Per which has been reported as a U Gem by VSX but this classification was challenged by ( <a href="#">Mobberley et al. 1997</a> ) . Our spectrum is consistent with a single star. It is above the main sequence in the HR diagram.                                                                                                                                                                                          |
| SDSSJ162450.04+654101.1 | This is Gaia16aat which was reported as a candidate CV by <i>Gaia</i> Alerts based upon being a blue star with a long-term brightening. The spectrum shows two humps typical of an extra-galactic source.                                                                                                                                                                                                                               |
| SDSSJ201649.48+382109.3 | This is V1377 Cyg. It has been reported as a candidate U Gem by VSX with a period of 17 d. Our spectrum shows a red continuum with emission lines. The object is above the main sequence in the HR diagram.                                                                                                                                                                                                                             |
| SDSSJ061043.98+251031.0 | This is NSV 2853 and is classified as a candidate CV on VSX. There are no emission lines visible in our spectrum. <a href="#">Liu &amp; Hu (2000)</a> confirmed that this is a G-type star which is consistent with its position on the main sequence in the HR diagram.                                                                                                                                                                |
| SDSSJ082253.13+231300.6 | Our spectrum shows a red donor with no obvious emission lines. It is on the main sequence. <a href="#">Szkody et al. (2009)</a> categorised this as a CV based upon an H $\alpha$ emission line with no other Balmer emission lines visible. This is more probably a flaring M-dwarf.                                                                                                                                                   |
| SDSSJ080826.00+314125.3 | <a href="#">Balanutsa et al. (2015b)</a> classified this as a CV based upon a transient detection. The spectrum shows the clear characteristics of an extra-galactic source.                                                                                                                                                                                                                                                            |
| SDSSJ165449.45+350803.7 | This has been classified by CRTS as a candidate CV based upon a transient. The spectrum shows the clear characteristics of an extra-galactic source.                                                                                                                                                                                                                                                                                    |
| SDSSJ074813.35+290512.0 | This is V0434 Gem. <a href="#">Samus' et al. (2017)</a> classify this as a novalike. Our spectrum shows the signature of a late M-dwarf which is consistent with the position on the HR diagram.                                                                                                                                                                                                                                        |
| SDSSJ213432.34-012040.5 | This is CSS 081120:213432-012040 and it was classified as a CV by CRTS based upon detection of a transient. Our spectrum shows a blue continuum typical of a white dwarf with no emission lines. The synthetic magnitude is 19.4 which is dimmer than the <i>Gaia</i> G-band magnitude of 18.8 and so this is not a CV in outburst. <a href="#">Coppejans et al. (2016)</a> concluded that this is not a CV                             |
| SDSSJ132444.33-142335.7 | This is Gaia17aoi. <a href="#">Delgado et al. (2017c)</a> reported a single transient of $\Delta m \approx 1$ . Our spectrum is typical of a white dwarf which is consistent with the position on the white dwarf cooling sequence in the HR diagram. There are no emission lines. This is probably a white dwarf and the transient had some other origin.                                                                              |
| SDSSJ012156.25+143737.2 | This object was classified as a candidate CV based upon a CRTS transient. Our spectrum is clearly that of an extra-galactic source.                                                                                                                                                                                                                                                                                                     |
| SDSSJ121929.32+471522.9 | <a href="#">Szkody et al. (2006)</a> classified this object as a novalike based upon a blue continuum and a small H $\alpha$ emission line. Our spectrum also shows an H $\alpha$ emission line offset from its rest frequency together with two broad emission humps reminiscent of a magnetic white dwarf ( <a href="#">Gänsicke et al. 2020</a> ). ( <a href="#">Pala et al. 2020</a> ) concluded that this is a single white dwarf. |

## 7 MIS-CATEGORISED CVS

The classification of a number of systems that were previously classified as CVs have now, with the benefit of new data from sources including *Gaia* and ZTF, been revised. The new classifications of these non-CV systems are discussed in Table 4.

## REFERENCES

- Adams W. S., Burwell C. G., 1920, *ApJ*, **51**, 121
- Ahnert P., Hoffmeister C., 1941, *Kleine Veroeffentlichungen der Universitaetssternwarte zu Berlin Babelsberg*, **7**, 4.1
- Antipin S. V., 1996, *Information Bulletin on Variable Stars*, **4360**, 1
- Antipin S. V., Kroll P., 2003, *Information Bulletin on Variable Stars*, **5461**, 1
- Araujo-Betancor S., Gänsicke B. T., Hagen H. J., Rodriguez-Gil P., Engels D., 2003a, *A&A*, **406**, 213
- Araujo-Betancor S., et al., 2003b, *ApJ*, **583**, 437
- Arjyotha S., Aungwerojwit A., Gänsicke B. T., Marsh T., Rodríguez-Gil P. R., 2009, in Murphy S. J., Bessell M. S., eds, *Astronomical Society of the Pacific Conference Series Vol. 404, The Eighth Pacific Rim Conference on Stellar Astrophysics: A Tribute to Kam-Ching Leung*. p. 272
- Ashok N. M., Banerjee D. P. K., Venkataraman V., Joshi V., 2014, *The Astronomer's Telegram*, **5996**, 1
- Augusteijn T., Tappert C., Dall T., Maza J., 2010, *MNRAS*, **405**, 621
- Aungwerojwit A., et al., 2006, *A&A*, **455**, 659
- Bailer-Jones C. A. L., Rybizki J., Founesneau M., Demleitner M., Andrae R., 2021, *AJ*, **161**, 147
- Balanutsa P., et al., 2012, *The Astronomer's Telegram*, **4458**, 1
- Balanutsa P., et al., 2013, *The Astronomer's Telegram*, **5676**, 1
- Balanutsa P., et al., 2015a, *The Astronomer's Telegram*, **8276**, 1
- Balanutsa P., et al., 2015b, *The Astronomer's Telegram*, **8426**, 1
- Balanutsa P., et al., 2016a, *The Astronomer's Telegram*, **8758**, 1
- Balanutsa P., et al., 2016b, *The Astronomer's Telegram*, **8941**, 1
- Balanutsa P., et al., 2016c, *The Astronomer's Telegram*, **9729**, 1
- Balanutsa P., et al., 2017a, *The Astronomer's Telegram*, **10353**, 1
- Balanutsa P., et al., 2017b, *The Astronomer's Telegram*, **10564**, 1
- Bao Supernova Survey Esamdin A., Dong X., Zhao Y., 1997, *IAU Circ.*, **6763**, 2
- Barwig H., Ritter H., Fiedler H., 1993, in *Astronomische Gesellschaft Abstract Series*. p. 35
- Barwig H., Ritter H., Barnbantner O., 1994, *A&A*, **288**, 204
- Bateson F. M., 1972, *Information Bulletin on Variable Stars*, **678**, 2
- Bateson F. M., 1982, *Royal Astronomical Society of New Zealand Publications of Variable Star Section*, **10**, 12
- Bateson F. M., McIntosh R., 1997, *Royal Astronomical Society of New Zealand Publications of Variable Star Section*, **22**, 22
- Bateson F., McIntosh R., Stubbings R., 1997, *Royal Astronomical Society of New Zealand Publications of Variable Star Section*, **22**, 44
- Berg C., Wegner G., Foltz C. B., Chaffee Frederic H. J., Hewett P. C., 1992, *ApJS*, **78**, 409
- Beuermann K., Thomas H. C., Reinsch K., Schwöpe A. D., Trümper J., Voges W., 1999, *A&A*, **347**, 47
- Bonnet-Bidaud J. M., de Martino D., Falanga M., Mouchet M., Masetti N., 2007, *A&A*, **473**, 185
- Boyd D., Denisenko D., Koff R., Miller I., Staels B., 2011, *Journal of the British Astronomical Association*, **121**, 233
- Breedt E., et al., 2014, *MNRAS*, **443**, 3174
- Brimacombe J., et al., 2014, *The Astronomer's Telegram*, **6768**, 1
- Bruch A., 1989, *A&AS*, **78**, 145
- Bruch A., 2023, *MNRAS*, **519**, 352
- Bruch A., Schimpke T., 1992, *A&AS*, **93**, 419
- Bruch A., Fischer F. J., Wilmsen U., 1987, *A&AS*, **70**, 481
- Bruch A., Schimpke T., Kochsiek A., 1997, *A&A*, **325**, 601
- Buckley D. A., et al., 1993, *MNRAS*, **262**, 93
- Campbell R. D., Shafter A. W., 1995, *ApJ*, **440**, 336
- Carbon D. F., Henze C., Nelson B. C., 2017, *ApJS*, **228**, 19
- Carter P. J., et al., 2013, *MNRAS*, **429**, 2143
- Ceraski W., 1908, *Astronomische Nachrichten*, **177**, 173
- Chen A., O'Donoghue D., Stobie R. S., Kilkeny D., Warner B., 2001, *MNRAS*, **325**, 89
- Chen X., Wang S., Deng L., de Grijs R., Yang M., Tian H., 2020, *ApJS*, **249**, 18
- Cheung C. C., Shore S. N., De Gennaro Aquino I., Charbonnel S., Edlin J., Hays E., Corbet R. H. D., Wood D. L., 2012, *The Astronomer's Telegram*, **4310**, 1
- Ciatti F., Rosino L., 1974, *A&AS*, **16**, 305
- Coppejans D. L., K rding E. G., Knigge C., Pretorius M. L., Woudt P. A., Groot P. J., Van Eck C. L., Drake A. J., 2016, *MNRAS*, **456**, 4441
- Cordonni J. P., Gleizes F., Jasiewicz G., 1977, *A&A*, **55**, 307
- Cragg T. A., 1960, *PASP*, **72**, 475
- Croom S. M., Smith R. J., Boyle B. J., Shanks T., Loaring N. S., Miller L., Lewis I. J., 2001, *MNRAS*, **322**, L29
- Croom S. M., Smith R. J., Boyle B. J., Shanks T., Miller L., Outram P. J., Loaring N. S., 2004, *MNRAS*, **349**, 1397
- Dai Z., Szkody P., Taani A., Garnavich P. M., Kennedy M., 2017, *A&A*, **606**, A45
- Delgado A., Harrison D., Hodgkin S., Leeuwen M. V., Rixon G., Yoldas A., 2016, *Transient Name Server Discovery Report*, **2016-481**, 1
- Delgado A., Harrison D., Hodgkin S., Leeuwen M. V., Rixon G., Yoldas A., 2017a, *Transient Name Server Discovery Report*, **2017-1223**, 1
- Delgado A., Harrison D., Hodgkin S., Leeuwen M. V., Rixon G., Yoldas A., 2017b, *Transient Name Server Discovery Report*, **2017-1230**, 1
- Delgado A., Harrison D., Hodgkin S., Leeuwen M. V., Rixon G., Yoldas A., 2017c, *Transient Name Server Discovery Report*, **2017-266**, 1
- Delgado A., Harrison D., Hodgkin S., Leeuwen M. V., Rixon G., Yoldas A., 2017d, *Transient Name Server Discovery Report*, **2017-312**, 1
- Delgado A., Harrison D., Hodgkin S., Leeuwen M. V., Rixon G., Yoldas A., 2017e, *Transient Name Server Discovery Report*, **2017-379**, 1
- Delgado A., Harrison D., Hodgkin S., Leeuwen M. V., Rixon G., Yoldas A., 2017f, *Transient Name Server Discovery Report*, **2017-524**, 1
- Delgado A., Harrison D., Hodgkin S., Leeuwen M. V., Rixon G., Yoldas A., 2017g, *Transient Name Server Discovery Report*, **2017-547**, 1
- Delgado A., Harrison D., Hodgkin S., Leeuwen M. V., Rixon G., Yoldas A., 2017h, *Transient Name Server Discovery Report*, **2017-873**, 1
- Delgado A., Harrison D., Hodgkin S., Leeuwen M. V., Rixon G., Yoldas A., 2017i, *Transient Name Server Discovery Report*, **2017-925**, 1
- Delgado A., Harrison D., Hodgkin S., Leeuwen M. V., Rixon G., Yoldas A., 2017j, *Transient Name Server Discovery Report*, **2017-933**, 1
- Delgado A., Harrison D., Hodgkin S., Leeuwen M. V., Rixon G., Yoldas A., 2018a, *Transient Name Server Discovery Report*, **2018-1291**, 1



- Delgado A., Harrison D., Hodgkin S., Leeuwen M. V., Rixon G., Yoldas A., 2018b, Transient Name Server Discovery Report, [2018-1819](#), 1
- Delgado A., Harrison D., Hodgkin S., Leeuwen M. V., Rixon G., Yoldas A., 2019a, Transient Name Server Discovery Report, [2019-1009](#), 1
- Delgado A., Harrison D., Hodgkin S., Leeuwen M. V., Rixon G., Yoldas A., 2019b, Transient Name Server Discovery Report, [2019-241](#), 1
- Delgado A., Harrison D., Hodgkin S., Leeuwen M. V., Rixon G., Yoldas A., 2019c, Transient Name Server Discovery Report, [2019-400](#), 1
- Delgado A., Harrison D., Hodgkin S., Leeuwen M. V., Rixon G., Yoldas A., 2019d, Transient Name Server Discovery Report, [2019-420](#), 1
- Denisenko D. V., Martinelli F., 2016, [arXiv e-prints](#), p. [arXiv:1609.08511](#)
- Denisenko D. V., Sokolovsky K. V., 2011, *Astronomy Letters*, **37**, 91
- Denisenko D. V., Kryachko T. V., Satovskiy B. L., 2008, The Astronomer's Telegram, [1640](#), 1
- Denisenko D., et al., 2012, The Astronomer's Telegram, [4441](#), 1
- Denisenko D., et al., 2014, The Astronomer's Telegram, [6049](#), 1
- Dillon M., et al., 2008, *MNRAS*, **386**, 1568
- Downes R. A., Shara M. M., 1993, *PASP*, **105**, 127
- Downes R., Hoard D. W., Szkody P., Wachter S., 1995, *AJ*, **110**, 1824
- Downes R., Webbink R. F., Shara M. M., 1997, *PASP*, **109**, 345
- Downes R. A., Webbink R. F., Shara M. M., Ritter H., Kolb U., Duerbeck H. W., 2001, *PASP*, **113**, 764
- Downes R. A., Webbink R. F., Shara M. M., Ritter H., Kolb U., Duerbeck H. W., 2005, *Journal of Astronomical Data*, **11**, 2
- Drake A. J., Mahabal A., Djorgovski S. G., Graham M. J., Williams R., Beshore E. C., Larson S. M., Christensen E., 2008, The Astronomer's Telegram, [1479](#), 1
- Drake A. J., et al., 2009a, *ApJ*, **696**, 870
- Drake A. J., et al., 2009b, The Astronomer's Telegram, [2266](#), 1
- Drake A. J., et al., 2014a, *ApJS*, **213**, 9
- Drake A. J., et al., 2014b, *MNRAS*, **441**, 1186
- Duerbeck H. W., 1987, *Space Sci. Rev.*, **45**, 1
- Dunér Hartwig Müller 1911, *Astronomische Nachrichten*, **190**, 57
- Echevarría J., Michel R., Costero R., Zharikov S., 2007, *A&A*, **462**, 1069
- Fiedler H., Barwig H., Mantel K. H., 1997, *A&A*, **327**, 173
- Förster F., et al., 2021, *AJ*, **161**, 242
- Fremling C., Blagorodnova N., Kupfer T., Neill J. D., Walters R., Cannella C. B., Kulkarni S. R., 2018, The Astronomer's Telegram, [11512](#), 1
- Fruth T., et al., 2013, *AJ*, **146**, 136
- Fuentes-Morales I., Tappert C., Zorotovic M., Vogt N., Puebla E. C., Schreiber M. R., Ederoclite A., Schmidtobreick L., 2021, *MNRAS*, **501**, 6083
- Gabdeev M. M., Borisov N. V., Shimansky V. V., Spiridonova O. I., 2015, *Astronomy Reports*, **59**, 213
- Gabdeev M. M., Shimansky V. V., Borisov N. V., Bikmaev I. F., Moskvitin A. S., Kolbin A. I., 2019, *Astrophysical Bulletin*, **74**, 308
- Gänsicke B. T., et al., 2005, *MNRAS*, **361**, 141
- Gänsicke B. T., et al., 2006, *MNRAS*, **365**, 969
- Gänsicke B. T., et al., 2009, *MNRAS*, **397**, 2170
- Gänsicke B. T., Rodríguez-Gil P., Gentile Fusillo N. P., Inight K., Schreiber M. R., Pala A. F., Tremblay P.-E., 2020, *MNRAS*, **499**, 2564
- Garnavich P., Deal S., 2013, The Astronomer's Telegram, [5178](#), 1
- Geisel S. L., Kleinmann D. E., Low F. J., 1970, *ApJ*, **161**, L101
- Gessner H., Meinunger I., 1974, *Veroeffentlichungen der Sternwarte Sonneberg*, **5**, 249
- Gezari S., et al., 2013, *ApJ*, **766**, 60
- Goetz W., Wenzel W., 1956, *Veroeffentlichungen der Sternwarte Sonneberg*, **2**, 279
- Goranskij V. P., 1972, *Peremennye Zvezdy Prilozhenie*, **1**, 304
- Greaves J., 2006, *Open European Journal on Variable Stars*, **37**, 1
- Green R. F., Ferguson D. H., Liebert J., Schmidt M., 1982, *PASP*, **94**, 560
- Green R. F., Schmidt M., Liebert J., 1986, *ApJS*, **61**, 305
- Gress O., et al., 2015, The Astronomer's Telegram, [7294](#), 1
- Gress O., et al., 2017, The Astronomer's Telegram, [10061](#), 1
- Groebele R., 2009, *BAV Rundbrief - Mitteilungsblatt der Berliner Arbeits-gemeinschaft fuer Veraenderliche Sterne*, **58**, 80
- Guthnick P., Prager R., 1926, *Astronomische Nachrichten*, **227**, 161
- Hackstein M., et al., 2015, *Astronomische Nachrichten*, **336**, 590
- Hagen H. J., Groote D., Engels D., Reimers D., 1995, *A&AS*, **111**, 195
- Halpern J. P., Mirabal N., 2006, The Astronomer's Telegram, [709](#), 1
- Halpern J. P., Thorstensen J. R., 2015, *AJ*, **150**, 170
- Hambach F. J., 2014, *AAVSO*, **42**, 324
- Hardy L. K., et al., 2017, *MNRAS*, **465**, 4968
- Hartwig Kempf Müller 1919, *Astronomische Nachrichten*, **208**, 57
- Heinze A. N., et al., 2018, *AJ*, **156**, 241
- Herbig G. H., 1958, *ApJ*, **128**, 259
- Hirayama T., Yamamoto M., Camilleri P., Sakurai Y., Collins M., Yamada M., Watanabe M., Baldwin M., 1993, *IAU Circ.*, **5791**, 1
- Hoard D. W., Szkody P., 1997, *ApJ*, **481**, 433
- Hodgkin S. T., et al., 2019a, Transient Name Server Discovery Report, [2019-1888](#), 1
- Hodgkin S. T., et al., 2019b, Transient Name Server Discovery Report, [2019-2107](#), 1
- Hodgkin S. T., et al., 2019c, Transient Name Server Discovery Report, [2019-2478](#), 1
- Hodgkin S. T., et al., 2020a, Transient Name Server Discovery Report, [2020-1817](#), 1
- Hodgkin S. T., et al., 2020b, Transient Name Server Discovery Report, [2020-768](#), 1
- Hodgkin S. T., et al., 2021a, *A&A*, **652**, A76
- Hodgkin S. T., et al., 2021b, Transient Name Server Discovery Report, [2021-594](#), 1
- Hodgkin S. T., et al., 2023, Transient Name Server Discovery Report, [2023-304](#), 1

- Hoffleit D., 1932, Harvard College Observatory Bulletin, **887**, 9
- Hoffmeister C., 1928, Mitteilungen der Sternwarte zu Sonneberg, **15**, 1
- Hoffmeister C., 1966a, *Astronomische Nachrichten*, **289**, 1
- Hoffmeister C., 1966b, *Astronomische Nachrichten*, **289**, 139
- Hoffmeister C., 1967a, *Astronomische Nachrichten*, **289**, 205
- Hoffmeister C., 1967b, *Astronomische Nachrichten*, **290**, 43
- Hoffmeister C., 1968, *Astronomische Nachrichten*, **290**, 277
- Homer L., et al., 2005, *ApJ*, **620**, 929
- Homer L., Szkody P., Henden A., Chen B., Schmidt G. D., Fraser O. J., West A. A., 2006, *AJ*, **132**, 2743
- Hou W., Luo A. I., Li Y.-B., Qin L., 2020, *AJ*, **159**, 43
- Howarth I. D., 1978a, Journal of the British Astronomical Association, **88**, 292
- Howarth I. D., 1978b, Journal of the British Astronomical Association, **88**, 608
- Hu J. Y., Qiu Y. L., Li W. D., Wei J. Y., Esamdin A., 1997, IAU Circ., **6731**, 1
- Huber M., et al., 2015, The Astronomer's Telegram, **7756**, 1
- Humason M. L., 1938, *ApJ*, **88**, 228
- Inight K. P., Copperwheat C. M., 2018, *Research Notes of the American Astronomical Society*, **2**, 222
- Inight K., et al., 2023a, *MNRAS*, **524**, 4867
- Inight K., et al., 2023b, *MNRAS*, **525**, 3597
- Israel G. L., Angelini L., Campana S., Giommi P., Stella L., White N. E., 1998, *MNRAS*, **298**, 502
- Ivezić Ž., et al., 2007, *AJ*, **134**, 973
- Jablonski F. J., Cieslinski D., 1992, *A&A*, **259**, 198
- Jayasinghe T., et al., 2018, *MNRAS*, **477**, 3145
- Jiang X. J., Engels D., Wei J. Y., Tesch F., Hu J. Y., 2000, *A&A*, **362**, 263
- Jones D. H., et al., 2009, *MNRAS*, **399**, 683
- Joshi V., 2013, in Astronomical Society of India Conference Series. p. 80
- Joshi A., Pandey J. C., Rawat N., Raj A., Wang W., Singh H. P., 2022, *AJ*, **163**, 221
- Kabath P., et al., 2009, *A&A*, **506**, 569
- Kamath U. S., Anupama G. C., Ashok N. M., Chandrasekhar T., 1997, *AJ*, **114**, 2671
- Kamath U. S., Anupama G. C., Ashok N. M., Mayya Y. D., Sahu D. K., 2005, *MNRAS*, **361**, 1165
- Kato T., 2022, *arXiv e-prints*, p. [arXiv:2203.06785](https://arxiv.org/abs/2203.06785)
- Kato T., Hambach F.-J., 2023, *arXiv e-prints*, p. [arXiv:2302.09782](https://arxiv.org/abs/2302.09782)
- Kato T., Romanov F. D., 2022, *arXiv e-prints*, p. [arXiv:2204.02598](https://arxiv.org/abs/2204.02598)
- Kato T., Ishioka R., Uemura M., Starkey D. R., Krajci T., 2004, *PASJ*, **56**, S125
- Kato T., et al., 2009, *PASJ*, **61**, S395
- Kato T., et al., 2010, *PASJ*, **62**, 1525
- Kato T., et al., 2012, *PASJ*, **64**, 21
- Kato T., et al., 2013, *PASJ*, **65**, 23
- Kato T., et al., 2014, *PASJ*, **66**, 30
- Kato T., et al., 2015, *PASJ*, **67**, 105
- Kato T., et al., 2016, *PASJ*, **68**, 65
- Kato T., et al., 2017, *PASJ*, **69**, 75
- Kato T., et al., 2020, *PASJ*, **72**, 14
- Khruslov A. V., Kusakin A. V., Barsukova E. A., Goranskij V. P., Valeev A. F., Samus N. N., 2015, *Research in Astronomy and Astrophysics*, **15**, 1005
- Kimura M., et al., 2016, *PASJ*, **68**, 55
- Kjurkchieva D., Khruzina T., Dimitrov D., Groebel R., Ibryamov S., Nikolov G., 2015, *A&A*, **584**, A40
- Kochanek C. S., et al., 2017, *PASP*, **129**, 104502
- Kozhevnikov V. P., 2016, *Ap&SS*, **361**, 273
- Kraft R. P., 1962, *ApJ*, **135**, 408
- Kraus A. L., Craine E. R., Giampapa M. S., Scharlach W. W. G., Tucker R. A., 2007, *AJ*, **134**, 1488
- Kreiner J. M., 2004, *Acta Astron.*, **54**, 207
- Kryachko T., Samokhvalov A., Satovskiy B., 2010, Information Bulletin on Variable Stars, **5952**, 1
- Littlefair S. P., Dhillon V. S., Marsh T. R., Gänsicke B. T., Southworth J., Baraffe I., Watson C. A., Copperwheat C., 2008, *MNRAS*, **388**, 1582
- Liu W., Hu J. Y., 2000, *ApJS*, **128**, 387
- Liu W., Hu J. Y., Zhu X. H., Li Z. Y., 1999, *ApJS*, **122**, 243
- Luo A. L., Zhao Y. H., Zhao G., et al. 2018, VizieR Online Data Catalog: LAMOST DR4 catalogs (Luo+, 2018), VizieR On-line Data Catalog: V/153. Originally published in: 2018RAA..in.prep..L
- Luyten W. J., 1933, *Astronomische Nachrichten*, **249**, 395
- Malkova A., et al., 2016, The Astronomer's Telegram, **8956**, 1
- Malkova A., et al., 2017, The Astronomer's Telegram, **10277**, 1
- Marin E., Shafter A. W., 2009, *PASP*, **121**, 1090
- Marsh T. R., et al., 2002, in Gänsicke B. T., Beuermann K., Reinsch K., eds, Astronomical Society of the Pacific Conference Series Vol. 261, The Physics of Cataclysmic Variables and Related Objects. p. 200 ([arXiv:astro-ph/0108334](https://arxiv.org/abs/astro-ph/0108334), doi:[10.48550/arXiv.astro-ph/0108334](https://doi.org/10.48550/arXiv.astro-ph/0108334))
- Masci F. J., et al., 2019, *PASP*, **131**, 018003
- Masetti N., et al., 2006, *A&A*, **459**, 21
- Masetti N., et al., 2010, *A&A*, **519**, A96
- Mason E., Howell S. B., 2003, *A&A*, **403**, 699
- Maza J., Hamuy M., Wischnjewsky M., Wells L., Phillips M., Barros S., 1990, IAU Circ., **5073**, 2
- Merloni A., et al., 2024, *A&A*, **682**, A34

- Miller W. J., 1971, *Ricerche Astronomiche*, **8**, 167
- Mobberley M. P., Barber P. M., Hurst G. M., 1997, *Journal of the British Astronomical Association*, **107**, 65
- Morgenroth O., 1934, *Astronomische Nachrichten*, **251**, 325
- Morokuma T., Tominaga N., Matsumoto E., Shibata T., Yamanaka M., Tanaka M., 2014, *Central Bureau Electronic Telegrams*, **4013**, 1
- Motch C., Haberl F., Guilloit P., Pakull M., Reinsch K., Krautter J., 1996, *A&A*, **307**, 459
- Motch C., et al., 1998, *A&AS*, **132**, 341
- Mowlavi N., et al., 2021, *A&A*, **648**, A44
- Munari U., Zwitter T., 1998, *A&AS*, **128**, 277
- Munari U., Bianchini A., Claudi R., 1990, *IAU Circ.*, **5024**, 2
- Nakano S., Tago A., Nishiyama K., Sakamoto T., 2007, *IAU Circ.*, **8821**, 1
- Oliveira A. S., Rodrigues C. V., Cieslinski D., Jablonski F. J., Silva K. M. G., Almeida L. A., Rodríguez-Ardila A., Palhares M. S., 2017, *AJ*, **153**, 144
- Oliveira A. S., Rodrigues C. V., Martins M., Palhares M. S., Silva K. M. G., Lima I. J., Jablonski F. J., 2020, *AJ*, **159**, 114
- Osawa K., Kuwano V., 1976, *IAU Circ.*, **2994**, 1
- Pala A. F., et al., 2020, *MNRAS*, **494**, 3799
- Parenago P. P., 1949, *Peremennye Zvezdy*, **7**, 109
- Parisi P., et al., 2014, *A&A*, **561**, A67
- Paterson K., Woudt P. A., Warner B., Breytenbach H., Gilligan C. K., Motsoaledi M., Thorstensen J. R., Worters H. L., 2019, *MNRAS*, **486**, 2422
- Patterson J., Thorstensen J. R., Fried R., Skillman D. R., Cook L. M., Jensen L., 2001, *PASP*, **113**, 72
- Patterson J., et al., 2003, *PASP*, **115**, 1308
- Peters C. S., Thorstensen J. R., 2005, *PASP*, **117**, 1386
- Peters C. S., Thorstensen J. R., 2006, *PASP*, **118**, 687
- Petit M., 1960, *Journal des Observateurs*, **43**, 17
- Poggiani R., 2009, *Astronomische Nachrichten*, **330**, 77
- Pojmanski G., 2002, *Acta Astron.*, **52**, 397
- Popova E., et al., 2015, *The Astronomer's Telegram*, **8172**, 1
- Pretorius M. L., 2009, *MNRAS*, **395**, 386
- Pretorius M. L., Knigge C., 2008a, *MNRAS*, **385**, 1471
- Pretorius M. L., Knigge C., 2008b, *MNRAS*, **385**, 1485
- Pretorius M. L., Knigge C., O'Donoghue D., Henry J. P., Gioia I. M., Mullis C. R., 2007, *MNRAS*, **382**, 1279
- Prins S., Telting J., Østensen R., 2019, *Open Astronomy*, **28**, 61
- Ramsay G., et al., 2018, *A&A*, **620**, A141
- Rau A., et al., 2007, *ApJ*, **664**, 474
- Remillard R. A., Stroozas B. A., Tapia S., Silber A., 1991, *ApJ*, **379**, 715
- Richter G. A., 1970, *Zentralinstitut fuer Astrophysik Sternwarte Sonneberg Mitteilungen ueber Veraenderliche Sterne*, **5**, 99
- Richter G. A., 1990, *Zentralinstitut fuer Astrophysik Sternwarte Sonneberg Mitteilungen ueber Veraenderliche Sterne*, **12**, 59
- Richter G. A., Notni P., Tiersch H., 1988, *Astronomische Nachrichten*, **309**, 91
- Ringwald F. A., Thorstensen J. R., Hamwey R. M., 1994, *MNRAS*, **271**, 323
- Ritter H., Kolb U., 2003, *A&A*, **404**, 301
- Rodríguez-Gil P., Schmidtobreick L., Gänsicke B. T., 2007a, *MNRAS*, **374**, 1359
- Rodríguez-Gil P., et al., 2007b, *MNRAS*, **377**, 1747
- Rodríguez A. C., et al., 2023, *ApJ*, **945**, 141
- Rosino L., Iijima T., Ortolani S., 1983, *MNRAS*, **205**, 1069
- Samus' N. N., Kazarovets E. V., Durevich O. V., Kireeva N. N., Pastukhova E. N., 2017, *Astronomy Reports*, **61**, 80
- Sanduleak N., 1975, *Information Bulletin on Variable Stars*, **1011**, 1
- Schaefer B. E., 2021, *Research Notes of the American Astronomical Society*, **5**, 150
- Schaefer B. E., 2022, *MNRAS*, **517**, 3640
- Schaefer B. E., et al., 2019, *MNRAS*, **487**, 1120
- Schlegel E. M., Honeycutt R. K., 2019, *ApJ*, **876**, 152
- Schmidt G. D., et al., 2005a, *ApJ*, **620**, 422
- Schmidt G. D., et al., 2005b, *ApJ*, **630**, 1037
- Schwarz R., Greiner J., Tovmassian G. H., Zharikov S. V., Wenzel W., 2002, *A&A*, **392**, 505
- Schwöpe A. D., Buckley D. A. H., O'Donoghue D., Hasinger G., Truemper J., Voges W., 1997, *A&A*, **326**, 195
- Schwöpe A., et al., 2024, *A&A*, **686**, A110
- Shafter A. W., 1983, PhD thesis, University of California, Los Angeles
- Shapley H., Boyce E. H., Boyd C. D., 1940, *Annals of Harvard College Observatory*, **90**, 239
- Shappee B. J., et al., 2013, *The Astronomer's Telegram*, **5052**, 1
- Shappee B. J., et al., 2014, *ApJ*, **788**, 48
- Shears J., Pickard R., Krajci T., Poyner G., 2008a, *Journal of the British Astronomical Association*, **118**, 145
- Shears J., Boyd D., Brady S., Pickard R., 2008b, *Journal of the British Astronomical Association*, **118**, 343
- Sheets H. A., Thorstensen J. R., Peters C. J., Kapusta A. B., Taylor C. J., 2007, *PASP*, **119**, 494
- Shimansky V. V., Nurtudinova D. N., Borisov N. V., Spiridonova O. I., 2011, *Astrophysical Bulletin*, **66**, 442
- Shore S. N., De Gennaro Aquino I., Schwarz G. J., Augusteijn T., Cheung C. C., Walter F. M., Starrfield S., 2013, *A&A*, **553**, A123
- Shumkov V., et al., 2014, *The Astronomer's Telegram*, **6833**, 1
- Shumkov V., et al., 2017, *The Astronomer's Telegram*, **10790**, 1
- Silber A. D., Remillard R. A., Horne K., Bradt H. V., 1994, *ApJ*, **424**, 955
- Simonian G., et al., 2014, *The Astronomer's Telegram*, **6608**, 1
- Siviero A., Munari U., 2016, *The Astronomer's Telegram*, **9862**, 1
- Skiff B. A., 1999, *Information Bulletin on Variable Stars*, **4675**, 1

- Southworth J., Gänsicke B. T., Marsh T. R., de Martino D., Hakala P., Littlefair S., Rodríguez-Gil P., Szkody P., 2006, *MNRAS*, **373**, 687
- Southworth J., Marsh T. R., Gänsicke B. T., Aungwerojwit A., Hakala P., de Martino D., Lehto H., 2007, *MNRAS*, **382**, 1145
- Southworth J., et al., 2008, *MNRAS*, **391**, 591
- Southworth J., Marsh T. R., Gänsicke B. T., Steeghs D., Copperwheat C. M., 2010, *A&A*, **524**, A86
- Southworth J., Tappert C., Gänsicke B. T., Copperwheat C. M., 2015, *A&A*, **573**, A61
- Stanek K. Z., 2017, Transient Name Server Discovery Report, [2017-1324](#), 1
- Stanek K. Z., et al., 2013a, The Astronomer's Telegram, [5118](#), 1
- Stanek K. Z., et al., 2013b, The Astronomer's Telegram, [5186](#), 1
- Stanek K. Z., Kochanek C. S., Shields J. V., Thompson T. A., Holoien T. W. S., Shappee B. J., Prieto J. L., Dong S., 2018, The Astronomer's Telegram, [11300](#), 1
- Stanishev V., Kraicheva Z., Genkov V., 2006, *A&A*, **455**, 223
- Stefanov S. Y., Stefanov A. K., 2023, *MNRAS*, **520**, 3355
- Stobie R. S., Kilkenney D., O'Donoghue D., 1995, *Ap&SS*, **230**, 101
- Sun Y., et al., 2021, *ApJS*, **257**, 65
- Swierczynski E., et al., 2010, in Prša A., Zejda M., eds, *Astronomical Society of the Pacific Conference Series Vol. 435, Binaries - Key to Comprehension of the Universe*. p. 297 ([arXiv:0909.5149](#)), doi:10.48550/arXiv.0909.5149
- Szkody P., 1985, *AJ*, **90**, 1837
- Szkody P., 1987, *ApJS*, **63**, 685
- Szkody P., Howell S. B., 1992, *ApJS*, **78**, 537
- Szkody P., Mateo M., 1986, *AJ*, **92**, 483
- Szkody P., et al., 2002, *AJ*, **123**, 430
- Szkody P., et al., 2003a, *AJ*, **126**, 1499
- Szkody P., et al., 2003b, *ApJ*, **583**, 902
- Szkody P., et al., 2004, *AJ*, **128**, 1882
- Szkody P., et al., 2005, *AJ*, **129**, 2386
- Szkody P., et al., 2006, *AJ*, **131**, 973
- Szkody P., et al., 2007, *AJ*, **134**, 185
- Szkody P., et al., 2009, *AJ*, **137**, 4011
- Szkody P., et al., 2011, *AJ*, **142**, 181
- Szkody P., Everett M. E., Howell S. B., Landolt A. U., Bond H. E., Silva D. R., Vazquez-Soltero S., 2014, *AJ*, **148**, 63
- Szkody P., Everett M. E., Dai Z., Serna-Grey D., 2018, *AJ*, **155**, 28
- Szkody P., et al., 2020, *AJ*, **159**, 198
- Tappert C., Augusteijn T., Maza J., 2004, *MNRAS*, **354**, 321
- Tappert C., Ederoclitte A., Mennickent R. E., Schmidtbreick L., Vogt N., 2012, *MNRAS*, **423**, 2476
- Tappert C., Vogt N., Schmidtbreick L., Ederoclitte A., Vanderbeke J., 2013, *MNRAS*, **431**, 92
- Tappert C., Vogt N., Della Valle M., Schmidtbreick L., Ederoclitte A., 2014, *MNRAS*, **442**, 565
- Taylor C. J., Thorstensen J. R., 1996, *PASP*, **108**, 894
- Tebbutt J., 1878, *MNRAS*, **38**, 330
- Teyssier F., 2019, The Astronomer's Telegram, [12936](#), 1
- Thorstensen J. R., 1986, *AJ*, **91**, 940
- Thorstensen J. R., 1997, *PASP*, **109**, 1241
- Thorstensen J. R., 2013, *PASP*, **125**, 506
- Thorstensen J. R., 2020, *AJ*, **160**, 6
- Thorstensen J. R., Freed I. W., 1985, *AJ*, **90**, 2082
- Thorstensen J. R., Halpern J. P., 2009, The Astronomer's Telegram, [2177](#), 1
- Thorstensen J. R., Halpern J., 2013, *AJ*, **146**, 107
- Thorstensen J. R., Skinner J. N., 2012, *AJ*, **144**, 81
- Thorstensen J. R., Taylor C. J., 1997, *PASP*, **109**, 1359
- Thorstensen J. R., Taylor C. J., 2000, *MNRAS*, **312**, 629
- Thorstensen J. R., Taylor C. J., 2001, *MNRAS*, **326**, 1235
- Thorstensen J. R., Patterson J. O., Shambrook A., Thomas G., 1996, *PASP*, **108**, 73
- Thorstensen J. R., Taylor C. J., Becker C. M., Remillard R. A., 1997, *PASP*, **109**, 477
- Thorstensen J. R., Patterson J., Kemp J., Vennes S., 2002, *PASP*, **114**, 1108
- Thorstensen J. R., Fenton W. H., Taylor C. J., 2004, *PASP*, **116**, 300
- Thorstensen J. R., Peters C. S., Sheets H. A., Skinner J. N., 2009, in *American Astronomical Society Meeting Abstracts #213*. p. 491.07
- Thorstensen J. R., Peters C. S., Skinner J. N., 2010, *PASP*, **122**, 1285
- Thorstensen J. R., Taylor C. J., Peters C. S., Skinner J. N., Southworth J., Gänsicke B. T., 2015, *AJ*, **149**, 128
- Thorstensen J. R., Alper E. H., Weil K. E., 2016, *AJ*, **152**, 226
- Thorstensen J. R., Ringwald F. A., Taylor C. J., Sheets H. A., Peters C. S., Skinner J. N., Alper E. H., Weil K. E., 2017, *Research Notes of the American Astronomical Society*, **1**, 29
- Thorstensen J. R., Motsoaledi M., Woudt P. A., Buckley D. A. H., Warner B., 2020, *AJ*, **160**, 70
- Thorstensen J. R., Alvarado-Anderson C. K., Burrows A. D., Goebel-Bain R. M., Katz D. C., 2023, *AJ*, **166**, 131
- Tovmassian G., et al., 2017, *A&A*, **608**, A36
- Uemura M., Kato T., Nogami D., Ohsugi T., 2010, *PASJ*, **62**, 613
- Unda-Sanzana E., et al., 2008, *MNRAS*, **388**, 889
- Vladimirov V., et al., 2014, The Astronomer's Telegram, [5950](#), 1
- Vladimirov V., et al., 2017, The Astronomer's Telegram, [10415](#), 1
- Vogt N., 1980, *A&A*, **88**, 66

- Vogt N., Bateson F. M., 1982, *A&AS*, **48**, 383
- Wagner R. M., Terndrup D., Darnley M. J., Starrfield S., Woodward C. E., Henze M., 2018, *The Astronomer's Telegram*, **11588**, 1
- Watson C. L., Henden A. A., Price A., 2006, *Society for Astronomical Sciences Annual Symposium*, **25**, 47
- Watson C., Henden A. A., Price A., 2017, *VizieR Online Data Catalog: AAVSO International Variable Star Index VSX (Watson+, 2006-2014)*, *VizieR On-line Data Catalog: B/vsx*. Originally published in: 2006SASS...25...47W
- Wei J., Li C., Xu D., Hu J., Li Q., 1997, *Acta Astrophysica Sinica*, **17**, 107
- Wei J. Y., Xu D. W., Dong X. Y., Hu J. Y., 1999, *A&AS*, **139**, 575
- Welsh B. Y., et al., 2005, *AJ*, **130**, 825
- Williams G., 1983, *ApJS*, **53**, 523
- Wils P., Gänsicke B. T., Drake A. J., Southworth J., 2010, *MNRAS*, **402**, 436
- Witham A. R., et al., 2007, *MNRAS*, **382**, 1158
- Witham A. R., Knigge C., Drew J. E., Greimel R., Steeghs D., Gänsicke B. T., Groot P. J., Mampaso A., 2008, *MNRAS*, **384**, 1277
- Woudt P. A., Warner B., 2010, *MNRAS*, **403**, 398
- Woudt P. A., Warner B., de Budé D., Macfarlane S., Schurch M. P. E., Zietsman E., 2012, *MNRAS*, **421**, 2414
- Wright D., et al., 2012, *The Astronomer's Telegram*, **4516**, 1
- Wyse A. B., 1936, *PASP*, **48**, 302
- Yakin D. G., Suleimanov V. F., Borisov N. V., Shimanskii V. V., Bikmaev I. F., 2011, *Astronomy Letters*, **37**, 845
- Yecheistov V., et al., 2013a, *The Astronomer's Telegram*, **4857**, 1
- Yecheistov V., et al., 2013b, *The Astronomer's Telegram*, **5536**, 1
- Zharikov S. V., Tovmassian G. H., Napiwotzki R., Michel R., Neustroev V., 2006, *A&A*, **449**, 645
- Zubareva A. M., Pavlenko E. P., Andreev M. V., Antipin S. V., Samus' N. N., Sergeev A. V., 2011, *Astronomy Reports*, **55**, 224
- di Cicco D., Vitorino C., Green D. W. E., 1999, *IAU Circ.*, **7323**, 1

This paper has been typeset from a  $\text{\LaTeX}$  file prepared by the author.
